# Supplementary material for: Many, many more intrinsically knotted graphs
Source: arXiv:1109.1632 ancillary file (2012-05-22)
Supplement: Supplementary file 1 [file many-appendix.pdf]

# Many, many more intrinsically knotted graphs: Appendix

NOAM GOLDBERG, THOMAS W. MATTMAN, AND RAMIN NAIMI

In this appendix we provide edge lists, and family diagrams when possible, for the graphs we mention in [1]. A more user-friendly version of this appendix can be found online at <http://faculty.oxy.edu/rnaimi/CV/publications/many-appendix/>

## References

[1] N. Goldberg, T. W. Mattman, R. Naimi. *Many, many more intrinsically knotted graphs*. Preprint. <http://faculty.oxy.edu/rnaimi/CV/publications/Many.pdf>

## Contents:

Section 1: K7 family

Section 2: K3311 family

Section 3: E9+e family

Section 4: G9,28 family

Diagrams for each family appear at the bottom of each section.

## Section 1:

### Edgelist for graphs in the K<sub>7</sub> family

The K7 family consists of 20 graphs (diagram at bottom). Six of them, Cousins 9, 14, 16, 17, 19, and 20, are not IK. The remaining 14 are MMIK.

K<sub>7</sub> is Cousin 1.

Cousin 1:  $\{\{1,2\},\{1,3\},\{1,4\},\{1,5\},\{1,6\},\{1,7\},\{2,3\},\{2,4\},\{2,5\},\{2,6\},\{2,7\},\{3,4\},\{3,5\},\{3,6\},\{3,7\},\{4,5\},\{4,6\},\{4,7\},\{5,6\},\{5,7\},\{6,7\}\}$

Cousin 2:  $\{\{1,4\},\{1,5\},\{1,6\},\{1,7\},\{1,8\},\{2,4\},\{2,5\},\{2,6\},\{2,7\},\{2,8\},\{3,4\},\{3,5\},\{3,6\},\{3,7\},\{3,8\},\{4,5\},\{4,6\},\{4,7\},\{5,6\},\{5,7\},\{6,7\}\}$

Cousin 3:  $\{\{1,6\},\{1,7\},\{1,8\},\{1,9\},\{2,4\},\{2,5\},\{2,6\},\{2,7\},\{2,8\},\{3,4\},\{3,5\},\{3,6\},\{3,7\},\{3,8\},\{4,6\},\{4,7\},\{4,9\},\{5,6\},\{5,7\},\{5,9\},\{6,7\}\}$

Cousin 4:  $\{\{1,4\},\{1,5\},\{1,6\},\{1,7\},\{1,8\},\{2,4\},\{2,5\},\{2,6\},\{2,7\},\{2,8\},\{3,4\},\{3,5\},\{3,6\},\{3,7\},\{3,8\},\{4,7\},\{4,9\},\{5,7\},\{5,9\},\{6,7\},\{6,9\}\}$

Cousin 5:  $\{\{1,8\},\{1,9\},\{1,10\},\{2,4\},\{2,5\},\{2,6\},\{2,7\},\{2,8\},\{3,4\},\{3,5\},\{3,6\},\{3,7\},\{3,8\},\{4,6\},\{4,7\},\{4,9\},\{5,6\},\{5,7\},\{5,9\},\{6,10\},\{7,10\}\}$

Cousin 6:  $\{\{1,6\},\{1,7\},\{1,8\},\{1,9\},\{2,5\},\{2,7\},\{2,8\},\{2,10\},\{3,4\},\{3,5\},\{3,6\},\{3,7\},\{3,8\},\{4,7\},\{4,9\},\{4,10\},\{5,6\},\{5,7\},\{5,9\},\{6,7\},\{6,10\}\}$

Cousin 7:  $\{\{1,6\},\{1,7\},\{1,8\},\{1,9\},\{2,4\},\{2,5\},\{2,8\},\{2,10\},\{3,4\},\{3,5\},\{3,6\},\{3,7\},\{3,8\},\{4,6\},\{4,7\},\{4,9\},\{5,6\},\{5,7\},\{5,9\},\{6,10\},\{7,10\}\}$

Cousin 8:  $\{\{1,8\},\{1,9\},\{1,10\},\{2,5\},\{2,7\},\{2,8\},\{2,11\},\{3,4\},\{3,5\},\{3,6\},\{3,7\},\{3,8\},\{4,7\},\{4,9\},\{4,11\},\{5,6\},\{5,7\},\{5,9\},\{6,10\},\{6,11\},\{7,10\}\}$

Cousin 9:  $\{\{1,6\},\{1,7\},\{1,8\},\{1,9\},\{2,4\},\{2,5\},\{2,6\},\{2,7\},\{2,8\},\{3,4\},\{3,5\},\{3,6\},\{3,7\},\{3,8\},\{4,6\},\{4,7\},\{4,9\},\{5,6\},\{5,7\},\{5,9\},\{8,9\}\}$

Cousin 10:  $\{\{1,6\},\{1,7\},\{1,8\},\{1,9\},\{2,5\},\{2,7\},\{2,8\},\{2,10\},\{3,4\},\{3,7\},\{3,8\},\{3,11\},\{4,7\},\{4,9\},\{4,10\},\{5,7\},\{5,9\},\{5,11\},\{6,7\},\{6,10\},\{6,11\}\}$

Cousin 11:  $\{\{1,6\},\{1,7\},\{1,8\},\{1,9\},\{2,5\},\{2,7\},\{2,8\},\{2,10\},\{3,4\},\{3,6\},\{3,8\},\{3,11\},\{4,7\},\{4,9\},\{4,10\},\{5,6\},\{5,9\},\{5,11\},\{6,7\},\{6,10\},\{7,11\}\}$

Cousin 12:  $\{\{1,8\},\{1,9\},\{1,10\},\{2,8\},\{2,11\},\{2,12\},\{3,4\},\{3,5\},\{3,6\},\{3,7\},\{3,8\},\{4,7\},\{4,9\},\{4,11\},\{5,6\},\{5,9\},\{5,12\},\{6,10\},\{6,11\},\{7,10\},\{7,12\}\}$

Cousin 13:  $\{\{1,8\},\{1,9\},\{1,10\},\{2,5\},\{2,7\},\{2,8\},\{2,11\},\{3,4\},\{3,6\},\{3,8\},\{3,12\},\{4,7\},\{4,9\},\{4,11\},\{5,6\},\{5,9\},\{5,12\},\{6,10\},\{6,11\},\{7,10\},\{7,12\}\}$

Cousin 14:  $\{\{1,2\},\{1,4\},\{1,6\},\{2,5\},\{2,7\},\{2,8\},\{3,4\},\{3,5\},\{3,6\},\{3,7\},\{3,8\},\{4,7\},\{4,9\},\{5,6\},\{5,7\},\{5,9\},\{6,10\},\{7,10\},\{8,9\},\{8,10\},\{9,10\}\}$

Cousin 15:  $\{\{1,8\},\{1,9\},\{1,10\},\{2,8\},\{2,11\},\{2,12\},\{3,5\},\{3,6\},\{3,8\},\{3,13\},\{4,9\},\{4,11\},\{4,13\},\{5,6\},\{5,9\},\{5,12\},\{6,10\},\{6,11\},\{7,10\},\{7,12\},\{7,13\}\}$

Cousin 16:  $\{\{1,2\},\{1,5\},\{1,7\},\{2,8\},\{2,11\},\{3,4\},\{3,5\},\{3,6\},\{3,7\},\{3,8\},\{4,7\},\{4,9\},\{4,11\},\{5,6\},\{5,9\},\{6,10\},\{6,11\},\{7,10\},\{8,9\},\{8,10\},\{9,10\}\}$

Cousin 17:  $\{\{1,3\},\{1,5\},\{1,7\},\{2,5\},\{2,7\},\{2,8\},\{2,11\},\{3,4\},\{3,6\},\{3,8\},\{4,7\},\{4,9\},\{4,11\},\{5,6\},\{5,9\},\{6,10\},\{6,11\},\{7,10\},\{8,9\},\{8,10\},\{9,10\}\}$

Cousin 18:  $\{\{1,8\},\{1,9\},\{1,10\},\{2,8\},\{2,11\},\{2,12\},\{3,8\},\{3,13\},\{3,14\},\{4,9\},\{4,11\},\{4,13\},\{5,9\},\{5,12\},\{5,14\},\{6,10\},\{6,11\},\{6,14\},\{7,10\},\{7,12\},\{7,13\}\}$

Cousin 19:  $\{\{1,3\},\{1,4\},\{1,7\},\{2,8\},\{2,11\},\{2,12\},\{3,5\},\{3,6\},\{3,8\},\{4,9\},\{4,11\},\{5,6\},\{5,9\},\{5,12\},\{6,10\},\{6,11\},\{7,10\},\{7,12\},\{8,9\},\{8,10\},\{9,10\}\}$

Cousin 20:  $\{\{1,2\},\{1,5\},\{1,7\},\{1,8\},\{2,4\},\{2,6\},\{2,8\},\{3,4\},\{3,5\},\{3,6\},\{3,7\},\{3,8\},\{4,7\},\{4,9\},\{5,6\},\{5,9\},\{6,10\},\{7,10\},\{8,9\},\{8,10\},\{9,10\}\}$

Diagram for the  $K_7$  family:

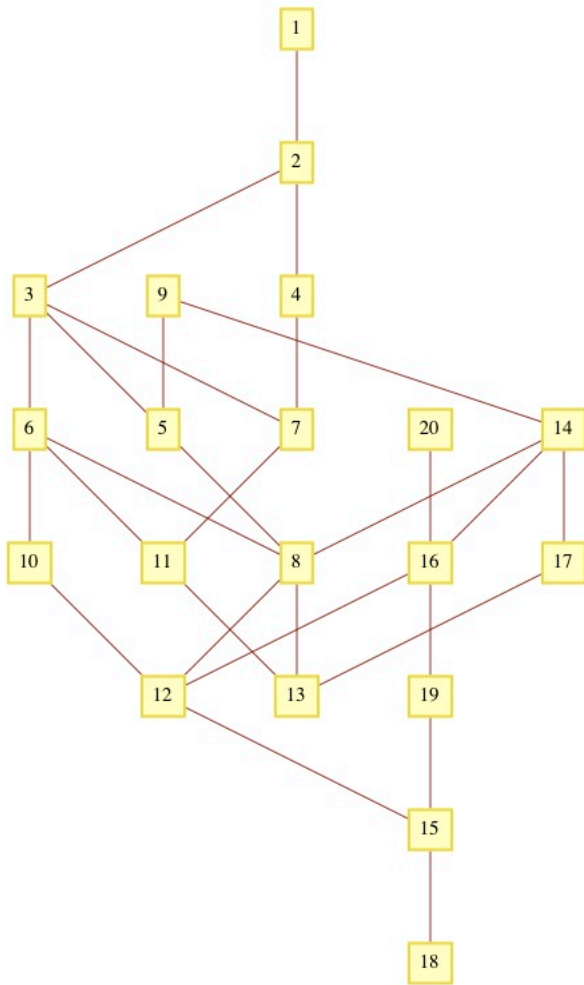

## Section 2:

### Edge lists for graphs in the $K_{\{3,3,1,1\}}$ family

The  $K_{3311}$  family consists of 58 graphs, all of which are MMIK.

$K_{3311}$  is Cousin 1.

Cousin 1 :

$\{\{1,4\},\{1,5\},\{1,6\},\{1,7\},\{1,8\},\{2,4\},\{2,5\},\{2,6\},\{2,7\},\{2,8\},\{3,4\},\{3,5\},\{3,6\},\{3,7\},\{3,8\},\{4,7\},\{4,8\},\{5,7\},\{5,8\},\{6,7\},\{6,8\},\{7,8\}\}$

Cousin 2 :

$\{\{1,5\},\{1,6\},\{1,8\},\{1,9\},\{2,4\},\{2,5\},\{2,6\},\{2,7\},\{2,8\},\{3,4\},\{3,5\},\{3,6\},\{3,7\},\{3,8\},\{4,8\},\{4,9\},\{5,7\},\{5,8\},\{6,7\},\{6,8\},\{7,8\},\{7,9\}\}$

Cousin 3 :

$\{\{1,4\},\{1,5\},\{1,6\},\{1,9\},\{2,4\},\{2,5\},\{2,6\},\{2,7\},\{2,8\},\{3,4\},\{3,5\},\{3,6\},\{3,7\},\{3,8\},\{4,7\},\{4,8\},\{5,7\},\{5,8\},\{6,7\},\{6,8\},\{7,9\},\{8,9\}\}$

Cousin 4 :

$\{\{1,6\},\{1,9\},\{1,10\},\{2,4\},\{2,5\},\{2,6\},\{2,7\},\{2,8\},\{3,4\},\{3,5\},\{3,6\},\{3,7\},\{3,8\},\{4,8\},\{4,9\},\{5,7\},\{5,10\},\{6,7\},\{6,8\},\{7,8\},\{7,9\},\{8,10\}\}$

Cousin 5 :

{{1,5},{1,6},{1,8},{1,9},{2,4},{2,6},{2,8},{2,10},{3,4},{3,5},{3,6},{3,7},{3,8},{4,8},{4,9},{5,8},{5,10},{6,7},{6,8},{7,8},{7,9},{7,10}}

Cousin 6 :

{{1,5},{1,6},{1,8},{1,9},{2,4},{2,6},{2,7},{2,10},{3,4},{3,5},{3,6},{3,7},{3,8},{4,8},{4,9},{5,7},{5,10},{6,7},{6,8},{7,8},{7,9},{8,10}}

Cousin 7 :

{{1,5},{1,6},{1,8},{1,9},{2,4},{2,5},{2,6},{2,10},{3,4},{3,5},{3,6},{3,7},{3,8},{4,8},{4,9},{5,7},{5,8},{6,7},{6,8},{7,9},{7,10},{8,10}}

Cousin 8 :

{{1,6},{1,9},{1,10},{2,5},{2,6},{2,7},{2,11},{3,4},{3,5},{3,6},{3,7},{3,8},{4,9},{4,11},{5,7},{5,10},{6,7},{6,8},{7,8},{7,9},{8,10},{8,11}}

Cousin 9 :

{{1,6},{1,9},{1,10},{2,4},{2,5},{2,8},{2,11},{3,4},{3,5},{3,6},{3,7},{3,8},{4,8},{4,9},{5,7},{5,10},{6,8},{6,11},{7,8},{7,9},{7,11},{8,10}}

Cousin 10 :

{{1,6},{1,9},{1,10},{2,4},{2,5},{2,6},{2,11},{3,4},{3,5},{3,6},{3,7},{3,8},{4,8},{4,9},{5,7},{5,10},{6,7},{6,8},{7,9},{7,11},{8,10},{8,11}}

Cousin 11 :

{{1,6},{1,9},{1,10},{2,4},{2,5},{2,6},{2,7},{2,8},{3,4},{3,5},{3,6},{3,7},{3,8},{4,8},{4,9},{5,7},{5,10},{6,11},{7,9},{7,11},{8,10},{8,11}}

Cousin 12 :

{{1,5},{1,6},{1,8},{1,9},{2,4},{2,5},{2,6},{2,7},{2,8},{3,4},{3,5},{3,6},{3,7},{3,8},{4,8},{4,9},{5,7},{6,7},{6,8},{6,9},{7,8},{7,9}}

Cousin 13 :

{{1,5},{1,6},{1,8},{1,9},{2,4},{2,6},{2,8},{2,10},{3,4},{3,5},{3,8},{3,11},{4,8},{4,9},{5,8},{5,10},{6,8},{6,11},{7,8},{7,9},{7,10},{7,11}}

Cousin 14 :

{{1,5},{1,6},{1,8},{1,9},{2,4},{2,6},{2,8},{2,10},{3,4},{3,5},{3,7},{3,11},{4,8},{4,9},{5,8},{5,10},{6,7},{6,11},{7,8},{7,9},{7,10},{8,11}}

Cousin 15 :

{{1,5},{1,6},{1,8},{1,9},{2,4},{2,6},{2,8},{2,10},{3,4},{3,5},{3,6},{3,11},{4,8},{4,9},{5,8},{5,10},{6,7},{6,8},{7,9},{7,10},{7,11},{8,11}}

Cousin 16 :

{{1,5},{1,6},{1,8},{1,9},{2,4},{2,6},{2,7},{2,10},{3,4},{3,5},{3,6},{3,11},{4,8},{4,9},{5,7},{5,10},{6,7},{6,8},{7,9},{7,11},{8,10},{8,11}}

Cousin 17 :

{{1,6},{1,9},{1,10},{2,6},{2,11},{2,12},{3,4},{3,5},{3,6},{3,7},{3,8},{4,9},{4,11},{5,10},{5,12},{6,7},{6,8},{7,8},{7,9},{7,12},{8,10},{8,11}}

Cousin 18 :

{{1,6},{1,9},{1,10},{2,5},{2,11},{2,12},{3,4},{3,5},{3,6},{3,7},{3,8},{4,9},{4,11},{5,7},{5,10},{6,8},{6,12},{7,8},{7,9},{7,12},{8,10},{8,11}}

Cousin 19 :

{{1,6},{1,9},{1,10},{2,5},{2,6},{2,7},{2,11},{3,4},{3,5},{3,8},{3,12},{4,9},{4,11},{5,7},{5,10},{6,8},{6,12},{7,8},{7,9},{7,12},{8,10},{8,11}}

Cousin 20 :

{{1,6},{1,9},{1,10},{2,5},{2,6},{2,7},{2,11},{3,4},{3,5},{3,7},{3,12},{4,9},{4,11},{5,7},{5,10},{6,7},{6,12},{7,8},{7,9},{8,10},{8,11},{8,12}}

Cousin 21 :

{{1,6},{1,9},{1,10},{2,5},{2,6},{2,7},{2,11},{3,4},{3,5},{3,6},{3,12},{4,9},{4,11},{5,7},{5,10},{6,7},{6,8},{7,9},{7,12},{8,10},{8,11},{8,12}}

Cousin 22 :

{{1,2},{1,4},{1,8},{2,5},{2,6},{2,7},{3,4},{3,5},{3,6},{3,7},{3,8},{4,9},{5,7},{5,10},{6,7},{6,8},{6,9},{6,10},{7,8},{7,9},{8,10},{9,10}}

Cousin 23 :

{{1,6},{1,9},{1,10},{2,4},{2,5},{2,8},{2,11},{3,4},{3,5},{3,7},{3,12},{4,8},{4,9},{5,7},{5,10},{6,11},{6,12},{7,8},{7,9},{7,11},{8,10},{8,12}}

Cousin 24 :

{{1,6},{1,9},{1,10},{2,4},{2,5},{2,8},{2,11},{3,4},{3,5},{3,6},{3,12},{4,8},{4,9},{5,7},{5,10},{6,8},{6,11},{7,9},{7,11},{7,12},{8,10},{8,12}}

Cousin 25 :

{{1,2},{1,6},{1,7},{2,4},{2,5},{2,8},{3,4},{3,5},{3,6},{3,7},{3,8},{4,8},{4,9},{5,7},{5,10},{6,8},{6,9},{6,10},{7,8},{7,9},{8,10},{9,10}}

Cousin 26 :

{{1,2},{1,7},{1,8},{2,4},{2,5},{2,6},{3,4},{3,5},{3,6},{3,7},{3,8},{4,8},{4,9},{5,7},{5,10},{6,7},{6,8},{6,9},{6,10},{7,9},{8,10},{9,10}}

Cousin 27 :

{{1,6},{1,7},{1,8},{2,4},{2,5},{2,6},{2,7},{2,8},{3,4},{3,5},{3,6},{3,7},{3,8},{4,8},{4,9},{5,7},{5,10},{6,9},{6,10},{7,9},{8,10},{9,10}}

Cousin 28 :

{{1,5},{1,9},{1,10},{2,4},{2,5},{2,6},{2,7},{2,8},{3,4},{3,5},{3,6},{3,7},{3,8},{4,8},{4,9},{5,7},{6,7},{6,9},{6,10},{7,8},{7,9},{8,10}}

Cousin 29 :

{{1,6},{1,9},{1,10},{2,6},{2,11},{2,12},{3,4},{3,5},{3,8},{3,13},{4,9},{4,11},{5,10},{5,12},{6,8},{6,13},{7,8},{7,9},{7,12},{7,13},{8,10},{8,11}}

Cousin 30 :

$\{\{1,6\},\{1,9\},\{1,10\},\{2,5\},\{2,11\},\{2,12\},\{3,4\},\{3,6\},\{3,8\},\{3,13\},\{4,9\},\{4,11\},\{5,10\},\{5,13\},\{6,8\},\{6,12\},\{7,8\},\{7,9\},\{7,12\},\{7,13\},\{8,10\},\{8,11\}\}$

Cousin 31 :

$\{\{1,6\},\{1,9\},\{1,10\},\{2,5\},\{2,11\},\{2,12\},\{3,4\},\{3,5\},\{3,6\},\{3,13\},\{4,9\},\{4,11\},\{5,7\},\{5,10\},\{6,8\},\{6,12\},\{7,9\},\{7,12\},\{7,13\},\{8,10\},\{8,11\},\{8,13\}\}$

Cousin 32 :

$\{\{1,2\},\{1,6\},\{1,7\},\{2,5\},\{2,11\},\{3,4\},\{3,5\},\{3,6\},\{3,7\},\{3,8\},\{4,9\},\{4,11\},\{5,7\},\{5,10\},\{6,8\},\{6,9\},\{6,10\},\{7,8\},\{7,9\},\{8,10\},\{8,11\},\{9,10\}\}$

Cousin 33 :

$\{\{1,6\},\{1,9\},\{1,10\},\{2,4\},\{2,5\},\{2,11\},\{3,5\},\{3,6\},\{3,7\},\{3,8\},\{3,9\},\{3,11\},\{4,6\},\{4,7\},\{5,7\},\{5,10\},\{6,8\},\{7,8\},\{7,9\},\{8,10\},\{8,11\},\{9,11\}\}$

Cousin 34 :

$\{\{1,3\},\{1,6\},\{1,7\},\{2,5\},\{2,6\},\{2,7\},\{2,11\},\{3,4\},\{3,5\},\{3,8\},\{4,9\},\{4,11\},\{5,7\},\{5,10\},\{6,8\},\{6,9\},\{6,10\},\{7,8\},\{7,9\},\{8,10\},\{8,11\},\{9,10\}\}$

Cousin 35 :

$\{\{1,3\},\{1,6\},\{1,8\},\{2,5\},\{2,6\},\{2,7\},\{2,11\},\{3,4\},\{3,5\},\{3,7\},\{4,9\},\{4,11\},\{5,7\},\{5,10\},\{6,7\},\{6,9\},\{6,10\},\{7,8\},\{7,9\},\{8,10\},\{8,11\},\{9,10\}\}$

Cousin 36 :

$\{\{1,3\},\{1,6\},\{1,8\},\{2,4\},\{2,5\},\{2,8\},\{2,11\},\{3,4\},\{3,5\},\{3,7\},\{4,8\},\{4,9\},\{5,7\},\{5,10\},\{6,9\},\{6,10\},\{6,11\},\{7,8\},\{7,9\},\{7,11\},\{8,10\},\{9,10\}\}$

Cousin 37 :

$\{\{1,3\},\{1,7\},\{1,8\},\{2,4\},\{2,5\},\{2,8\},\{2,11\},\{3,4\},\{3,5\},\{3,6\},\{4,8\},\{4,9\},\{5,7\},\{5,10\},\{6,8\},\{6,9\},\{6,10\},\{6,11\},\{7,9\},\{7,11\},\{8,10\},\{9,10\}\}$

Cousin 38 :

$\{\{1,2\},\{1,6\},\{1,7\},\{2,4\},\{2,5\},\{2,8\},\{3,4\},\{3,5\},\{3,6\},\{3,7\},\{3,8\},\{4,8\},\{4,9\},\{5,7\},\{5,10\},\{6,9\},\{6,11\},\{7,8\},\{7,9\},\{8,11\},\{9,10\},\{10,11\}\}$

Cousin 39 :

$\{\{1,2\},\{1,7\},\{1,8\},\{2,4\},\{2,5\},\{2,6\},\{3,4\},\{3,5\},\{3,6\},\{3,7\},\{3,8\},\{4,8\},\{4,9\},\{5,7\},\{5,10\},\{6,8\},\{6,10\},\{6,11\},\{7,11\},\{8,10\},\{9,10\},\{9,11\}\}$

Cousin 40 :

$\{\{1,5\},\{1,9\},\{1,10\},\{2,4\},\{2,5\},\{2,6\},\{2,7\},\{2,8\},\{3,4\},\{3,5\},\{3,6\},\{3,7\},\{3,8\},\{4,8\},\{4,9\},\{5,7\},\{6,10\},\{6,11\},\{7,8\},\{7,11\},\{8,10\},\{9,11\}\}$

Cousin 41 :

$\{\{1,5\},\{1,6\},\{1,8\},\{1,9\},\{2,4\},\{2,5\},\{2,6\},\{2,7\},\{2,8\},\{3,4\},\{3,5\},\{3,6\},\{3,7\},\{3,8\},\{4,8\},\{4,9\},\{5,7\},\{5,9\},\{6,7\},\{6,9\},\{7,8\},\{7,9\}\}$

Cousin 42 :

$\{\{1,6\},\{1,9\},\{1,10\},\{2,5\},\{2,11\},\{2,12\},\{3,4\},\{3,13\},\{3,14\},\{4,9\},\{4,11\},\{5,10\},\{5,13\},\{6,12\},\{6,14\},\{7,8\},\{7,9\},\{7,12\},\{7,13\},\{8,10\},\{8,11\},\{8,14\}\}$

Cousin 43 :

$\{\{1,3\},\{1,5\},\{1,7\},\{2,5\},\{2,11\},\{2,12\},\{3,4\},\{3,6\},\{3,8\},\{4,9\},\{4,11\},\{5,10\},\{6,8\},\{6,9\},\{6,10\},\{6,12\},\{7,8\},\{7,9\},\{7,12\},\{8,10\},\{8,11\},\{9,10\}\}$

Cousin 44 :

$\{\{1,6\},\{1,9\},\{1,10\},\{2,3\},\{2,5\},\{2,7\},\{3,4\},\{3,6\},\{3,8\},\{4,9\},\{4,11\},\{5,10\},\{5,11\},\{5,12\},\{6,8\},\{6,12\},\{7,8\},\{7,9\},\{7,12\},\{8,10\},\{8,11\},\{11,12\}\}$

Cousin 45 :

$\{\{1,3\},\{1,7\},\{1,8\},\{2,5\},\{2,11\},\{2,12\},\{3,4\},\{3,5\},\{3,6\},\{4,9\},\{4,11\},\{5,7\},\{5,10\},\{6,8\},\{6,9\},\{6,10\},\{6,12\},\{7,9\},\{7,12\},\{8,10\},\{8,11\},\{9,10\}\}$

Cousin 46 :

$\{\{1,6\},\{1,9\},\{1,10\},\{2,5\},\{2,11\},\{2,12\},\{3,4\},\{3,5\},\{3,6\},\{3,9\},\{3,11\},\{4,7\},\{4,8\},\{5,7\},\{5,10\},\{6,8\},\{6,12\},\{7,9\},\{7,12\},\{8,10\},\{8,11\},\{9,11\}\}$

Cousin 47 :

$\{\{1,2\},\{1,6\},\{1,7\},\{2,5\},\{2,11\},\{3,4\},\{3,5\},\{3,6\},\{3,7\},\{3,8\},\{4,9\},\{4,11\},\{5,7\},\{5,10\},\{6,9\},\{6,12\},\{7,8\},\{7,9\},\{8,11\},\{8,12\},\{9,10\},\{10,12\}\}$

Cousin 48 :

$\{\{1,2\},\{1,5\},\{1,6\},\{1,7\},\{2,4\},\{2,5\},\{2,8\},\{3,4\},\{3,5\},\{3,6\},\{3,7\},\{3,8\},\{4,9\},\{5,7\},\{5,10\},\{6,8\},\{6,9\},\{6,10\},\{7,8\},\{7,9\},\{8,10\},\{9,10\}\}$

Cousin 49 :

$\{\{1,3\},\{1,7\},\{1,8\},\{2,4\},\{2,5\},\{2,8\},\{2,11\},\{3,4\},\{3,5\},\{3,6\},\{4,8\},\{4,9\},\{5,7\},\{5,10\},\{6,9\},\{6,11\},\{6,12\},\{7,9\},\{7,11\},\{8,12\},\{9,10\},\{10,12\}\}$

Cousin 50 :

$\{\{1,2\},\{1,7\},\{1,8\},\{2,4\},\{2,5\},\{2,6\},\{3,4\},\{3,5\},\{3,6\},\{3,7\},\{3,8\},\{4,8\},\{4,9\},\{5,7\},\{5,10\},\{6,11\},\{6,12\},\{7,11\},\{8,12\},\{9,10\},\{9,11\},\{10,12\}\}$

Cousin 51 :

$\{\{1,2\},\{1,7\},\{1,8\},\{2,4\},\{2,5\},\{2,6\},\{3,4\},\{3,5\},\{3,6\},\{3,7\},\{3,8\},\{4,8\},\{4,9\},\{4,10\},\{5,7\},\{5,10\},\{6,8\},\{6,9\},\{6,10\},\{7,9\},\{8,10\},\{9,10\}\}$

Cousin 52 :

$\{\{1,3\},\{1,6\},\{1,8\},\{2,5\},\{2,11\},\{2,12\},\{3,4\},\{3,13\},\{4,9\},\{4,11\},\{5,10\},\{5,13\},\{6,9\},\{6,10\},\{6,12\},\{7,8\},\{7,9\},\{7,12\},\{7,13\},\{8,10\},\{8,11\},\{9,10\}\}$

Cousin 53 :

$\{\{1,3\},\{1,5\},\{1,7\},\{2,5\},\{2,11\},\{2,12\},\{3,4\},\{3,6\},\{3,8\},\{4,9\},\{4,11\},\{5,10\},\{6,9\},\{6,12\},\{6,13\},\{7,8\},\{7,9\},\{7,12\},\{8,11\},\{8,13\},\{9,10\},\{10,13\}\}$

Cousin 54 :

$\{\{1,3\},\{1,5\},\{1,7\},\{2,5\},\{2,6\},\{2,7\},\{2,11\},\{3,4\},\{3,6\},\{3,8\},\{4,9\},\{4,11\},\{5,10\},\{5,11\},\{6,8\},\{6,9\},\{6,10\},\{7,8\},\{7,9\},\{8,10\},\{8,11\},\{9,10\}\}$

Cousin 55 :

$\{\{1,3\},\{1,7\},\{1,8\},\{2,5\},\{2,6\},\{2,7\},\{2,11\},\{3,4\},\{3,5\},\{3,6\},\{4,9\},\{4,11\},\{5,7\},\{5,10\},\{5,11\},\{6,8\},\{6,9\},\{6,10\},\{7,9\},\{8,10\},\{8,11\},\{9,10\}\}$

Cousin 56 :

$\{\{1,2\},\{1,7\},\{1,8\},\{2,4\},\{2,5\},\{2,6\},\{3,4\},\{3,5\},\{3,6\},\{3,7\},\{3,8\},\{4,8\},\{4,10\},\{4,11\},\{5,7\},\{5,10\},\{6,9\},\{6,11\},\{7,11\},\{8,9\},\{9,10\},\{10,11\}\}$

Cousin 57 :

$\{\{1,3\},\{1,6\},\{1,8\},\{2,3\},\{2,5\},\{2,7\},\{3,4\},\{4,9\},\{4,11\},\{5,10\},\{5,11\},\{5,12\},\{6,9\},\{6,10\},\{6,12\},\{7,8\},\{7,9\},\{7,12\},\{8,10\},\{8,11\},\{9,10\},\{11,12\}\}$

Cousin 58 :

$\{\{1,2\},\{1,4\},\{1,6\},\{1,8\},\{2,4\},\{2,5\},\{2,7\},\{3,5\},\{3,6\},\{3,7\},\{3,11\},\{4,9\},\{4,11\},\{5,10\},\{5,11\},\{6,9\},\{6,10\},\{7,8\},\{7,9\},\{8,10\},\{8,11\},\{9,10\}\}$

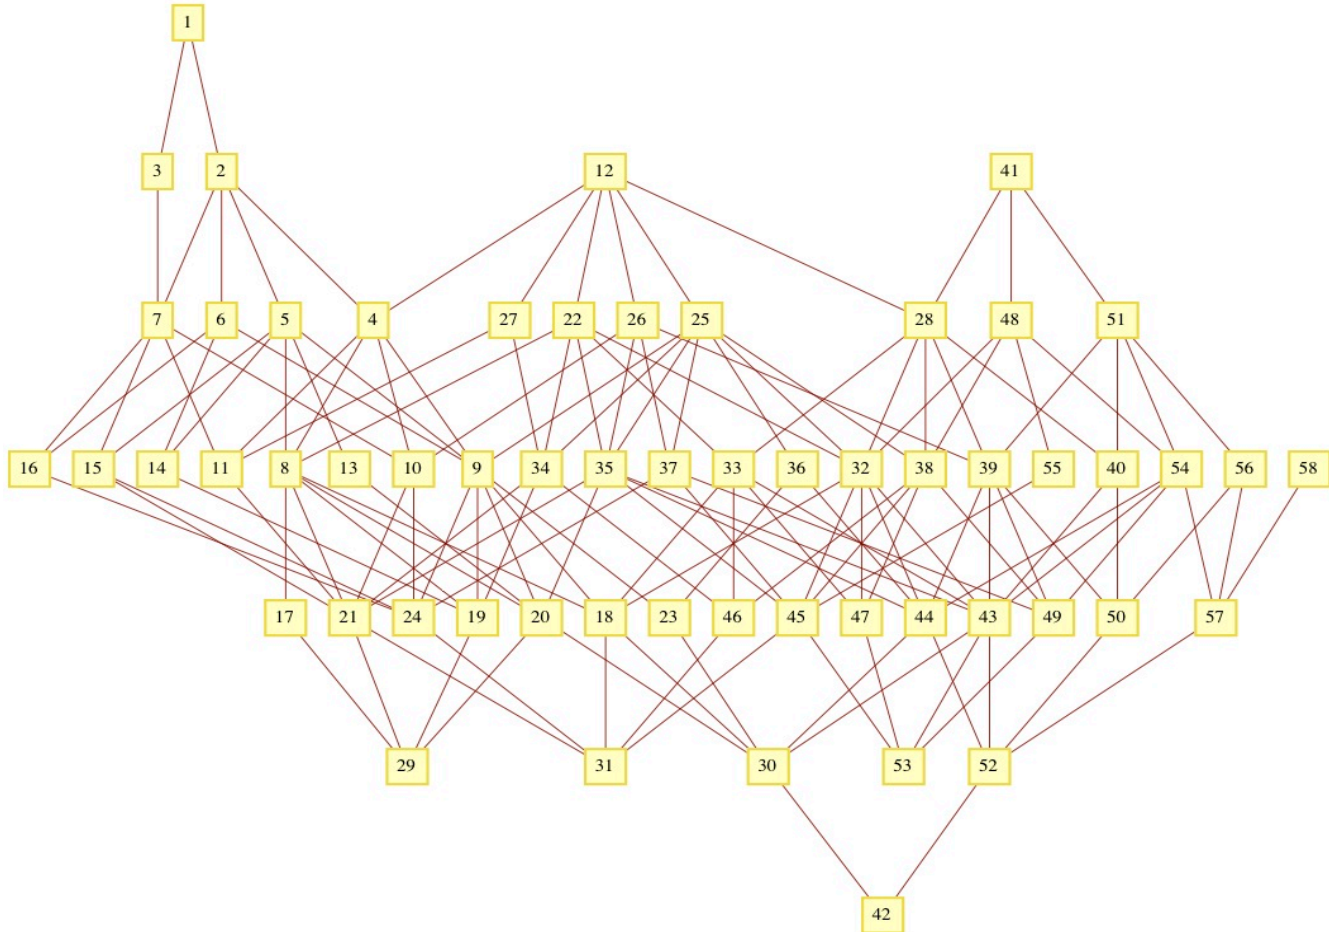

### Section 3:

#### Edge lists for graphs in the E<sub>9</sub> + e family

The E<sub>9</sub>+e family consists of 110 graphs, all of which are IK, but only 33 of them are MMIK.

Minor minimal cousins:

$\{1,3,9,10,11,12,13,14,15,28,31,38,39,40,41,42,43,44,45,46,47,48,49,50,54,64,70,79,83,84,85,86,98\}$

Non-minor minimal cousins:

$\{2,4,5,6,7,8,16,17,18,19,20,21,22,23,24,25,26,27,29,30,32,33,34,35,36,37,51,52,53,55,56,57,58,59,60,61,62,63,65,66,67,68,69,71,72,73,74,75,76,77,78,80,81,82,87,88,89,90,91,92,93,94,95,96,97,99,100,101,102,103,104,105,106,107,108,109,110\}$

E<sub>9</sub>+e is Cousin 1.

Cousin 1:

$\{\{1,3\},\{1,4\},\{1,5\},\{1,6\},\{2,4\},\{2,5\},\{2,6\},\{2,7\},\{2,8\},\{3,6\},\{3,7\},\{3,8\},\{4,7\},\{4,8\},\{5,7\},\{5,8\},\{9,3\},\{9,4\},\{9,5\},\{9,6\},\{9,7\},\{9,8\}\}$

Cousin 2:

$\{\{1,4\},\{1,5\},\{1,10\},\{2,4\},\{2,5\},\{2,6\},\{2,7\},\{2,8\},\{3,7\},\{3,8\},\{3,9\},\{3,10\},\{4,7\},\{4,8\},\{4,9\},\{5,7\},\{5,8\},\{5,9\},\{6,9\},\{6,10\},\{7,9\},\{8,9\}\}$

## Cousin 3:

{{1,3},{1,4},{1,5},{1,6},{2,5},{2,6},{2,8},{2,10},{3,6},{3,7},{3,8},{3,9},{4,8},{4,9},{4,10},{5,7},{5,8},{5,9},{6,9},{7,9},{7,10},{8,9}}

## Cousin 4:

{{1,4},{1,5},{1,10},{2,5},{2,6},{2,8},{2,11},{3,7},{3,8},{3,9},{3,10},{4,8},{4,9},{4,11},{5,7},{5,8},{5,9},{6,9},{6,10},{7,9},{7,11},{8,9}}

## Cousin 5:

{{1,4},{1,5},{1,10},{2,4},{2,5},{2,6},{2,7},{2,8},{3,8},{3,10},{3,11},{4,7},{4,8},{4,9},{5,7},{5,8},{5,9},{6,9},{6,10},{7,11},{8,9},{9,11}}

## Cousin 6:

{{1,4},{1,5},{1,10},{2,4},{2,5},{2,6},{2,7},{2,8},{3,7},{3,8},{3,9},{3,10},{4,8},{4,11},{5,7},{5,8},{5,9},{6,9},{6,10},{7,11},{8,9},{9,11}}

## Cousin 7:

{{1,3},{1,4},{1,5},{1,6},{2,4},{2,5},{2,6},{2,7},{2,8},{3,7},{3,8},{3,9},{4,5},{4,7},{4,8},{4,9},{5,7},{5,8},{5,9},{6,9},{7,9},{8,9}}

## Cousin 8:

{{1,4},{1,5},{1,6},{2,4},{2,5},{2,6},{2,7},{2,8},{2,9},{3,6},{3,7},{3,8},{3,9},{4,7},{4,8},{4,9},{5,7},{5,8},{5,9},{6,9},{7,9},{8,9}}

## Cousin 9:

{{1,3},{1,4},{1,5},{1,6},{2,6},{2,10},{2,11},{3,6},{3,7},{3,8},{3,9},{4,8},{4,9},{4,10},{5,7},{5,9},{5,11},{6,9},{7,9},{7,10},{8,9},{8,11}}

## Cousin 10:

{{1,3},{1,4},{1,5},{1,6},{2,5},{2,6},{2,8},{2,10},{3,7},{3,8},{3,11},{4,8},{4,9},{4,10},{5,7},{5,8},{5,9},{6,11},{7,9},{7,10},{8,9},{9,11}}

## Cousin 11:

{{1,3},{1,4},{1,5},{1,6},{2,5},{2,6},{2,8},{2,10},{3,6},{3,8},{3,11},{4,8},{4,9},{4,10},{5,7},{5,8},{5,9},{6,9},{7,10},{7,11},{8,9},{9,11}}

## Cousin 12:

{{1,3},{1,4},{1,5},{1,6},{2,5},{2,6},{2,8},{2,10},{3,6},{3,7},{3,11},{4,8},{4,9},{4,10},{5,7},{5,8},{5,9},{6,9},{7,9},{7,10},{8,11},{9,11}}

## Cousin 13:

{{1,3},{1,4},{1,5},{1,6},{2,5},{2,6},{2,8},{2,10},{3,6},{3,7},{3,8},{3,9},{4,10},{4,11},{5,7},{5,8},{5,9},{6,9},{7,9},{7,10},{8,11},{9,11}}

## Cousin 14:

{{1,3},{1,4},{1,5},{1,6},{2,5},{2,6},{2,8},{2,10},{3,6},{3,7},{3,8},{3,9},{4,8},{4,9},{4,10},{5,8},{5,11},{6,9},{7,10},{7,11},{8,9},{9,11}}

## Cousin 15:

{{1,3},{1,4},{1,5},{1,6},{2,5},{2,6},{2,8},{2,10},{3,6},{3,7},{3,8},{3,9},{4,8},{4,9},{4,10},{5,7},{5,11},{6,9},{7,9},{7,10},{8,11},{9,11}}

## Cousin 16:

{{1,4},{1,5},{1,10},{2,6},{2,11},{2,12},{3,7},{3,8},{3,9},{3,10},{4,8},{4,9},{4,11},{5,7},{5,9},{5,12},{6,9},{6,10},{7,9},{7,11},{8,9},{8,12}}

## Cousin 17:

{{1,4},{1,5},{1,10},{2,5},{2,6},{2,8},{2,11},{3,8},{3,10},{3,12},{4,8},{4,9},{4,11},{5,7},{5,8},{5,9},{6,9},{6,10},{7,11},{7,12},{8,9},{9,12}}

## Cousin 18:

{{1,4},{1,5},{1,10},{2,5},{2,6},{2,8},{2,11},{3,7},{3,10},{3,12},{4,8},{4,9},{4,11},{5,7},{5,8},{5,9},{6,9},{6,10},{7,9},{7,11},{8,12},{9,12}}

## Cousin 19:

{{1,4},{1,5},{1,10},{2,5},{2,6},{2,8},{2,11},{3,7},{3,8},{3,9},{3,10},{4,11},{4,12},{5,7},{5,8},{5,9},{6,9},{6,10},{7,9},{7,11},{8,12},{9,12}}

## Cousin 20:

{{1,4},{1,5},{1,10},{2,5},{2,6},{2,8},{2,11},{3,7},{3,8},{3,9},{3,10},{4,8},{4,9},{4,11},{5,8},{5,12},{6,9},{6,10},{7,11},{7,12},{8,9},{9,12}}

## Cousin 21:

{{1,4},{1,5},{1,10},{2,5},{2,6},{2,8},{2,11},{3,7},{3,8},{3,9},{3,10},{4,8},{4,9},{4,11},{5,7},{5,12},{6,9},{6,10},{7,9},{7,11},{8,12},{9,12}}

## Cousin 22:

{{1,2},{1,4},{1,7},{2,5},{2,6},{2,8},{3,7},{3,8},{3,9},{3,10},{4,5},{4,8},{4,9},{4,10},{5,7},{5,8},{5,9},{5,10},{6,9},{6,10},{7,9},{8,9}}

## Cousin 23:

{{1,4},{1,5},{1,10},{2,5},{2,6},{2,8},{2,9},{2,10},{3,7},{3,8},{3,9},{3,10},{4,6},{4,8},{4,9},{5,7},{5,8},{5,9},{6,7},{7,9},{8,9},{9,10}}

## Cousin 24:

{{1,4},{1,5},{1,10},{2,4},{2,5},{2,6},{2,7},{2,8},{3,8},{3,10},{3,11},{4,7},{4,12},{5,7},{5,8},{5,9},{6,9},{6,10},{7,11},{8,12},{9,11},{9,12}}

## Cousin 25:

{{1,3},{1,7},{1,9},{2,4},{2,5},{2,6},{2,7},{2,8},{3,8},{3,10},{4,5},{4,7},{4,8},{4,9},{4,10},{5,7},{5,8},{5,9},{5,10},{6,9},{6,10},{8,9}}

## Cousin 26:

{{1,4},{1,5},{1,10},{2,4},{2,5},{2,6},{2,7},{2,8},{3,7},{3,8},{3,9},{3,10},{4,7},{4,8},{4,9},{5,7},{5,8},{5,9},{6,9},{6,10},{8,9},{8,10}}

## Cousin 27:

{{1,4},{1,5},{1,10},{2,4},{2,5},{2,7},{2,8},{2,9},{2,10},{3,6},{3,8},{3,10},{4,7},{4,8},{4,9},{5,7},{5,8},{5,9},{6,7},{6,9},{8,9},{9,10}}

Cousin 28:

{{1,3},{1,4},{1,5},{1,6},{2,4},{2,5},{2,6},{2,7},{2,8},{3,6},{3,8},{3,10},{4,7},{4,8},{4,9},{5,7},{5,8},{5,9},{6,9},{7,10},{8,9},{9,10}}

Cousin 29:

{{1,4},{1,5},{1,10},{2,4},{2,5},{2,6},{2,7},{2,8},{3,7},{3,8},{3,9},{3,10},{4,8},{4,11},{5,7},{5,12},{6,9},{6,10},{7,11},{8,12},{9,11},{9,12}}

Cousin 30:

{{1,4},{1,7},{1,9},{2,4},{2,5},{2,6},{2,7},{2,8},{3,7},{3,8},{3,9},{3,10},{4,5},{4,8},{4,10},{5,7},{5,8},{5,9},{5,10},{6,9},{6,10},{8,9}}

Cousin 31:

{{1,3},{1,4},{1,5},{1,6},{2,4},{2,5},{2,6},{2,7},{2,8},{3,6},{3,7},{3,8},{3,9},{4,8},{4,10},{5,7},{5,8},{5,9},{6,9},{7,10},{8,9},{9,10}}

Cousin 32:

{{1,3},{1,4},{1,5},{1,6},{2,6},{2,7},{2,8},{2,10},{3,7},{3,8},{3,9},{4,7},{4,8},{4,9},{4,10},{5,7},{5,8},{5,9},{5,10},{6,9},{7,9},{8,9}}

Cousin 33:

{{1,3},{1,4},{1,5},{1,6},{2,4},{2,5},{2,6},{2,7},{2,8},{3,7},{3,8},{3,9},{4,8},{4,9},{4,10},{5,8},{5,9},{5,10},{6,9},{7,9},{7,10},{8,9}}

Cousin 34:

{{1,3},{1,4},{1,5},{1,6},{2,4},{2,5},{2,6},{2,7},{2,8},{3,7},{3,8},{3,9},{4,7},{4,8},{4,10},{5,7},{5,8},{5,10},{6,9},{7,9},{8,9},{9,10}}

Cousin 35:

{{1,2},{1,3},{1,4},{1,5},{1,6},{2,4},{2,5},{2,6},{2,7},{2,8},{3,6},{3,7},{3,8},{4,5},{4,6},{4,7},{4,8},{5,6},{5,7},{5,8},{6,7},{6,8}}

Cousin 36:

{{1,4},{1,5},{1,6},{2,5},{2,6},{2,7},{2,8},{2,10},{3,6},{3,7},{3,8},{3,9},{4,7},{4,8},{4,10},{5,7},{5,8},{5,9},{6,9},{7,9},{8,9},{9,10}}

Cousin 37:

{{1,4},{1,5},{1,6},{2,4},{2,5},{2,6},{2,7},{2,8},{2,9},{3,7},{3,8},{3,10},{4,7},{4,8},{4,9},{5,7},{5,8},{5,9},{6,10},{7,9},{8,9},{9,10}}

Cousin 38:

{{1,3},{1,4},{1,5},{1,6},{2,6},{2,10},{2,11},{3,7},{3,8},{3,12},{4,8},{4,9},{4,10},{5,7},{5,9},{5,11},{6,12},{7,9},{7,10},{8,9},{8,11},{9,12}}

Cousin 39:

{{1,3},{1,4},{1,5},{1,6},{2,6},{2,10},{2,11},{3,6},{3,8},{3,12},{4,8},{4,9},{4,10},{5,7},{5,9},{5,11},{6,9},{7,10},{7,12},{8,9},{8,11},{9,12}}

Cousin 40:

{{1,3},{1,4},{1,5},{1,6},{2,6},{2,10},{2,11},{3,6},{3,7},{3,8},{3,9},{4,10},{4,12},{5,7},{5,9},{5,11},{6,9},{7,9},{7,10},{8,11},{8,12},{9,12}}

Cousin 41:

{{1,3},{1,4},{1,5},{1,6},{2,5},{2,6},{2,8},{2,10},{3,6},{3,7},{3,8},{3,9},{4,8},{4,9},{4,10},{5,7},{5,9},{6,9},{6,10},{7,9},{7,10},{8,9}}

Cousin 42:

{{1,3},{1,4},{1,5},{1,6},{2,5},{2,6},{2,8},{2,10},{3,7},{3,8},{3,11},{4,10},{4,12},{5,7},{5,8},{5,9},{6,11},{7,9},{7,10},{8,12},{9,11},{9,12}}

Cousin 43:

{{1,3},{1,4},{1,5},{1,6},{2,5},{2,6},{2,8},{2,10},{3,7},{3,8},{3,11},{4,8},{4,9},{4,10},{5,7},{5,12},{6,11},{7,9},{7,10},{8,12},{9,11},{9,12}}

Cousin 44:

{{1,3},{1,4},{1,5},{1,6},{2,4},{2,5},{2,6},{2,7},{2,8},{3,7},{3,8},{3,10},{4,7},{4,8},{4,9},{5,7},{5,8},{5,9},{6,10},{7,9},{8,9},{9,10}}

Cousin 45:

{{1,3},{1,4},{1,5},{1,6},{2,5},{2,6},{2,8},{2,10},{3,6},{3,8},{3,11},{4,10},{4,12},{5,7},{5,8},{5,9},{6,9},{7,10},{7,11},{8,12},{9,11},{9,12}}

Cousin 46:

{{1,3},{1,4},{1,5},{1,6},{2,5},{2,6},{2,8},{2,10},{3,6},{3,8},{3,11},{4,8},{4,9},{4,10},{5,7},{5,12},{6,9},{7,10},{7,11},{8,12},{9,11},{9,12}}

Cousin 47:

{{1,3},{1,4},{1,5},{1,6},{2,5},{2,6},{2,8},{2,10},{3,6},{3,7},{3,8},{4,8},{4,9},{4,10},{5,7},{5,8},{5,9},{5,10},{6,9},{7,9},{7,10},{8,9}}

Cousin 48:

{{1,3},{1,4},{1,5},{1,6},{2,5},{2,6},{2,8},{2,10},{3,6},{3,7},{3,11},{4,8},{4,9},{4,10},{5,8},{5,12},{6,9},{7,10},{7,12},{8,11},{9,11},{9,12}}

Cousin 49:

{{1,3},{1,4},{1,5},{1,6},{2,5},{2,6},{2,8},{2,10},{3,6},{3,7},{3,8},{3,9},{4,10},{4,11},{5,8},{5,12},{6,9},{7,10},{7,12},{8,11},{9,11},{9,12}}

Cousin 50:

{{1,3},{1,4},{1,5},{1,6},{1,10},{2,5},{2,6},{2,8},{2,10},{3,6},{3,7},{3,8},{3,9},{4,8},{4,9},{4,10},{5,7},{5,8},{5,9},{6,9},{7,9},{7,10}}

Cousin 51:

{{1,4},{1,5},{1,10},{2,6},{2,11},{2,12},{3,8},{3,10},{3,13},{4,8},{4,9},{4,11},{5,7},{5,9},{5,12},{6,9},{6,10},{7,11},{7,13},{8,9},{8,12},{9,13}}

Cousin 52:

{{1,4},{1,5},{1,10},{2,6},{2,11},{2,12},{3,7},{3,8},{3,9},{3,10},{4,11},{4,13},{5,7},{5,9},{5,12},{6,9},{6,10},{7,9},{7,11},{8,12},{8,13},{9,13}}

Cousin 53:

{{1,2},{1,5},{1,8},{2,6},{2,11},{3,7},{3,8},{3,9},{3,10},{4,5},{4,8},{4,9},{4,10},{4,11},{5,7},{5,9},{5,10},{6,9},{6,10},{7,9},{7,11},{8,9}}

Cousin 54:

{{1,4},{1,5},{1,10},{2,5},{2,6},{2,8},{2,11},{3,7},{3,8},{3,9},{3,10},{4,8},{4,9},{4,11},{5,7},{5,9},{6,9},{6,10},{6,11},{7,9},{7,11},{8,9}}

Cousin 55:

{{1,4},{1,5},{1,10},{2,6},{2,9},{2,10},{2,11},{3,7},{3,8},{3,9},{3,10},{4,8},{4,9},{4,11},{5,6},{5,7},{5,9},{6,8},{7,9},{7,11},{8,9},{9,10}}

Cousin 56:

{{1,4},{1,5},{1,10},{2,5},{2,6},{2,8},{2,11},{3,8},{3,10},{3,12},{4,8},{4,9},{4,11},{5,7},{5,13},{6,9},{6,10},{7,11},{7,12},{8,13},{9,12},{9,13}}

Cousin 57:

{{1,3},{1,7},{1,9},{2,5},{2,6},{2,8},{2,11},{3,8},{3,10},{4,5},{4,8},{4,9},{4,10},{4,11},{5,7},{5,8},{5,9},{5,10},{6,9},{6,10},{7,11},{8,9}}

Cousin 58:

{{1,4},{1,5},{1,10},{2,5},{2,6},{2,8},{2,11},{3,7},{3,8},{3,9},{3,10},{4,8},{4,9},{4,11},{5,7},{5,8},{5,9},{6,9},{6,10},{7,11},{8,9},{8,10}}

Cousin 59:

{{1,4},{1,5},{1,10},{2,5},{2,6},{2,8},{2,11},{3,7},{3,10},{3,12},{4,8},{4,9},{4,11},{5,8},{5,13},{6,9},{6,10},{7,11},{7,13},{8,12},{9,12},{9,13}}

Cousin 60:

{{1,4},{1,5},{1,10},{2,5},{2,6},{2,8},{2,11},{3,7},{3,8},{3,9},{3,10},{4,8},{4,9},{4,11},{5,7},{5,8},{5,9},{6,9},{6,10},{7,9},{7,10},{7,11}}

Cousin 61:

{{1,4},{1,5},{1,10},{2,5},{2,8},{2,9},{2,10},{2,11},{3,6},{3,7},{3,10},{4,8},{4,9},{4,11},{5,7},{5,8},{5,9},{6,8},{6,9},{7,9},{7,11},{9,10}}

Cousin 62:

{{1,4},{1,5},{1,10},{2,5},{2,6},{2,8},{2,11},{3,7},{3,8},{3,9},{3,10},{4,11},{4,12},{5,8},{5,13},{6,9},{6,10},{7,11},{7,13},{8,12},{9,12},{9,13}}

Cousin 63:

{{1,4},{1,8},{1,9},{2,5},{2,6},{2,8},{2,11},{3,7},{3,8},{3,9},{3,10},{4,5},{4,10},{4,11},{5,7},{5,8},{5,9},{5,10},{6,9},{6,10},{7,9},{7,11}}

Cousin 64:

{{1,4},{1,5},{1,10},{1,11},{2,5},{2,6},{2,8},{2,11},{3,7},{3,8},{3,9},{3,10},{4,8},{4,9},{4,11},{5,7},{5,8},{5,9},{6,9},{6,10},{7,9},{7,11}}

Cousin 65:

{{1,5},{1,8},{1,9},{2,5},{2,6},{2,8},{2,11},{3,7},{3,8},{3,9},{3,10},{4,5},{4,8},{4,9},{4,10},{4,11},{5,7},{5,10},{6,9},{6,10},{7,9},{7,11}}

Cousin 66:

{{1,4},{1,5},{1,10},{2,5},{2,8},{2,9},{2,10},{2,11},{3,7},{3,8},{3,9},{3,10},{4,8},{4,9},{4,11},{5,6},{5,7},{6,8},{6,9},{7,9},{7,11},{9,10}}

Cousin 67:

{{1,2},{1,4},{1,7},{2,5},{2,6},{2,8},{3,7},{3,8},{3,9},{3,10},{4,8},{4,10},{4,11},{5,7},{5,8},{5,10},{5,11},{6,9},{6,10},{7,9},{8,9},{9,11}}

Cousin 68:

{{1,4},{1,5},{1,10},{2,6},{2,8},{2,10},{2,11},{3,7},{3,8},{3,9},{3,10},{4,6},{4,8},{4,9},{5,7},{5,8},{5,11},{6,7},{7,9},{8,9},{9,10},{9,11}}

Cousin 69:

{{1,4},{1,8},{1,9},{2,4},{2,5},{2,6},{2,7},{2,8},{3,8},{3,10},{3,11},{4,5},{4,7},{4,10},{5,7},{5,8},{5,9},{5,10},{6,9},{6,10},{7,11},{9,11}}

Cousin 70:

{{1,3},{1,4},{1,5},{1,6},{2,4},{2,5},{2,6},{2,7},{2,8},{3,6},{3,8},{3,11},{4,7},{4,10},{5,7},{5,8},{5,9},{6,9},{7,11},{8,10},{9,10},{9,11}}

Cousin 71:

{{1,3},{1,7},{1,9},{2,6},{2,7},{2,8},{2,11},{3,8},{3,10},{4,7},{4,8},{4,9},{4,10},{4,11},{5,7},{5,8},{5,9},{5,10},{5,11},{6,9},{6,10},{8,9}}

Cousin 72:

{{1,3},{1,7},{1,9},{2,4},{2,5},{2,6},{2,7},{2,8},{3,8},{3,10},{4,8},{4,9},{4,10},{4,11},{5,8},{5,9},{5,10},{5,11},{6,9},{6,10},{7,11},{8,9}}

Cousin 73:

{{1,3},{1,7},{1,9},{2,4},{2,5},{2,6},{2,7},{2,8},{3,8},{3,10},{4,7},{4,9},{4,10},{4,11},{5,7},{5,9},{5,10},{5,11},{6,9},{6,10},{8,9},{8,11}}

Cousin 74:

{{1,3},{1,7},{1,9},{2,4},{2,5},{2,6},{2,7},{2,8},{3,8},{3,10},{4,7},{4,8},{4,10},{4,11},{5,7},{5,8},{5,10},{5,11},{6,9},{6,10},{8,9},{9,11}}

Cousin 75:

{{1,3},{1,7},{1,8},{1,9},{2,4},{2,5},{2,6},{2,7},{2,8},{3,4},{3,5},{3,6},{3,8},{4,5},{4,7},{4,8},{4,9},{5,7},{5,8},{5,9},{6,9},{8,9}}

Cousin 76:

{{1,3},{1,7},{1,9},{2,4},{2,5},{2,6},{2,7},{2,8},{2,9},{3,6},{3,8},{4,5},{4,6},{4,7},{4,8},{4,9},{5,6},{5,7},{5,8},{5,9},{6,9},{8,9}}

Cousin 77:

{{1,4},{1,5},{1,10},{2,5},{2,7},{2,8},{2,10},{2,11},{3,6},{3,8},{3,10},{4,7},{4,8},{4,11},{5,7},{5,8},{5,9},{6,7},{6,9},{8,9},{9,10},{9,11}}

Cousin 78:

{{1,5},{1,8},{1,9},{2,4},{2,5},{2,6},{2,7},{2,8},{3,7},{3,8},{3,9},{3,10},{4,5},{4,8},{4,10},{4,11},{5,7},{5,10},{6,9},{6,10},{7,11},{9,11}}



Cousin 79:

{{1,3},{1,4},{1,5},{1,6},{2,4},{2,5},{2,6},{2,7},{2,8},{3,6},{3,7},{3,8},{3,9},{4,8},{4,11},{5,7},{5,10},{6,9},{7,11},{8,10},{9,10},{9,11}}

Cousin 80:

{{1,4},{1,7},{1,9},{2,6},{2,7},{2,8},{2,11},{3,7},{3,8},{3,9},{3,10},{4,8},{4,10},{4,11},{5,7},{5,8},{5,9},{5,10},{5,11},{6,9},{6,10},{8,9}}

Cousin 81:

{{1,2},{1,3},{1,4},{1,5},{1,9},{2,6},{2,7},{2,8},{2,9},{3,7},{3,8},{3,9},{4,6},{4,7},{4,8},{4,9},{5,6},{5,7},{5,8},{5,9},{7,9},{8,9}}

Cousin 82:

{{1,2},{1,3},{1,4},{1,5},{1,9},{2,4},{2,5},{2,7},{2,8},{2,9},{3,7},{3,8},{3,9},{4,6},{4,7},{4,8},{5,6},{5,7},{5,8},{6,9},{7,9},{8,9}}

Cousin 83:

{{1,3},{1,4},{1,5},{1,6},{2,6},{2,10},{2,11},{3,7},{3,8},{3,12},{4,10},{4,13},{5,7},{5,9},{5,11},{6,12},{7,9},{7,10},{8,11},{8,13},{9,12},{9,13}}

Cousin 84:

{{1,3},{1,4},{1,5},{1,6},{2,3},{2,6},{2,9},{3,7},{3,8},{4,8},{4,9},{4,10},{5,7},{5,9},{5,11},{6,10},{6,11},{7,9},{7,10},{8,9},{8,11},{10,11}}

Cousin 85:

{{1,3},{1,4},{1,5},{1,6},{2,3},{2,7},{2,9},{3,6},{3,8},{4,8},{4,9},{4,10},{5,7},{5,9},{5,11},{6,9},{6,10},{6,11},{7,10},{8,9},{8,11},{10,11}}

Cousin 86:

{{1,3},{1,4},{1,5},{1,6},{2,5},{2,6},{2,8},{2,10},{3,6},{3,8},{3,11},{4,8},{4,9},{4,10},{5,7},{5,10},{5,11},{6,9},{7,8},{7,9},{9,11},{10,11}}

Cousin 87:

{{1,4},{1,5},{1,10},{2,6},{2,11},{2,12},{3,8},{3,10},{3,13},{4,11},{4,14},{5,7},{5,9},{5,12},{6,9},{6,10},{7,11},{7,13},{8,12},{8,14},{9,13},{9,14}}

Cousin 88:

{{1,4},{1,5},{1,10},{2,9},{2,10},{2,11},{2,12},{3,6},{3,8},{3,10},{4,8},{4,9},{4,11},{5,7},{5,9},{5,12},{6,7},{6,9},{7,11},{8,9},{8,12},{9,10}}

Cousin 89:

{{1,4},{1,5},{1,10},{2,6},{2,11},{2,12},{3,7},{3,8},{3,9},{3,10},{4,11},{4,13},{5,12},{5,14},{6,9},{6,10},{7,11},{7,14},{8,12},{8,13},{9,13},{9,14}}

Cousin 90:

{{1,2},{1,5},{1,8},{2,6},{2,11},{3,7},{3,8},{3,9},{3,10},{4,8},{4,10},{4,11},{4,12},{5,7},{5,10},{5,12},{6,9},{6,10},{7,9},{7,11},{8,9},{9,12}}

Cousin 91:

{{1,5},{1,8},{1,9},{2,5},{2,6},{2,8},{2,11},{3,8},{3,10},{3,12},{4,5},{4,8},{4,9},{4,10},{4,11},{5,7},{5,10},{6,9},{6,10},{7,11},{7,12},{9,12}}

Cousin 92:

{{1,4},{1,5},{1,10},{2,5},{2,6},{2,8},{2,11},{3,5},{3,8},{3,9},{4,8},{4,9},{4,11},{5,7},{6,9},{6,10},{7,11},{7,12},{8,10},{8,12},{9,12},{10,12}}

Cousin 93:

{{1,4},{1,5},{1,10},{2,5},{2,8},{2,9},{2,10},{2,11},{3,8},{3,10},{3,12},{4,8},{4,9},{4,11},{5,6},{5,7},{6,8},{6,9},{7,11},{7,12},{9,10},{9,12}}

Cousin 94:

{{1,3},{1,7},{1,9},{2,5},{2,6},{2,8},{2,11},{3,8},{3,10},{4,9},{4,10},{4,11},{4,12},{5,7},{5,9},{5,10},{5,12},{6,9},{6,10},{7,11},{8,9},{8,12}}

Cousin 95:

{{1,4},{1,5},{1,10},{2,5},{2,6},{2,8},{2,11},{3,5},{3,7},{3,9},{4,8},{4,9},{4,11},{5,8},{6,9},{6,10},{7,10},{7,11},{7,12},{8,12},{9,12},{10,12}}

Cousin 96:

{{1,4},{1,5},{1,10},{2,5},{2,6},{2,8},{2,9},{2,10},{3,7},{3,8},{3,9},{3,10},{4,6},{4,8},{4,9},{5,7},{5,8},{5,9},{6,7},{7,9},{7,10},{9,10}}

Cousin 97:

{{1,4},{1,5},{1,10},{2,8},{2,10},{2,11},{2,12},{3,6},{3,7},{3,10},{4,8},{4,9},{4,11},{5,7},{5,8},{5,12},{6,8},{6,9},{7,9},{7,11},{9,10},{9,12}}

Cousin 98:

{{1,5},{1,10},{1,11},{1,12},{2,5},{2,6},{2,8},{2,11},{3,7},{3,8},{3,9},{3,10},{4,5},{4,7},{4,9},{5,8},{6,9},{6,10},{7,11},{8,12},{9,12},{11,12}}

Cousin 99:

{{1,4},{1,8},{1,9},{2,6},{2,7},{2,8},{2,12},{3,8},{3,10},{3,11},{4,7},{4,10},{4,12},{5,7},{5,8},{5,9},{5,10},{5,12},{6,9},{6,10},{7,11},{9,11}}

Cousin 100:

{{1,7},{1,8},{1,9},{1,10},{2,3},{2,6},{2,7},{2,8},{3,4},{3,5},{4,7},{4,8},{4,9},{4,10},{5,7},{5,8},{5,9},{5,10},{6,9},{6,10},{8,9},{8,10}}

Cousin 101:

{{1,3},{1,7},{1,9},{2,6},{2,7},{2,8},{2,9},{2,10},{3,8},{3,10},{4,6},{4,7},{4,8},{4,9},{4,10},{5,6},{5,7},{5,8},{5,9},{5,10},{8,9},{9,10}}

Cousin 102:

{{1,7},{1,8},{1,9},{1,10},{2,4},{2,5},{2,6},{2,7},{2,8},{3,4},{3,5},{3,7},{4,8},{4,9},{4,10},{5,8},{5,9},{5,10},{6,9},{6,10},{8,9},{8,10}}

Cousin 103:

{{1,7},{1,8},{1,9},{1,10},{2,4},{2,5},{2,6},{2,7},{2,8},{3,4},{3,5},{3,8},{4,7},{4,9},{4,10},{5,7},{5,9},{5,10},{6,9},{6,10},{8,9},{8,10}}

Cousin 104:

{{1,3},{1,6},{1,7},{1,8},{2,3},{2,4},{2,5},{2,6},{2,7},{2,8},{3,4},{3,5},{3,6},{3,8},{4,5},{4,6},{4,7},{4,8},{5,6},{5,7},{5,8},{6,8}}

Cousin 105:

{{1,5},{1,8},{1,9},{2,6},{2,7},{2,8},{2,12},{3,7},{3,8},{3,9},{3,10},{4,8},{4,10},{4,11},{4,12},{5,7},{5,10},{5,12},{6,9},{6,10},{7,11},{9,11}}

Cousin 106:

{{1,4},{1,5},{1,10},{2,6},{2,8},{2,10},{2,11},{3,7},{3,8},{3,9},{3,10},{4,6},{4,8},{4,9},{5,7},{5,8},{5,11},{6,7},{7,9},{7,10},{9,10},{9,11}}

Cousin 107:

{{1,4},{1,5},{1,10},{2,5},{2,6},{2,8},{2,9},{2,10},{3,7},{3,8},{3,9},{3,10},{4,6},{4,8},{4,9},{5,7},{5,8},{5,9},{6,7},{7,11},{9,11},{10,11}}

Cousin 108:

{{1,6},{1,7},{1,8},{1,9},{2,3},{2,6},{2,7},{2,8},{2,9},{3,4},{3,5},{4,6},{4,7},{4,8},{4,9},{5,6},{5,7},{5,8},{5,9},{6,8},{6,9},{8,9}}

Cousin 109:

{{1,4},{1,5},{1,10},{2,6},{2,8},{2,10},{2,11},{3,7},{3,8},{3,9},{3,10},{4,6},{4,8},{4,9},{5,7},{5,8},{5,11},{6,7},{7,12},{9,11},{9,12},{10,12}}

Cousin 110:

{{1,6},{1,7},{1,8},{1,9},{2,3},{2,6},{2,7},{2,8},{2,9},{3,4},{3,5},{4,6},{4,7},{4,8},{4,9},{5,6},{5,7},{5,8},{5,9},{6,10},{8,10},{9,10}}

Diagram of the entire family:

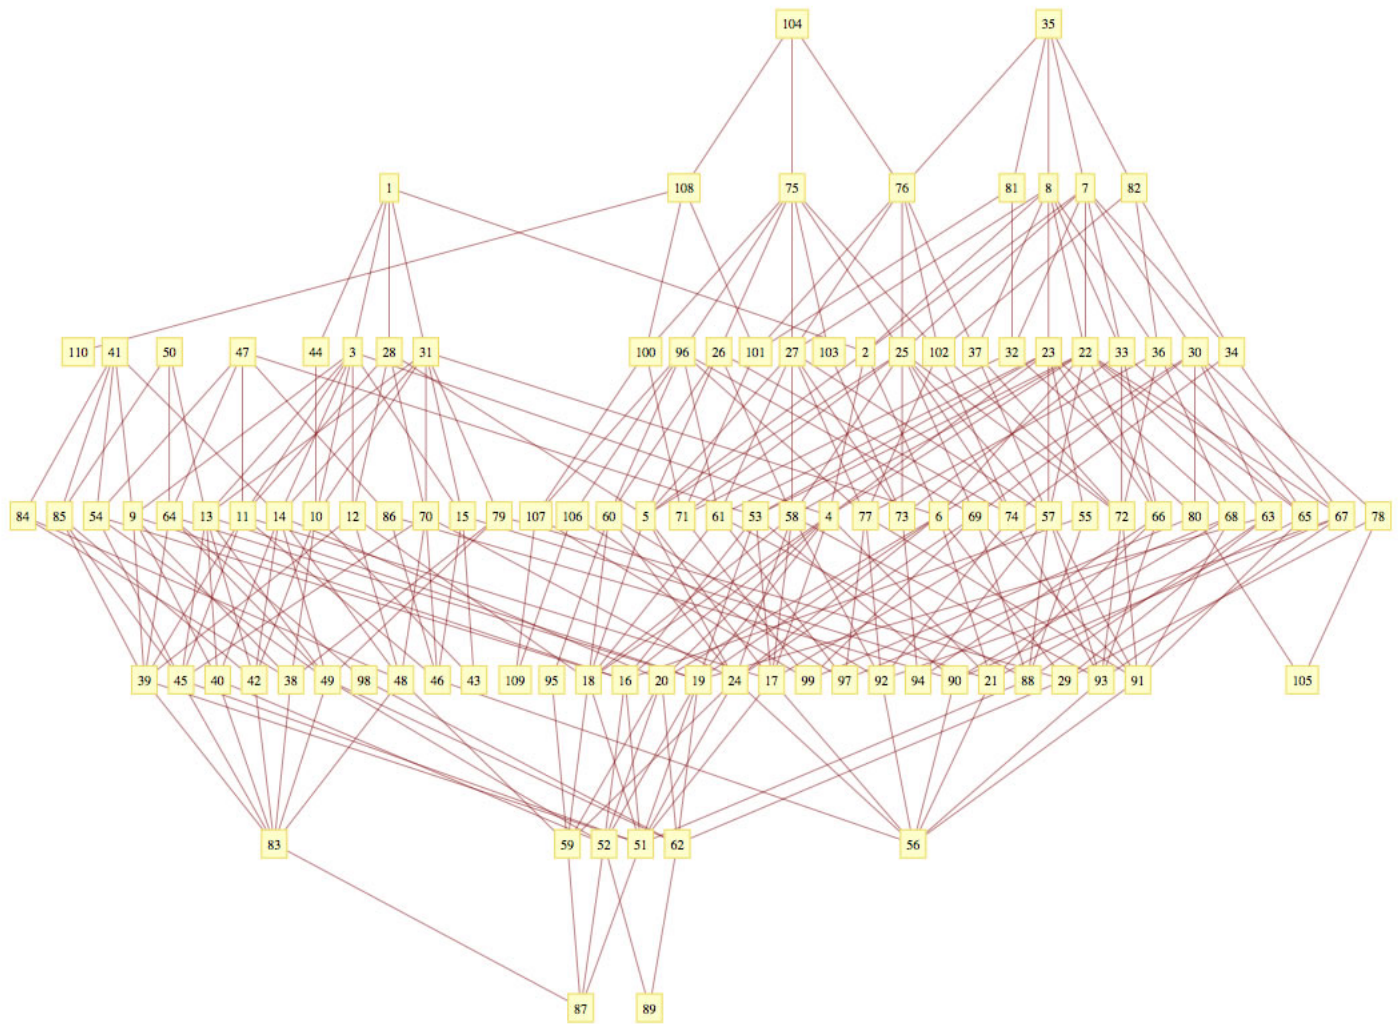

Diagram of minor minimal cousins only:

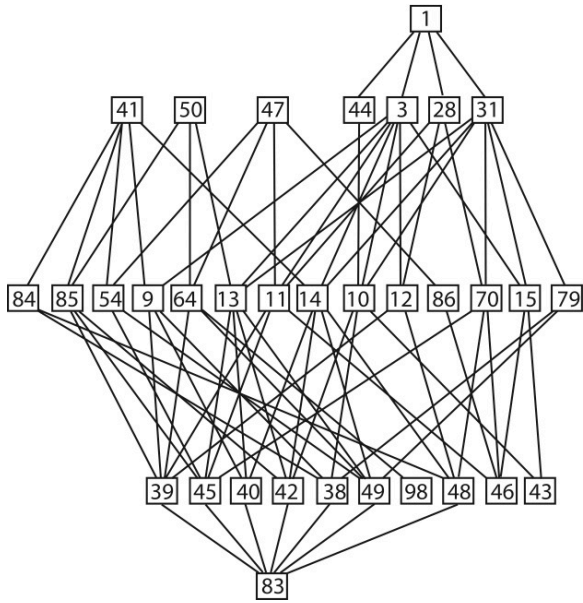

Another diagram of the minor minimal cousins (disregard the graphs below Cousin 83):

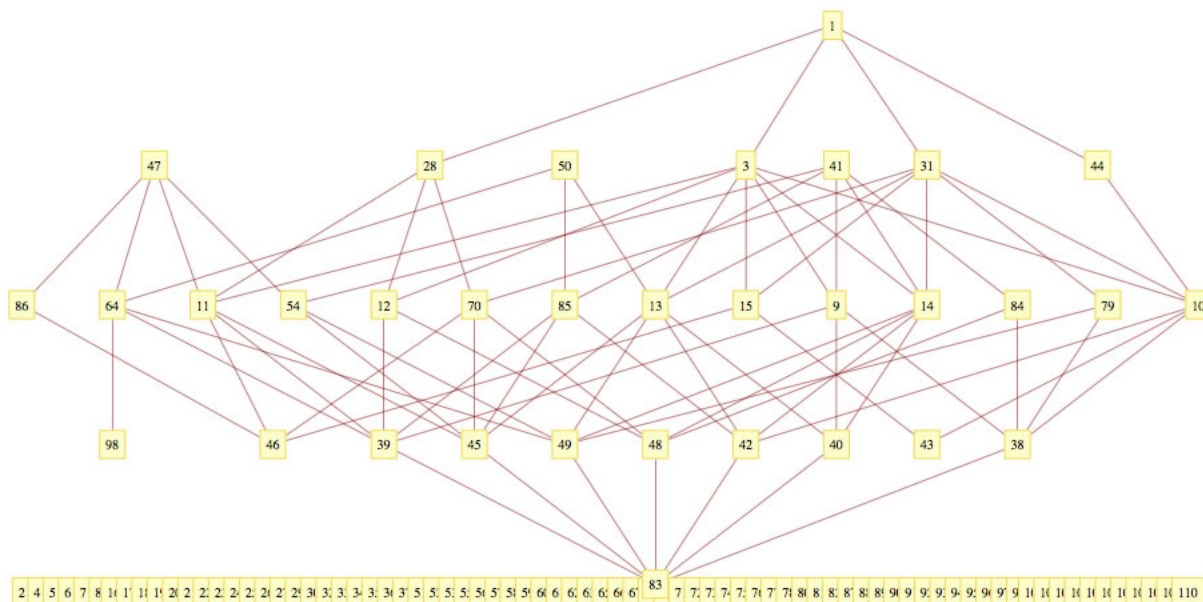

## Section 4:

### Edge lists for graphs in the $G_{\{9,28\}}$ family

The  $G_{9,28}$  family consists of 1609 graphs, all of which are IK; at least 156 are MMIK, and at least 4 are not MMIK (there is reason to believe that well over half of them are MMIK). Below, we provide edge lists for all 1609 graphs. Since this family is too large to give a family diagram for it here, we instead give a list of all children for each cousin in Section 4.1, below.

Cousin 1151 and its ancestors consist of 156 graphs, all of which are MMIK:

{1, 2, 3, 4, 5, 6, 7, 8, 9, 10, 12, 14, 18, 19, 24, 25, 29, 30, 31, 32, 34, 35, 36, 47, 50, 53, 60, 61, 62, 64, 65, 68, 69, 71, 72, 74, 75, 85, 102, 104, 121, 129, 136, 137, 138, 140, 142, 143, 144, 145, 146, 149, 151, 158, 159, 163, 172, 174, 177, 184, 186, 246, 255, 256, 292, 294, 298, 300, 302, 303, 305, 311, 316, 324, 388, 430, 431, 435, 436, 437, 438, 445, 447, 455, 459, 460, 462, 463, 464, 480, 481, 487, 489, 492, 547, 549, 553, 576, 580, 684, 728, 730, 732, 736, 742, 827, 830, 831, 832, 835, 836, 837, 849, 853, 861, 863, 864,

865, 866, 870, 880, 906, 908, 912, 913, 1022, 1045, 1115, 1117, 1151, 1152, 1153, 1157, 1158, 1159, 1162, 1177, 1178, 1185, 1186, 1194, 1242, 1243, 1248, 1374, 1375, 1376, 1377, 1381, 1391, 1393, 1451, 1500, 1501, 1502, 1567}

G<sub>9,28</sub> is Cousin 1.

Cousin 1: {{1,3},{1,4},{1,5},{1,6},{1,8},{1,9},{2,4},{2,5},{2,6},{2,7},{2,8},{2,9},{3,5},{3,6},{3,7},{3,8},{3,9},{4,6},{4,7},{4,8},{4,9},{5,7},{5,8},{5,9},{6,8},{6,9},{7,8},{7,9}}

Cousin 2: {{1,4},{1,6},{1,8},{1,9},{1,10},{2,4},{2,5},{2,6},{2,7},{2,8},{2,9},{3,6},{3,7},{3,8},{3,9},{3,10},{4,6},{4,7},{4,8},{4,9},{5,7},{5,8},{5,9},{5,10},{6,8},{6,9},{7,8},{7,9}}

Cousin 3: {{1,4},{1,5},{1,6},{1,9},{1,10},{2,4},{2,5},{2,6},{2,7},{2,8},{2,9},{3,5},{3,6},{3,7},{3,9},{3,10},{4,6},{4,7},{4,8},{4,9},{5,7},{5,8},{5,9},{6,8},{6,9},{7,8},{7,9},{8,10}}

Cousin 4: {{1,3},{1,5},{1,6},{1,9},{1,10},{2,4},{2,5},{2,6},{2,7},{2,8},{2,9},{3,5},{3,6},{3,7},{3,8},{3,9},{4,6},{4,7},{4,9},{4,10},{5,7},{5,8},{5,9},{6,8},{6,9},{7,8},{7,9},{8,10}}

Cousin 5: {{1,8},{1,9},{1,10},{1,11},{2,4},{2,5},{2,6},{2,7},{2,8},{2,9},{3,6},{3,7},{3,8},{3,9},{3,10},{4,7},{4,8},{4,9},{4,11},{5,7},{5,8},{5,9},{5,10},{6,8},{6,9},{6,11},{7,8},{7,9}}

Cousin 6: {{1,6},{1,9},{1,10},{1,11},{2,4},{2,5},{2,6},{2,7},{2,8},{2,9},{3,6},{3,7},{3,8},{3,9},{3,10},{4,6},{4,7},{4,9},{4,11},{5,7},{5,8},{5,9},{5,10},{6,8},{6,9},{7,8},{7,9},{8,11}}

Cousin 7: {{1,4},{1,9},{1,10},{1,11},{2,4},{2,5},{2,6},{2,7},{2,8},{2,9},{3,6},{3,7},{3,8},{3,9},{3,10},{4,6},{4,7},{4,8},{4,9},{5,7},{5,8},{5,9},{5,10},{6,9},{6,11},{7,8},{7,9},{8,11}}

Cousin 8: {{1,4},{1,6},{1,8},{1,9},{1,10},{2,5},{2,7},{2,8},{2,9},{2,11},{3,6},{3,7},{3,8},{3,9},{3,10},{4,7},{4,8},{4,9},{4,11},{5,7},{5,8},{5,9},{5,10},{6,8},{6,9},{6,11},{7,8},{7,9}}

Cousin 9: {{1,4},{1,6},{1,8},{1,9},{1,10},{2,5},{2,6},{2,7},{2,9},{2,11},{3,6},{3,7},{3,8},{3,9},{3,10},{4,6},{4,7},{4,9},{4,11},{5,7},{5,8},{5,9},{5,10},{6,8},{6,9},{7,8},{7,9},{8,11}}

Cousin 10: {{1,4},{1,6},{1,8},{1,9},{1,10},{2,4},{2,5},{2,7},{2,9},{2,11},{3,6},{3,7},{3,8},{3,9},{3,10},{4,6},{4,7},{4,8},{4,9},{5,7},{5,8},{5,9},{5,10},{6,9},{6,11},{7,8},{7,9},{8,11}}

Cousin 11: {{1,4},{1,6},{1,8},{1,9},{1,10},{2,4},{2,5},{2,6},{2,9},{2,11},{3,6},{3,7},{3,8},{3,9},{3,10},{4,6},{4,7},{4,8},{4,9},{5,7},{5,8},{5,9},{5,10},{6,8},{6,9},{7,9},{7,11},{8,11}}

Cousin 12: {{1,4},{1,6},{1,8},{1,9},{1,10},{2,4},{2,5},{2,6},{2,7},{2,8},{2,9},{3,7},{3,9},{3,10},{3,11},{4,6},{4,7},{4,8},{4,9},{5,7},{5,8},{5,9},{5,10},{6,9},{6,11},{7,8},{7,9},{8,11}}

Cousin 13: {{1,5},{1,6},{1,10},{1,11},{2,4},{2,5},{2,6},{2,7},{2,8},{2,9},{3,5},{3,6},{3,7},{3,9},{3,10},{4,6},{4,7},{4,8},{4,11},{5,7},{5,8},{5,9},{6,8},{6,9},{7,8},{7,9},{8,10},{9,11}}

Cousin 14: {{1,4},{1,6},{1,10},{1,11},{2,4},{2,5},{2,6},{2,7},{2,8},{2,9},{3,5},{3,6},{3,7},{3,9},{3,10},{4,6},{4,7},{4,8},{4,9},{5,7},{5,8},{5,11},{6,8},{6,9},{7,8},{7,9},{8,10},{9,11}}

Cousin 15: {{1,4},{1,5},{1,10},{1,11},{2,4},{2,5},{2,6},{2,7},{2,8},{2,9},{3,5},{3,6},{3,7},{3,9},{3,10},{4,6},{4,7},{4,8},{4,9},{5,7},{5,8},{5,9},{6,8},{6,11},{7,8},{7,9},{8,10},{9,11}}

Cousin 16: {{1,4},{1,5},{1,6},{1,9},{1,10},{2,5},{2,6},{2,7},{2,9},{2,11},{3,5},{3,6},{3,7},{3,9},{3,10},{4,6},{4,7},{4,9},{4,11},{5,7},{5,8},{5,9},{6,8},{6,9},{7,8},{7,9},{8,10},{8,11}}

Cousin 17: {{1,4},{1,5},{1,6},{1,9},{1,10},{2,5},{2,6},{2,7},{2,8},{2,11},{3,5},{3,6},{3,7},{3,9},{3,10},{4,6},{4,7},{4,8},{4,11},{5,7},{5,8},{5,9},{6,8},{6,9},{7,8},{7,9},{8,10},{9,11}}

Cousin 18: {{1,4},{1,5},{1,6},{1,9},{1,10},{2,4},{2,6},{2,7},{2,9},{2,11},{3,5},{3,6},{3,7},{3,9},{3,10},{4,6},{4,7},{4,8},{4,9},{5,7},{5,9},{5,11},{6,8},{6,9},{7,8},{7,9},{8,10},{8,11}}

Cousin 19: {{1,4},{1,5},{1,6},{1,9},{1,10},{2,4},{2,6},{2,7},{2,8},{2,11},{3,5},{3,6},{3,7},{3,9},{3,10},{4,6},{4,7},{4,8},{4,9},{5,7},{5,8},{5,11},{6,8},{6,9},{7,8},{7,9},{8,10},{9,11}}

Cousin 20: {{1,4},{1,5},{1,6},{1,9},{1,10},{2,4},{2,5},{2,6},{2,7},{2,8},{2,9},{3,5},{3,6},{3,7},{3,9},{3,10},{4,7},{4,9},{4,11},{5,7},{5,8},{5,9},{6,9},{6,11},{7,8},{7,9},{8,10},{8,11}}

Cousin 21: {{1,4},{1,5},{1,6},{1,9},{1,10},{2,4},{2,5},{2,6},{2,7},{2,8},{2,9},{3,5},{3,6},{3,7},{3,9},{3,10},{4,7},{4,8},{4,11},{5,7},{5,8},{5,9},{6,8},{6,11},{7,8},{7,9},{8,10},{9,11}}

Cousin 22: {{1,4},{1,5},{1,6},{1,9},{1,10},{2,4},{2,5},{2,6},{2,7},{2,8},{2,9},{3,5},{3,6},{3,7},{3,9},{3,10},{4,6},{4,9},{4,11},{5,7},{5,8},{5,9},{6,8},{6,9},{7,9},{7,11},{8,10},{8,11}}

Cousin 23: {{1,4},{1,5},{1,6},{1,9},{1,10},{2,4},{2,5},{2,6},{2,7},{2,8},{2,9},{3,5},{3,6},{3,7},{3,9},{3,10},{4,6},{4,8},{4,11},{5,7},{5,8},{5,9},{6,8},{6,9},{7,8},{7,11},{8,10},{9,11}}

Cousin 24: {{1,3},{1,6},{1,10},{1,11},{2,4},{2,5},{2,6},{2,7},{2,8},{2,9},{3,5},{3,6},{3,7},{3,8},{3,9},{4,6},{4,7},{4,9},{4,10},{5,7},{5,8},{5,11},{6,8},{6,9},{7,8},{7,9},{8,10},{9,11}}

Cousin 25: {{1,3},{1,5},{1,6},{1,9},{1,10},{2,4},{2,6},{2,7},{2,9},{2,11},{3,5},{3,6},{3,7},{3,8},{3,9},{4,6},{4,7},{4,9},{4,10},{5,7},{5,9},{5,11},{6,8},{6,9},{7,8},{7,9},{8,10},{8,11}}

Cousin 26: {{1,3},{1,5},{1,6},{1,9},{1,10},{2,4},{2,6},{2,7},{2,8},{2,11},{3,5},{3,6},{3,7},{3,8},{3,9},{4,6},{4,7},{4,9},{4,10},{5,7},{5,8},{5,11},{6,8},{6,9},{7,8},{7,9},{8,10},{9,11}}

Cousin 27: {{1,3},{1,5},{1,6},{1,9},{1,10},{2,4},{2,5},{2,7},{2,9},{2,11},{3,5},{3,6},{3,7},{3,8},{3,9},{4,6},{4,7},{4,9},{4,10},{5,7},{5,8},{5,9},{6,9},{6,11},{7,8},{7,9},{8,10},{8,11}}

Cousin 28: {{1,3},{1,5},{1,6},{1,9},{1,10},{2,4},{2,5},{2,7},{2,8},{2,11},{3,5},{3,6},{3,7},{3,8},{3,9},{4,6},{4,7},{4,9},{4,10},{5,7},{5,8},{5,9},{6,8},{6,11},{7,8},{7,9},{8,10},{9,11}}

Cousin 29: {{1,8},{1,9},{1,10},{1,11},{2,5},{2,6},{2,8},{2,9},{2,12},{3,6},{3,7},{3,8},{3,9},{3,10},{4,8},{4,9},{4,11},{4,12},{5,7},{5,8},{5,9},{5,10},{6,8},{6,9},{6,11},{7,8},{7,9},{7,12}}

Cousin 30: {{1,8},{1,9},{1,10},{1,11},{2,5},{2,6},{2,7},{2,9},{2,12},{3,6},{3,7},{3,8},{3,9},{3,10},{4,7},{4,9},{4,11},{4,12},{5,7},{5,8},{5,9},{5,10},{6,8},{6,9},{6,11},{7,8},{7,9},{8,12}}

Cousin 31: {{1,8},{1,9},{1,10},{1,11},{2,4},{2,6},{2,7},{2,9},{2,12},{3,6},{3,7},{3,8},{3,9},{3,10},{4,7},{4,8},{4,9},{4,11},{5,7},{5,9},{5,10},{5,12},{6,8},{6,9},{6,11},{7,8},{7,9},{8,12}}

Cousin 32: {{1,8},{1,9},{1,10},{1,11},{2,4},{2,5},{2,7},{2,9},{2,12},{3,6},{3,7},{3,8},{3,9},{3,10},{4,7},{4,8},{4,9},{4,11},{5,7},{5,8},{5,9},{5,10},{6,9},{6,11},{6,12},{7,8},{7,9},{8,12}}

Cousin 33: {{1,8},{1,9},{1,10},{1,11},{2,4},{2,5},{2,6},{2,9},{2,12},{3,6},{3,7},{3,8},{3,9},{3,10},{4,7},{4,8},{4,9},{4,11},{5,7},{5,8},{5,9},{5,10},{6,8},{6,9},{6,11},{7,9},{7,12},{8,12}}

Cousin 34: {{1,8},{1,9},{1,10},{1,11},{2,4},{2,5},{2,6},{2,7},{2,8},{2,9},{3,7},{3,9},{3,10},{3,12},{4,7},{4,8},{4,9},{4,11},{5,7},{5,8},{5,9},{5,10},{6,9},{6,11},{6,12},{7,8},{7,9},{8,12}}

Cousin 35: {{1,10},{1,11},{1,12},{2,4},{2,5},{2,6},{2,7},{2,8},{2,9},{3,6},{3,7},{3,8},{3,9},{3,10},{4,6},{4,7},{4,9},{4,11},{5,7},{5,8},{5,9},{5,10},{6,8},{6,12},{7,8},{7,9},{8,11},{9,12}}

Cousin 36: {{1,6},{1,9},{1,10},{1,11},{2,5},{2,7},{2,8},{2,9},{2,12},{3,6},{3,7},{3,8},{3,9},{3,10},{4,7},{4,9},{4,11},{4,12},{5,7},{5,8},{5,9},{5,10},{6,8},{6,9},{6,12},{7,8},{7,9},{8,11}}

Cousin 37: {{1,6},{1,9},{1,10},{1,11},{2,5},{2,6},{2,8},{2,9},{2,12},{3,6},{3,7},{3,8},{3,9},{3,10},{4,6},{4,9},{4,11},{4,12},{5,7},{5,8},{5,9},{5,10},{6,8},{6,9},{7,8},{7,9},{7,12},{8,11}}

Cousin 38: {{1,6},{1,9},{1,10},{1,11},{2,5},{2,6},{2,7},{2,8},{2,12},{3,6},{3,7},{3,8},{3,9},{3,10},{4,6},{4,7},{4,11},{4,12},{5,7},{5,8},{5,9},{5,10},{6,8},{6,9},{7,8},{7,9},{8,11},{9,12}}

Cousin 39: {{1,6},{1,9},{1,10},{1,11},{2,4},{2,6},{2,7},{2,9},{2,12},{3,6},{3,7},{3,8},{3,9},{3,10},{4,6},{4,7},{4,9},{4,11},{5,7},{5,9},{5,10},{5,12},{6,8},{6,9},{7,8},{7,9},{8,11},{8,12}}

Cousin 40: {{1,6},{1,9},{1,10},{1,11},{2,4},{2,6},{2,7},{2,8},{2,12},{3,6},{3,7},{3,8},{3,9},{3,10},{4,6},{4,7},{4,9},{4,11},{5,7},{5,8},{5,10},{5,12},{6,8},{6,9},{7,8},{7,9},{8,11},{9,12}}

Cousin 41: {{1,6},{1,9},{1,10},{1,11},{2,4},{2,5},{2,7},{2,9},{2,12},{3,6},{3,7},{3,8},{3,9},{3,10},{4,6},{4,7},{4,9},{4,11},{5,7},{5,8},{5,9},{5,10},{6,9},{6,12},{7,8},{7,9},{8,11},{8,12}}

Cousin 42: {{1,6},{1,9},{1,10},{1,11},{2,4},{2,5},{2,7},{2,8},{2,12},{3,6},{3,7},{3,8},{3,9},{3,10},{4,6},{4,7},{4,9},{4,11},{5,7},{5,8},{5,9},{5,10},{6,8},{6,12},{7,8},{7,9},{8,11},{9,12}}

Cousin 43: {{1,6},{1,9},{1,10},{1,11},{2,4},{2,5},{2,6},{2,9},{2,12},{3,6},{3,7},{3,8},{3,9},{3,10},{4,6},{4,7},{4,9},{4,11},{5,7},{5,8},{5,9},{5,10},{6,8},{6,9},{7,9},{7,12},{8,11},{8,12}}

Cousin 44: {{1,6},{1,9},{1,10},{1,11},{2,4},{2,5},{2,6},{2,8},{2,12},{3,6},{3,7},{3,8},{3,9},{3,10},{4,6},{4,7},{4,9},{4,11},{5,7},{5,8},{5,9},{5,10},{6,8},{6,9},{7,8},{7,12},{8,11},{9,12}}

Cousin 45: {{1,6},{1,9},{1,10},{1,11},{2,4},{2,5},{2,6},{2,7},{2,8},{2,9},{3,7},{3,9},{3,10},{3,12},{4,6},{4,7},{4,9},{4,11},{5,7},{5,8},{5,9},{5,10},{6,9},{6,12},{7,8},{7,9},{8,11},{8,12}}

Cousin 46: {{1,6},{1,9},{1,10},{1,11},{2,4},{2,5},{2,6},{2,7},{2,8},{2,9},{3,7},{3,8},{3,10},{3,12},{4,6},{4,7},{4,9},{4,11},{5,7},{5,8},{5,9},{5,10},{6,8},{6,12},{7,8},{7,9},{8,11},{9,12}}

Cousin 47: {{1,6},{1,9},{1,10},{1,11},{2,4},{2,5},{2,6},{2,7},{2,8},{2,9},{3,6},{3,9},{3,10},{3,12},{4,6},{4,7},{4,9},{4,11},{5,7},{5,8},{5,9},{5,10},{6,8},{6,9},{7,9},{7,12},{8,11},{8,12}}

Cousin 48: {{1,6},{1,9},{1,10},{1,11},{2,4},{2,5},{2,6},{2,7},{2,8},{2,9},{3,6},{3,8},{3,10},{3,12},{4,6},{4,7},{4,9},{4,11},{5,7},{5,8},{5,9},{5,10},{6,8},{6,9},{7,8},{7,12},{8,11},{9,12}}

- Cousin 49: {{1,6},{1,9},{1,10},{1,11},{2,4},{2,5},{2,6},{2,7},{2,8},{2,9},{3,6},{3,7},{3,8},{3,9},{3,10},{4,7},{4,11},{4,12},{5,7},{5,8},{5,9},{5,10},{6,8},{6,12},{7,8},{7,9},{8,11},{9,12}}
- Cousin 50: {{1,6},{1,9},{1,10},{1,11},{2,4},{2,5},{2,6},{2,7},{2,8},{2,9},{3,6},{3,7},{3,8},{3,9},{3,10},{4,6},{4,11},{4,12},{5,7},{5,8},{5,9},{5,10},{6,8},{6,9},{7,8},{7,12},{8,11},{9,12}}
- Cousin 51: {{1,6},{1,9},{1,10},{1,11},{2,4},{2,5},{2,6},{2,7},{2,8},{2,9},{3,6},{3,7},{3,8},{3,9},{3,10},{4,6},{4,7},{4,9},{4,11},{5,9},{5,10},{5,12},{6,8},{6,9},{7,9},{7,12},{8,11},{8,12}}
- Cousin 52: {{1,6},{1,9},{1,10},{1,11},{2,4},{2,5},{2,6},{2,7},{2,8},{2,9},{3,6},{3,7},{3,8},{3,9},{3,10},{4,6},{4,7},{4,9},{4,11},{5,8},{5,10},{5,12},{6,8},{6,9},{7,8},{7,12},{8,11},{9,12}}
- Cousin 53: {{1,4},{1,9},{1,10},{1,11},{2,5},{2,7},{2,8},{2,9},{2,12},{3,6},{3,7},{3,8},{3,9},{3,10},{4,7},{4,8},{4,9},{4,12},{5,7},{5,8},{5,9},{5,10},{6,9},{6,11},{6,12},{7,8},{7,9},{8,11}}
- Cousin 54: {{1,4},{1,9},{1,10},{1,11},{2,5},{2,6},{2,8},{2,9},{2,12},{3,6},{3,7},{3,8},{3,9},{3,10},{4,6},{4,8},{4,9},{4,12},{5,7},{5,8},{5,9},{5,10},{6,9},{6,11},{7,8},{7,9},{7,12},{8,11}}
- Cousin 55: {{1,4},{1,9},{1,10},{1,11},{2,5},{2,6},{2,7},{2,9},{2,12},{3,6},{3,7},{3,8},{3,9},{3,10},{4,6},{4,7},{4,9},{4,12},{5,7},{5,8},{5,9},{5,10},{6,9},{6,11},{7,8},{7,9},{8,11},{8,12}}
- Cousin 56: {{1,4},{1,9},{1,10},{1,11},{2,5},{2,6},{2,7},{2,8},{2,12},{3,6},{3,7},{3,8},{3,9},{3,10},{4,6},{4,7},{4,8},{4,12},{5,7},{5,8},{5,9},{5,10},{6,9},{6,11},{7,8},{7,9},{8,11},{9,12}}
- Cousin 57: {{1,4},{1,9},{1,10},{1,11},{2,4},{2,5},{2,7},{2,8},{2,12},{3,6},{3,7},{3,8},{3,9},{3,10},{4,6},{4,7},{4,8},{4,9},{5,7},{5,8},{5,9},{5,10},{6,11},{6,12},{7,8},{7,9},{8,11},{9,12}}
- Cousin 58: {{1,4},{1,9},{1,10},{1,11},{2,4},{2,5},{2,6},{2,9},{2,12},{3,6},{3,7},{3,8},{3,9},{3,10},{4,6},{4,7},{4,8},{4,9},{5,7},{5,8},{5,9},{5,10},{6,9},{6,11},{7,9},{7,12},{8,11},{8,12}}
- Cousin 59: {{1,4},{1,9},{1,10},{1,11},{2,4},{2,5},{2,6},{2,8},{2,12},{3,6},{3,7},{3,8},{3,9},{3,10},{4,6},{4,7},{4,8},{4,9},{5,7},{5,8},{5,9},{5,10},{6,9},{6,11},{7,8},{7,12},{8,11},{9,12}}
- Cousin 60: {{1,4},{1,9},{1,10},{1,11},{2,4},{2,5},{2,6},{2,7},{2,8},{2,9},{3,7},{3,8},{3,10},{3,12},{4,6},{4,7},{4,8},{4,9},{5,7},{5,8},{5,9},{5,10},{6,11},{6,12},{7,8},{7,9},{8,11},{9,12}}
- Cousin 61: {{1,4},{1,9},{1,10},{1,11},{2,4},{2,5},{2,6},{2,7},{2,8},{2,9},{3,6},{3,9},{3,10},{3,12},{4,6},{4,7},{4,8},{4,9},{5,7},{5,8},{5,9},{5,10},{6,9},{6,11},{7,9},{7,12},{8,11},{8,12}}
- Cousin 62: {{1,4},{1,9},{1,10},{1,11},{2,4},{2,5},{2,6},{2,7},{2,8},{2,9},{3,6},{3,8},{3,10},{3,12},{4,6},{4,7},{4,8},{4,9},{5,7},{5,8},{5,9},{5,10},{6,9},{6,11},{7,8},{7,12},{8,11},{9,12}}
- Cousin 63: {{1,4},{1,9},{1,10},{1,11},{2,4},{2,5},{2,6},{2,7},{2,8},{2,9},{3,6},{3,7},{3,8},{3,9},{3,10},{4,7},{4,8},{4,12},{5,7},{5,8},{5,9},{5,10},{6,11},{6,12},{7,8},{7,9},{8,11},{9,12}}
- Cousin 64: {{1,4},{1,9},{1,10},{1,11},{2,4},{2,5},{2,6},{2,7},{2,8},{2,9},{3,6},{3,7},{3,8},{3,9},{3,10},{4,6},{4,9},{4,12},{5,7},{5,8},{5,9},{5,10},{6,9},{6,11},{7,9},{7,12},{8,11},{8,12}}
- Cousin 65: {{1,4},{1,9},{1,10},{1,11},{2,4},{2,5},{2,6},{2,7},{2,8},{2,9},{3,6},{3,7},{3,8},{3,9},{3,10},{4,6},{4,8},{4,12},{5,7},{5,8},{5,9},{5,10},{6,9},{6,11},{7,8},{7,12},{8,11},{9,12}}
- Cousin 66: {{1,4},{1,9},{1,10},{1,11},{2,4},{2,5},{2,6},{2,7},{2,8},{2,9},{3,6},{3,7},{3,8},{3,9},{3,10},{4,6},{4,7},{4,8},{4,9},{5,9},{5,10},{5,12},{6,9},{6,11},{7,9},{7,12},{8,11},{8,12}}
- Cousin 67: {{1,4},{1,9},{1,10},{1,11},{2,4},{2,5},{2,6},{2,7},{2,8},{2,9},{3,6},{3,7},{3,8},{3,9},{3,10},{4,6},{4,7},{4,8},{4,9},{5,8},{5,10},{5,12},{6,9},{6,11},{7,8},{7,12},{8,11},{9,12}}
- Cousin 68: {{1,4},{1,6},{1,8},{1,9},{1,10},{2,5},{2,7},{2,8},{2,9},{2,11},{3,6},{3,9},{3,10},{3,12},{4,7},{4,8},{4,9},{4,11},{5,7},{5,8},{5,9},{5,10},{6,8},{6,9},{6,11},{7,9},{7,12},{8,12}}
- Cousin 69: {{1,4},{1,6},{1,8},{1,9},{1,10},{2,5},{2,7},{2,11},{2,12},{3,6},{3,7},{3,8},{3,9},{3,10},{4,6},{4,7},{4,9},{4,11},{5,7},{5,8},{5,9},{5,10},{6,8},{6,12},{7,8},{7,9},{8,11},{9,12}}
- Cousin 70: {{1,4},{1,6},{1,8},{1,9},{1,10},{2,5},{2,6},{2,11},{2,12},{3,6},{3,7},{3,8},{3,9},{3,10},{4,6},{4,7},{4,9},{4,11},{5,7},{5,8},{5,9},{5,10},{6,8},{6,9},{7,8},{7,12},{8,11},{9,12}}
- Cousin 71: {{1,4},{1,6},{1,8},{1,9},{1,10},{2,5},{2,6},{2,7},{2,9},{2,11},{3,7},{3,9},{3,10},{3,12},{4,6},{4,7},{4,9},{4,11},{5,7},{5,8},{5,9},{5,10},{6,9},{6,12},{7,8},{7,9},{8,11},{8,12}}
- Cousin 72: {{1,4},{1,6},{1,8},{1,9},{1,10},{2,5},{2,6},{2,7},{2,9},{2,11},{3,7},{3,8},{3,10},{3,12},{4,6},{4,7},{4,9},{4,11},{5,7},{5,8},{5,9},{5,10},{6,8},{6,12},{7,8},{7,9},{8,11},{9,12}}
- Cousin 73: {{1,4},{1,6},{1,8},{1,9},{1,10},{2,4},{2,5},{2,11},{2,12},{3,6},{3,7},{3,8},{3,9},{3,10},{4,6},{4,7},{4,8},{4,9},{5,7},{5,8},{5,9},{5,10},{6,9},{6,11},{7,8},{7,12},{8,11},{9,12}}
- Cousin 74: {{1,4},{1,6},{1,8},{1,9},{1,10},{2,4},{2,5},{2,7},{2,9},{2,11},{3,7},{3,8},{3,10},{3,12},{4,6},{4,7},{4,8},{4,9},{5,7},{5,8},{5,9},{5,10},{6,11},{6,12},{7,8},{7,9},{8,11},{9,12}}



{7,9},{8,11},{9,12}}

Cousin 75: {{1,4},{1,6},{1,8},{1,9},{1,10},{2,4},{2,5},{2,7},{2,9},{2,11},{3,6},{3,9},{3,10},{3,12},{4,6},{4,7},{4,8},{4,9},{5,7},{5,8},{5,9},{5,10},{6,9},{6,11},{7,9},{7,12},{8,11},{8,12}}

Cousin 76: {{1,4},{1,6},{1,8},{1,9},{1,10},{2,4},{2,5},{2,7},{2,9},{2,11},{3,6},{3,8},{3,10},{3,12},{4,6},{4,7},{4,8},{4,9},{5,7},{5,8},{5,9},{5,10},{6,9},{6,11},{7,8},{7,12},{8,11},{9,12}}

Cousin 77: {{1,4},{1,6},{1,8},{1,9},{1,10},{2,4},{2,5},{2,7},{2,9},{2,11},{3,6},{3,7},{3,8},{3,9},{3,10},{4,7},{4,8},{4,12},{5,7},{5,8},{5,9},{5,10},{6,11},{6,12},{7,8},{7,9},{8,11},{9,12}}

Cousin 78: {{1,4},{1,6},{1,8},{1,9},{1,10},{2,4},{2,5},{2,7},{2,9},{2,11},{3,6},{3,7},{3,8},{3,9},{3,10},{4,6},{4,9},{4,12},{5,7},{5,8},{5,9},{5,10},{6,9},{6,11},{7,9},{7,12},{8,11},{8,12}}

Cousin 79: {{1,4},{1,6},{1,8},{1,9},{1,10},{2,4},{2,5},{2,7},{2,9},{2,11},{3,6},{3,7},{3,8},{3,9},{3,10},{4,6},{4,8},{4,12},{5,7},{5,8},{5,9},{5,10},{6,9},{6,11},{7,8},{7,12},{8,11},{9,12}}

Cousin 80: {{1,4},{1,6},{1,8},{1,9},{1,10},{2,4},{2,5},{2,6},{2,9},{2,11},{3,7},{3,9},{3,10},{3,12},{4,6},{4,7},{4,8},{4,9},{5,7},{5,8},{5,9},{5,10},{6,9},{6,12},{7,9},{7,11},{8,11},{8,12}}

Cousin 81: {{1,4},{1,6},{1,8},{1,9},{1,10},{2,4},{2,5},{2,6},{2,9},{2,11},{3,7},{3,8},{3,10},{3,12},{4,6},{4,7},{4,8},{4,9},{5,7},{5,8},{5,9},{5,10},{6,8},{6,12},{7,9},{7,11},{8,11},{9,12}}

Cousin 82: {{1,4},{1,6},{1,8},{1,9},{1,10},{2,4},{2,5},{2,6},{2,9},{2,11},{3,6},{3,8},{3,10},{3,12},{4,6},{4,7},{4,8},{4,9},{5,7},{5,8},{5,9},{5,10},{6,8},{6,9},{7,11},{7,12},{8,11},{9,12}}

Cousin 83: {{1,4},{1,6},{1,8},{1,9},{1,10},{2,4},{2,5},{2,6},{2,9},{2,11},{3,6},{3,7},{3,8},{3,9},{3,10},{4,7},{4,9},{4,12},{5,7},{5,8},{5,9},{5,10},{6,9},{6,12},{7,9},{7,11},{8,11},{8,12}}

Cousin 84: {{1,4},{1,6},{1,8},{1,9},{1,10},{2,4},{2,5},{2,6},{2,9},{2,11},{3,6},{3,7},{3,8},{3,9},{3,10},{4,7},{4,8},{4,12},{5,7},{5,8},{5,9},{5,10},{6,8},{6,12},{7,9},{7,11},{8,11},{9,12}}

Cousin 85: {{1,4},{1,6},{1,8},{1,9},{1,10},{2,4},{2,5},{2,6},{2,7},{2,8},{2,9},{3,10},{3,11},{3,12},{4,6},{4,7},{4,8},{4,9},{5,7},{5,8},{5,9},{5,10},{6,9},{6,11},{7,8},{7,12},{8,11},{9,12}}

Cousin 86: {{1,5},{1,6},{1,10},{1,11},{2,5},{2,6},{2,7},{2,9},{2,12},{3,5},{3,6},{3,7},{3,9},{3,10},{4,6},{4,7},{4,11},{4,12},{5,7},{5,8},{5,9},{6,8},{6,9},{7,8},{7,9},{8,10},{8,12},{9,11}}

Cousin 87: {{1,5},{1,6},{1,10},{1,11},{2,4},{2,6},{2,7},{2,9},{2,12},{3,5},{3,6},{3,7},{3,9},{3,10},{4,6},{4,7},{4,8},{4,11},{5,7},{5,9},{5,12},{6,8},{6,9},{7,8},{7,9},{8,10},{8,12},{9,11}}

Cousin 88: {{1,5},{1,6},{1,10},{1,11},{2,4},{2,6},{2,7},{2,8},{2,12},{3,5},{3,6},{3,7},{3,9},{3,10},{4,6},{4,7},{4,8},{4,11},{5,7},{5,8},{5,12},{6,8},{6,9},{7,8},{7,9},{8,10},{9,11},{9,12}}

Cousin 89: {{1,5},{1,6},{1,10},{1,11},{2,4},{2,5},{2,7},{2,9},{2,12},{3,5},{3,6},{3,7},{3,9},{3,10},{4,6},{4,7},{4,8},{4,11},{5,7},{5,8},{5,9},{6,9},{6,12},{7,8},{7,9},{8,10},{8,12},{9,11}}

Cousin 90: {{1,5},{1,6},{1,10},{1,11},{2,4},{2,5},{2,7},{2,8},{2,12},{3,5},{3,6},{3,7},{3,9},{3,10},{4,6},{4,7},{4,8},{4,11},{5,7},{5,8},{5,9},{6,8},{6,12},{7,8},{7,9},{8,10},{9,11},{9,12}}

Cousin 91: {{1,5},{1,6},{1,10},{1,11},{2,4},{2,5},{2,6},{2,9},{2,12},{3,5},{3,6},{3,7},{3,9},{3,10},{4,6},{4,7},{4,8},{4,11},{5,7},{5,8},{5,9},{6,8},{6,9},{7,9},{7,12},{8,10},{8,12},{9,11}}

Cousin 92: {{1,5},{1,6},{1,10},{1,11},{2,4},{2,5},{2,6},{2,8},{2,12},{3,5},{3,6},{3,7},{3,9},{3,10},{4,6},{4,7},{4,8},{4,11},{5,7},{5,8},{5,9},{6,8},{6,9},{7,8},{7,12},{8,10},{9,11},{9,12}}

Cousin 93: {{1,5},{1,6},{1,10},{1,11},{2,4},{2,5},{2,6},{2,7},{2,8},{2,9},{3,6},{3,7},{3,10},{3,12},{4,6},{4,7},{4,8},{4,11},{5,7},{5,8},{5,12},{6,8},{6,9},{7,8},{7,9},{8,10},{9,11},{9,12}}

Cousin 94: {{1,5},{1,6},{1,10},{1,11},{2,4},{2,5},{2,6},{2,7},{2,8},{2,9},{3,5},{3,7},{3,10},{3,12},{4,6},{4,7},{4,8},{4,11},{5,7},{5,8},{5,9},{6,8},{6,12},{7,8},{7,9},{8,10},{9,11},{9,12}}

Cousin 95: {{1,5},{1,6},{1,10},{1,11},{2,4},{2,5},{2,6},{2,7},{2,8},{2,9},{3,5},{3,6},{3,10},{3,12},{4,6},{4,7},{4,8},{4,11},{5,7},{5,8},{5,9},{6,8},{6,9},{7,8},{7,12},{8,10},{9,11},{9,12}}

Cousin 96: {{1,5},{1,6},{1,10},{1,11},{2,4},{2,5},{2,6},{2,7},{2,8},{2,9},{3,5},{3,6},{3,7},{3,9},{3,10},{4,7},{4,11},{4,12},{5,7},{5,8},{5,9},{6,9},{6,12},{7,8},{7,9},{8,10},{8,12},{9,11}}

Cousin 97: {{1,5},{1,6},{1,10},{1,11},{2,4},{2,5},{2,6},{2,7},{2,8},{2,9},{3,5},{3,6},{3,7},{3,9},{3,10},{4,6},{4,11},{4,12},{5,7},{5,8},{5,9},{6,8},{6,9},{7,9},{7,12},{8,10},{8,12},{9,11}}

Cousin 98: {{1,5},{1,6},{1,10},{1,11},{2,4},{2,5},{2,6},{2,7},{2,8},{2,9},{3,5},{3,6},{3,7},{3,9},{3,10},{4,6},{4,7},{4,8},{4,11},{5,9},{5,12},{6,8},{6,9},{7,9},{7,12},{8,10},{8,12},{9,11}}

Cousin 99: {{1,5},{1,6},{1,10},{1,11},{2,4},{2,5},{2,6},{2,7},{2,8},{2,9},{3,5},{3,6},{3,7},{3,9},{3,10},{4,6},{4,7},{4,8},{4,11},{5,8},{5,12},{6,8},{6,9},{7,8},{7,12},{8,10},{9,11},{9,12}}

Cousin 100: {{1,4},{1,6},{1,10},{1,11},{2,5},{2,6},{2,7},{2,9},{2,12},{3,5},{3,6},{3,7},{3,9},{3,10},{4,6},{4,7},{4,9},{4,12},{5,7},{5,8},{5,11},{6,8},{6,9},{7,8},{7,9},{8,10},{8,12},{9,11}}

Cousin 101: {{1,4},{1,6},{1,10},{1,11},{2,5},{2,6},{2,7},{2,8},{2,12},{3,5},{3,6},{3,7},{3,9},{3,10},{4,6},{4,7},{4,8},{4,12},{5,7},{5,8},{5,11},{6,8},{6,9},{7,8},{7,9},{8,10},{9,11},{9,12}}

Cousin 102: {{1,4},{1,6},{1,10},{1,11},{2,4},{2,6},{2,7},{2,9},{2,12},{3,5},{3,6},{3,7},{3,9},{3,10},{4,6},{4,7},{4,8},{4,9},{5,7},{5,11},{5,12},{6,8},{6,9},{7,8},{7,9},{8,10},{8,12},{9,11}}

Cousin 103: {{1,4},{1,6},{1,10},{1,11},{2,4},{2,5},{2,7},{2,9},{2,12},{3,5},{3,6},{3,7},{3,9},{3,10},{4,6},{4,7},{4,8},{4,9},{5,7},{5,8},{5,11},{6,9},{6,12},{7,8},{7,9},{8,10},{8,12},{9,11}}

Cousin 104: {{1,4},{1,6},{1,10},{1,11},{2,4},{2,5},{2,7},{2,8},{2,12},{3,5},{3,6},{3,7},{3,9},{3,10},{4,6},{4,7},{4,8},{4,9},{5,7},{5,8},{5,11},{6,8},{6,12},{7,8},{7,9},{8,10},{9,11},{9,12}}

Cousin 105: {{1,4},{1,6},{1,10},{1,11},{2,4},{2,5},{2,6},{2,9},{2,12},{3,5},{3,6},{3,7},{3,9},{3,10},{4,6},{4,7},{4,8},{4,9},{5,7},{5,8},{5,11},{6,8},{6,9},{7,9},{7,12},{8,10},{8,12},{9,11}}

Cousin 106: {{1,4},{1,6},{1,10},{1,11},{2,4},{2,5},{2,6},{2,8},{2,12},{3,5},{3,6},{3,7},{3,9},{3,10},{4,6},{4,7},{4,8},{4,9},{5,7},{5,8},{5,11},{6,8},{6,9},{7,8},{7,12},{8,10},{9,11},{9,12}}

Cousin 107: {{1,4},{1,6},{1,10},{1,11},{2,4},{2,5},{2,6},{2,7},{2,8},{2,9},{3,5},{3,7},{3,10},{3,12},{4,6},{4,7},{4,8},{4,9},{5,7},{5,8},{5,11},{6,8},{6,12},{7,8},{7,9},{8,10},{9,11},{9,12}}

Cousin 108: {{1,4},{1,6},{1,10},{1,11},{2,4},{2,5},{2,6},{2,7},{2,8},{2,9},{3,5},{3,6},{3,7},{3,9},{3,10},{4,7},{4,9},{4,12},{5,7},{5,8},{5,11},{6,9},{6,12},{7,8},{7,9},{8,10},{8,12},{9,11}}

Cousin 109: {{1,4},{1,6},{1,10},{1,11},{2,4},{2,5},{2,6},{2,7},{2,8},{2,9},{3,5},{3,6},{3,7},{3,9},{3,10},{4,7},{4,8},{4,12},{5,7},{5,8},{5,11},{6,8},{6,12},{7,8},{7,9},{8,10},{9,11},{9,12}}

Cousin 110: {{1,4},{1,6},{1,10},{1,11},{2,4},{2,5},{2,6},{2,7},{2,8},{2,9},{3,5},{3,6},{3,7},{3,9},{3,10},{4,6},{4,9},{4,12},{5,7},{5,8},{5,11},{6,8},{6,9},{7,9},{7,12},{8,10},{8,12},{9,11}}

Cousin 111: {{1,4},{1,6},{1,10},{1,11},{2,4},{2,5},{2,6},{2,7},{2,8},{2,9},{3,5},{3,6},{3,7},{3,9},{3,10},{4,6},{4,8},{4,12},{5,7},{5,8},{5,11},{6,8},{6,9},{7,8},{7,12},{8,10},{9,11},{9,12}}

Cousin 112: {{1,4},{1,5},{1,10},{1,11},{2,5},{2,6},{2,7},{2,9},{2,12},{3,5},{3,6},{3,7},{3,9},{3,10},{4,6},{4,7},{4,9},{4,12},{5,7},{5,8},{5,9},{6,8},{6,11},{7,8},{7,9},{8,10},{8,12},{9,11}}

Cousin 113: {{1,4},{1,5},{1,10},{1,11},{2,5},{2,6},{2,7},{2,8},{2,12},{3,5},{3,6},{3,7},{3,9},{3,10},{4,6},{4,7},{4,8},{4,12},{5,7},{5,8},{5,9},{6,8},{6,11},{7,8},{7,9},{8,10},{9,11},{9,12}}

Cousin 114: {{1,4},{1,5},{1,10},{1,11},{2,4},{2,6},{2,7},{2,9},{2,12},{3,5},{3,6},{3,7},{3,9},{3,10},{4,6},{4,7},{4,8},{4,9},{5,7},{5,9},{5,12},{6,8},{6,11},{7,8},{7,9},{8,10},{8,12},{9,11}}

Cousin 115: {{1,4},{1,5},{1,10},{1,11},{2,4},{2,6},{2,7},{2,8},{2,12},{3,5},{3,6},{3,7},{3,9},{3,10},{4,6},{4,7},{4,8},{4,9},{5,7},{5,8},{5,12},{6,8},{6,11},{7,8},{7,9},{8,10},{9,11},{9,12}}

Cousin 116: {{1,4},{1,5},{1,10},{1,11},{2,4},{2,5},{2,6},{2,9},{2,12},{3,5},{3,6},{3,7},{3,9},{3,10},{4,6},{4,7},{4,8},{4,9},{5,7},{5,8},{5,9},{6,8},{6,11},{7,9},{7,12},{8,10},{8,12},{9,11}}

Cousin 117: {{1,4},{1,5},{1,10},{1,11},{2,4},{2,5},{2,6},{2,7},{2,8},{2,9},{3,6},{3,7},{3,10},{3,12},{4,6},{4,7},{4,8},{4,9},{5,7},{5,8},{5,12},{6,8},{6,11},{7,8},{7,9},{8,10},{9,11},{9,12}}

Cousin 118: {{1,4},{1,5},{1,6},{1,9},{1,10},{2,5},{2,6},{2,7},{2,9},{2,11},{3,5},{3,6},{3,7},{3,9},{3,10},{4,6},{4,7},{4,9},{4,11},{5,9},{5,12},{6,8},{6,9},{7,9},{7,12},{8,10},{8,11},{8,12}}

Cousin 119: {{1,4},{1,5},{1,6},{1,9},{1,10},{2,5},{2,6},{2,7},{2,9},{2,11},{3,5},{3,6},{3,7},{3,9},{3,10},{4,6},{4,7},{4,9},{4,11},{5,8},{5,12},{6,8},{6,9},{7,8},{7,12},{8,10},{8,11},{9,12}}

Cousin 120: {{1,4},{1,5},{1,6},{1,9},{1,10},{2,5},{2,6},{2,7},{2,8},{2,11},{3,5},{3,6},{3,7},{3,9},{3,10},{4,6},{4,7},{4,8},{4,11},{5,9},{5,12},{6,8},{6,9},{7,9},{7,12},{8,10},{8,12},{9,11}}

Cousin 121: {{1,4},{1,5},{1,6},{1,9},{1,10},{2,4},{2,7},{2,11},{2,12},{3,5},{3,6},{3,7},{3,9},{3,10},{4,6},{4,7},{4,8},{4,9},{5,7},{5,9},{5,11},{6,8},{6,12},{7,8},{7,9},{8,10},{8,11},{9,12}}

Cousin 122: {{1,4},{1,5},{1,6},{1,9},{1,10},{2,4},{2,6},{2,7},{2,9},{2,11},{3,5},{3,6},{3,7},{3,9},{3,10},{4,7},{4,9},{4,12},{5,7},{5,9},{5,11},{6,9},{6,12},{7,8},{7,9},{8,10},{8,11},{8,12}}

Cousin 123: {{1,4},{1,5},{1,6},{1,9},{1,10},{2,4},{2,6},{2,7},{2,9},{2,11},{3,5},{3,6},{3,7},{3,9},{3,10},{4,7},{4,8},{4,12},{5,7},{5,9},{5,11},{6,8},{6,12},{7,8},{7,9},{8,10},{8,11},{9,12}}

Cousin 124: {{1,4},{1,5},{1,6},{1,9},{1,10},{2,4},{2,6},{2,7},{2,9},{2,11},{3,5},{3,6},{3,7},{3,9},{3,10},{4,6},{4,9},{4,12},{5,7},{5,9},{5,11},{6,8},{6,9},{7,9},{7,12},{8,10},{8,11},{8,12}}

Cousin 125: {{1,4},{1,5},{1,6},{1,9},{1,10},{2,4},{2,6},{2,7},{2,9},{2,11},{3,5},{3,6},{3,7},{3,9},{3,10},{4,6},{4,8},{4,12},{5,7},{5,9},{5,11},{6,8},{6,9},{7,8},{7,12},{8,10},{8,11},{9,12}}

Cousin 126: {{1,4},{1,5},{1,6},{1,9},{1,10},{2,4},{2,6},{2,7},{2,8},{2,11},{3,5},{3,6},{3,7},{3,9},{3,10},{4,7},{4,9},{4,12},{5,7},{5,8},{5,11},{6,9},{6,12},{7,8},{7,9},{8,10},{8,12},{9,11}}

Cousin 127: {{1,4},{1,5},{1,6},{1,9},{1,10},{2,4},{2,6},{2,7},{2,8},{2,11},{3,5},{3,6},{3,7},{3,9},{3,10},{4,6},{4,9},{4,12},{5,7},{5,8},{5,11},{6,8},{6,9},{7,9},{7,12},{8,10},{8,12},{9,11}}

Cousin 128: {{1,4},{1,5},{1,6},{1,9},{1,10},{2,4},{2,6},{2,7},{2,8},{2,11},{3,5},{3,6},{3,7},{3,9},{3,10},{4,6},{4,8},{4,12},{5,7},{5,8},{5,11},{6,8},{6,9},{7,8},{7,12},{8,10},{9,11},{9,12}}

Cousin 129: {{1,3},{1,6},{1,10},{1,11},{2,4},{2,6},{2,7},{2,9},{2,12},{3,5},{3,6},{3,7},{3,8},{3,9},{4,6},{4,7},{4,9},{4,10},{5,7},{5,11},{5,12},{6,8},{6,9},{7,8},{7,9},{8,10},{8,12},{9,11}}

Cousin 130: {{1,3},{1,6},{1,10},{1,11},{2,4},{2,5},{2,7},{2,9},{2,12},{3,5},{3,6},{3,7},{3,8},{3,9},{4,6},{4,7},{4,9},{4,10},{5,7},{5,8},{5,11},{6,9},{6,12},{7,8},{7,9},{8,10},{8,12},{9,11}}

Cousin 131: {{1,3},{1,6},{1,10},{1,11},{2,4},{2,5},{2,7},{2,8},{2,12},{3,5},{3,6},{3,7},{3,8},{3,9},{4,6},{4,7},{4,9},{4,10},{5,7},{5,8},{5,11},{6,8},{6,12},{7,8},{7,9},{8,10},{9,11},{9,12}}

Cousin 132: {{1,3},{1,6},{1,10},{1,11},{2,4},{2,5},{2,6},{2,7},{2,8},{2,9},{3,5},{3,7},{3,9},{3,12},{4,6},{4,7},{4,9},{4,10},{5,7},{5,8},{5,11},{6,9},{6,12},{7,8},{7,9},{8,10},{8,12},{9,11}}

Cousin 133: {{1,3},{1,5},{1,6},{1,9},{1,10},{2,4},{2,6},{2,7},{2,9},{2,11},{3,5},{3,7},{3,9},{3,12},{4,6},{4,7},{4,9},{4,10},{5,7},{5,9},{5,11},{6,9},{6,12},{7,8},{7,9},{8,10},{8,11},{8,12}}

Cousin 134: {{1,3},{1,5},{1,6},{1,9},{1,10},{2,4},{2,6},{2,7},{2,9},{2,11},{3,5},{3,7},{3,8},{3,12},{4,6},{4,7},{4,9},{4,10},{5,7},{5,9},{5,11},{6,8},{6,12},{7,8},{7,9},{8,10},{8,11},{9,12}}

Cousin 135: {{1,3},{1,5},{1,6},{1,9},{1,10},{2,4},{2,6},{2,7},{2,8},{2,11},{3,5},{3,7},{3,9},{3,12},{4,6},{4,7},{4,9},{4,10},{5,7},{5,8},{5,11},{6,9},{6,12},{7,8},{7,9},{8,10},{8,12},{9,11}}

Cousin 136: {{1,8},{1,9},{1,10},{1,11},{2,6},{2,9},{2,12},{2,13},{3,6},{3,7},{3,8},{3,9},{3,10},{4,8},{4,9},{4,11},{4,12},{5,7},{5,9},{5,10},{5,13},{6,8},{6,9},{6,11},{7,8},{7,9},{7,12},{8,13}}

Cousin 137: {{1,8},{1,9},{1,10},{1,11},{2,5},{2,9},{2,12},{2,13},{3,6},{3,7},{3,8},{3,9},{3,10},{4,8},{4,9},{4,11},{4,12},{5,7},{5,8},{5,9},{5,10},{6,9},{6,11},{6,13},{7,8},{7,9},{7,12},{8,13}}

Cousin 138: {{1,8},{1,9},{1,10},{1,11},{2,5},{2,6},{2,8},{2,9},{2,12},{3,6},{3,7},{3,8},{3,9},{3,10},{4,8},{4,9},{4,11},{4,12},{5,9},{5,10},{5,13},{6,8},{6,9},{6,11},{7,9},{7,12},{7,13},{8,13}}

Cousin 139: {{1,8},{1,9},{1,10},{1,11},{2,6},{2,7},{2,12},{2,13},{3,6},{3,7},{3,8},{3,9},{3,10},{4,7},{4,9},{4,11},{4,12},{5,7},{5,8},{5,10},{5,13},{6,8},{6,9},{6,11},{7,8},{7,9},{8,12},{9,13}}

Cousin 140: {{1,8},{1,9},{1,10},{1,11},{2,5},{2,7},{2,12},{2,13},{3,6},{3,7},{3,8},{3,9},{3,10},{4,7},{4,9},{4,11},{4,12},{5,7},{5,8},{5,9},{5,10},{6,8},{6,11},{6,13},{7,8},{7,9},{8,12},{9,13}}

Cousin 141: {{1,8},{1,9},{1,10},{1,11},{2,5},{2,6},{2,12},{2,13},{3,6},{3,7},{3,8},{3,9},{3,10},{4,7},{4,9},{4,11},{4,12},{5,7},{5,8},{5,9},{5,10},{6,8},{6,9},{6,11},{7,8},{7,13},{8,12},{9,13}}

Cousin 142: {{1,8},{1,9},{1,10},{1,11},{2,5},{2,6},{2,7},{2,9},{2,12},{3,7},{3,9},{3,10},{3,13},{4,7},{4,9},{4,11},{4,12},{5,7},{5,8},{5,9},{5,10},{6,9},{6,11},{6,13},{7,8},{7,9},{8,12},{8,13}}

Cousin 143: {{1,8},{1,9},{1,10},{1,11},{2,5},{2,6},{2,7},{2,9},{2,12},{3,7},{3,8},{3,10},{3,13},{4,7},{4,9},{4,11},{4,12},{5,7},{5,8},{5,9},{5,10},{6,8},{6,11},{6,13},{7,8},{7,9},{8,12},{9,13}}

Cousin 144: {{1,8},{1,9},{1,10},{1,11},{2,5},{2,6},{2,7},{2,9},{2,12},{3,6},{3,9},{3,10},{3,13},{4,7},{4,9},{4,11},{4,12},{5,7},{5,8},{5,9},{5,10},{6,8},{6,9},{6,11},{7,9},{7,13},{8,12},{8,13}}

Cousin 145: {{1,8},{1,9},{1,10},{1,11},{2,5},{2,6},{2,7},{2,9},{2,12},{3,6},{3,8},{3,10},{3,13},{4,7},{4,9},{4,11},{4,12},{5,7},{5,8},{5,9},{5,10},{6,8},{6,9},{6,11},{7,8},{7,13},{8,12},{9,13}}

Cousin 146: {{1,8},{1,9},{1,10},{1,11},{2,5},{2,6},{2,7},{2,9},{2,12},{3,6},{3,7},{3,8},{3,9},{3,10},{4,11},{4,12},{4,13},{5,7},{5,8},{5,9},{5,10},{6,8},{6,9},{6,11},{7,8},{7,13},{8,12},{9,13}}

Cousin 147: {{1,8},{1,9},{1,10},{1,11},{2,5},{2,6},{2,7},{2,9},{2,12},{3,6},{3,7},{3,8},{3,9},{3,10},{4,7},{4,9},{4,11},{4,12},{5,9},{5,10},{5,13},{6,8},{6,9},{6,11},{7,9},{7,13},{8,12},{8,13}}

Cousin 148: {{1,8},{1,9},{1,10},{1,11},{2,5},{2,6},{2,7},{2,9},{2,12},{3,6},{3,7},{3,8},{3,9},{3,10},{4,7},{4,9},{4,11},{4,12},{5,8},{5,10},{5,13},{6,8},{6,9},{6,11},{7,8},{7,13},{8,12},{9,13}}

Cousin 149: {{1,8},{1,9},{1,10},{1,11},{2,4},{2,7},{2,12},{2,13},{3,6},{3,7},{3,8},{3,9},{3,10},{4,7},{4,8},{4,9},{4,11},{5,7},{5,9},{5,10},{5,12},{6,8},{6,11},{6,13},{7,8},{7,9},{8,12},{9,13}}

Cousin 150: {{1,8},{1,9},{1,10},{1,11},{2,4},{2,6},{2,12},{2,13},{3,6},{3,7},{3,8},{3,9},{3,10},{4,7},{4,8},{4,9},{4,11},{5,7},{5,9},{5,10},{5,12},{6,8},{6,9},{6,11},{7,8},{7,9},{8,12},{9,13}}

{7,8},{7,13},{8,12},{9,13}}

Cousin 151: {{1,8},{1,9},{1,10},{1,11},{2,4},{2,6},{2,7},{2,9},{2,12},{3,7},{3,9},{3,10},{3,13},{4,7},{4,8},{4,9},{4,11},{5,7},{5,9},{5,10},{5,12},{6,9},{6,11},{6,13},{7,8},{7,9},{8,12},{8,13}}

Cousin 152: {{1,8},{1,9},{1,10},{1,11},{2,4},{2,6},{2,7},{2,9},{2,12},{3,7},{3,8},{3,10},{3,13},{4,7},{4,8},{4,9},{4,11},{5,7},{5,9},{5,10},{5,12},{6,8},{6,11},{6,13},{7,8},{7,9},{8,12},{9,13}}

Cousin 153: {{1,8},{1,9},{1,10},{1,11},{2,4},{2,6},{2,7},{2,9},{2,12},{3,6},{3,9},{3,10},{3,13},{4,7},{4,8},{4,9},{4,11},{5,7},{5,9},{5,10},{5,12},{6,8},{6,9},{6,11},{7,9},{7,13},{8,12},{8,13}}

Cousin 154: {{1,8},{1,9},{1,10},{1,11},{2,4},{2,6},{2,7},{2,9},{2,12},{3,6},{3,8},{3,10},{3,13},{4,7},{4,8},{4,9},{4,11},{5,7},{5,9},{5,10},{5,12},{6,8},{6,9},{6,11},{7,8},{7,13},{8,12},{9,13}}

Cousin 155: {{1,8},{1,9},{1,10},{1,11},{2,4},{2,6},{2,7},{2,9},{2,12},{3,6},{3,7},{3,8},{3,9},{3,10},{4,9},{4,11},{4,13},{5,7},{5,9},{5,10},{5,12},{6,8},{6,9},{6,11},{7,9},{7,13},{8,12},{8,13}}

Cousin 156: {{1,8},{1,9},{1,10},{1,11},{2,4},{2,6},{2,7},{2,9},{2,12},{3,6},{3,7},{3,8},{3,9},{3,10},{4,8},{4,11},{4,13},{5,7},{5,9},{5,10},{5,12},{6,8},{6,9},{6,11},{7,8},{7,13},{8,12},{9,13}}

Cousin 157: {{1,8},{1,9},{1,10},{1,11},{2,4},{2,5},{2,12},{2,13},{3,6},{3,7},{3,8},{3,9},{3,10},{4,7},{4,8},{4,9},{4,11},{5,7},{5,8},{5,9},{5,10},{6,9},{6,11},{6,12},{7,8},{7,13},{8,12},{9,13}}

Cousin 158: {{1,8},{1,9},{1,10},{1,11},{2,4},{2,5},{2,7},{2,9},{2,12},{3,7},{3,8},{3,10},{3,13},{4,7},{4,8},{4,9},{4,11},{5,7},{5,8},{5,9},{5,10},{6,11},{6,12},{6,13},{7,8},{7,9},{8,12},{9,13}}

Cousin 159: {{1,8},{1,9},{1,10},{1,11},{2,4},{2,5},{2,7},{2,9},{2,12},{3,6},{3,9},{3,10},{3,13},{4,7},{4,8},{4,9},{4,11},{5,7},{5,8},{5,9},{5,10},{6,9},{6,11},{6,12},{7,9},{7,13},{8,12},{8,13}}

Cousin 160: {{1,8},{1,9},{1,10},{1,11},{2,4},{2,5},{2,7},{2,9},{2,12},{3,6},{3,8},{3,10},{3,13},{4,7},{4,8},{4,9},{4,11},{5,7},{5,8},{5,9},{5,10},{6,9},{6,11},{6,12},{7,8},{7,13},{8,12},{9,13}}

Cousin 161: {{1,8},{1,9},{1,10},{1,11},{2,4},{2,5},{2,6},{2,9},{2,12},{3,7},{3,9},{3,10},{3,13},{4,7},{4,8},{4,9},{4,11},{5,7},{5,8},{5,9},{5,10},{6,9},{6,11},{6,13},{7,9},{7,12},{8,12},{8,13}}

Cousin 162: {{1,8},{1,9},{1,10},{1,11},{2,4},{2,5},{2,6},{2,9},{2,12},{3,7},{3,8},{3,10},{3,13},{4,7},{4,8},{4,9},{4,11},{5,7},{5,8},{5,9},{5,10},{6,8},{6,11},{6,13},{7,9},{7,12},{8,12},{9,13}}

Cousin 163: {{1,10},{1,11},{1,12},{2,5},{2,7},{2,8},{2,9},{2,13},{3,6},{3,7},{3,8},{3,9},{3,10},{4,7},{4,9},{4,11},{4,13},{5,7},{5,8},{5,9},{5,10},{6,8},{6,12},{6,13},{7,8},{7,9},{8,11},{9,12}}

Cousin 164: {{1,10},{1,11},{1,12},{2,5},{2,6},{2,8},{2,9},{2,13},{3,6},{3,7},{3,8},{3,9},{3,10},{4,6},{4,9},{4,11},{4,13},{5,7},{5,8},{5,9},{5,10},{6,8},{6,12},{7,8},{7,9},{7,13},{8,11},{9,12}}

Cousin 165: {{1,10},{1,11},{1,12},{2,5},{2,6},{2,7},{2,8},{2,13},{3,6},{3,7},{3,8},{3,9},{3,10},{4,6},{4,7},{4,11},{4,13},{5,7},{5,8},{5,9},{5,10},{6,8},{6,12},{7,8},{7,9},{8,11},{9,12},{9,13}}

Cousin 166: {{1,10},{1,11},{1,12},{2,4},{2,6},{2,7},{2,9},{2,13},{3,6},{3,7},{3,8},{3,9},{3,10},{4,6},{4,7},{4,9},{4,11},{5,7},{5,9},{5,10},{5,13},{6,8},{6,12},{7,8},{7,9},{8,11},{8,13},{9,12}}

Cousin 167: {{1,10},{1,11},{1,12},{2,4},{2,6},{2,7},{2,8},{2,13},{3,6},{3,7},{3,8},{3,9},{3,10},{4,6},{4,7},{4,9},{4,11},{5,7},{5,8},{5,10},{5,13},{6,8},{6,12},{7,8},{7,9},{8,11},{9,12},{9,13}}

Cousin 168: {{1,10},{1,11},{1,12},{2,4},{2,5},{2,7},{2,9},{2,13},{3,6},{3,7},{3,8},{3,9},{3,10},{4,6},{4,7},{4,9},{4,11},{5,7},{5,8},{5,9},{5,10},{6,12},{6,13},{7,8},{7,9},{8,11},{8,13},{9,12}}

Cousin 169: {{1,10},{1,11},{1,12},{2,4},{2,5},{2,6},{2,9},{2,13},{3,6},{3,7},{3,8},{3,9},{3,10},{4,6},{4,7},{4,9},{4,11},{5,7},{5,8},{5,9},{5,10},{6,8},{6,12},{7,9},{7,13},{8,11},{8,13},{9,12}}

Cousin 170: {{1,10},{1,11},{1,12},{2,4},{2,5},{2,6},{2,8},{2,13},{3,6},{3,7},{3,8},{3,9},{3,10},{4,6},{4,7},{4,9},{4,11},{5,7},{5,8},{5,9},{5,10},{6,8},{6,12},{7,8},{7,13},{8,11},{9,12},{9,13}}

Cousin 171: {{1,10},{1,11},{1,12},{2,4},{2,5},{2,6},{2,7},{2,8},{2,9},{3,7},{3,9},{3,10},{3,13},{4,6},{4,7},{4,9},{4,11},{5,7},{5,8},{5,9},{5,10},{6,12},{6,13},{7,8},{7,9},{8,11},{8,13},{9,12}}

Cousin 172: {{1,10},{1,11},{1,12},{2,4},{2,5},{2,6},{2,7},{2,8},{2,9},{3,6},{3,9},{3,10},{3,13},{4,6},{4,7},{4,9},{4,11},{5,7},{5,8},{5,9},{5,10},{6,8},{6,12},{7,9},{7,13},{8,11},{8,13},{9,12}}

Cousin 173: {{1,10},{1,11},{1,12},{2,4},{2,5},{2,6},{2,7},{2,8},{2,9},{3,6},{3,8},{3,10},{3,13},{4,6},{4,7},{4,9},{4,11},{5,7},{5,8},{5,9},{5,10},{6,8},{6,12},{7,8},{7,13},{8,11},{9,12},{9,13}}

Cousin 174: {{1,10},{1,11},{1,12},{2,4},{2,5},{2,6},{2,7},{2,8},{2,9},{3,6},{3,7},{3,8},{3,9},{3,10},{4,6},{4,11},{4,13},{5,7},{5,8},{5,9},{5,10},{6,8},{6,12},{7,8},{7,13},{8,11},{9,12},{9,13}}

Cousin 175: {{1,10},{1,11},{1,12},{2,4},{2,5},{2,6},{2,7},{2,8},{2,9},{3,6},{3,7},{3,8},{3,9},{3,10},{4,6},{4,7},{4,9},{4,11},{5,9},{5,10},{5,13},{6,8},{6,12},{7,9},{7,13},{8,11},{8,13},{9,12}}

Cousin 176: {{1,10},{1,11},{1,12},{2,4},{2,5},{2,6},{2,7},{2,8},{2,9},{3,6},{3,7},{3,8},{3,9},{3,10},{4,6},{4,7},{4,9},{4,11},{5,8},{5,10},{5,13},{6,8},{6,12},{7,8},{7,13},{8,11},{9,12},{9,13}}

Cousin 177: {{1,6},{1,9},{1,10},{1,11},{2,4},{2,5},{2,6},{2,7},{2,8},{2,9},{3,6},{3,7},{3,8},{3,9},{3,10},{4,6},{4,7},{4,9},{4,11},{5,7},{5,8},{5,9},{5,10},{6,8},{7,8},{7,9},{8,11},{10,11}}

Cousin 178: {{1,6},{1,9},{1,10},{1,11},{2,7},{2,9},{2,12},{2,13},{3,6},{3,7},{3,8},{3,9},{3,10},{4,7},{4,9},{4,11},{4,12},{5,7},{5,9},{5,10},{5,13},{6,8},{6,9},{6,12},{7,8},{7,9},{8,11},{8,13}}

Cousin 179: {{1,6},{1,9},{1,10},{1,11},{2,7},{2,8},{2,12},{2,13},{3,6},{3,7},{3,8},{3,9},{3,10},{4,7},{4,9},{4,11},{4,12},{5,7},{5,8},{5,10},{5,13},{6,8},{6,9},{6,12},{7,8},{7,9},{8,11},{9,13}}

Cousin 180: {{1,6},{1,9},{1,10},{1,11},{2,5},{2,9},{2,12},{2,13},{3,6},{3,7},{3,8},{3,9},{3,10},{4,7},{4,9},{4,11},{4,12},{5,7},{5,8},{5,9},{5,10},{6,8},{6,9},{6,12},{7,9},{7,13},{8,11},{8,13}}

Cousin 181: {{1,6},{1,9},{1,10},{1,11},{2,5},{2,8},{2,12},{2,13},{3,6},{3,7},{3,8},{3,9},{3,10},{4,7},{4,9},{4,11},{4,12},{5,7},{5,8},{5,9},{5,10},{6,8},{6,9},{6,12},{7,8},{7,13},{8,11},{9,13}}

Cousin 182: {{1,6},{1,9},{1,10},{1,11},{2,5},{2,7},{2,8},{2,9},{2,12},{3,7},{3,9},{3,10},{3,13},{4,7},{4,9},{4,11},{4,12},{5,7},{5,8},{5,9},{5,10},{6,9},{6,12},{6,13},{7,8},{7,9},{8,11},{8,13}}

Cousin 183: {{1,6},{1,9},{1,10},{1,11},{2,5},{2,7},{2,8},{2,9},{2,12},{3,7},{3,8},{3,10},{3,13},{4,7},{4,9},{4,11},{4,12},{5,7},{5,8},{5,9},{5,10},{6,8},{6,12},{6,13},{7,8},{7,9},{8,11},{9,13}}

Cousin 184: {{1,6},{1,9},{1,10},{1,11},{2,5},{2,7},{2,8},{2,9},{2,12},{3,6},{3,9},{3,10},{3,13},{4,7},{4,9},{4,11},{4,12},{5,7},{5,8},{5,9},{5,10},{6,8},{6,9},{6,12},{7,9},{7,13},{8,11},{8,13}}

Cousin 185: {{1,6},{1,9},{1,10},{1,11},{2,5},{2,7},{2,8},{2,9},{2,12},{3,6},{3,8},{3,10},{3,13},{4,7},{4,9},{4,11},{4,12},{5,7},{5,8},{5,9},{5,10},{6,8},{6,9},{6,12},{7,8},{7,13},{8,11},{9,13}}

Cousin 186: {{1,6},{1,9},{1,10},{1,11},{2,5},{2,7},{2,8},{2,9},{2,12},{3,6},{3,7},{3,8},{3,9},{3,10},{4,11},{4,12},{4,13},{5,7},{5,8},{5,9},{5,10},{6,8},{6,9},{6,12},{7,8},{7,13},{8,11},{9,13}}

Cousin 187: {{1,6},{1,9},{1,10},{1,11},{2,5},{2,7},{2,8},{2,9},{2,12},{3,6},{3,7},{3,8},{3,9},{3,10},{4,7},{4,9},{4,11},{4,12},{5,9},{5,10},{5,13},{6,8},{6,9},{6,12},{7,9},{7,13},{8,11},{8,13}}

Cousin 188: {{1,6},{1,9},{1,10},{1,11},{2,5},{2,7},{2,8},{2,9},{2,12},{3,6},{3,7},{3,8},{3,9},{3,10},{4,7},{4,9},{4,11},{4,12},{5,8},{5,10},{5,13},{6,8},{6,9},{6,12},{7,8},{7,13},{8,11},{9,13}}

Cousin 189: {{1,6},{1,9},{1,10},{1,11},{2,5},{2,9},{2,12},{2,13},{3,6},{3,7},{3,8},{3,9},{3,10},{4,6},{4,9},{4,11},{4,12},{5,7},{5,8},{5,9},{5,10},{6,9},{6,13},{7,8},{7,9},{7,12},{8,11},{8,13}}

Cousin 190: {{1,6},{1,9},{1,10},{1,11},{2,5},{2,8},{2,12},{2,13},{3,6},{3,7},{3,8},{3,9},{3,10},{4,6},{4,9},{4,11},{4,12},{5,7},{5,8},{5,9},{5,10},{6,8},{6,13},{7,8},{7,9},{7,12},{8,11},{9,13}}

Cousin 191: {{1,6},{1,9},{1,10},{1,11},{2,5},{2,6},{2,8},{2,9},{2,12},{3,6},{3,7},{3,8},{3,9},{3,10},{4,6},{4,9},{4,11},{4,12},{5,9},{5,10},{5,13},{6,8},{6,9},{7,9},{7,12},{7,13},{8,11},{8,13}}

Cousin 192: {{1,6},{1,9},{1,10},{1,11},{2,5},{2,6},{2,8},{2,9},{2,12},{3,6},{3,7},{3,8},{3,9},{3,10},{4,6},{4,9},{4,11},{4,12},{5,8},{5,10},{5,13},{6,8},{6,9},{7,8},{7,12},{7,13},{8,11},{9,13}}

Cousin 193: {{1,6},{1,9},{1,10},{1,11},{2,6},{2,7},{2,12},{2,13},{3,6},{3,7},{3,8},{3,9},{3,10},{4,6},{4,7},{4,11},{4,12},{5,7},{5,9},{5,10},{5,13},{6,8},{6,9},{7,8},{7,9},{8,11},{8,13},{9,12}}

Cousin 194: {{1,6},{1,9},{1,10},{1,11},{2,5},{2,7},{2,12},{2,13},{3,6},{3,7},{3,8},{3,9},{3,10},{4,6},{4,7},{4,11},{4,12},{5,7},{5,8},{5,9},{5,10},{6,9},{6,13},{7,8},{7,9},{8,11},{8,13},{9,12}}

Cousin 195: {{1,6},{1,9},{1,10},{1,11},{2,5},{2,6},{2,12},{2,13},{3,6},{3,7},{3,8},{3,9},{3,10},{4,6},{4,7},{4,11},{4,12},{5,7},{5,8},{5,9},{5,10},{6,8},{6,9},{7,9},{7,13},{8,11},{8,13},{9,12}}

Cousin 196: {{1,6},{1,9},{1,10},{1,11},{2,5},{2,6},{2,7},{2,8},{2,12},{3,7},{3,9},{3,10},{3,13},{4,6},{4,7},{4,11},{4,12},{5,7},{5,8},{5,9},{5,10},{6,9},{6,13},{7,8},{7,9},{8,11},{8,13},{9,12}}

Cousin 197: {{1,6},{1,9},{1,10},{1,11},{2,5},{2,6},{2,7},{2,8},{2,12},{3,7},{3,8},{3,10},{3,13},{4,6},{4,7},{4,11},{4,12},{5,7},{5,8},{5,9},{5,10},{6,8},{6,13},{7,8},{7,9},{8,11},{9,12},{9,13}}

Cousin 198: {{1,6},{1,9},{1,10},{1,11},{2,5},{2,6},{2,7},{2,8},{2,12},{3,6},{3,9},{3,10},{3,13},{4,6},{4,7},{4,11},{4,12},{5,7},{5,8},{5,9},{5,10},{6,8},{6,9},{7,9},{7,13},{8,11},{8,13},{9,12}}

Cousin 199: {{1,6},{1,9},{1,10},{1,11},{2,5},{2,6},{2,7},{2,8},{2,12},{3,6},{3,8},{3,10},{3,13},{4,6},{4,7},{4,11},{4,12},{5,7},{5,8},{5,9},{5,10},{6,8},{6,9},{7,8},{7,13},{8,11},{9,12},{9,13}}

Cousin 200: {{1,6},{1,9},{1,10},{1,11},{2,5},{2,6},{2,7},{2,8},{2,12},{3,6},{3,7},{3,8},{3,9},{3,10},{4,6},{4,7},{4,11},{4,12},{5,9},{5,10},{5,13},{6,8},{6,9},{7,9},{7,13},{8,11},{8,13},{9,12}}

<http://faculty.oxy.edu/rnaimi/CV/publications/many-appendix/combined.htm> Page 22 of 126

{7,12},{8,11},{8,12},{9,13}}

Cousin 227: {{1,6},{1,9},{1,10},{1,11},{2,4},{2,5},{2,6},{2,9},{2,12},{3,6},{3,8},{3,10},{3,13},{4,6},{4,7},{4,9},{4,11},{5,7},{5,8},{5,9},{5,10},{6,8},{6,9},{7,12},{7,13},{8,11},{8,12},{9,13}}

Cousin 228: {{1,6},{1,9},{1,10},{1,11},{2,4},{2,5},{2,6},{2,9},{2,12},{3,6},{3,7},{3,8},{3,9},{3,10},{4,7},{4,11},{4,13},{5,7},{5,8},{5,9},{5,10},{6,8},{6,13},{7,9},{7,12},{8,11},{8,12},{9,13}}

Cousin 229: {{1,6},{1,9},{1,10},{1,11},{2,4},{2,5},{2,6},{2,9},{2,12},{3,6},{3,7},{3,8},{3,9},{3,10},{4,6},{4,11},{4,13},{5,7},{5,8},{5,9},{5,10},{6,8},{6,9},{7,12},{7,13},{8,11},{8,12},{9,13}}

Cousin 230: {{1,6},{1,9},{1,10},{1,11},{2,4},{2,5},{2,6},{2,9},{2,12},{3,6},{3,7},{3,8},{3,9},{3,10},{4,6},{4,7},{4,9},{4,11},{5,8},{5,10},{5,13},{6,8},{6,9},{7,12},{7,13},{8,11},{8,12},{9,13}}

Cousin 231: {{1,6},{1,9},{1,10},{1,11},{2,4},{2,5},{2,6},{2,8},{2,12},{3,7},{3,9},{3,10},{3,13},{4,6},{4,7},{4,9},{4,11},{5,7},{5,8},{5,9},{5,10},{6,9},{6,13},{7,8},{7,12},{8,11},{8,13},{9,12}}

Cousin 232: {{1,6},{1,9},{1,10},{1,11},{2,4},{2,5},{2,6},{2,8},{2,12},{3,7},{3,8},{3,10},{3,13},{4,6},{4,7},{4,9},{4,11},{5,7},{5,8},{5,9},{5,10},{6,8},{6,13},{7,8},{7,12},{8,11},{9,12},{9,13}}

Cousin 233: {{1,6},{1,9},{1,10},{1,11},{2,4},{2,5},{2,6},{2,8},{2,12},{3,6},{3,9},{3,10},{3,13},{4,6},{4,7},{4,9},{4,11},{5,7},{5,8},{5,9},{5,10},{6,8},{6,9},{7,12},{7,13},{8,11},{8,13},{9,12}}

Cousin 234: {{1,6},{1,9},{1,10},{1,11},{2,4},{2,5},{2,6},{2,8},{2,12},{3,6},{3,7},{3,8},{3,9},{3,10},{4,7},{4,11},{4,13},{5,7},{5,8},{5,9},{5,10},{6,8},{6,13},{7,8},{7,12},{8,11},{9,12},{9,13}}

Cousin 235: {{1,6},{1,9},{1,10},{1,11},{2,4},{2,5},{2,6},{2,8},{2,12},{3,6},{3,7},{3,8},{3,9},{3,10},{4,6},{4,7},{4,9},{4,11},{5,9},{5,10},{5,13},{6,8},{6,9},{7,12},{7,13},{8,11},{8,13},{9,12}}

Cousin 236: {{1,6},{1,9},{1,10},{1,11},{2,4},{2,5},{2,6},{2,7},{2,8},{2,9},{3,10},{3,12},{3,13},{4,6},{4,7},{4,9},{4,11},{5,7},{5,8},{5,9},{5,10},{6,9},{6,12},{7,8},{7,13},{8,11},{8,12},{9,13}}

Cousin 237: {{1,6},{1,9},{1,10},{1,11},{2,4},{2,5},{2,6},{2,7},{2,8},{2,9},{3,7},{3,9},{3,10},{3,12},{4,7},{4,11},{4,13},{5,7},{5,8},{5,9},{5,10},{6,12},{6,13},{7,8},{7,9},{8,11},{8,12},{9,13}}

Cousin 238: {{1,6},{1,9},{1,10},{1,11},{2,4},{2,5},{2,6},{2,7},{2,8},{2,9},{3,7},{3,9},{3,10},{3,12},{4,6},{4,11},{4,13},{5,7},{5,8},{5,9},{5,10},{6,9},{6,12},{7,8},{7,13},{8,11},{8,12},{9,13}}

Cousin 239: {{1,6},{1,9},{1,10},{1,11},{2,4},{2,5},{2,6},{2,7},{2,8},{2,9},{3,7},{3,9},{3,10},{3,12},{4,6},{4,7},{4,9},{4,11},{5,9},{5,10},{5,13},{6,9},{6,12},{7,9},{7,13},{8,11},{8,12},{8,13}}

Cousin 240: {{1,6},{1,9},{1,10},{1,11},{2,4},{2,5},{2,6},{2,7},{2,8},{2,9},{3,7},{3,9},{3,10},{3,12},{4,6},{4,7},{4,9},{4,11},{5,8},{5,10},{5,13},{6,9},{6,12},{7,8},{7,13},{8,11},{8,12},{9,13}}

Cousin 241: {{1,6},{1,9},{1,10},{1,11},{2,4},{2,5},{2,6},{2,7},{2,8},{2,9},{3,10},{3,12},{3,13},{4,6},{4,7},{4,9},{4,11},{5,7},{5,8},{5,9},{5,10},{6,8},{6,12},{7,9},{7,13},{8,11},{8,13},{9,12}}

Cousin 242: {{1,6},{1,9},{1,10},{1,11},{2,4},{2,5},{2,6},{2,7},{2,8},{2,9},{3,7},{3,8},{3,10},{3,12},{4,6},{4,11},{4,13},{5,7},{5,8},{5,9},{5,10},{6,8},{6,12},{7,8},{7,13},{8,11},{9,12},{9,13}}

Cousin 243: {{1,6},{1,9},{1,10},{1,11},{2,4},{2,5},{2,6},{2,7},{2,8},{2,9},{3,7},{3,8},{3,10},{3,12},{4,6},{4,7},{4,9},{4,11},{5,9},{5,10},{5,13},{6,8},{6,12},{7,9},{7,13},{8,11},{8,13},{9,12}}

Cousin 244: {{1,6},{1,9},{1,10},{1,11},{2,4},{2,5},{2,6},{2,7},{2,8},{2,9},{3,7},{3,8},{3,10},{3,12},{4,6},{4,7},{4,9},{4,11},{5,8},{5,10},{5,13},{6,8},{6,12},{7,8},{7,13},{8,11},{9,12},{9,13}}

Cousin 245: {{1,6},{1,9},{1,10},{1,11},{2,4},{2,5},{2,6},{2,7},{2,8},{2,9},{3,6},{3,9},{3,10},{3,12},{4,7},{4,11},{4,13},{5,7},{5,8},{5,9},{5,10},{6,8},{6,13},{7,9},{7,12},{8,11},{8,12},{9,13}}

Cousin 246: {{1,6},{1,9},{1,10},{1,11},{2,4},{2,5},{2,6},{2,7},{2,8},{2,9},{3,6},{3,9},{3,10},{3,12},{4,6},{4,11},{4,13},{5,7},{5,8},{5,9},{5,10},{6,8},{6,9},{7,12},{7,13},{8,11},{8,12},{9,13}}

Cousin 247: {{1,6},{1,9},{1,10},{1,11},{2,4},{2,5},{2,6},{2,7},{2,8},{2,9},{3,6},{3,9},{3,10},{3,12},{4,6},{4,7},{4,9},{4,11},{5,8},{5,10},{5,13},{6,8},{6,9},{7,12},{7,13},{8,11},{8,12},{9,13}}

Cousin 248: {{1,6},{1,9},{1,10},{1,11},{2,4},{2,5},{2,6},{2,7},{2,8},{2,9},{3,6},{3,8},{3,10},{3,12},{4,7},{4,11},{4,13},{5,7},{5,8},{5,9},{5,10},{6,8},{6,13},{7,8},{7,12},{8,11},{9,12},{9,13}}

Cousin 249: {{1,6},{1,9},{1,10},{1,11},{2,4},{2,5},{2,6},{2,7},{2,8},{2,9},{3,6},{3,8},{3,10},{3,12},{4,6},{4,7},{4,9},{4,11},{5,9},{5,10},{5,13},{6,8},{6,9},{7,12},{7,13},{8,11},{8,13},{9,12}}

Cousin 250: {{1,6},{1,9},{1,10},{1,11},{2,4},{2,5},{2,6},{2,7},{2,8},{2,9},{3,6},{3,7},{3,8},{3,9},{3,10},{4,7},{4,11},{4,12},{5,9},{5,10},{5,13},{6,8},{6,12},{7,9},{7,13},{8,11},{8,13},{9,12}}

Cousin 251: {{1,6},{1,9},{1,10},{1,11},{2,4},{2,5},{2,6},{2,7},{2,8},{2,9},{3,6},{3,7},{3,8},{3,9},{3,10},{4,7},{4,11},{4,12},{5,8},{5,10},{5,13},{6,8},{6,12},{7,8},{7,13},{8,11},{9,12},{9,13}}

Cousin 252: {{1,6},{1,9},{1,10},{1,11},{2,4},{2,5},{2,6},{2,7},{2,8},{2,9},{3,6},{3,7},{3,8},{3,9},{3,10},{4,6},{4,11},{4,12},{5,9},{5,10},{5,13},{6,8},{6,9},{7,12},{7,13},{8,11},{8,13},{9,12}}

Cousin 253: {{1,4},{1,9},{1,10},{1,11},{2,5},{2,9},{2,12},{2,13},{3,6},{3,7},{3,8},{3,9},{3,10},{4,7},{4,8},{4,9},{4,12},{5,7},{5,8},{5,9},{5,10},{6,9},{6,11},{6,12},{7,9},{7,13},{8,11},{8,13}}

Cousin 254: {{1,4},{1,9},{1,10},{1,11},{2,5},{2,8},{2,12},{2,13},{3,6},{3,7},{3,8},{3,9},{3,10},{4,7},{4,8},{4,9},{4,12},{5,7},{5,8},{5,9},{5,10},{6,9},{6,11},{6,12},{7,8},{7,13},{8,11},{9,13}}

Cousin 255: {{1,4},{1,9},{1,10},{1,11},{2,5},{2,7},{2,8},{2,9},{2,12},{3,6},{3,9},{3,10},{3,13},{4,7},{4,8},{4,9},{4,12},{5,7},{5,8},{5,9},{5,10},{6,9},{6,11},{6,12},{7,9},{7,13},{8,11},{8,13}}

Cousin 256: {{1,4},{1,9},{1,10},{1,11},{2,5},{2,7},{2,8},{2,9},{2,12},{3,6},{3,8},{3,10},{3,13},{4,7},{4,8},{4,9},{4,12},{5,7},{5,8},{5,9},{5,10},{6,9},{6,11},{6,12},{7,8},{7,13},{8,11},{9,13}}

Cousin 257: {{1,4},{1,9},{1,10},{1,11},{2,5},{2,8},{2,12},{2,13},{3,6},{3,7},{3,8},{3,9},{3,10},{4,6},{4,8},{4,9},{4,12},{5,7},{5,8},{5,9},{5,10},{6,11},{6,13},{7,8},{7,9},{7,12},{8,11},{9,13}}

Cousin 258: {{1,4},{1,9},{1,10},{1,11},{2,5},{2,6},{2,8},{2,9},{2,12},{3,7},{3,8},{3,10},{3,13},{4,6},{4,8},{4,9},{4,12},{5,7},{5,8},{5,9},{5,10},{6,11},{6,13},{7,8},{7,9},{7,12},{8,11},{9,13}}

Cousin 259: {{1,4},{1,9},{1,10},{1,11},{2,5},{2,6},{2,8},{2,9},{2,12},{3,6},{3,7},{3,8},{3,9},{3,10},{4,8},{4,12},{4,13},{5,7},{5,8},{5,9},{5,10},{6,11},{6,13},{7,8},{7,9},{7,12},{8,11},{9,13}}

Cousin 260: {{1,4},{1,9},{1,10},{1,11},{2,5},{2,7},{2,12},{2,13},{3,6},{3,7},{3,8},{3,9},{3,10},{4,6},{4,7},{4,9},{4,12},{5,7},{5,8},{5,9},{5,10},{6,11},{6,13},{7,8},{7,9},{8,11},{8,12},{9,13}}

Cousin 261: {{1,4},{1,9},{1,10},{1,11},{2,5},{2,6},{2,12},{2,13},{3,6},{3,7},{3,8},{3,9},{3,10},{4,6},{4,7},{4,9},{4,12},{5,7},{5,8},{5,9},{5,10},{6,9},{6,11},{7,8},{7,13},{8,11},{8,12},{9,13}}

Cousin 262: {{1,4},{1,9},{1,10},{1,11},{2,5},{2,6},{2,7},{2,9},{2,12},{3,7},{3,8},{3,10},{3,13},{4,6},{4,7},{4,9},{4,12},{5,7},{5,8},{5,9},{5,10},{6,11},{6,13},{7,8},{7,9},{8,11},{8,12},{9,13}}

Cousin 263: {{1,4},{1,9},{1,10},{1,11},{2,5},{2,6},{2,7},{2,9},{2,12},{3,6},{3,9},{3,10},{3,13},{4,6},{4,7},{4,9},{4,12},{5,7},{5,8},{5,9},{5,10},{6,9},{6,11},{7,9},{7,13},{8,11},{8,12},{8,13}}

Cousin 264: {{1,4},{1,9},{1,10},{1,11},{2,5},{2,6},{2,7},{2,9},{2,12},{3,6},{3,8},{3,10},{3,13},{4,6},{4,7},{4,9},{4,12},{5,7},{5,8},{5,9},{5,10},{6,9},{6,11},{7,8},{7,13},{8,11},{8,12},{9,13}}

Cousin 265: {{1,4},{1,9},{1,10},{1,11},{2,5},{2,6},{2,7},{2,9},{2,12},{3,6},{3,7},{3,8},{3,9},{3,10},{4,7},{4,12},{4,13},{5,7},{5,8},{5,9},{5,10},{6,11},{6,13},{7,8},{7,9},{8,11},{8,12},{9,13}}

Cousin 266: {{1,4},{1,9},{1,10},{1,11},{2,5},{2,6},{2,7},{2,9},{2,12},{3,6},{3,7},{3,8},{3,9},{3,10},{4,6},{4,12},{4,13},{5,7},{5,8},{5,9},{5,10},{6,9},{6,11},{7,8},{7,13},{8,11},{8,12},{9,13}}

Cousin 267: {{1,4},{1,9},{1,10},{1,11},{2,5},{2,6},{2,7},{2,9},{2,12},{3,6},{3,7},{3,8},{3,9},{3,10},{4,6},{4,7},{4,9},{4,12},{5,9},{5,10},{5,13},{6,9},{6,11},{7,9},{7,13},{8,11},{8,12},{8,13}}

Cousin 268: {{1,4},{1,9},{1,10},{1,11},{2,5},{2,6},{2,7},{2,9},{2,12},{3,6},{3,7},{3,8},{3,9},{3,10},{4,6},{4,7},{4,9},{4,12},{5,8},{5,10},{5,13},{6,9},{6,11},{7,8},{7,13},{8,11},{8,12},{9,13}}

Cousin 269: {{1,4},{1,9},{1,10},{1,11},{2,5},{2,6},{2,12},{2,13},{3,6},{3,7},{3,8},{3,9},{3,10},{4,6},{4,7},{4,8},{4,12},{5,7},{5,8},{5,9},{5,10},{6,9},{6,11},{7,9},{7,13},{8,11},{8,13},{9,12}}

Cousin 270: {{1,4},{1,9},{1,10},{1,11},{2,5},{2,6},{2,7},{2,8},{2,12},{3,7},{3,8},{3,10},{3,13},{4,6},{4,7},{4,8},{4,12},{5,7},{5,8},{5,9},{5,10},{6,11},{6,13},{7,8},{7,9},{8,11},{9,12},{9,13}}

Cousin 271: {{1,4},{1,9},{1,10},{1,11},{2,5},{2,6},{2,7},{2,8},{2,12},{3,6},{3,9},{3,10},{3,13},{4,6},{4,7},{4,8},{4,12},{5,7},{5,8},{5,9},{5,10},{6,9},{6,11},{7,9},{7,13},{8,11},{8,13},{9,12}}

Cousin 272: {{1,4},{1,9},{1,10},{1,11},{2,5},{2,6},{2,7},{2,8},{2,12},{3,6},{3,8},{3,10},{3,13},{4,6},{4,7},{4,8},{4,12},{5,7},{5,8},{5,9},{5,10},{6,9},{6,11},{7,8},{7,13},{8,11},{9,12},{9,13}}

Cousin 273: {{1,4},{1,9},{1,10},{1,11},{2,5},{2,6},{2,7},{2,8},{2,12},{3,6},{3,7},{3,8},{3,9},{3,10},{4,6},{4,12},{4,13},{5,7},{5,8},{5,9},{5,10},{6,9},{6,11},{7,9},{7,13},{8,11},{8,13},{9,12}}

Cousin 274: {{1,4},{1,9},{1,10},{1,11},{2,5},{2,6},{2,7},{2,8},{2,12},{3,6},{3,7},{3,8},{3,9},{3,10},{4,6},{4,7},{4,8},{4,12},{5,9},{5,10},{5,13},{6,9},{6,11},{7,9},{7,13},{8,11},{8,13},{9,12}}

Cousin 275: {{1,4},{1,9},{1,10},{1,11},{2,4},{2,5},{2,12},{2,13},{3,6},{3,7},{3,8},{3,9},{3,10},{4,6},{4,7},{4,8},{4,9},{5,7},{5,8},{5,9},{5,10},{6,11},{6,12},{7,9},{7,13},{8,11},{8,13},{9,12}}

Cousin 276: {{1,4},{1,9},{1,10},{1,11},{2,4},{2,5},{2,7},{2,8},{2,12},{3,6},{3,9},{3,10},{3,13},{4,6},{4,7},{4,8},{4,9},{5,7},{5,8},{5,9},{5,10},{6,11},{6,12},{7,9},{7,13},{8,11},{8,13},{9,12}}



<http://faculty.oxy.edu/rnaimi/CV/publications/many-appendix/combined.htm> Page 25 of 126

{7,12},{7,13},{8,12},{9,13}}

Cousin 303: {{1,4},{1,6},{1,8},{1,9},{1,10},{2,5},{2,7},{2,11},{2,12},{3,7},{3,9},{3,10},{3,13},{4,6},{4,7},{4,9},{4,11},{5,7},{5,8},{5,9},{5,10},{6,12},{6,13},{7,8},{7,9},{8,11},{8,13},{9,12}}

Cousin 304: {{1,4},{1,6},{1,8},{1,9},{1,10},{2,5},{2,7},{2,11},{2,12},{3,6},{3,9},{3,10},{3,13},{4,6},{4,7},{4,9},{4,11},{5,7},{5,8},{5,9},{5,10},{6,8},{6,12},{7,9},{7,13},{8,11},{8,13},{9,12}}

Cousin 305: {{1,4},{1,6},{1,8},{1,9},{1,10},{2,5},{2,7},{2,11},{2,12},{3,6},{3,8},{3,10},{3,13},{4,6},{4,7},{4,9},{4,11},{5,7},{5,8},{5,9},{5,10},{6,8},{6,12},{7,8},{7,13},{8,11},{9,12},{9,13}}

Cousin 306: {{1,4},{1,6},{1,8},{1,9},{1,10},{2,5},{2,7},{2,11},{2,12},{3,6},{3,7},{3,8},{3,9},{3,10},{4,6},{4,11},{4,13},{5,7},{5,8},{5,9},{5,10},{6,8},{6,12},{7,8},{7,13},{8,11},{9,12},{9,13}}

Cousin 307: {{1,4},{1,6},{1,8},{1,9},{1,10},{2,5},{2,6},{2,11},{2,12},{3,7},{3,9},{3,10},{3,13},{4,6},{4,7},{4,9},{4,11},{5,7},{5,8},{5,9},{5,10},{6,9},{6,13},{7,8},{7,12},{8,11},{8,13},{9,12}}

Cousin 308: {{1,4},{1,6},{1,8},{1,9},{1,10},{2,5},{2,6},{2,11},{2,12},{3,7},{3,8},{3,10},{3,13},{4,6},{4,7},{4,9},{4,11},{5,7},{5,8},{5,9},{5,10},{6,8},{6,13},{7,8},{7,12},{8,11},{9,12},{9,13}}

Cousin 309: {{1,4},{1,6},{1,8},{1,9},{1,10},{2,5},{2,6},{2,11},{2,12},{3,6},{3,9},{3,10},{3,13},{4,6},{4,7},{4,9},{4,11},{5,7},{5,8},{5,9},{5,10},{6,8},{6,9},{7,12},{7,13},{8,11},{8,13},{9,12}}

Cousin 310: {{1,4},{1,6},{1,8},{1,9},{1,10},{2,5},{2,6},{2,11},{2,12},{3,6},{3,7},{3,8},{3,9},{3,10},{4,7},{4,11},{4,13},{5,7},{5,8},{5,9},{5,10},{6,8},{6,13},{7,8},{7,12},{8,11},{9,12},{9,13}}

Cousin 311: {{1,4},{1,6},{1,8},{1,9},{1,10},{2,5},{2,6},{2,7},{2,9},{2,11},{3,10},{3,12},{3,13},{4,6},{4,7},{4,9},{4,11},{5,7},{5,8},{5,9},{5,10},{6,9},{6,12},{7,8},{7,13},{8,11},{8,12},{9,13}}

Cousin 312: {{1,4},{1,6},{1,8},{1,9},{1,10},{2,4},{2,5},{2,11},{2,12},{3,7},{3,8},{3,10},{3,13},{4,6},{4,7},{4,8},{4,9},{5,7},{5,8},{5,9},{5,10},{6,11},{6,13},{7,8},{7,12},{8,11},{9,12},{9,13}}

Cousin 313: {{1,4},{1,6},{1,8},{1,9},{1,10},{2,4},{2,5},{2,11},{2,12},{3,6},{3,9},{3,10},{3,13},{4,6},{4,7},{4,8},{4,9},{5,7},{5,8},{5,9},{5,10},{6,9},{6,11},{7,12},{7,13},{8,11},{8,13},{9,12}}

Cousin 314: {{1,4},{1,6},{1,8},{1,9},{1,10},{2,4},{2,5},{2,11},{2,12},{3,6},{3,7},{3,8},{3,9},{3,10},{4,7},{4,8},{4,13},{5,7},{5,8},{5,9},{5,10},{6,11},{6,13},{7,8},{7,12},{8,11},{9,12},{9,13}}

Cousin 315: {{1,4},{1,6},{1,8},{1,9},{1,10},{2,4},{2,5},{2,11},{2,12},{3,6},{3,7},{3,8},{3,9},{3,10},{4,6},{4,9},{4,13},{5,7},{5,8},{5,9},{5,10},{6,9},{6,11},{7,12},{7,13},{8,11},{8,13},{9,12}}

Cousin 316: {{1,4},{1,6},{1,8},{1,9},{1,10},{2,4},{2,5},{2,7},{2,9},{2,11},{3,10},{3,12},{3,13},{4,6},{4,7},{4,8},{4,9},{5,7},{5,8},{5,9},{5,10},{6,11},{6,12},{7,9},{7,13},{8,11},{8,13},{9,12}}

Cousin 317: {{1,4},{1,6},{1,8},{1,9},{1,10},{2,4},{2,5},{2,7},{2,9},{2,11},{3,7},{3,8},{3,10},{3,12},{4,6},{4,9},{4,13},{5,7},{5,8},{5,9},{5,10},{6,11},{6,12},{7,9},{7,13},{8,11},{8,13},{9,12}}

Cousin 318: {{1,4},{1,6},{1,8},{1,9},{1,10},{2,4},{2,5},{2,7},{2,9},{2,11},{3,7},{3,8},{3,10},{3,12},{4,6},{4,8},{4,13},{5,7},{5,8},{5,9},{5,10},{6,11},{6,12},{7,8},{7,13},{8,11},{9,12},{9,13}}

Cousin 319: {{1,4},{1,6},{1,8},{1,9},{1,10},{2,4},{2,5},{2,7},{2,9},{2,11},{3,6},{3,9},{3,10},{3,12},{4,7},{4,8},{4,13},{5,7},{5,8},{5,9},{5,10},{6,11},{6,13},{7,9},{7,12},{8,11},{8,12},{9,13}}

Cousin 320: {{1,4},{1,6},{1,8},{1,9},{1,10},{2,4},{2,5},{2,7},{2,9},{2,11},{3,6},{3,8},{3,10},{3,12},{4,7},{4,8},{4,13},{5,7},{5,8},{5,9},{5,10},{6,11},{6,13},{7,8},{7,12},{8,11},{9,12},{9,13}}

Cousin 321: {{1,4},{1,6},{1,8},{1,9},{1,10},{2,4},{2,5},{2,6},{2,9},{2,11},{3,10},{3,12},{3,13},{4,6},{4,7},{4,8},{4,9},{5,7},{5,8},{5,9},{5,10},{6,9},{6,12},{7,11},{7,13},{8,11},{8,12},{9,13}}

Cousin 322: {{1,4},{1,6},{1,8},{1,9},{1,10},{2,4},{2,5},{2,6},{2,9},{2,11},{3,7},{3,9},{3,10},{3,12},{4,7},{4,8},{4,13},{5,7},{5,8},{5,9},{5,10},{6,12},{6,13},{7,9},{7,11},{8,11},{8,12},{9,13}}

Cousin 323: {{1,4},{1,6},{1,8},{1,9},{1,10},{2,4},{2,5},{2,6},{2,9},{2,11},{3,7},{3,8},{3,10},{3,12},{4,7},{4,9},{4,13},{5,7},{5,8},{5,9},{5,10},{6,12},{6,13},{7,9},{7,11},{8,11},{8,13},{9,12}}

Cousin 324: {{1,4},{1,6},{1,8},{1,9},{1,10},{2,4},{2,5},{2,6},{2,7},{2,8},{2,9},{3,7},{3,9},{3,10},{3,11},{4,6},{4,7},{4,8},{4,9},{5,7},{5,8},{5,9},{5,10},{6,9},{6,11},{7,8},{8,11},{10,11}}

Cousin 325: {{1,5},{1,6},{1,10},{1,11},{2,6},{2,7},{2,12},{2,13},{3,5},{3,6},{3,7},{3,9},{3,10},{4,6},{4,7},{4,11},{4,12},{5,7},{5,8},{5,13},{6,8},{6,9},{7,8},{7,9},{8,10},{8,12},{9,11},{9,13}}

Cousin 326: {{1,5},{1,6},{1,10},{1,11},{2,5},{2,7},{2,12},{2,13},{3,5},{3,6},{3,7},{3,9},{3,10},{4,6},{4,7},{4,11},{4,12},{5,7},{5,8},{5,9},{6,8},{6,13},{7,8},{7,9},{8,10},{8,12},{9,11},{9,13}}

Cousin 327: {{1,5},{1,6},{1,10},{1,11},{2,5},{2,6},{2,12},{2,13},{3,5},{3,6},{3,7},{3,9},{3,10},{4,6},{4,7},{4,11},{4,12},{5,7},{5,8},{5,9},{6,8},{6,9},{7,8},{7,13},{8,10},{8,12},{9,11},{9,13}}

Cousin 328: {{1,5},{1,6},{1,10},{1,11},{2,5},{2,6},{2,7},{2,9},{2,12},{3,5},{3,6},{3,7},{3,9},{3,10},{4,6},{4,7},{4,11},{4,12},{5,9},{5,13},{6,8},{6,9},{7,9},{7,13},{8,10},{8,12},{8,13},{9,11}}

Cousin 329: {{1,5},{1,6},{1,10},{1,11},{2,5},{2,6},{2,7},{2,9},{2,12},{3,5},{3,6},{3,7},{3,9},{3,10},{4,6},{4,7},{4,11},{4,12},{5,8},{5,13},{6,8},{6,9},{7,8},{7,13},{8,10},{8,12},{9,11},{9,13}}

Cousin 330: {{1,5},{1,6},{1,10},{1,11},{2,4},{2,7},{2,12},{2,13},{3,5},{3,6},{3,7},{3,9},{3,10},{4,6},{4,7},{4,8},{4,11},{5,7},{5,9},{5,12},{6,8},{6,13},{7,8},{7,9},{8,10},{8,12},{9,11},{9,13}}

Cousin 331: {{1,5},{1,6},{1,10},{1,11},{2,4},{2,6},{2,12},{2,13},{3,5},{3,6},{3,7},{3,9},{3,10},{4,6},{4,7},{4,8},{4,11},{5,7},{5,9},{5,12},{6,8},{6,9},{7,8},{7,13},{8,10},{8,12},{9,11},{9,13}}

Cousin 332: {{1,5},{1,6},{1,10},{1,11},{2,4},{2,6},{2,7},{2,9},{2,12},{3,6},{3,7},{3,10},{3,13},{4,6},{4,7},{4,8},{4,11},{5,7},{5,12},{5,13},{6,8},{6,9},{7,8},{7,9},{8,10},{8,12},{9,11},{9,13}}

Cousin 333: {{1,5},{1,6},{1,10},{1,11},{2,4},{2,6},{2,7},{2,9},{2,12},{3,5},{3,7},{3,10},{3,13},{4,6},{4,7},{4,8},{4,11},{5,7},{5,9},{5,12},{6,8},{6,13},{7,8},{7,9},{8,10},{8,12},{9,11},{9,13}}

Cousin 334: {{1,5},{1,6},{1,10},{1,11},{2,4},{2,6},{2,7},{2,9},{2,12},{3,5},{3,6},{3,10},{3,13},{4,6},{4,7},{4,8},{4,11},{5,7},{5,9},{5,12},{6,8},{6,9},{7,8},{7,13},{8,10},{8,12},{9,11},{9,13}}

Cousin 335: {{1,5},{1,6},{1,10},{1,11},{2,4},{2,6},{2,7},{2,9},{2,12},{3,5},{3,6},{3,7},{3,9},{3,10},{4,7},{4,11},{4,13},{5,7},{5,9},{5,12},{6,9},{6,13},{7,8},{7,9},{8,10},{8,12},{8,13},{9,11}}

Cousin 336: {{1,5},{1,6},{1,10},{1,11},{2,4},{2,6},{2,7},{2,9},{2,12},{3,5},{3,6},{3,7},{3,9},{3,10},{4,6},{4,11},{4,13},{5,7},{5,9},{5,12},{6,8},{6,9},{7,9},{7,13},{8,10},{8,12},{8,13},{9,11}}

Cousin 337: {{1,5},{1,6},{1,10},{1,11},{2,4},{2,6},{2,7},{2,9},{2,12},{3,5},{3,6},{3,7},{3,9},{3,10},{4,6},{4,7},{4,8},{4,11},{5,12},{5,13},{6,8},{6,9},{7,8},{7,13},{8,10},{8,12},{9,11},{9,13}}

Cousin 338: {{1,5},{1,6},{1,10},{1,11},{2,4},{2,7},{2,12},{2,13},{3,5},{3,6},{3,7},{3,9},{3,10},{4,6},{4,7},{4,8},{4,11},{5,7},{5,8},{5,12},{6,9},{6,13},{7,8},{7,9},{8,10},{8,13},{9,11},{9,12}}

Cousin 339: {{1,5},{1,6},{1,10},{1,11},{2,4},{2,6},{2,12},{2,13},{3,5},{3,6},{3,7},{3,9},{3,10},{4,6},{4,7},{4,8},{4,11},{5,7},{5,8},{5,12},{6,8},{6,9},{7,9},{7,13},{8,10},{8,13},{9,11},{9,12}}

Cousin 340: {{1,5},{1,6},{1,10},{1,11},{2,4},{2,6},{2,7},{2,8},{2,12},{3,5},{3,7},{3,10},{3,13},{4,6},{4,7},{4,8},{4,11},{5,7},{5,8},{5,12},{6,8},{6,13},{7,8},{7,9},{8,10},{9,11},{9,12},{9,13}}

Cousin 341: {{1,5},{1,6},{1,10},{1,11},{2,4},{2,6},{2,7},{2,8},{2,12},{3,5},{3,6},{3,10},{3,13},{4,6},{4,7},{4,8},{4,11},{5,7},{5,8},{5,12},{6,8},{6,9},{7,8},{7,13},{8,10},{9,11},{9,12},{9,13}}

Cousin 342: {{1,5},{1,6},{1,10},{1,11},{2,4},{2,6},{2,7},{2,8},{2,12},{3,5},{3,6},{3,7},{3,9},{3,10},{4,7},{4,11},{4,13},{5,7},{5,8},{5,12},{6,9},{6,13},{7,8},{7,9},{8,10},{8,13},{9,11},{9,12}}

Cousin 343: {{1,5},{1,6},{1,10},{1,11},{2,4},{2,6},{2,7},{2,8},{2,12},{3,5},{3,6},{3,7},{3,9},{3,10},{4,6},{4,11},{4,13},{5,7},{5,8},{5,12},{6,8},{6,9},{7,9},{7,13},{8,10},{8,13},{9,11},{9,12}}

Cousin 344: {{1,5},{1,6},{1,10},{1,11},{2,4},{2,6},{2,7},{2,8},{2,12},{3,5},{3,6},{3,7},{3,9},{3,10},{4,6},{4,7},{4,8},{4,11},{5,12},{5,13},{6,8},{6,9},{7,9},{7,13},{8,10},{8,13},{9,11},{9,12}}

Cousin 345: {{1,5},{1,6},{1,10},{1,11},{2,4},{2,5},{2,12},{2,13},{3,5},{3,6},{3,7},{3,9},{3,10},{4,6},{4,7},{4,8},{4,11},{5,7},{5,8},{5,9},{6,9},{6,12},{7,8},{7,13},{8,10},{8,12},{9,11},{9,13}}

Cousin 346: {{1,5},{1,6},{1,10},{1,11},{2,4},{2,5},{2,7},{2,9},{2,12},{3,6},{3,7},{3,10},{3,13},{4,6},{4,7},{4,8},{4,11},{5,7},{5,8},{5,13},{6,9},{6,12},{7,8},{7,9},{8,10},{8,12},{9,11},{9,13}}

Cousin 347: {{1,5},{1,6},{1,10},{1,11},{2,4},{2,5},{2,7},{2,9},{2,12},{3,5},{3,7},{3,10},{3,13},{4,6},{4,7},{4,8},{4,11},{5,7},{5,8},{5,9},{6,12},{6,13},{7,8},{7,9},{8,10},{8,12},{9,11},{9,13}}

Cousin 348: {{1,5},{1,6},{1,10},{1,11},{2,4},{2,5},{2,7},{2,9},{2,12},{3,5},{3,6},{3,7},{3,9},{3,10},{4,6},{4,11},{4,13},{5,7},{5,8},{5,9},{6,9},{6,12},{7,9},{7,13},{8,10},{8,12},{8,13},{9,11}}

Cousin 349: {{1,5},{1,6},{1,10},{1,11},{2,4},{2,5},{2,7},{2,9},{2,12},{3,5},{3,6},{3,7},{3,9},{3,10},{4,6},{4,7},{4,8},{4,11},{5,9},{5,13},{6,9},{6,12},{7,9},{7,13},{8,10},{8,12},{8,13},{9,11}}

Cousin 350: {{1,5},{1,6},{1,10},{1,11},{2,4},{2,5},{2,7},{2,9},{2,12},{3,5},{3,6},{3,7},{3,9},{3,10},{4,6},{4,7},{4,8},{4,11},{5,8},{5,13},{6,9},{6,12},{7,8},{7,13},{8,10},{8,12},{9,11},{9,13}}

Cousin 351: {{1,5},{1,6},{1,10},{1,11},{2,4},{2,5},{2,12},{2,13},{3,5},{3,6},{3,7},{3,9},{3,10},{4,6},{4,7},{4,8},{4,11},{5,7},{5,8},{5,9},{6,8},{6,12},{7,9},{7,13},{8,10},{8,13},{9,11},{9,12}}

Cousin 352: {{1,5},{1,6},{1,10},{1,11},{2,4},{2,5},{2,7},{2,8},{2,12},{3,6},{3,7},{3,10},{3,13},{4,6},{4,7},{4,8},{4,11},{5,7},{5,8},{5,13},{6,8},{6,12},{7,8},{7,9},{8,10},{9,11},{9,12},{9,13}}

Cousin 353: {{1,5},{1,6},{1,10},{1,11},{2,4},{2,5},{2,7},{2,8},{2,12},{3,5},{3,6},{3,7},{3,9},{3,10},{4,7},{4,11},{4,13},{5,7},{5,8},{5,9},{6,12},{6,13},{7,8},{7,9},{8,10},{8,13},{9,11},{9,12}}

Cousin 354: {{1,5},{1,6},{1,10},{1,11},{2,4},{2,5},{2,7},{2,8},{2,12},{3,5},{3,6},{3,7},{3,9},{3,10},{4,6},{4,11},{4,13},{5,7},{5,8},{5,9},{6,8},{6,12},{7,9},{7,13},{8,10},{8,13},{9,11},{9,12}}

Cousin 355: {{1,5},{1,6},{1,10},{1,11},{2,4},{2,5},{2,7},{2,8},{2,12},{3,5},{3,6},{3,7},{3,9},{3,10},{4,6},{4,7},{4,8},{4,11},{5,9},{5,13},{6,8},{6,12},{7,9},{7,13},{8,10},{8,13},{9,11},{9,12}}

Cousin 356: {{1,5},{1,6},{1,10},{1,11},{2,4},{2,5},{2,7},{2,8},{2,12},{3,5},{3,6},{3,7},{3,9},{3,10},{4,6},{4,7},{4,8},{4,11},{5,8},{5,13},{6,8},{6,12},{7,8},{7,13},{8,10},{9,11},{9,12},{9,13}}

Cousin 357: {{1,5},{1,6},{1,10},{1,11},{2,4},{2,5},{2,6},{2,9},{2,12},{3,6},{3,7},{3,10},{3,13},{4,6},{4,7},{4,8},{4,11},{5,7},{5,8},{5,13},{6,8},{6,9},{7,9},{7,12},{8,10},{8,12},{9,11},{9,13}}

Cousin 358: {{1,5},{1,6},{1,10},{1,11},{2,4},{2,5},{2,6},{2,9},{2,12},{3,5},{3,7},{3,10},{3,13},{4,6},{4,7},{4,8},{4,11},{5,7},{5,8},{5,9},{6,8},{6,13},{7,9},{7,12},{8,10},{8,12},{9,11},{9,13}}

Cousin 359: {{1,5},{1,6},{1,10},{1,11},{2,4},{2,5},{2,6},{2,9},{2,12},{3,5},{3,6},{3,7},{3,9},{3,10},{4,7},{4,11},{4,13},{5,7},{5,8},{5,9},{6,9},{6,13},{7,9},{7,12},{8,10},{8,12},{8,13},{9,11}}

Cousin 360: {{1,5},{1,6},{1,10},{1,11},{2,4},{2,5},{2,6},{2,9},{2,12},{3,5},{3,6},{3,7},{3,9},{3,10},{4,6},{4,7},{4,8},{4,11},{5,8},{5,13},{6,8},{6,9},{7,12},{7,13},{8,10},{8,12},{9,11},{9,13}}

Cousin 361: {{1,5},{1,6},{1,10},{1,11},{2,4},{2,5},{2,6},{2,8},{2,12},{3,6},{3,7},{3,10},{3,13},{4,6},{4,7},{4,8},{4,11},{5,7},{5,8},{5,13},{6,8},{6,9},{7,8},{7,12},{8,10},{9,11},{9,12},{9,13}}

Cousin 362: {{1,5},{1,6},{1,10},{1,11},{2,4},{2,5},{2,6},{2,8},{2,12},{3,5},{3,7},{3,10},{3,13},{4,6},{4,7},{4,8},{4,11},{5,7},{5,8},{5,9},{6,8},{6,13},{7,8},{7,12},{8,10},{9,11},{9,12},{9,13}}

Cousin 363: {{1,5},{1,6},{1,10},{1,11},{2,4},{2,5},{2,6},{2,8},{2,12},{3,5},{3,6},{3,7},{3,9},{3,10},{4,7},{4,11},{4,13},{5,7},{5,8},{5,9},{6,9},{6,13},{7,8},{7,12},{8,10},{8,13},{9,11},{9,12}}

Cousin 364: {{1,5},{1,6},{1,10},{1,11},{2,4},{2,5},{2,6},{2,8},{2,12},{3,5},{3,6},{3,7},{3,9},{3,10},{4,6},{4,11},{4,13},{5,7},{5,8},{5,9},{6,8},{6,9},{7,12},{7,13},{8,10},{8,13},{9,11},{9,12}}

Cousin 365: {{1,5},{1,6},{1,10},{1,11},{2,4},{2,5},{2,6},{2,8},{2,12},{3,5},{3,6},{3,7},{3,9},{3,10},{4,6},{4,7},{4,8},{4,11},{5,9},{5,13},{6,8},{6,9},{7,12},{7,13},{8,10},{8,13},{9,11},{9,12}}

Cousin 366: {{1,5},{1,6},{1,10},{1,11},{2,4},{2,5},{2,6},{2,7},{2,8},{2,9},{3,6},{3,7},{3,10},{3,12},{4,7},{4,11},{4,13},{5,7},{5,8},{5,12},{6,9},{6,13},{7,8},{7,9},{8,10},{8,13},{9,11},{9,12}}

Cousin 367: {{1,5},{1,6},{1,10},{1,11},{2,4},{2,5},{2,6},{2,7},{2,8},{2,9},{3,6},{3,7},{3,10},{3,12},{4,6},{4,11},{4,13},{5,7},{5,8},{5,12},{6,8},{6,9},{7,9},{7,13},{8,10},{8,13},{9,11},{9,12}}

Cousin 368: {{1,5},{1,6},{1,10},{1,11},{2,4},{2,5},{2,6},{2,7},{2,8},{2,9},{3,6},{3,7},{3,10},{3,12},{4,6},{4,7},{4,8},{4,11},{5,12},{5,13},{6,8},{6,9},{7,9},{7,13},{8,10},{8,13},{9,11},{9,12}}

Cousin 369: {{1,5},{1,6},{1,10},{1,11},{2,4},{2,5},{2,6},{2,7},{2,8},{2,9},{3,5},{3,7},{3,10},{3,12},{4,7},{4,11},{4,13},{5,7},{5,8},{5,9},{6,12},{6,13},{7,8},{7,9},{8,10},{8,13},{9,11},{9,12}}

Cousin 370: {{1,5},{1,6},{1,10},{1,11},{2,4},{2,5},{2,6},{2,7},{2,8},{2,9},{3,5},{3,7},{3,10},{3,12},{4,6},{4,11},{4,13},{5,7},{5,8},{5,9},{6,8},{6,12},{7,9},{7,13},{8,10},{8,13},{9,11},{9,12}}

Cousin 371: {{1,5},{1,6},{1,10},{1,11},{2,4},{2,5},{2,6},{2,7},{2,8},{2,9},{3,5},{3,7},{3,10},{3,12},{4,6},{4,7},{4,8},{4,11},{5,9},{5,13},{6,8},{6,12},{7,9},{7,13},{8,10},{8,13},{9,11},{9,12}}

Cousin 372: {{1,5},{1,6},{1,10},{1,11},{2,4},{2,5},{2,6},{2,7},{2,8},{2,9},{3,5},{3,7},{3,10},{3,12},{4,6},{4,7},{4,8},{4,11},{5,8},{5,13},{6,8},{6,12},{7,8},{7,13},{8,10},{9,11},{9,12},{9,13}}

Cousin 373: {{1,5},{1,6},{1,10},{1,11},{2,4},{2,5},{2,6},{2,7},{2,8},{2,9},{3,5},{3,6},{3,10},{3,12},{4,7},{4,11},{4,13},{5,7},{5,8},{5,9},{6,9},{6,13},{7,8},{7,12},{8,10},{8,13},{9,11},{9,12}}

Cousin 374: {{1,5},{1,6},{1,10},{1,11},{2,4},{2,5},{2,6},{2,7},{2,8},{2,9},{3,5},{3,6},{3,10},{3,12},{4,6},{4,11},{4,13},{5,7},{5,8},{5,9},{6,8},{6,9},{7,12},{7,13},{8,10},{8,13},{9,11},{9,12}}

Cousin 375: {{1,5},{1,6},{1,10},{1,11},{2,4},{2,5},{2,6},{2,7},{2,8},{2,9},{3,5},{3,6},{3,7},{3,9},{3,10},{4,7},{4,11},{4,12},{5,9},{5,13},{6,9},{6,12},{7,9},{7,13},{8,10},{8,12},{8,13},{9,11}}

Cousin 376: {{1,5},{1,6},{1,10},{1,11},{2,4},{2,5},{2,6},{2,7},{2,8},{2,9},{3,5},{3,6},{3,7},{3,9},{3,10},{4,7},{4,11},{4,12},{5,8},{5,13},{6,9},{6,12},{7,8},{7,13},{8,10},{8,12},{9,11},{9,13}}

Cousin 377: {{1,5},{1,6},{1,10},{1,11},{2,4},{2,5},{2,6},{2,7},{2,8},{2,9},{3,5},{3,6},{3,7},{3,9},{3,10},{4,6},{4,11},{4,12},{5,8},{5,13},{6,8},{6,9},{7,12},{7,13},{8,10},{8,12},{9,11},{9,13}}

Cousin 378: {{1,4},{1,6},{1,10},{1,11},{2,5},{2,7},{2,12},{2,13},{3,5},{3,6},{3,7},{3,9},{3,10},{4,6},{4,7},{4,9},{4,12},{5,7},{5,8},{5,11},{6,8},{6,13},{7,8},{7,9},{8,10},{8,12},{9,11},{9,13}}

{8,10},{8,12},{9,11},{9,13}}

Cousin 379: {{1,4},{1,6},{1,10},{1,11},{2,5},{2,6},{2,12},{2,13},{3,5},{3,6},{3,7},{3,9},{3,10},{4,6},{4,7},{4,9},{4,12},{5,7},{5,8},{5,11},{6,8},{6,9},{7,8},{7,13},{8,10},{8,12},{9,11},{9,13}}

Cousin 380: {{1,4},{1,6},{1,10},{1,11},{2,5},{2,6},{2,7},{2,9},{2,12},{3,5},{3,7},{3,10},{3,13},{4,6},{4,7},{4,9},{4,12},{5,7},{5,8},{5,11},{6,8},{6,13},{7,8},{7,9},{8,10},{8,12},{9,11},{9,13}}

Cousin 381: {{1,4},{1,6},{1,10},{1,11},{2,5},{2,6},{2,7},{2,9},{2,12},{3,5},{3,6},{3,7},{3,9},{3,10},{4,7},{4,12},{4,13},{5,7},{5,8},{5,11},{6,8},{6,13},{7,8},{7,9},{8,10},{8,12},{9,11},{9,13}}

Cousin 382: {{1,4},{1,6},{1,10},{1,11},{2,5},{2,6},{2,7},{2,9},{2,12},{3,5},{3,6},{3,7},{3,9},{3,10},{4,6},{4,12},{4,13},{5,7},{5,8},{5,11},{6,8},{6,9},{7,8},{7,13},{8,10},{8,12},{9,11},{9,13}}

Cousin 383: {{1,4},{1,6},{1,10},{1,11},{2,5},{2,7},{2,12},{2,13},{3,5},{3,6},{3,7},{3,9},{3,10},{4,6},{4,7},{4,8},{4,12},{5,7},{5,8},{5,11},{6,9},{6,13},{7,8},{7,9},{8,10},{8,13},{9,11},{9,12}}

Cousin 384: {{1,4},{1,6},{1,10},{1,11},{2,5},{2,6},{2,12},{2,13},{3,5},{3,6},{3,7},{3,9},{3,10},{4,6},{4,7},{4,8},{4,12},{5,7},{5,8},{5,11},{6,8},{6,9},{7,9},{7,13},{8,10},{8,13},{9,11},{9,12}}

Cousin 385: {{1,4},{1,6},{1,10},{1,11},{2,5},{2,6},{2,7},{2,8},{2,12},{3,5},{3,7},{3,10},{3,13},{4,6},{4,7},{4,8},{4,12},{5,7},{5,8},{5,11},{6,8},{6,13},{7,8},{7,9},{8,10},{9,11},{9,12},{9,13}}

Cousin 386: {{1,4},{1,6},{1,10},{1,11},{2,5},{2,6},{2,7},{2,8},{2,12},{3,5},{3,6},{3,7},{3,9},{3,10},{4,7},{4,12},{4,13},{5,7},{5,8},{5,11},{6,9},{6,13},{7,8},{7,9},{8,10},{8,13},{9,11},{9,12}}

Cousin 387: {{1,4},{1,6},{1,10},{1,11},{2,5},{2,6},{2,7},{2,8},{2,12},{3,5},{3,6},{3,7},{3,9},{3,10},{4,6},{4,12},{4,13},{5,7},{5,8},{5,11},{6,8},{6,9},{7,9},{7,13},{8,10},{8,13},{9,11},{9,12}}

Cousin 388: {{1,4},{1,6},{1,10},{1,11},{2,4},{2,7},{2,12},{2,13},{3,5},{3,6},{3,7},{3,9},{3,10},{4,6},{4,7},{4,8},{4,9},{5,7},{5,11},{5,12},{6,8},{6,13},{7,8},{7,9},{8,10},{8,12},{9,11},{9,13}}

Cousin 389: {{1,4},{1,6},{1,10},{1,11},{2,4},{2,6},{2,12},{2,13},{3,5},{3,6},{3,7},{3,9},{3,10},{4,6},{4,7},{4,8},{4,9},{5,7},{5,11},{5,12},{6,8},{6,9},{7,8},{7,13},{8,10},{8,12},{9,11},{9,13}}

Cousin 390: {{1,4},{1,6},{1,10},{1,11},{2,4},{2,6},{2,7},{2,9},{2,12},{3,5},{3,7},{3,10},{3,13},{4,6},{4,7},{4,8},{4,9},{5,7},{5,11},{5,12},{6,8},{6,13},{7,8},{7,9},{8,10},{8,12},{9,11},{9,13}}

Cousin 391: {{1,4},{1,6},{1,10},{1,11},{2,4},{2,6},{2,7},{2,9},{2,12},{3,5},{3,6},{3,7},{3,9},{3,10},{4,7},{4,9},{4,13},{5,7},{5,11},{5,12},{6,9},{6,13},{7,8},{7,9},{8,10},{8,12},{8,13},{9,11}}

Cousin 392: {{1,4},{1,6},{1,10},{1,11},{2,4},{2,6},{2,7},{2,9},{2,12},{3,5},{3,6},{3,7},{3,9},{3,10},{4,7},{4,8},{4,13},{5,7},{5,11},{5,12},{6,8},{6,13},{7,8},{7,9},{8,10},{8,12},{9,11},{9,13}}

Cousin 393: {{1,4},{1,6},{1,10},{1,11},{2,4},{2,6},{2,7},{2,9},{2,12},{3,5},{3,6},{3,7},{3,9},{3,10},{4,6},{4,9},{4,13},{5,7},{5,11},{5,12},{6,8},{6,9},{7,9},{7,13},{8,10},{8,12},{8,13},{9,11}}

Cousin 394: {{1,4},{1,6},{1,10},{1,11},{2,4},{2,6},{2,7},{2,9},{2,12},{3,5},{3,6},{3,7},{3,9},{3,10},{4,6},{4,8},{4,13},{5,7},{5,11},{5,12},{6,8},{6,9},{7,8},{7,13},{8,10},{8,12},{9,11},{9,13}}

Cousin 395: {{1,4},{1,6},{1,10},{1,11},{2,4},{2,5},{2,7},{2,9},{2,12},{3,5},{3,6},{3,7},{3,9},{3,10},{4,7},{4,8},{4,13},{5,7},{5,8},{5,11},{6,12},{6,13},{7,8},{7,9},{8,10},{8,12},{9,11},{9,13}}

Cousin 396: {{1,4},{1,6},{1,10},{1,11},{2,4},{2,5},{2,7},{2,9},{2,12},{3,5},{3,6},{3,7},{3,9},{3,10},{4,6},{4,9},{4,13},{5,7},{5,8},{5,11},{6,9},{6,12},{7,9},{7,13},{8,10},{8,12},{8,13},{9,11}}

Cousin 397: {{1,4},{1,6},{1,10},{1,11},{2,4},{2,5},{2,7},{2,9},{2,12},{3,5},{3,6},{3,7},{3,9},{3,10},{4,6},{4,8},{4,13},{5,7},{5,8},{5,11},{6,9},{6,12},{7,8},{7,13},{8,10},{8,12},{9,11},{9,13}}

Cousin 398: {{1,4},{1,6},{1,10},{1,11},{2,4},{2,5},{2,7},{2,8},{2,12},{3,5},{3,6},{3,7},{3,9},{3,10},{4,7},{4,9},{4,13},{5,7},{5,8},{5,11},{6,12},{6,13},{7,8},{7,9},{8,10},{8,13},{9,11},{9,12}}

Cousin 399: {{1,4},{1,6},{1,10},{1,11},{2,4},{2,5},{2,7},{2,8},{2,12},{3,5},{3,6},{3,7},{3,9},{3,10},{4,6},{4,9},{4,13},{5,7},{5,8},{5,11},{6,8},{6,12},{7,9},{7,13},{8,10},{8,13},{9,11},{9,12}}

Cousin 400: {{1,4},{1,6},{1,10},{1,11},{2,4},{2,5},{2,7},{2,8},{2,12},{3,5},{3,6},{3,7},{3,9},{3,10},{4,6},{4,8},{4,13},{5,7},{5,8},{5,11},{6,8},{6,12},{7,8},{7,13},{8,10},{9,11},{9,12},{9,13}}

Cousin 401: {{1,4},{1,6},{1,10},{1,11},{2,4},{2,5},{2,6},{2,9},{2,12},{3,5},{3,6},{3,7},{3,9},{3,10},{4,7},{4,9},{4,13},{5,7},{5,8},{5,11},{6,9},{6,13},{7,9},{7,12},{8,10},{8,12},{8,13},{9,11}}

Cousin 402: {{1,4},{1,6},{1,10},{1,11},{2,4},{2,5},{2,6},{2,9},{2,12},{3,5},{3,6},{3,7},{3,9},{3,10},{4,7},{4,8},{4,13},{5,7},{5,8},{5,11},{6,8},{6,13},{7,9},{7,12},{8,10},{8,12},{9,11},{9,13}}

Cousin 403: {{1,4},{1,6},{1,10},{1,11},{2,4},{2,5},{2,6},{2,8},{2,12},{3,5},{3,6},{3,7},{3,9},{3,10},{4,7},{4,9},{4,13},{5,7},{5,8},{5,11},{6,9},{6,13},{7,8},{7,12},{8,10},{8,13},{9,11},{9,12}}

Cousin 404: {{1,4},{1,6},{1,10},{1,11},{2,4},{2,5},{2,6},{2,8},{2,12},{3,5},{3,6},{3,7},{3,9},{3,10},{4,7},{4,8},{4,13},{5,7},{5,8},{5,11},{6,8},{6,13},{7,8},{7,12},{8,10},{9,11},{9,12},{9,13}}

Cousin 405: {{1,4},{1,6},{1,10},{1,11},{2,4},{2,5},{2,6},{2,7},{2,8},{2,9},{3,5},{3,7},{3,10},{3,12},{4,6},{4,9},{4,13},{5,7},{5,8},{5,11},{6,8},{6,12},{7,9},{7,13},{8,10},{8,13},{9,11},{9,12}}

Cousin 406: {{1,4},{1,6},{1,10},{1,11},{2,4},{2,5},{2,6},{2,7},{2,8},{2,9},{3,5},{3,7},{3,10},{3,12},{4,6},{4,8},{4,13},{5,7},{5,8},{5,11},{6,8},{6,12},{7,8},{7,13},{8,10},{9,11},{9,12},{9,13}}

Cousin 407: {{1,4},{1,5},{1,10},{1,11},{2,5},{2,6},{2,12},{2,13},{3,5},{3,6},{3,7},{3,9},{3,10},{4,6},{4,7},{4,9},{4,12},{5,7},{5,8},{5,9},{6,8},{6,11},{7,8},{7,13},{8,10},{8,12},{9,11},{9,13}}

Cousin 408: {{1,4},{1,5},{1,10},{1,11},{2,5},{2,6},{2,7},{2,9},{2,12},{3,6},{3,7},{3,10},{3,13},{4,6},{4,7},{4,9},{4,12},{5,7},{5,8},{5,13},{6,8},{6,11},{7,8},{7,9},{8,10},{8,12},{9,11},{9,13}}

Cousin 409: {{1,4},{1,5},{1,10},{1,11},{2,5},{2,6},{2,7},{2,9},{2,12},{3,5},{3,6},{3,7},{3,9},{3,10},{4,6},{4,7},{4,9},{4,12},{5,9},{5,13},{6,8},{6,11},{7,9},{7,13},{8,10},{8,12},{8,13},{9,11}}

Cousin 410: {{1,4},{1,5},{1,10},{1,11},{2,5},{2,6},{2,7},{2,9},{2,12},{3,5},{3,6},{3,7},{3,9},{3,10},{4,6},{4,7},{4,9},{4,12},{5,8},{5,13},{6,8},{6,11},{7,8},{7,13},{8,10},{8,12},{9,11},{9,13}}

Cousin 411: {{1,4},{1,5},{1,10},{1,11},{2,5},{2,6},{2,12},{2,13},{3,5},{3,6},{3,7},{3,9},{3,10},{4,6},{4,7},{4,8},{4,12},{5,7},{5,8},{5,9},{6,8},{6,11},{7,9},{7,13},{8,10},{8,13},{9,11},{9,12}}

Cousin 412: {{1,4},{1,5},{1,10},{1,11},{2,5},{2,6},{2,7},{2,8},{2,12},{3,6},{3,7},{3,10},{3,13},{4,6},{4,7},{4,8},{4,12},{5,7},{5,8},{5,13},{6,8},{6,11},{7,8},{7,9},{8,10},{9,11},{9,12},{9,13}}

Cousin 413: {{1,4},{1,5},{1,10},{1,11},{2,5},{2,6},{2,7},{2,8},{2,12},{3,5},{3,6},{3,7},{3,9},{3,10},{4,7},{4,12},{4,13},{5,7},{5,8},{5,9},{6,11},{6,13},{7,8},{7,9},{8,10},{8,13},{9,11},{9,12}}

Cousin 414: {{1,4},{1,5},{1,10},{1,11},{2,5},{2,6},{2,7},{2,8},{2,12},{3,5},{3,6},{3,7},{3,9},{3,10},{4,6},{4,7},{4,8},{4,12},{5,9},{5,13},{6,8},{6,11},{7,9},{7,13},{8,10},{8,13},{9,11},{9,12}}

Cousin 415: {{1,4},{1,5},{1,10},{1,11},{2,4},{2,6},{2,7},{2,9},{2,12},{3,5},{3,6},{3,7},{3,9},{3,10},{4,7},{4,9},{4,13},{5,7},{5,8},{5,12},{6,11},{6,13},{7,8},{7,9},{8,10},{8,12},{8,13},{9,11}}

Cousin 416: {{1,4},{1,5},{1,10},{1,11},{2,4},{2,6},{2,7},{2,9},{2,12},{3,5},{3,6},{3,7},{3,9},{3,10},{4,6},{4,9},{4,13},{5,7},{5,9},{5,12},{6,8},{6,11},{7,9},{7,13},{8,10},{8,12},{8,13},{9,11}}

Cousin 417: {{1,4},{1,5},{1,10},{1,11},{2,4},{2,6},{2,7},{2,9},{2,12},{3,5},{3,6},{3,7},{3,9},{3,10},{4,6},{4,8},{4,13},{5,7},{5,9},{5,12},{6,8},{6,11},{7,8},{7,13},{8,10},{8,12},{9,11},{9,13}}

Cousin 418: {{1,4},{1,5},{1,10},{1,11},{2,4},{2,6},{2,7},{2,8},{2,12},{3,5},{3,6},{3,7},{3,9},{3,10},{4,7},{4,9},{4,13},{5,7},{5,8},{5,12},{6,11},{6,13},{7,8},{7,9},{8,10},{8,13},{9,11},{9,12}}

Cousin 419: {{1,4},{1,5},{1,10},{1,11},{2,4},{2,6},{2,7},{2,8},{2,12},{3,5},{3,6},{3,7},{3,9},{3,10},{4,6},{4,9},{4,13},{5,7},{5,8},{5,12},{6,8},{6,11},{7,9},{7,13},{8,10},{8,13},{9,11},{9,12}}

Cousin 420: {{1,4},{1,5},{1,6},{1,9},{1,10},{2,4},{2,7},{2,11},{2,12},{3,5},{3,6},{3,7},{3,9},{3,10},{4,6},{4,9},{4,13},{5,7},{5,9},{5,11},{6,8},{6,12},{7,9},{7,13},{8,10},{8,11},{8,13},{9,12}}

Cousin 421: {{1,4},{1,5},{1,6},{1,9},{1,10},{2,4},{2,7},{2,11},{2,12},{3,5},{3,6},{3,7},{3,9},{3,10},{4,6},{4,8},{4,13},{5,7},{5,9},{5,11},{6,8},{6,12},{7,8},{7,13},{8,10},{8,11},{9,12},{9,13}}

Cousin 422: {{1,3},{1,6},{1,10},{1,11},{2,4},{2,7},{2,12},{2,13},{3,5},{3,6},{3,7},{3,8},{3,9},{4,6},{4,7},{4,9},{4,10},{5,7},{5,11},{5,12},{6,8},{6,13},{7,8},{7,9},{8,10},{8,12},{9,11},{9,13}}

Cousin 423: {{1,3},{1,6},{1,10},{1,11},{2,4},{2,6},{2,7},{2,9},{2,12},{3,5},{3,7},{3,9},{3,13},{4,6},{4,7},{4,9},{4,10},{5,7},{5,11},{5,12},{6,9},{6,13},{7,8},{7,9},{8,10},{8,12},{8,13},{9,11}}

Cousin 424: {{1,3},{1,6},{1,10},{1,11},{2,4},{2,6},{2,7},{2,9},{2,12},{3,5},{3,7},{3,8},{3,13},{4,6},{4,7},{4,9},{4,10},{5,7},{5,11},{5,12},{6,8},{6,13},{7,8},{7,9},{8,10},{8,12},{9,11},{9,13}}

Cousin 425: {{1,3},{1,6},{1,10},{1,11},{2,4},{2,5},{2,7},{2,9},{2,12},{3,5},{3,7},{3,8},{3,13},{4,6},{4,7},{4,9},{4,10},{5,7},{5,8},{5,11},{6,12},{6,13},{7,8},{7,9},{8,10},{8,12},{9,11},{9,13}}

Cousin 426: {{1,3},{1,6},{1,10},{1,11},{2,4},{2,5},{2,7},{2,9},{2,12},{3,5},{3,6},{3,9},{3,13},{4,6},{4,7},{4,9},{4,10},{5,7},{5,8},{5,11},{6,9},{6,12},{7,9},{7,13},{8,10},{8,12},{8,13},{9,11}}

Cousin 427: {{1,3},{1,6},{1,10},{1,11},{2,4},{2,5},{2,7},{2,9},{2,12},{3,5},{3,6},{3,8},{3,13},{4,6},{4,7},{4,9},{4,10},{5,7},{5,8},{5,11},{6,9},{6,12},{7,8},{7,13},{8,10},{8,12},{9,11},{9,13}}

Cousin 428: {{1,3},{1,6},{1,10},{1,11},{2,4},{2,5},{2,7},{2,8},{2,12},{3,5},{3,7},{3,9},{3,13},{4,6},{4,7},{4,9},{4,10},{5,7},{5,8},{5,11},{6,12},{6,13},{7,8},{7,9},{8,10},{8,13},{9,11},{9,12}}

Cousin 429: {{1,3},{1,6},{1,10},{1,11},{2,4},{2,5},{2,7},{2,8},{2,12},{3,5},{3,6},{3,9},{3,13},{4,6},{4,7},{4,9},{4,10},{5,7},{5,8},{5,11},{6,8},{6,12},{7,9},{7,13},{8,10},{8,13},{9,11},{9,12}}

Cousin 430: {{1,8},{1,9},{1,10},{1,11},{2,12},{2,13},{2,14},{3,6},{3,7},{3,8},{3,9},{3,10},{4,8},{4,9},{4,11},{4,12},{5,7},{5,9},{5,10},{5,13},{6,8},{6,11},{6,14},{7,8},{7,9},{7,12},{8,13},{9,14}}

Cousin 431: {{1,8},{1,9},{1,10},{1,11},{2,6},{2,9},{2,12},{2,13},{3,7},{3,9},{3,10},{3,14},{4,8},{4,9},{4,11},{4,12},{5,7},{5,9},{5,10},{5,13},{6,9},{6,11},{6,14},{7,8},{7,9},{7,12},{8,13},{8,14}}

Cousin 432: {{1,8},{1,9},{1,10},{1,11},{2,6},{2,9},{2,12},{2,13},{3,7},{3,8},{3,10},{3,14},{4,8},{4,9},{4,11},{4,12},{5,7},{5,9},{5,10},{5,13},{6,8},{6,11},{6,14},{7,8},{7,9},{7,12},{8,13},{9,14}}

Cousin 433: {{1,8},{1,9},{1,10},{1,11},{2,6},{2,9},{2,12},{2,13},{3,6},{3,9},{3,10},{3,14},{4,8},{4,9},{4,11},{4,12},{5,7},{5,9},{5,10},{5,13},{6,8},{6,9},{6,11},{7,9},{7,12},{7,14},{8,13},{8,14}}

Cousin 434: {{1,8},{1,9},{1,10},{1,11},{2,6},{2,9},{2,12},{2,13},{3,6},{3,8},{3,10},{3,14},{4,8},{4,9},{4,11},{4,12},{5,7},{5,9},{5,10},{5,13},{6,8},{6,9},{6,11},{7,8},{7,12},{7,14},{8,13},{9,14}}

Cousin 435: {{1,8},{1,9},{1,10},{1,11},{2,6},{2,9},{2,12},{2,13},{3,6},{3,7},{3,8},{3,9},{3,10},{4,8},{4,9},{4,11},{4,12},{5,10},{5,13},{5,14},{6,8},{6,9},{6,11},{7,8},{7,12},{7,14},{8,13},{9,14}}

Cousin 436: {{1,8},{1,9},{1,10},{1,11},{2,5},{2,9},{2,12},{2,13},{3,7},{3,8},{3,10},{3,14},{4,8},{4,9},{4,11},{4,12},{5,7},{5,8},{5,9},{5,10},{6,11},{6,13},{6,14},{7,8},{7,9},{7,12},{8,13},{9,14}}

Cousin 437: {{1,8},{1,9},{1,10},{1,11},{2,5},{2,9},{2,12},{2,13},{3,6},{3,7},{3,8},{3,9},{3,10},{4,8},{4,9},{4,11},{4,12},{5,9},{5,10},{5,14},{6,9},{6,11},{6,13},{7,9},{7,12},{7,14},{8,13},{8,14}}

Cousin 438: {{1,8},{1,9},{1,10},{1,11},{2,5},{2,9},{2,12},{2,13},{3,6},{3,7},{3,8},{3,9},{3,10},{4,8},{4,9},{4,11},{4,12},{5,8},{5,10},{5,14},{6,9},{6,11},{6,13},{7,8},{7,12},{7,14},{8,13},{9,14}}

Cousin 439: {{1,8},{1,9},{1,10},{1,11},{2,6},{2,7},{2,12},{2,13},{3,7},{3,9},{3,10},{3,14},{4,7},{4,9},{4,11},{4,12},{5,7},{5,8},{5,10},{5,13},{6,9},{6,11},{6,14},{7,8},{7,9},{8,12},{8,14},{9,13}}

Cousin 440: {{1,8},{1,9},{1,10},{1,11},{2,6},{2,7},{2,12},{2,13},{3,7},{3,8},{3,10},{3,14},{4,7},{4,9},{4,11},{4,12},{5,7},{5,8},{5,10},{5,13},{6,8},{6,11},{6,14},{7,8},{7,9},{8,12},{9,13},{9,14}}

Cousin 441: {{1,8},{1,9},{1,10},{1,11},{2,6},{2,7},{2,12},{2,13},{3,6},{3,9},{3,10},{3,14},{4,7},{4,9},{4,11},{4,12},{5,7},{5,8},{5,10},{5,13},{6,8},{6,9},{6,11},{7,9},{7,14},{8,12},{8,14},{9,13}}

Cousin 442: {{1,8},{1,9},{1,10},{1,11},{2,6},{2,7},{2,12},{2,13},{3,6},{3,8},{3,10},{3,14},{4,7},{4,9},{4,11},{4,12},{5,7},{5,8},{5,10},{5,13},{6,8},{6,9},{6,11},{7,8},{7,14},{8,12},{9,13},{9,14}}

Cousin 443: {{1,8},{1,9},{1,10},{1,11},{2,6},{2,7},{2,12},{2,13},{3,6},{3,7},{3,8},{3,9},{3,10},{4,11},{4,12},{4,14},{5,7},{5,8},{5,10},{5,13},{6,8},{6,9},{6,11},{7,8},{7,14},{8,12},{9,13},{9,14}}

Cousin 444: {{1,8},{1,9},{1,10},{1,11},{2,6},{2,7},{2,12},{2,13},{3,6},{3,7},{3,8},{3,9},{3,10},{4,7},{4,9},{4,11},{4,12},{5,10},{5,13},{5,14},{6,8},{6,9},{6,11},{7,9},{7,14},{8,12},{8,14},{9,13}}

Cousin 445: {{1,8},{1,9},{1,10},{1,11},{2,5},{2,7},{2,12},{2,13},{3,7},{3,9},{3,10},{3,14},{4,7},{4,9},{4,11},{4,12},{5,7},{5,8},{5,9},{5,10},{6,11},{6,13},{6,14},{7,8},{7,9},{8,12},{8,14},{9,13}}

Cousin 446: {{1,8},{1,9},{1,10},{1,11},{2,5},{2,7},{2,12},{2,13},{3,6},{3,9},{3,10},{3,14},{4,7},{4,9},{4,11},{4,12},{5,7},{5,8},{5,9},{5,10},{6,8},{6,11},{6,13},{7,9},{7,14},{8,12},{8,14},{9,13}}

Cousin 447: {{1,8},{1,9},{1,10},{1,11},{2,5},{2,7},{2,12},{2,13},{3,6},{3,8},{3,10},{3,14},{4,7},{4,9},{4,11},{4,12},{5,7},{5,8},{5,9},{5,10},{6,8},{6,11},{6,13},{7,8},{7,14},{8,12},{9,13},{9,14}}

Cousin 448: {{1,8},{1,9},{1,10},{1,11},{2,5},{2,7},{2,12},{2,13},{3,6},{3,7},{3,8},{3,9},{3,10},{4,11},{4,12},{4,14},{5,7},{5,8},{5,9},{5,10},{6,8},{6,11},{6,13},{7,8},{7,14},{8,12},{9,13},{9,14}}

Cousin 449: {{1,8},{1,9},{1,10},{1,11},{2,5},{2,7},{2,12},{2,13},{3,6},{3,7},{3,8},{3,9},{3,10},{4,7},{4,9},{4,11},{4,12},{5,9},{5,10},{5,14},{6,8},{6,11},{6,13},{7,9},{7,14},{8,12},{8,14},{9,13}}

Cousin 450: {{1,8},{1,9},{1,10},{1,11},{2,5},{2,7},{2,12},{2,13},{3,6},{3,7},{3,8},{3,9},{3,10},{4,7},{4,9},{4,11},{4,12},{5,8},{5,10},{5,14},{6,8},{6,11},{6,13},{7,8},{7,14},{8,12},{9,13},{9,14}}

Cousin 451: {{1,8},{1,9},{1,10},{1,11},{2,5},{2,6},{2,12},{2,13},{3,7},{3,9},{3,10},{3,14},{4,7},{4,9},{4,11},{4,12},{5,7},{5,8},{5,9},{5,10},{6,9},{6,11},{6,14},{7,8},{7,13},{8,12},{8,14},{9,13}}

Cousin 452: {{1,8},{1,9},{1,10},{1,11},{2,5},{2,6},{2,12},{2,13},{3,7},{3,8},{3,10},{3,14},{4,7},{4,9},{4,11},{4,12},{5,7},{5,8},{5,9},{5,10},{6,8},{6,11},{6,14},{7,8},{7,13},{8,12},{9,13},{9,14}}

Cousin 453: {{1,8},{1,9},{1,10},{1,11},{2,5},{2,6},{2,12},{2,13},{3,6},{3,9},{3,10},{3,14},{4,7},{4,9},{4,11},{4,12},{5,7},{5,8},{5,9},{5,10},{6,8},{6,9},{6,11},{7,13},{7,14},{8,12},{8,14},{9,13}}

Cousin 454: {{1,8},{1,9},{1,10},{1,11},{2,5},{2,6},{2,12},{2,13},{3,6},{3,7},{3,8},{3,9},{3,10},{4,7},{4,9},{4,11},{4,12},{5,9},{5,10},{5,14},{6,8},{6,9},{6,11},{7,13},{7,14},{8,12},{8,14},{9,13}}

{7,14},{8,12},{8,14},{9,13}}

Cousin 455: {{1,8},{1,9},{1,10},{1,11},{2,5},{2,6},{2,7},{2,9},{2,12},{3,10},{3,13},{3,14},{4,7},{4,9},{4,11},{4,12},{5,7},{5,8},{5,9},{5,10},{6,9},{6,11},{6,13},{7,8},{7,14},{8,12},{8,13},{9,14}}

Cousin 456: {{1,8},{1,9},{1,10},{1,11},{2,5},{2,6},{2,7},{2,9},{2,12},{3,7},{3,9},{3,10},{3,13},{4,11},{4,12},{4,14},{5,7},{5,8},{5,9},{5,10},{6,9},{6,11},{6,13},{7,8},{7,14},{8,12},{8,13},{9,14}}

Cousin 457: {{1,8},{1,9},{1,10},{1,11},{2,5},{2,6},{2,7},{2,9},{2,12},{3,7},{3,9},{3,10},{3,13},{4,7},{4,9},{4,11},{4,12},{5,9},{5,10},{5,14},{6,9},{6,11},{6,13},{7,9},{7,14},{8,12},{8,13},{8,14}}

Cousin 458: {{1,8},{1,9},{1,10},{1,11},{2,5},{2,6},{2,7},{2,9},{2,12},{3,7},{3,9},{3,10},{3,13},{4,7},{4,9},{4,11},{4,12},{5,8},{5,10},{5,14},{6,9},{6,11},{6,13},{7,8},{7,14},{8,12},{8,13},{9,14}}

Cousin 459: {{1,8},{1,9},{1,10},{1,11},{2,5},{2,6},{2,7},{2,9},{2,12},{3,10},{3,13},{3,14},{4,7},{4,9},{4,11},{4,12},{5,7},{5,8},{5,9},{5,10},{6,8},{6,11},{6,13},{7,9},{7,14},{8,12},{8,14},{9,13}}

Cousin 460: {{1,8},{1,9},{1,10},{1,11},{2,5},{2,6},{2,7},{2,9},{2,12},{3,7},{3,8},{3,10},{3,13},{4,11},{4,12},{4,14},{5,7},{5,8},{5,9},{5,10},{6,8},{6,11},{6,13},{7,8},{7,14},{8,12},{9,13},{9,14}}

Cousin 461: {{1,8},{1,9},{1,10},{1,11},{2,5},{2,6},{2,7},{2,9},{2,12},{3,7},{3,8},{3,10},{3,13},{4,7},{4,9},{4,11},{4,12},{5,9},{5,10},{5,14},{6,8},{6,11},{6,13},{7,9},{7,14},{8,12},{8,14},{9,13}}

Cousin 462: {{1,8},{1,9},{1,10},{1,11},{2,5},{2,6},{2,7},{2,9},{2,12},{3,6},{3,9},{3,10},{3,13},{4,11},{4,12},{4,14},{5,7},{5,8},{5,9},{5,10},{6,8},{6,9},{6,11},{7,13},{7,14},{8,12},{8,13},{9,14}}

Cousin 463: {{1,8},{1,9},{1,10},{1,11},{2,5},{2,6},{2,7},{2,9},{2,12},{3,6},{3,7},{3,8},{3,9},{3,10},{4,7},{4,9},{4,11},{4,12},{5,7},{5,8},{5,9},{5,10},{6,8},{6,9},{6,11},{7,8},{8,12},{11,12}}

Cousin 464: {{1,8},{1,9},{1,10},{1,11},{2,4},{2,7},{2,12},{2,13},{3,7},{3,9},{3,10},{3,14},{4,7},{4,8},{4,9},{4,11},{5,7},{5,9},{5,10},{5,12},{6,11},{6,13},{6,14},{7,8},{7,9},{8,12},{8,14},{9,13}}

Cousin 465: {{1,8},{1,9},{1,10},{1,11},{2,4},{2,7},{2,12},{2,13},{3,6},{3,9},{3,10},{3,14},{4,7},{4,8},{4,9},{4,11},{5,7},{5,9},{5,10},{5,12},{6,8},{6,11},{6,13},{7,9},{7,14},{8,12},{8,14},{9,13}}

Cousin 466: {{1,8},{1,9},{1,10},{1,11},{2,4},{2,7},{2,12},{2,13},{3,6},{3,8},{3,10},{3,14},{4,7},{4,8},{4,9},{4,11},{5,7},{5,9},{5,10},{5,12},{6,8},{6,11},{6,13},{7,8},{7,14},{8,12},{9,13},{9,14}}

Cousin 467: {{1,8},{1,9},{1,10},{1,11},{2,4},{2,7},{2,12},{2,13},{3,6},{3,7},{3,8},{3,9},{3,10},{4,9},{4,11},{4,14},{5,7},{5,9},{5,10},{5,12},{6,8},{6,11},{6,13},{7,9},{7,14},{8,12},{8,14},{9,13}}

Cousin 468: {{1,8},{1,9},{1,10},{1,11},{2,4},{2,7},{2,12},{2,13},{3,6},{3,7},{3,8},{3,9},{3,10},{4,8},{4,11},{4,14},{5,7},{5,9},{5,10},{5,12},{6,8},{6,11},{6,13},{7,8},{7,14},{8,12},{9,13},{9,14}}

Cousin 469: {{1,8},{1,9},{1,10},{1,11},{2,4},{2,6},{2,12},{2,13},{3,7},{3,9},{3,10},{3,14},{4,7},{4,8},{4,9},{4,11},{5,7},{5,9},{5,10},{5,12},{6,9},{6,11},{6,14},{7,8},{7,13},{8,12},{8,14},{9,13}}

Cousin 470: {{1,8},{1,9},{1,10},{1,11},{2,4},{2,6},{2,12},{2,13},{3,7},{3,8},{3,10},{3,14},{4,7},{4,8},{4,9},{4,11},{5,7},{5,9},{5,10},{5,12},{6,8},{6,11},{6,14},{7,8},{7,13},{8,12},{9,13},{9,14}}

Cousin 471: {{1,8},{1,9},{1,10},{1,11},{2,4},{2,6},{2,12},{2,13},{3,6},{3,9},{3,10},{3,14},{4,7},{4,8},{4,9},{4,11},{5,7},{5,9},{5,10},{5,12},{6,8},{6,9},{6,11},{7,13},{7,14},{8,12},{8,14},{9,13}}

Cousin 472: {{1,8},{1,9},{1,10},{1,11},{2,4},{2,6},{2,12},{2,13},{3,6},{3,7},{3,8},{3,9},{3,10},{4,9},{4,11},{4,14},{5,7},{5,9},{5,10},{5,12},{6,8},{6,9},{6,11},{7,13},{7,14},{8,12},{8,14},{9,13}}

Cousin 473: {{1,8},{1,9},{1,10},{1,11},{2,4},{2,6},{2,7},{2,9},{2,12},{3,10},{3,13},{3,14},{4,7},{4,8},{4,9},{4,11},{5,7},{5,9},{5,10},{5,12},{6,9},{6,11},{6,13},{7,8},{7,14},{8,12},{8,13},{9,14}}

Cousin 474: {{1,8},{1,9},{1,10},{1,11},{2,4},{2,6},{2,7},{2,9},{2,12},{3,7},{3,9},{3,10},{3,13},{4,9},{4,11},{4,14},{5,7},{5,9},{5,10},{5,12},{6,9},{6,11},{6,13},{7,9},{7,14},{8,12},{8,13},{8,14}}

Cousin 475: {{1,8},{1,9},{1,10},{1,11},{2,4},{2,6},{2,7},{2,9},{2,12},{3,7},{3,9},{3,10},{3,13},{4,8},{4,11},{4,14},{5,7},{5,9},{5,10},{5,12},{6,9},{6,11},{6,13},{7,8},{7,14},{8,12},{8,13},{9,14}}

Cousin 476: {{1,8},{1,9},{1,10},{1,11},{2,4},{2,6},{2,7},{2,9},{2,12},{3,10},{3,13},{3,14},{4,7},{4,8},{4,9},{4,11},{5,7},{5,9},{5,10},{5,12},{6,8},{6,11},{6,13},{7,9},{7,14},{8,12},{8,14},{9,13}}

Cousin 477: {{1,8},{1,9},{1,10},{1,11},{2,4},{2,6},{2,7},{2,9},{2,12},{3,7},{3,8},{3,10},{3,13},{4,9},{4,11},{4,14},{5,7},{5,9},{5,10},{5,12},{6,8},{6,11},{6,13},{7,9},{7,14},{8,12},{8,14},{9,13}}

Cousin 478: {{1,8},{1,9},{1,10},{1,11},{2,4},{2,5},{2,12},{2,13},{3,7},{3,8},{3,10},{3,14},{4,7},{4,8},{4,9},{4,11},{5,7},{5,8},{5,9},{5,10},{6,11},{6,12},{6,14},{7,8},{7,13},{8,12},{9,13},{9,14}}

Cousin 479: {{1,8},{1,9},{1,10},{1,11},{2,4},{2,5},{2,12},{2,13},{3,6},{3,9},{3,10},{3,14},{4,7},{4,8},{4,9},{4,11},{5,7},{5,8},{5,9},{5,10},{6,9},{6,11},{6,12},{7,13},{7,14},{8,12},{8,14},{9,13}}



Cousin 480: {{1,8},{1,9},{1,10},{1,11},{2,4},{2,5},{2,7},{2,9},{2,12},{3,10},{3,13},{3,14},{4,7},{4,8},{4,9},{4,11},{5,7},{5,8},{5,9},{5,10},{6,11},{6,12},{6,13},{7,9},{7,14},{8,12},{8,14},{9,13}}

Cousin 481: {{1,8},{1,9},{1,10},{1,11},{2,4},{2,5},{2,7},{2,9},{2,12},{3,6},{3,7},{3,8},{3,10},{4,7},{4,8},{4,9},{4,11},{5,7},{5,8},{5,9},{5,10},{6,9},{6,11},{6,12},{7,8},{7,9},{8,12},{11,12}}

Cousin 482: {{1,10},{1,11},{1,12},{2,7},{2,9},{2,13},{2,14},{3,6},{3,7},{3,8},{3,9},{3,10},{4,7},{4,9},{4,11},{4,13},{5,7},{5,9},{5,10},{5,14},{6,8},{6,12},{6,13},{7,8},{7,9},{8,11},{8,14},{9,12}}

Cousin 483: {{1,10},{1,11},{1,12},{2,7},{2,8},{2,13},{2,14},{3,6},{3,7},{3,8},{3,9},{3,10},{4,7},{4,9},{4,11},{4,13},{5,7},{5,8},{5,10},{5,14},{6,8},{6,12},{6,13},{7,8},{7,9},{8,11},{9,12},{9,14}}

Cousin 484: {{1,10},{1,11},{1,12},{2,5},{2,9},{2,13},{2,14},{3,6},{3,7},{3,8},{3,9},{3,10},{4,7},{4,9},{4,11},{4,13},{5,7},{5,8},{5,9},{5,10},{6,8},{6,12},{6,13},{7,9},{7,14},{8,11},{8,14},{9,12}}

Cousin 485: {{1,10},{1,11},{1,12},{2,5},{2,8},{2,13},{2,14},{3,6},{3,7},{3,8},{3,9},{3,10},{4,7},{4,9},{4,11},{4,13},{5,7},{5,8},{5,9},{5,10},{6,8},{6,12},{6,13},{7,8},{7,14},{8,11},{9,12},{9,14}}

Cousin 486: {{1,10},{1,11},{1,12},{2,5},{2,7},{2,8},{2,9},{2,13},{3,7},{3,9},{3,10},{3,14},{4,7},{4,9},{4,11},{4,13},{5,7},{5,8},{5,9},{5,10},{6,12},{6,13},{6,14},{7,8},{7,9},{8,11},{8,14},{9,12}}

Cousin 487: {{1,10},{1,11},{1,12},{2,5},{2,7},{2,8},{2,9},{2,13},{3,6},{3,9},{3,10},{3,14},{4,7},{4,9},{4,11},{4,13},{5,7},{5,8},{5,9},{5,10},{6,8},{6,12},{6,13},{7,9},{7,14},{8,11},{8,14},{9,12}}

Cousin 488: {{1,10},{1,11},{1,12},{2,5},{2,7},{2,8},{2,9},{2,13},{3,6},{3,8},{3,10},{3,14},{4,7},{4,9},{4,11},{4,13},{5,7},{5,8},{5,9},{5,10},{6,8},{6,12},{6,13},{7,8},{7,14},{8,11},{9,12},{9,14}}

Cousin 489: {{1,10},{1,11},{1,12},{2,5},{2,7},{2,8},{2,9},{2,13},{3,6},{3,7},{3,8},{3,9},{3,10},{4,11},{4,13},{4,14},{5,7},{5,8},{5,9},{5,10},{6,8},{6,12},{6,13},{7,8},{7,14},{8,11},{9,12},{9,14}}

Cousin 490: {{1,10},{1,11},{1,12},{2,5},{2,7},{2,8},{2,9},{2,13},{3,6},{3,7},{3,8},{3,9},{3,10},{4,7},{4,9},{4,11},{4,13},{5,9},{5,10},{5,14},{6,8},{6,12},{6,13},{7,9},{7,14},{8,11},{8,14},{9,12}}

Cousin 491: {{1,10},{1,11},{1,12},{2,5},{2,7},{2,8},{2,9},{2,13},{3,6},{3,7},{3,8},{3,9},{3,10},{4,7},{4,9},{4,11},{4,13},{5,8},{5,10},{5,14},{6,8},{6,12},{6,13},{7,8},{7,14},{8,11},{9,12},{9,14}}

Cousin 492: {{1,2},{1,4},{1,6},{2,5},{2,7},{2,8},{2,9},{3,6},{3,7},{3,8},{3,9},{3,10},{4,7},{4,9},{4,11},{5,7},{5,8},{5,9},{5,10},{6,8},{6,12},{7,8},{7,9},{8,11},{9,12},{10,11},{10,12},{11,12}}

Cousin 493: {{1,10},{1,11},{1,12},{2,6},{2,9},{2,13},{2,14},{3,6},{3,7},{3,8},{3,9},{3,10},{4,6},{4,9},{4,11},{4,13},{5,7},{5,9},{5,10},{5,14},{6,8},{6,12},{7,8},{7,9},{7,13},{8,11},{8,14},{9,12}}

Cousin 494: {{1,10},{1,11},{1,12},{2,6},{2,8},{2,13},{2,14},{3,6},{3,7},{3,8},{3,9},{3,10},{4,6},{4,9},{4,11},{4,13},{5,7},{5,8},{5,10},{5,14},{6,8},{6,12},{7,8},{7,9},{7,13},{8,11},{9,12},{9,14}}

Cousin 495: {{1,10},{1,11},{1,12},{2,5},{2,9},{2,13},{2,14},{3,6},{3,7},{3,8},{3,9},{3,10},{4,6},{4,9},{4,11},{4,13},{5,7},{5,8},{5,9},{5,10},{6,12},{6,14},{7,8},{7,9},{7,13},{8,11},{8,14},{9,12}}

Cousin 496: {{1,10},{1,11},{1,12},{2,5},{2,6},{2,8},{2,9},{2,13},{3,7},{3,9},{3,10},{3,14},{4,6},{4,9},{4,11},{4,13},{5,7},{5,8},{5,9},{5,10},{6,12},{6,14},{7,8},{7,9},{7,13},{8,11},{8,14},{9,12}}

Cousin 497: {{1,10},{1,11},{1,12},{2,5},{2,6},{2,8},{2,9},{2,13},{3,6},{3,9},{3,10},{3,14},{4,6},{4,9},{4,11},{4,13},{5,7},{5,8},{5,9},{5,10},{6,8},{6,12},{7,9},{7,13},{7,14},{8,11},{8,14},{9,12}}

Cousin 498: {{1,10},{1,11},{1,12},{2,5},{2,6},{2,8},{2,9},{2,13},{3,6},{3,8},{3,10},{3,14},{4,6},{4,9},{4,11},{4,13},{5,7},{5,8},{5,9},{5,10},{6,8},{6,12},{7,8},{7,13},{7,14},{8,11},{9,12},{9,14}}

Cousin 499: {{1,10},{1,11},{1,12},{2,5},{2,6},{2,8},{2,9},{2,13},{3,6},{3,7},{3,8},{3,9},{3,10},{4,6},{4,9},{4,11},{4,13},{5,9},{5,10},{5,14},{6,8},{6,12},{7,9},{7,13},{7,14},{8,11},{8,14},{9,12}}

Cousin 500: {{1,10},{1,11},{1,12},{2,5},{2,6},{2,8},{2,9},{2,13},{3,6},{3,7},{3,8},{3,9},{3,10},{4,6},{4,9},{4,11},{4,13},{5,8},{5,10},{5,14},{6,8},{6,12},{7,8},{7,13},{7,14},{8,11},{9,12},{9,14}}

Cousin 501: {{1,2},{1,4},{1,7},{2,5},{2,6},{2,8},{2,9},{3,6},{3,7},{3,8},{3,9},{3,10},{4,6},{4,9},{4,11},{5,7},{5,8},{5,9},{5,10},{6,8},{6,12},{7,8},{7,9},{8,11},{9,12},{10,11},{10,12},{11,12}}

Cousin 502: {{1,10},{1,11},{1,12},{2,6},{2,7},{2,13},{2,14},{3,6},{3,7},{3,8},{3,9},{3,10},{4,6},{4,7},{4,11},{4,13},{5,7},{5,9},{5,10},{5,14},{6,8},{6,12},{7,8},{7,9},{8,11},{8,14},{9,12},{9,13}}

Cousin 503: {{1,10},{1,11},{1,12},{2,5},{2,7},{2,13},{2,14},{3,6},{3,7},{3,8},{3,9},{3,10},{4,6},{4,7},{4,11},{4,13},{5,7},{5,8},{5,9},{5,10},{6,12},{6,14},{7,8},{7,9},{8,11},{8,14},{9,12},{9,13}}

Cousin 504: {{1,10},{1,11},{1,12},{2,5},{2,6},{2,13},{2,14},{3,6},{3,7},{3,8},{3,9},{3,10},{4,6},{4,7},{4,11},{4,13},{5,7},{5,8},{5,9},{5,10},{6,8},{6,12},{7,9},{7,14},{8,11},{8,14},{9,12},{9,13}}

Cousin 530:  $\{\{1,10\},\{1,11\},\{1,12\},\{2,4\},\{2,5\},\{2,7\},\{2,9\},\{2,13\},\{3,6\},\{3,7\},\{3,8\},\{3,9\},\{3,10\},\{4,6\},\{4,7\},\{4,9\},\{4,11\},\{5,9\},\{5,10\},\{5,14\},\{6,12\},\{6,13\},\{7,9\},\{7,14\},$

{8,11},{8,13},{8,14},{9,12}}

Cousin 531: {{1,10},{1,11},{1,12},{2,4},{2,5},{2,7},{2,9},{2,13},{3,6},{3,7},{3,8},{3,9},{3,10},{4,6},{4,7},{4,9},{4,11},{5,8},{5,10},{5,14},{6,12},{6,13},{7,8},{7,14},{8,11},{8,13},{9,12},{9,14}}

Cousin 532: {{1,2},{1,6},{1,8},{2,4},{2,5},{2,7},{2,9},{3,6},{3,7},{3,8},{3,9},{3,10},{4,6},{4,7},{4,9},{4,11},{5,7},{5,8},{5,9},{5,10},{6,12},{7,8},{7,9},{8,11},{9,12},{10,11},{10,12},{11,12}}

Cousin 533: {{1,10},{1,11},{1,12},{2,4},{2,5},{2,6},{2,9},{2,13},{3,7},{3,9},{3,10},{3,14},{4,6},{4,7},{4,9},{4,11},{5,7},{5,8},{5,9},{5,10},{6,12},{6,14},{7,9},{7,13},{8,11},{8,13},{8,14},{9,12}}

Cousin 534: {{1,10},{1,11},{1,12},{2,4},{2,5},{2,6},{2,9},{2,13},{3,6},{3,8},{3,10},{3,14},{4,6},{4,7},{4,9},{4,11},{5,7},{5,8},{5,9},{5,10},{6,8},{6,12},{7,13},{7,14},{8,11},{8,13},{9,12},{9,14}}

Cousin 535: {{1,10},{1,11},{1,12},{2,4},{2,5},{2,6},{2,9},{2,13},{3,6},{3,7},{3,8},{3,9},{3,10},{4,6},{4,11},{4,14},{5,7},{5,8},{5,9},{5,10},{6,8},{6,12},{7,13},{7,14},{8,11},{8,13},{9,12},{9,14}}

Cousin 536: {{1,10},{1,11},{1,12},{2,4},{2,5},{2,6},{2,9},{2,13},{3,6},{3,7},{3,8},{3,9},{3,10},{4,6},{4,7},{4,9},{4,11},{5,8},{5,10},{5,14},{6,8},{6,12},{7,13},{7,14},{8,11},{8,13},{9,12},{9,14}}

Cousin 537: {{1,2},{1,7},{1,8},{2,4},{2,5},{2,6},{2,9},{3,6},{3,7},{3,8},{3,9},{3,10},{4,6},{4,7},{4,9},{4,11},{5,7},{5,8},{5,9},{5,10},{6,8},{6,12},{7,9},{8,11},{9,12},{10,11},{10,12},{11,12}}

Cousin 538: {{1,10},{1,11},{1,12},{2,4},{2,5},{2,6},{2,8},{2,13},{3,7},{3,9},{3,10},{3,14},{4,6},{4,7},{4,9},{4,11},{5,7},{5,8},{5,9},{5,10},{6,12},{6,14},{7,8},{7,13},{8,11},{8,14},{9,12},{9,13}}

Cousin 539: {{1,10},{1,11},{1,12},{2,4},{2,5},{2,6},{2,8},{2,13},{3,6},{3,9},{3,10},{3,14},{4,6},{4,7},{4,9},{4,11},{5,7},{5,8},{5,9},{5,10},{6,8},{6,12},{7,13},{7,14},{8,11},{8,14},{9,12},{9,13}}

Cousin 540: {{1,10},{1,11},{1,12},{2,4},{2,5},{2,6},{2,8},{2,13},{3,6},{3,7},{3,8},{3,9},{3,10},{4,6},{4,7},{4,9},{4,11},{5,9},{5,10},{5,14},{6,8},{6,12},{7,13},{7,14},{8,11},{8,14},{9,12},{9,13}}

Cousin 541: {{1,2},{1,7},{1,9},{2,4},{2,5},{2,6},{2,8},{3,6},{3,7},{3,8},{3,9},{3,10},{4,6},{4,7},{4,9},{4,11},{5,7},{5,8},{5,9},{5,10},{6,8},{6,12},{7,8},{8,11},{9,12},{10,11},{10,12},{11,12}}

Cousin 542: {{1,10},{1,11},{1,12},{2,4},{2,5},{2,6},{2,7},{2,8},{2,9},{3,10},{3,13},{3,14},{4,6},{4,7},{4,9},{4,11},{5,7},{5,8},{5,9},{5,10},{6,12},{6,13},{7,8},{7,14},{8,11},{8,13},{9,12},{9,14}}

Cousin 543: {{1,10},{1,11},{1,12},{2,4},{2,5},{2,6},{2,7},{2,8},{2,9},{3,7},{3,9},{3,10},{3,13},{4,6},{4,11},{4,14},{5,7},{5,8},{5,9},{5,10},{6,12},{6,13},{7,8},{7,14},{8,11},{8,13},{9,12},{9,14}}

Cousin 544: {{1,10},{1,11},{1,12},{2,4},{2,5},{2,6},{2,7},{2,8},{2,9},{3,7},{3,9},{3,10},{3,13},{4,6},{4,7},{4,9},{4,11},{5,9},{5,10},{5,14},{6,12},{6,13},{7,9},{7,14},{8,11},{8,13},{8,14},{9,12}}

Cousin 545: {{1,10},{1,11},{1,12},{2,4},{2,5},{2,6},{2,7},{2,8},{2,9},{3,7},{3,9},{3,10},{3,13},{4,6},{4,7},{4,9},{4,11},{5,8},{5,10},{5,14},{6,12},{6,13},{7,8},{7,14},{8,11},{8,13},{9,12},{9,14}}

Cousin 546: {{1,3},{1,6},{1,8},{2,4},{2,5},{2,6},{2,7},{2,8},{2,9},{3,7},{3,9},{3,10},{4,6},{4,7},{4,9},{4,11},{5,7},{5,8},{5,9},{5,10},{6,12},{7,8},{7,9},{8,11},{9,12},{10,11},{10,12},{11,12}}

Cousin 547: {{1,10},{1,11},{1,12},{2,4},{2,5},{2,6},{2,7},{2,8},{2,9},{3,6},{3,9},{3,10},{3,13},{4,6},{4,11},{4,14},{5,7},{5,8},{5,9},{5,10},{6,8},{6,12},{7,13},{7,14},{8,11},{8,13},{9,12},{9,14}}

Cousin 548: {{1,10},{1,11},{1,12},{2,4},{2,5},{2,6},{2,7},{2,8},{2,9},{3,6},{3,9},{3,10},{3,13},{4,6},{4,7},{4,9},{4,11},{5,8},{5,10},{5,14},{6,8},{6,12},{7,13},{7,14},{8,11},{8,13},{9,12},{9,14}}

Cousin 549: {{1,3},{1,7},{1,8},{2,4},{2,5},{2,6},{2,7},{2,8},{2,9},{3,6},{3,9},{3,10},{4,6},{4,7},{4,9},{4,11},{5,7},{5,8},{5,9},{5,10},{6,8},{6,12},{7,9},{8,11},{9,12},{10,11},{10,12},{11,12}}

Cousin 550: {{1,10},{1,11},{1,12},{2,4},{2,5},{2,6},{2,7},{2,8},{2,9},{3,6},{3,8},{3,10},{3,13},{4,6},{4,7},{4,9},{4,11},{5,9},{5,10},{5,14},{6,8},{6,12},{7,13},{7,14},{8,11},{8,14},{9,12},{9,13}}

Cousin 551: {{1,3},{1,7},{1,9},{2,4},{2,5},{2,6},{2,7},{2,8},{2,9},{3,6},{3,8},{3,10},{4,6},{4,7},{4,9},{4,11},{5,7},{5,8},{5,9},{5,10},{6,8},{6,12},{7,8},{8,11},{9,12},{10,11},{10,12},{11,12}}

Cousin 552: {{1,10},{1,11},{1,12},{2,4},{2,5},{2,6},{2,7},{2,8},{2,9},{3,6},{3,7},{3,8},{3,9},{3,10},{4,6},{4,11},{4,13},{5,9},{5,10},{5,14},{6,8},{6,12},{7,13},{7,14},{8,11},{8,14},{9,12},{9,13}}

Cousin 553: {{1,4},{1,7},{1,9},{2,4},{2,5},{2,6},{2,7},{2,8},{2,9},{3,6},{3,7},{3,8},{3,9},{3,10},{4,6},{4,11},{5,7},{5,8},{5,9},{5,10},{6,8},{6,12},{7,8},{8,11},{9,12},{10,11},{10,12},{11,12}}

Cousin 554: {{1,5},{1,7},{1,8},{2,4},{2,5},{2,6},{2,7},{2,8},{2,9},{3,6},{3,7},{3,8},{3,9},{3,10},{4,6},{4,7},{4,9},{4,11},{5,9},{5,10},{6,8},{6,12},{7,9},{8,11},{9,12},{10,11},{10,12},{11,12}}

Cousin 555: {{1,5},{1,7},{1,9},{2,4},{2,5},{2,6},{2,7},{2,8},{2,9},{3,6},{3,7},{3,8},{3,9},{3,10},{4,6},{4,7},{4,9},{4,11},{5,8},{5,10},{6,8},{6,12},{7,8},{8,11},{9,12},{10,11},{10,12},{11,12}}

[illegible]

Cousin 581: {{1,6},{1,9},{1,10},{1,11},{2,5},{2,9},{2,12},{2,13},{3,7},{3,8},{3,10},{3,14},{4,6},{4,9},{4,11},{4,12},{5,7},{5,8},{5,9},{5,10},{6,13},{6,14},{7,8},{7,9},{7,12},{8,11},{8,13},{9,14}}

Cousin 582: {{1,6},{1,9},{1,10},{1,11},{2,5},{2,9},{2,12},{2,13},{3,6},{3,7},{3,8},{3,9},{3,10},{4,6},{4,9},{4,11},{4,12},{5,9},{5,10},{5,14},{6,9},{6,13},{7,9},{7,12},{7,14},{8,11},{8,13},{8,14}}

Cousin 583: {{1,6},{1,9},{1,10},{1,11},{2,5},{2,9},{2,12},{2,13},{3,6},{3,7},{3,8},{3,9},{3,10},{4,6},{4,9},{4,11},{4,12},{5,8},{5,10},{5,14},{6,9},{6,13},{7,8},{7,12},{7,14},{8,11},{8,13},{9,14}}

Cousin 584: {{1,6},{1,9},{1,10},{1,11},{2,5},{2,8},{2,12},{2,13},{3,6},{3,7},{3,8},{3,9},{3,10},{4,6},{4,9},{4,11},{4,12},{5,9},{5,10},{5,14},{6,8},{6,13},{7,9},{7,12},{7,14},{8,11},{8,14},{9,13}}

Cousin 585: {{1,6},{1,9},{1,10},{1,11},{2,5},{2,8},{2,12},{2,13},{3,6},{3,7},{3,8},{3,9},{3,10},{4,6},{4,9},{4,11},{4,12},{5,8},{5,10},{5,14},{6,8},{6,13},{7,8},{7,12},{7,14},{8,11},{9,13},{9,14}}

Cousin 586: {{1,6},{1,9},{1,10},{1,11},{2,6},{2,7},{2,12},{2,13},{3,7},{3,9},{3,10},{3,14},{4,6},{4,7},{4,11},{4,12},{5,7},{5,9},{5,10},{5,13},{6,9},{6,14},{7,8},{7,9},{8,11},{8,13},{8,14},{9,12}}

Cousin 587: {{1,6},{1,9},{1,10},{1,11},{2,6},{2,7},{2,12},{2,13},{3,7},{3,8},{3,10},{3,14},{4,6},{4,7},{4,11},{4,12},{5,7},{5,9},{5,10},{5,13},{6,8},{6,14},{7,8},{7,9},{8,11},{8,13},{9,12},{9,14}}

Cousin 588: {{1,6},{1,9},{1,10},{1,11},{2,5},{2,7},{2,12},{2,13},{3,7},{3,8},{3,10},{3,14},{4,6},{4,7},{4,11},{4,12},{5,7},{5,8},{5,9},{5,10},{6,13},{6,14},{7,8},{7,9},{8,11},{8,13},{9,12},{9,14}}

Cousin 589: {{1,6},{1,9},{1,10},{1,11},{2,5},{2,7},{2,12},{2,13},{3,6},{3,9},{3,10},{3,14},{4,6},{4,7},{4,11},{4,12},{5,7},{5,8},{5,9},{5,10},{6,9},{6,13},{7,9},{7,14},{8,11},{8,13},{8,14},{9,12}}

Cousin 590: {{1,6},{1,9},{1,10},{1,11},{2,5},{2,7},{2,12},{2,13},{3,6},{3,8},{3,10},{3,14},{4,6},{4,7},{4,11},{4,12},{5,7},{5,8},{5,9},{5,10},{6,9},{6,13},{7,8},{7,14},{8,11},{8,13},{9,12},{9,14}}

Cousin 591: {{1,6},{1,9},{1,10},{1,11},{2,5},{2,7},{2,12},{2,13},{3,6},{3,7},{3,8},{3,9},{3,10},{4,6},{4,7},{4,11},{4,12},{5,9},{5,10},{5,14},{6,9},{6,13},{7,9},{7,14},{8,11},{8,13},{8,14},{9,12}}

Cousin 592: {{1,6},{1,9},{1,10},{1,11},{2,5},{2,7},{2,12},{2,13},{3,6},{3,7},{3,8},{3,9},{3,10},{4,6},{4,7},{4,11},{4,12},{5,8},{5,10},{5,14},{6,9},{6,13},{7,8},{7,14},{8,11},{8,13},{9,12},{9,14}}

Cousin 593: {{1,6},{1,9},{1,10},{1,11},{2,5},{2,6},{2,12},{2,13},{3,7},{3,9},{3,10},{3,14},{4,6},{4,7},{4,11},{4,12},{5,7},{5,8},{5,9},{5,10},{6,9},{6,14},{7,9},{7,13},{8,11},{8,13},{8,14},{9,12}}

Cousin 594: {{1,6},{1,9},{1,10},{1,11},{2,5},{2,6},{2,12},{2,13},{3,7},{3,8},{3,10},{3,14},{4,6},{4,7},{4,11},{4,12},{5,7},{5,8},{5,9},{5,10},{6,8},{6,14},{7,9},{7,13},{8,11},{8,13},{9,12},{9,14}}

Cousin 595: {{1,6},{1,9},{1,10},{1,11},{2,5},{2,6},{2,12},{2,13},{3,6},{3,8},{3,10},{3,14},{4,6},{4,7},{4,11},{4,12},{5,7},{5,8},{5,9},{5,10},{6,8},{6,9},{7,13},{7,14},{8,11},{8,13},{9,12},{9,14}}

Cousin 596: {{1,6},{1,9},{1,10},{1,11},{2,5},{2,6},{2,12},{2,13},{3,6},{3,7},{3,8},{3,9},{3,10},{4,6},{4,7},{4,11},{4,12},{5,8},{5,10},{5,14},{6,8},{6,9},{7,13},{7,14},{8,11},{8,13},{9,12},{9,14}}

Cousin 597: {{1,6},{1,9},{1,10},{1,11},{2,5},{2,6},{2,7},{2,8},{2,12},{3,10},{3,13},{3,14},{4,6},{4,7},{4,11},{4,12},{5,7},{5,8},{5,9},{5,10},{6,9},{6,13},{7,8},{7,14},{8,11},{8,13},{9,12},{9,14}}

Cousin 598: {{1,6},{1,9},{1,10},{1,11},{2,5},{2,6},{2,7},{2,8},{2,12},{3,7},{3,9},{3,10},{3,13},{4,6},{4,7},{4,11},{4,12},{5,9},{5,10},{5,14},{6,9},{6,13},{7,9},{7,14},{8,11},{8,13},{8,14},{9,12}}

Cousin 599: {{1,6},{1,9},{1,10},{1,11},{2,5},{2,6},{2,7},{2,8},{2,12},{3,7},{3,9},{3,10},{3,13},{4,6},{4,7},{4,11},{4,12},{5,8},{5,10},{5,14},{6,9},{6,13},{7,8},{7,14},{8,11},{8,13},{9,12},{9,14}}

Cousin 600: {{1,6},{1,9},{1,10},{1,11},{2,5},{2,6},{2,7},{2,8},{2,12},{3,10},{3,13},{3,14},{4,6},{4,7},{4,11},{4,12},{5,7},{5,8},{5,9},{5,10},{6,8},{6,13},{7,9},{7,14},{8,11},{8,14},{9,12},{9,13}}

Cousin 601: {{1,6},{1,9},{1,10},{1,11},{2,5},{2,6},{2,7},{2,8},{2,12},{3,7},{3,8},{3,10},{3,13},{4,6},{4,7},{4,11},{4,12},{5,9},{5,10},{5,14},{6,8},{6,13},{7,9},{7,14},{8,11},{8,14},{9,12},{9,13}}

Cousin 602: {{1,6},{1,9},{1,10},{1,11},{2,5},{2,6},{2,7},{2,8},{2,12},{3,7},{3,8},{3,10},{3,13},{4,6},{4,7},{4,11},{4,12},{5,8},{5,10},{5,14},{6,8},{6,13},{7,8},{7,14},{8,11},{9,12},{9,13},{9,14}}

Cousin 603: {{1,6},{1,9},{1,10},{1,11},{2,5},{2,6},{2,7},{2,8},{2,12},{3,6},{3,9},{3,10},{3,13},{4,6},{4,7},{4,11},{4,12},{5,8},{5,10},{5,14},{6,8},{6,9},{7,13},{7,14},{8,11},{8,13},{9,12},{9,14}}

Cousin 604: {{1,6},{1,9},{1,10},{1,11},{2,5},{2,6},{2,7},{2,8},{2,12},{3,6},{3,8},{3,10},{3,13},{4,6},{4,7},{4,11},{4,12},{5,9},{5,10},{5,14},{6,8},{6,9},{7,13},{7,14},{8,11},{8,14},{9,12},{9,13}}

Cousin 605: {{1,6},{1,9},{1,10},{1,11},{2,4},{2,7},{2,12},{2,13},{3,7},{3,9},{3,10},{3,14},{4,6},{4,7},{4,9},{4,11},{5,7},{5,9},{5,10},{5,12},{6,13},{6,14},{7,8},{7,9},{8,11},{8,12},{8,14},{9,13}}

Cousin 606: {{1,6},{1,9},{1,10},{1,11},{2,4},{2,7},{2,12},{2,13},{3,6},{3,9},{3,10},{3,14},{4,6},{4,7},{4,9},{4,11},{5,7},{5,9},{5,10},{5,12},{6,8},{6,13},{7,9},{7,14},{8,11},{8,12},{8,13},{8,14},{9,13}}

{8,11},{8,12},{8,14},{9,13}}

Cousin 607: {{1,6},{1,9},{1,10},{1,11},{2,4},{2,7},{2,12},{2,13},{3,6},{3,8},{3,10},{3,14},{4,6},{4,7},{4,9},{4,11},{5,7},{5,9},{5,10},{5,12},{6,8},{6,13},{7,8},{7,14},{8,11},{8,12},{9,13},{9,14}}

Cousin 608: {{1,6},{1,9},{1,10},{1,11},{2,4},{2,7},{2,12},{2,13},{3,6},{3,7},{3,8},{3,9},{3,10},{4,6},{4,11},{4,14},{5,7},{5,9},{5,10},{5,12},{6,8},{6,13},{7,8},{7,14},{8,11},{8,12},{9,13},{9,14}}

Cousin 609: {{1,6},{1,9},{1,10},{1,11},{2,4},{2,6},{2,12},{2,13},{3,7},{3,9},{3,10},{3,14},{4,6},{4,7},{4,9},{4,11},{5,7},{5,9},{5,10},{5,12},{6,9},{6,14},{7,8},{7,13},{8,11},{8,12},{8,14},{9,13}}

Cousin 610: {{1,6},{1,9},{1,10},{1,11},{2,4},{2,6},{2,12},{2,13},{3,7},{3,8},{3,10},{3,14},{4,6},{4,7},{4,9},{4,11},{5,7},{5,9},{5,10},{5,12},{6,8},{6,14},{7,8},{7,13},{8,11},{8,12},{9,13},{9,14}}

Cousin 611: {{1,6},{1,9},{1,10},{1,11},{2,4},{2,6},{2,12},{2,13},{3,6},{3,9},{3,10},{3,14},{4,6},{4,7},{4,9},{4,11},{5,7},{5,9},{5,10},{5,12},{6,8},{6,9},{7,13},{7,14},{8,11},{8,12},{8,14},{9,13}}

Cousin 612: {{1,6},{1,9},{1,10},{1,11},{2,4},{2,6},{2,12},{2,13},{3,6},{3,7},{3,8},{3,9},{3,10},{4,7},{4,11},{4,14},{5,7},{5,9},{5,10},{5,12},{6,8},{6,14},{7,8},{7,13},{8,11},{8,12},{9,13},{9,14}}

Cousin 613: {{1,6},{1,9},{1,10},{1,11},{2,4},{2,6},{2,7},{2,9},{2,12},{3,10},{3,13},{3,14},{4,6},{4,7},{4,9},{4,11},{5,7},{5,9},{5,10},{5,12},{6,9},{6,13},{7,8},{7,14},{8,11},{8,12},{8,13},{9,14}}

Cousin 614: {{1,6},{1,9},{1,10},{1,11},{2,4},{2,7},{2,12},{2,13},{3,7},{3,8},{3,10},{3,14},{4,6},{4,7},{4,9},{4,11},{5,7},{5,8},{5,10},{5,12},{6,13},{6,14},{7,8},{7,9},{8,11},{8,13},{9,12},{9,14}}

Cousin 615: {{1,6},{1,9},{1,10},{1,11},{2,4},{2,7},{2,12},{2,13},{3,6},{3,9},{3,10},{3,14},{4,6},{4,7},{4,9},{4,11},{5,7},{5,8},{5,10},{5,12},{6,9},{6,13},{7,9},{7,14},{8,11},{8,13},{8,14},{9,12}}

Cousin 616: {{1,6},{1,9},{1,10},{1,11},{2,4},{2,7},{2,12},{2,13},{3,6},{3,8},{3,10},{3,14},{4,6},{4,7},{4,9},{4,11},{5,7},{5,8},{5,10},{5,12},{6,9},{6,13},{7,8},{7,14},{8,11},{8,13},{9,12},{9,14}}

Cousin 617: {{1,6},{1,9},{1,10},{1,11},{2,4},{2,7},{2,12},{2,13},{3,6},{3,7},{3,8},{3,9},{3,10},{4,7},{4,11},{4,14},{5,7},{5,8},{5,10},{5,12},{6,13},{6,14},{7,8},{7,9},{8,11},{8,13},{9,12},{9,14}}

Cousin 618: {{1,6},{1,9},{1,10},{1,11},{2,4},{2,7},{2,12},{2,13},{3,6},{3,7},{3,8},{3,9},{3,10},{4,6},{4,11},{4,14},{5,7},{5,8},{5,10},{5,12},{6,9},{6,13},{7,8},{7,14},{8,11},{8,13},{9,12},{9,14}}

Cousin 619: {{1,6},{1,9},{1,10},{1,11},{2,4},{2,6},{2,12},{2,13},{3,7},{3,9},{3,10},{3,14},{4,6},{4,7},{4,9},{4,11},{5,7},{5,8},{5,10},{5,12},{6,9},{6,14},{7,9},{7,13},{8,11},{8,13},{8,14},{9,12}}

Cousin 620: {{1,6},{1,9},{1,10},{1,11},{2,4},{2,6},{2,12},{2,13},{3,7},{3,8},{3,10},{3,14},{4,6},{4,7},{4,9},{4,11},{5,7},{5,8},{5,10},{5,12},{6,8},{6,14},{7,9},{7,13},{8,11},{8,13},{9,12},{9,14}}

Cousin 621: {{1,6},{1,9},{1,10},{1,11},{2,4},{2,6},{2,12},{2,13},{3,6},{3,8},{3,10},{3,14},{4,6},{4,7},{4,9},{4,11},{5,7},{5,8},{5,10},{5,12},{6,8},{6,9},{7,13},{7,14},{8,11},{8,13},{9,12},{9,14}}

Cousin 622: {{1,6},{1,9},{1,10},{1,11},{2,4},{2,6},{2,12},{2,13},{3,6},{3,7},{3,8},{3,9},{3,10},{4,7},{4,11},{4,14},{5,7},{5,8},{5,10},{5,12},{6,8},{6,14},{7,9},{7,13},{8,11},{8,13},{9,12},{9,14}}

Cousin 623: {{1,6},{1,9},{1,10},{1,11},{2,4},{2,6},{2,7},{2,8},{2,12},{3,10},{3,13},{3,14},{4,6},{4,7},{4,9},{4,11},{5,7},{5,8},{5,10},{5,12},{6,9},{6,13},{7,8},{7,14},{8,11},{8,13},{9,12},{9,14}}

Cousin 624: {{1,6},{1,9},{1,10},{1,11},{2,4},{2,6},{2,7},{2,8},{2,12},{3,10},{3,13},{3,14},{4,6},{4,7},{4,9},{4,11},{5,7},{5,8},{5,10},{5,12},{6,8},{6,13},{7,9},{7,14},{8,11},{8,14},{9,12},{9,13}}

Cousin 625: {{1,6},{1,9},{1,10},{1,11},{2,4},{2,5},{2,12},{2,13},{3,7},{3,8},{3,10},{3,14},{4,6},{4,7},{4,9},{4,11},{5,7},{5,8},{5,9},{5,10},{6,12},{6,14},{7,8},{7,13},{8,11},{8,12},{9,13},{9,14}}

Cousin 626: {{1,6},{1,9},{1,10},{1,11},{2,4},{2,5},{2,12},{2,13},{3,6},{3,9},{3,10},{3,14},{4,6},{4,7},{4,9},{4,11},{5,7},{5,8},{5,9},{5,10},{6,9},{6,12},{7,13},{7,14},{8,11},{8,12},{8,14},{9,13}}

Cousin 627: {{1,6},{1,9},{1,10},{1,11},{2,4},{2,5},{2,12},{2,13},{3,6},{3,7},{3,8},{3,9},{3,10},{4,7},{4,11},{4,14},{5,7},{5,8},{5,9},{5,10},{6,12},{6,14},{7,8},{7,13},{8,11},{8,12},{9,13},{9,14}}

Cousin 628: {{1,6},{1,9},{1,10},{1,11},{2,4},{2,5},{2,12},{2,13},{3,6},{3,7},{3,8},{3,9},{3,10},{4,6},{4,7},{4,9},{4,11},{5,9},{5,10},{5,14},{6,9},{6,12},{7,13},{7,14},{8,11},{8,12},{8,14},{9,13}}

Cousin 629: {{1,6},{1,9},{1,10},{1,11},{2,4},{2,5},{2,7},{2,9},{2,12},{3,10},{3,13},{3,14},{4,6},{4,7},{4,9},{4,11},{5,7},{5,8},{5,9},{5,10},{6,12},{6,13},{7,9},{7,14},{8,11},{8,12},{8,14},{9,13}}

Cousin 630: {{1,6},{1,9},{1,10},{1,11},{2,4},{2,5},{2,7},{2,9},{2,12},{3,7},{3,8},{3,10},{3,13},{4,6},{4,11},{4,14},{5,7},{5,8},{5,9},{5,10},{6,12},{6,13},{7,8},{7,14},{8,11},{8,12},{9,13},{9,14}}

Cousin 631: {{1,6},{1,9},{1,10},{1,11},{2,4},{2,5},{2,7},{2,9},{2,12},{3,7},{3,8},{3,10},{3,13},{4,6},{4,7},{4,9},{4,11},{5,9},{5,10},{5,14},{6,12},{6,13},{7,9},{7,14},{8,11},{8,12},{8,14},{9,13}}

Cousin 632: {{1,6},{1,9},{1,10},{1,11},{2,4},{2,5},{2,7},{2,9},{2,12},{3,7},{3,8},{3,10},{3,13},{4,6},{4,7},{4,9},{4,11},{5,8},{5,10},{5,14},{6,12},{6,13},{7,8},{7,14},{8,11},{8,12},{9,13},{9,14}}

Cousin 633: {{1,6},{1,9},{1,10},{1,11},{2,4},{2,5},{2,7},{2,9},{2,12},{3,6},{3,9},{3,10},{3,13},{4,7},{4,11},{4,14},{5,7},{5,8},{5,9},{5,10},{6,12},{6,14},{7,9},{7,13},{8,11},{8,12},{8,13},{9,14}}

Cousin 634: {{1,6},{1,9},{1,10},{1,11},{2,4},{2,5},{2,7},{2,9},{2,12},{3,6},{3,9},{3,10},{3,13},{4,6},{4,11},{4,14},{5,7},{5,8},{5,9},{5,10},{6,9},{6,12},{7,13},{7,14},{8,11},{8,12},{8,13},{9,14}}

Cousin 635: {{1,6},{1,9},{1,10},{1,11},{2,4},{2,5},{2,7},{2,9},{2,12},{3,6},{3,9},{3,10},{3,13},{4,6},{4,7},{4,9},{4,11},{5,8},{5,10},{5,14},{6,9},{6,12},{7,13},{7,14},{8,11},{8,12},{8,13},{9,14}}

Cousin 636: {{1,6},{1,9},{1,10},{1,11},{2,4},{2,5},{2,7},{2,9},{2,12},{3,6},{3,8},{3,10},{3,13},{4,7},{4,11},{4,14},{5,7},{5,8},{5,9},{5,10},{6,12},{6,14},{7,8},{7,13},{8,11},{8,12},{9,13},{9,14}}

Cousin 637: {{1,6},{1,9},{1,10},{1,11},{2,4},{2,5},{2,7},{2,9},{2,12},{3,6},{3,8},{3,10},{3,13},{4,6},{4,7},{4,9},{4,11},{5,9},{5,10},{5,14},{6,9},{6,12},{7,13},{7,14},{8,11},{8,12},{8,14},{9,13}}

Cousin 638: {{1,6},{1,9},{1,10},{1,11},{2,4},{2,5},{2,7},{2,9},{2,12},{3,6},{3,7},{3,8},{3,9},{3,10},{4,7},{4,11},{4,13},{5,9},{5,10},{5,14},{6,12},{6,13},{7,9},{7,14},{8,11},{8,12},{8,14},{9,13}}

Cousin 639: {{1,6},{1,9},{1,10},{1,11},{2,4},{2,5},{2,7},{2,9},{2,12},{3,6},{3,7},{3,8},{3,9},{3,10},{4,7},{4,11},{4,13},{5,8},{5,10},{5,14},{6,12},{6,13},{7,8},{7,14},{8,11},{8,12},{9,13},{9,14}}

Cousin 640: {{1,6},{1,9},{1,10},{1,11},{2,4},{2,5},{2,7},{2,9},{2,12},{3,6},{3,7},{3,8},{3,9},{3,10},{4,6},{4,11},{4,13},{5,9},{5,10},{5,14},{6,9},{6,12},{7,13},{7,14},{8,11},{8,12},{8,14},{9,13}}

Cousin 641: {{1,6},{1,9},{1,10},{1,11},{2,4},{2,5},{2,12},{2,13},{3,7},{3,9},{3,10},{3,14},{4,6},{4,7},{4,9},{4,11},{5,7},{5,8},{5,9},{5,10},{6,12},{6,14},{7,9},{7,13},{8,11},{8,13},{8,14},{9,12}}

Cousin 642: {{1,6},{1,9},{1,10},{1,11},{2,4},{2,5},{2,12},{2,13},{3,6},{3,8},{3,10},{3,14},{4,6},{4,7},{4,9},{4,11},{5,7},{5,8},{5,9},{5,10},{6,8},{6,12},{7,13},{7,14},{8,11},{8,13},{9,12},{9,14}}

Cousin 643: {{1,6},{1,9},{1,10},{1,11},{2,4},{2,5},{2,12},{2,13},{3,6},{3,7},{3,8},{3,9},{3,10},{4,6},{4,11},{4,14},{5,7},{5,8},{5,9},{5,10},{6,8},{6,12},{7,13},{7,14},{8,11},{8,13},{9,12},{9,14}}

Cousin 644: {{1,6},{1,9},{1,10},{1,11},{2,4},{2,5},{2,12},{2,13},{3,6},{3,7},{3,8},{3,9},{3,10},{4,6},{4,7},{4,9},{4,11},{5,8},{5,10},{5,14},{6,8},{6,12},{7,13},{7,14},{8,11},{8,13},{9,12},{9,14}}

Cousin 645: {{1,6},{1,9},{1,10},{1,11},{2,4},{2,5},{2,7},{2,8},{2,12},{3,10},{3,13},{3,14},{4,6},{4,7},{4,9},{4,11},{5,7},{5,8},{5,9},{5,10},{6,12},{6,13},{7,8},{7,14},{8,11},{8,13},{9,12},{9,14}}

Cousin 646: {{1,6},{1,9},{1,10},{1,11},{2,4},{2,5},{2,7},{2,8},{2,12},{3,7},{3,9},{3,10},{3,13},{4,6},{4,11},{4,14},{5,7},{5,8},{5,9},{5,10},{6,12},{6,13},{7,8},{7,14},{8,11},{8,13},{9,12},{9,14}}

Cousin 647: {{1,6},{1,9},{1,10},{1,11},{2,4},{2,5},{2,7},{2,8},{2,12},{3,7},{3,9},{3,10},{3,13},{4,6},{4,7},{4,9},{4,11},{5,9},{5,10},{5,14},{6,12},{6,13},{7,9},{7,14},{8,11},{8,13},{8,14},{9,12}}

Cousin 648: {{1,6},{1,9},{1,10},{1,11},{2,4},{2,5},{2,7},{2,8},{2,12},{3,7},{3,9},{3,10},{3,13},{4,6},{4,7},{4,9},{4,11},{5,8},{5,10},{5,14},{6,12},{6,13},{7,8},{7,14},{8,11},{8,13},{9,12},{9,14}}

Cousin 649: {{1,6},{1,9},{1,10},{1,11},{2,4},{2,5},{2,7},{2,8},{2,12},{3,6},{3,9},{3,10},{3,13},{4,6},{4,11},{4,14},{5,7},{5,8},{5,9},{5,10},{6,8},{6,12},{7,13},{7,14},{8,11},{8,13},{9,12},{9,14}}

Cousin 650: {{1,6},{1,9},{1,10},{1,11},{2,4},{2,5},{2,7},{2,8},{2,12},{3,6},{3,9},{3,10},{3,13},{4,6},{4,7},{4,9},{4,11},{5,8},{5,10},{5,14},{6,8},{6,12},{7,13},{7,14},{8,11},{8,13},{9,12},{9,14}}

Cousin 651: {{1,6},{1,9},{1,10},{1,11},{2,4},{2,5},{2,7},{2,8},{2,12},{3,6},{3,8},{3,10},{3,13},{4,6},{4,7},{4,9},{4,11},{5,9},{5,10},{5,14},{6,8},{6,12},{7,13},{7,14},{8,11},{8,14},{9,12},{9,13}}

Cousin 652: {{1,6},{1,9},{1,10},{1,11},{2,4},{2,5},{2,7},{2,8},{2,12},{3,6},{3,7},{3,8},{3,9},{3,10},{4,6},{4,11},{4,13},{5,9},{5,10},{5,14},{6,8},{6,12},{7,13},{7,14},{8,11},{8,14},{9,12},{9,13}}

Cousin 653: {{1,6},{1,9},{1,10},{1,11},{2,4},{2,5},{2,6},{2,9},{2,12},{3,10},{3,13},{3,14},{4,6},{4,7},{4,9},{4,11},{5,7},{5,8},{5,9},{5,10},{6,9},{6,13},{7,12},{7,14},{8,11},{8,12},{8,13},{9,14}}

Cousin 654: {{1,6},{1,9},{1,10},{1,11},{2,4},{2,5},{2,6},{2,9},{2,12},{3,7},{3,9},{3,10},{3,13},{4,7},{4,11},{4,14},{5,7},{5,8},{5,9},{5,10},{6,13},{6,14},{7,9},{7,12},{8,11},{8,12},{8,13},{9,14}}

Cousin 655: {{1,6},{1,9},{1,10},{1,11},{2,4},{2,5},{2,6},{2,9},{2,12},{3,7},{3,9},{3,10},{3,13},{4,6},{4,11},{4,14},{5,7},{5,8},{5,9},{5,10},{6,9},{6,13},{7,12},{7,14},{8,11},{8,12},{8,13},{9,14}}

Cousin 656: {{1,6},{1,9},{1,10},{1,11},{2,4},{2,5},{2,6},{2,9},{2,12},{3,7},{3,9},{3,10},{3,13},{4,6},{4,7},{4,9},{4,11},{5,8},{5,10},{5,14},{6,9},{6,13},{7,12},{7,14},{8,11},{8,12},{8,13},{9,14}}

Cousin 657: {{1,6},{1,9},{1,10},{1,11},{2,4},{2,5},{2,6},{2,9},{2,12},{3,7},{3,8},{3,10},{3,13},{4,6},{4,11},{4,14},{5,7},{5,8},{5,9},{5,10},{6,8},{6,13},{7,12},{7,14},{8,11},{8,12},{9,13},{9,14}}

Cousin 658: {{1,6},{1,9},{1,10},{1,11},{2,4},{2,5},{2,6},{2,9},{2,12},{3,7},{3,8},{3,10},{3,13},{4,6},{4,7},{4,9},{4,11},{5,8},{5,10},{5,14},{6,8},{6,13},{7,12},{7,14},{8,11},{8,12},{9,13},{9,14}}

Cousin 659: {{1,6},{1,9},{1,10},{1,11},{2,4},{2,5},{2,6},{2,9},{2,12},{3,6},{3,8},{3,10},{3,13},{4,7},{4,11},{4,14},{5,7},{5,8},{5,9},{5,10},{6,8},{6,14},{7,12},{7,13},{8,11},{8,12},{9,13},{9,14}}

Cousin 660: {{1,6},{1,9},{1,10},{1,11},{2,4},{2,5},{2,6},{2,9},{2,12},{3,6},{3,7},{3,8},{3,9},{3,10},{4,7},{4,11},{4,13},{5,8},{5,10},{5,14},{6,8},{6,13},{7,12},{7,14},{8,11},{8,12},{9,13},{9,14}}

Cousin 661: {{1,6},{1,9},{1,10},{1,11},{2,4},{2,5},{2,6},{2,8},{2,12},{3,7},{3,9},{3,10},{3,13},{4,7},{4,11},{4,14},{5,7},{5,8},{5,9},{5,10},{6,13},{6,14},{7,8},{7,12},{8,11},{8,13},{9,12},{9,14}}

Cousin 662: {{1,6},{1,9},{1,10},{1,11},{2,4},{2,5},{2,6},{2,8},{2,12},{3,7},{3,9},{3,10},{3,13},{4,6},{4,7},{4,9},{4,11},{5,9},{5,10},{5,14},{6,9},{6,13},{7,12},{7,14},{8,11},{8,13},{8,14},{9,12}}

Cousin 663: {{1,6},{1,9},{1,10},{1,11},{2,4},{2,5},{2,6},{2,8},{2,12},{3,10},{3,13},{3,14},{4,6},{4,7},{4,9},{4,11},{5,7},{5,8},{5,9},{5,10},{6,8},{6,13},{7,12},{7,14},{8,11},{8,14},{9,12},{9,13}}

Cousin 664: {{1,6},{1,9},{1,10},{1,11},{2,4},{2,5},{2,6},{2,8},{2,12},{3,7},{3,8},{3,10},{3,13},{4,6},{4,7},{4,9},{4,11},{5,9},{5,10},{5,14},{6,8},{6,13},{7,12},{7,14},{8,11},{8,14},{9,12},{9,13}}

Cousin 665: {{1,6},{1,9},{1,10},{1,11},{2,4},{2,5},{2,6},{2,8},{2,12},{3,6},{3,9},{3,10},{3,13},{4,7},{4,11},{4,14},{5,7},{5,8},{5,9},{5,10},{6,8},{6,14},{7,12},{7,13},{8,11},{8,13},{9,12},{9,14}}

Cousin 666: {{1,6},{1,9},{1,10},{1,11},{2,4},{2,5},{2,6},{2,8},{2,12},{3,6},{3,7},{3,8},{3,9},{3,10},{4,7},{4,11},{4,13},{5,9},{5,10},{5,14},{6,8},{6,13},{7,12},{7,14},{8,11},{8,14},{9,12},{9,13}}

Cousin 667: {{1,6},{1,9},{1,10},{1,11},{2,4},{2,5},{2,6},{2,7},{2,8},{2,9},{3,10},{3,12},{3,13},{4,7},{4,11},{4,14},{5,7},{5,8},{5,9},{5,10},{6,12},{6,14},{7,8},{7,13},{8,11},{8,12},{9,13},{9,14}}

Cousin 668: {{1,6},{1,9},{1,10},{1,11},{2,4},{2,5},{2,6},{2,7},{2,8},{2,9},{3,10},{3,12},{3,13},{4,6},{4,7},{4,9},{4,11},{5,9},{5,10},{5,14},{6,9},{6,12},{7,13},{7,14},{8,11},{8,12},{8,14},{9,13}}

Cousin 669: {{1,6},{1,9},{1,10},{1,11},{2,4},{2,5},{2,6},{2,7},{2,8},{2,9},{3,7},{3,9},{3,10},{3,12},{4,6},{4,7},{4,9},{4,11},{5,7},{5,8},{5,9},{5,10},{6,9},{6,12},{7,8},{8,11},{8,12},{10,12}}

Cousin 670: {{1,6},{1,9},{1,10},{1,11},{2,4},{2,5},{2,6},{2,7},{2,8},{2,9},{3,7},{3,9},{3,10},{3,12},{4,7},{4,11},{4,13},{5,9},{5,10},{5,14},{6,12},{6,13},{7,9},{7,14},{8,11},{8,12},{8,14},{9,13}}

Cousin 671: {{1,6},{1,9},{1,10},{1,11},{2,4},{2,5},{2,6},{2,7},{2,8},{2,9},{3,7},{3,9},{3,10},{3,12},{4,7},{4,11},{4,13},{5,8},{5,10},{5,14},{6,12},{6,13},{7,8},{7,14},{8,11},{8,12},{9,13},{9,14}}

Cousin 672: {{1,6},{1,9},{1,10},{1,11},{2,4},{2,5},{2,6},{2,7},{2,8},{2,9},{3,7},{3,9},{3,10},{3,12},{4,6},{4,11},{4,13},{5,9},{5,10},{5,14},{6,9},{6,12},{7,13},{7,14},{8,11},{8,12},{8,14},{9,13}}

Cousin 673: {{1,6},{1,9},{1,10},{1,11},{2,4},{2,5},{2,6},{2,7},{2,8},{2,9},{3,10},{3,12},{3,13},{4,6},{4,11},{4,14},{5,7},{5,8},{5,9},{5,10},{6,8},{6,12},{7,13},{7,14},{8,11},{8,13},{9,12},{9,14}}

Cousin 674: {{1,6},{1,9},{1,10},{1,11},{2,4},{2,5},{2,6},{2,7},{2,8},{2,9},{3,10},{3,12},{3,13},{4,6},{4,7},{4,9},{4,11},{5,8},{5,10},{5,14},{6,8},{6,12},{7,13},{7,14},{8,11},{8,13},{9,12},{9,14}}

Cousin 675: {{1,6},{1,9},{1,10},{1,11},{2,4},{2,5},{2,6},{2,7},{2,8},{2,9},{3,7},{3,8},{3,10},{3,12},{4,6},{4,7},{4,9},{4,11},{5,7},{5,8},{5,9},{5,10},{6,8},{6,12},{7,9},{8,11},{9,12},{10,12}}

Cousin 676: {{1,6},{1,9},{1,10},{1,11},{2,4},{2,5},{2,6},{2,7},{2,8},{2,9},{3,7},{3,8},{3,10},{3,12},{4,6},{4,11},{4,13},{5,9},{5,10},{5,14},{6,8},{6,12},{7,13},{7,14},{8,11},{8,14},{9,12},{9,13}}

Cousin 677: {{1,6},{1,9},{1,10},{1,11},{2,4},{2,5},{2,6},{2,7},{2,8},{2,9},{3,6},{3,9},{3,10},{3,12},{4,7},{4,11},{4,13},{5,8},{5,10},{5,14},{6,8},{6,13},{7,12},{7,14},{8,11},{8,12},{9,13},{9,14}}

Cousin 678: {{1,6},{1,9},{1,10},{1,11},{2,4},{2,5},{2,6},{2,7},{2,8},{2,9},{3,6},{3,8},{3,10},{3,12},{4,7},{4,11},{4,13},{5,9},{5,10},{5,14},{6,8},{6,13},{7,12},{7,14},{8,11},{8,14},{9,12},{9,13}}

Cousin 679: {{1,4},{1,9},{1,10},{1,11},{2,5},{2,9},{2,12},{2,13},{3,6},{3,8},{3,10},{3,14},{4,7},{4,8},{4,9},{4,12},{5,7},{5,8},{5,9},{5,10},{6,9},{6,11},{6,12},{7,13},{7,14},{8,11},{8,13},{9,14}}

Cousin 680: {{1,4},{1,9},{1,10},{1,11},{2,5},{2,9},{2,12},{2,13},{3,6},{3,7},{3,8},{3,9},{3,10},{4,8},{4,12},{4,14},{5,7},{5,8},{5,9},{5,10},{6,9},{6,11},{6,12},{7,13},{7,14},{8,11},{8,13},{9,14}}

Cousin 681: {{1,4},{1,9},{1,10},{1,11},{2,5},{2,9},{2,12},{2,13},{3,6},{3,7},{3,8},{3,9},{3,10},{4,7},{4,8},{4,9},{4,12},{5,8},{5,10},{5,14},{6,9},{6,11},{6,12},{7,13},{7,14},{8,11},{8,13},{9,14}}

Cousin 682: {{1,4},{1,9},{1,10},{1,11},{2,5},{2,8},{2,12},{2,13},{3,6},{3,9},{3,10},{3,14},{4,7},{4,8},{4,9},{4,12},{5,7},{5,8},{5,9},{5,10},{6,9},{6,11},{6,12},{7,13},



{7,14},{8,11},{8,14},{9,13}}

Cousin 683: {{1,4},{1,9},{1,10},{1,11},{2,5},{2,8},{2,12},{2,13},{3,6},{3,7},{3,8},{3,9},{3,10},{4,9},{4,12},{4,14},{5,7},{5,8},{5,9},{5,10},{6,9},{6,11},{6,12},{7,13},{7,14},{8,11},{8,14},{9,13}}

Cousin 684: {{1,4},{1,9},{1,10},{1,11},{2,5},{2,7},{2,8},{2,9},{2,12},{3,6},{3,9},{3,10},{3,13},{4,8},{4,12},{4,14},{5,7},{5,8},{5,9},{5,10},{6,9},{6,11},{6,12},{7,13},{7,14},{8,11},{8,13},{9,14}}

Cousin 685: {{1,4},{1,9},{1,10},{1,11},{2,5},{2,7},{2,12},{2,13},{3,6},{3,9},{3,10},{3,14},{4,6},{4,7},{4,9},{4,12},{5,7},{5,8},{5,9},{5,10},{6,11},{6,13},{7,9},{7,14},{8,11},{8,12},{8,14},{9,13}}

Cousin 686: {{1,4},{1,9},{1,10},{1,11},{2,5},{2,7},{2,12},{2,13},{3,6},{3,8},{3,10},{3,14},{4,6},{4,7},{4,9},{4,12},{5,7},{5,8},{5,9},{5,10},{6,11},{6,13},{7,8},{7,14},{8,11},{8,12},{9,13},{9,14}}

Cousin 687: {{1,4},{1,9},{1,10},{1,11},{2,5},{2,7},{2,12},{2,13},{3,6},{3,7},{3,8},{3,9},{3,10},{4,6},{4,12},{4,14},{5,7},{5,8},{5,9},{5,10},{6,11},{6,13},{7,8},{7,14},{8,11},{8,12},{9,13},{9,14}}

Cousin 688: {{1,4},{1,9},{1,10},{1,11},{2,5},{2,7},{2,12},{2,13},{3,6},{3,7},{3,8},{3,9},{3,10},{4,6},{4,7},{4,9},{4,12},{5,9},{5,10},{5,14},{6,11},{6,13},{7,9},{7,14},{8,11},{8,12},{8,14},{9,13}}

Cousin 689: {{1,4},{1,9},{1,10},{1,11},{2,5},{2,7},{2,12},{2,13},{3,6},{3,7},{3,8},{3,9},{3,10},{4,6},{4,7},{4,9},{4,12},{5,8},{5,10},{5,14},{6,11},{6,13},{7,8},{7,14},{8,11},{8,12},{9,13},{9,14}}

Cousin 690: {{1,4},{1,9},{1,10},{1,11},{2,5},{2,6},{2,12},{2,13},{3,7},{3,8},{3,10},{3,14},{4,6},{4,7},{4,9},{4,12},{5,7},{5,8},{5,9},{5,10},{6,11},{6,14},{7,8},{7,13},{8,11},{8,12},{9,13},{9,14}}

Cousin 691: {{1,4},{1,9},{1,10},{1,11},{2,5},{2,6},{2,12},{2,13},{3,6},{3,9},{3,10},{3,14},{4,6},{4,7},{4,9},{4,12},{5,7},{5,8},{5,9},{5,10},{6,9},{6,11},{7,13},{7,14},{8,11},{8,12},{8,14},{9,13}}

Cousin 692: {{1,4},{1,9},{1,10},{1,11},{2,5},{2,6},{2,12},{2,13},{3,6},{3,7},{3,8},{3,9},{3,10},{4,7},{4,12},{4,14},{5,7},{5,8},{5,9},{5,10},{6,11},{6,14},{7,8},{7,13},{8,11},{8,12},{9,13},{9,14}}

Cousin 693: {{1,4},{1,9},{1,10},{1,11},{2,5},{2,6},{2,12},{2,13},{3,6},{3,7},{3,8},{3,9},{3,10},{4,6},{4,7},{4,9},{4,12},{5,9},{5,10},{5,14},{6,9},{6,11},{7,13},{7,14},{8,11},{8,12},{8,14},{9,13}}

Cousin 694: {{1,4},{1,9},{1,10},{1,11},{2,5},{2,6},{2,7},{2,9},{2,12},{3,10},{3,13},{3,14},{4,6},{4,7},{4,9},{4,12},{5,7},{5,8},{5,9},{5,10},{6,11},{6,13},{7,9},{7,14},{8,11},{8,12},{8,14},{9,13}}

Cousin 695: {{1,4},{1,9},{1,10},{1,11},{2,5},{2,6},{2,7},{2,9},{2,12},{3,7},{3,8},{3,10},{3,13},{4,6},{4,12},{4,14},{5,7},{5,8},{5,9},{5,10},{6,11},{6,13},{7,8},{7,14},{8,11},{8,12},{9,13},{9,14}}

Cousin 696: {{1,4},{1,9},{1,10},{1,11},{2,5},{2,6},{2,7},{2,9},{2,12},{3,7},{3,8},{3,10},{3,13},{4,6},{4,7},{4,9},{4,12},{5,9},{5,10},{5,14},{6,11},{6,13},{7,9},{7,14},{8,11},{8,12},{8,14},{9,13}}

Cousin 697: {{1,4},{1,9},{1,10},{1,11},{2,5},{2,6},{2,7},{2,9},{2,12},{3,7},{3,8},{3,10},{3,13},{4,6},{4,7},{4,9},{4,12},{5,8},{5,10},{5,14},{6,11},{6,13},{7,8},{7,14},{8,11},{8,12},{9,13},{9,14}}

Cousin 698: {{1,4},{1,9},{1,10},{1,11},{2,5},{2,6},{2,7},{2,9},{2,12},{3,6},{3,9},{3,10},{3,13},{4,7},{4,12},{4,14},{5,7},{5,8},{5,9},{5,10},{6,11},{6,14},{7,9},{7,13},{8,11},{8,12},{8,13},{9,14}}

Cousin 699: {{1,4},{1,9},{1,10},{1,11},{2,5},{2,6},{2,7},{2,9},{2,12},{3,6},{3,9},{3,10},{3,13},{4,6},{4,12},{4,14},{5,7},{5,8},{5,9},{5,10},{6,9},{6,11},{7,13},{7,14},{8,11},{8,12},{8,13},{9,14}}

Cousin 700: {{1,4},{1,9},{1,10},{1,11},{2,5},{2,6},{2,7},{2,9},{2,12},{3,6},{3,9},{3,10},{3,13},{4,6},{4,7},{4,9},{4,12},{5,8},{5,10},{5,14},{6,9},{6,11},{7,13},{7,14},{8,11},{8,12},{8,13},{9,14}}

Cousin 701: {{1,4},{1,9},{1,10},{1,11},{2,5},{2,6},{2,7},{2,9},{2,12},{3,6},{3,8},{3,10},{3,13},{4,7},{4,12},{4,14},{5,7},{5,8},{5,9},{5,10},{6,11},{6,14},{7,8},{7,13},{8,11},{8,12},{9,13},{9,14}}

Cousin 702: {{1,4},{1,9},{1,10},{1,11},{2,5},{2,6},{2,7},{2,9},{2,12},{3,6},{3,7},{3,8},{3,9},{3,10},{4,7},{4,12},{4,13},{5,8},{5,10},{5,14},{6,11},{6,13},{7,8},{7,14},{8,11},{8,12},{9,13},{9,14}}

Cousin 703: {{1,4},{1,9},{1,10},{1,11},{2,5},{2,6},{2,12},{2,13},{3,7},{3,8},{3,10},{3,14},{4,6},{4,7},{4,8},{4,12},{5,7},{5,8},{5,9},{5,10},{6,11},{6,14},{7,9},{7,13},{8,11},{8,13},{9,12},{9,14}}

Cousin 704: {{1,4},{1,9},{1,10},{1,11},{2,5},{2,6},{2,12},{2,13},{3,6},{3,8},{3,10},{3,14},{4,6},{4,7},{4,8},{4,12},{5,7},{5,8},{5,9},{5,10},{6,9},{6,11},{7,13},{7,14},{8,11},{8,13},{9,12},{9,14}}

Cousin 705: {{1,4},{1,9},{1,10},{1,11},{2,5},{2,6},{2,7},{2,8},{2,12},{3,10},{3,13},{3,14},{4,6},{4,7},{4,8},{4,12},{5,7},{5,8},{5,9},{5,10},{6,11},{6,13},{7,9},{7,14},{8,11},{8,14},{9,12},{9,13}}

Cousin 706: {{1,4},{1,9},{1,10},{1,11},{2,5},{2,6},{2,7},{2,8},{2,12},{3,7},{3,8},{3,10},{3,13},{4,6},{4,12},{4,14},{5,7},{5,8},{5,9},{5,10},{6,11},{6,13},{7,9},{7,14},{8,11},{8,14},{9,12},{9,13}}

Cousin 707: {{1,4},{1,9},{1,10},{1,11},{2,5},{2,6},{2,7},{2,8},{2,12},{3,7},{3,8},{3,10},{3,13},{4,6},{4,7},{4,8},{4,12},{5,9},{5,10},{5,14},{6,11},{6,13},{7,9},{7,14},{8,11},{8,14},{9,12},{9,13}}

Cousin 708: {{1,4},{1,9},{1,10},{1,11},{2,5},{2,6},{2,7},{2,8},{2,12},{3,6},{3,8},{3,10},{3,13},{4,6},{4,12},{4,14},{5,7},{5,8},{5,9},{5,10},{6,9},{6,11},{7,13},{7,14},{8,11},{8,14},{9,12},{9,13}}

Cousin 709: {{1,4},{1,9},{1,10},{1,11},{2,4},{2,5},{2,12},{2,13},{3,6},{3,8},{3,10},{3,14},{4,6},{4,7},{4,8},{4,9},{5,7},{5,8},{5,9},{5,10},{6,11},{6,12},{7,13},{7,14},{8,11},{8,13},{9,12},{9,14}}

Cousin 710: {{1,4},{1,9},{1,10},{1,11},{2,4},{2,5},{2,12},{2,13},{3,6},{3,7},{3,8},{3,9},{3,10},{4,6},{4,8},{4,14},{5,7},{5,8},{5,9},{5,10},{6,11},{6,12},{7,13},{7,14},{8,11},{8,13},{9,12},{9,14}}

Cousin 711: {{1,4},{1,9},{1,10},{1,11},{2,4},{2,5},{2,12},{2,13},{3,6},{3,7},{3,8},{3,9},{3,10},{4,6},{4,7},{4,8},{4,9},{5,8},{5,10},{5,14},{6,11},{6,12},{7,13},{7,14},{8,11},{8,13},{9,12},{9,14}}

Cousin 712: {{1,4},{1,9},{1,10},{1,11},{2,4},{2,5},{2,7},{2,8},{2,12},{3,6},{3,9},{3,10},{3,13},{4,6},{4,8},{4,14},{5,7},{5,8},{5,9},{5,10},{6,11},{6,12},{7,13},{7,14},{8,11},{8,13},{9,12},{9,14}}

Cousin 713: {{1,4},{1,9},{1,10},{1,11},{2,4},{2,5},{2,7},{2,8},{2,12},{3,6},{3,9},{3,10},{3,13},{4,6},{4,7},{4,8},{4,9},{5,8},{5,10},{5,14},{6,11},{6,12},{7,13},{7,14},{8,11},{8,13},{9,12},{9,14}}

Cousin 714: {{1,4},{1,9},{1,10},{1,11},{2,4},{2,5},{2,7},{2,8},{2,12},{3,6},{3,8},{3,10},{3,13},{4,6},{4,9},{4,14},{5,7},{5,8},{5,9},{5,10},{6,11},{6,12},{7,13},{7,14},{8,11},{8,14},{9,12},{9,13}}

Cousin 715: {{1,4},{1,9},{1,10},{1,11},{2,4},{2,5},{2,7},{2,8},{2,12},{3,6},{3,8},{3,10},{3,13},{4,6},{4,7},{4,8},{4,9},{5,9},{5,10},{5,14},{6,11},{6,12},{7,13},{7,14},{8,11},{8,14},{9,12},{9,13}}

Cousin 716: {{1,4},{1,9},{1,10},{1,11},{2,4},{2,5},{2,7},{2,8},{2,12},{3,6},{3,7},{3,8},{3,9},{3,10},{4,6},{4,9},{4,13},{5,8},{5,10},{5,14},{6,11},{6,12},{7,13},{7,14},{8,11},{8,13},{9,12},{9,14}}

Cousin 717: {{1,4},{1,9},{1,10},{1,11},{2,4},{2,5},{2,7},{2,8},{2,12},{3,6},{3,7},{3,8},{3,9},{3,10},{4,6},{4,8},{4,13},{5,9},{5,10},{5,14},{6,11},{6,12},{7,13},{7,14},{8,11},{8,14},{9,12},{9,13}}

Cousin 718: {{1,4},{1,9},{1,10},{1,11},{2,4},{2,5},{2,6},{2,9},{2,12},{3,7},{3,8},{3,10},{3,13},{4,6},{4,8},{4,14},{5,7},{5,8},{5,9},{5,10},{6,11},{6,13},{7,12},{7,14},{8,11},{8,12},{9,13},{9,14}}

Cousin 719: {{1,4},{1,9},{1,10},{1,11},{2,4},{2,5},{2,6},{2,9},{2,12},{3,7},{3,8},{3,10},{3,13},{4,6},{4,7},{4,8},{4,9},{5,8},{5,10},{5,14},{6,11},{6,13},{7,12},{7,14},{8,11},{8,12},{9,13},{9,14}}

Cousin 720: {{1,4},{1,9},{1,10},{1,11},{2,4},{2,5},{2,6},{2,9},{2,12},{3,6},{3,8},{3,10},{3,13},{4,7},{4,8},{4,14},{5,7},{5,8},{5,9},{5,10},{6,11},{6,14},{7,12},{7,13},{8,11},{8,12},{9,13},{9,14}}

Cousin 721: {{1,4},{1,9},{1,10},{1,11},{2,4},{2,5},{2,6},{2,9},{2,12},{3,6},{3,7},{3,8},{3,9},{3,10},{4,7},{4,8},{4,13},{5,8},{5,10},{5,14},{6,11},{6,13},{7,12},{7,14},{8,11},{8,12},{9,13},{9,14}}

Cousin 722: {{1,4},{1,9},{1,10},{1,11},{2,4},{2,5},{2,6},{2,8},{2,12},{3,10},{3,13},{3,14},{4,6},{4,7},{4,8},{4,9},{5,7},{5,8},{5,9},{5,10},{6,11},{6,13},{7,12},{7,14},{8,11},{8,14},{9,12},{9,13}}

Cousin 723: {{1,4},{1,9},{1,10},{1,11},{2,4},{2,5},{2,6},{2,8},{2,12},{3,7},{3,8},{3,10},{3,13},{4,6},{4,9},{4,14},{5,7},{5,8},{5,9},{5,10},{6,11},{6,13},{7,12},{7,14},{8,11},{8,14},{9,12},{9,13}}

Cousin 724: {{1,4},{1,9},{1,10},{1,11},{2,4},{2,5},{2,6},{2,8},{2,12},{3,7},{3,8},{3,10},{3,13},{4,6},{4,7},{4,8},{4,9},{5,9},{5,10},{5,14},{6,11},{6,13},{7,12},{7,14},{8,11},{8,14},{9,12},{9,13}}

Cousin 725: {{1,4},{1,9},{1,10},{1,11},{2,4},{2,5},{2,6},{2,8},{2,12},{3,6},{3,9},{3,10},{3,13},{4,7},{4,8},{4,14},{5,7},{5,8},{5,9},{5,10},{6,11},{6,14},{7,12},{7,13},{8,11},{8,13},{9,12},{9,14}}

Cousin 726: {{1,4},{1,9},{1,10},{1,11},{2,4},{2,5},{2,6},{2,8},{2,12},{3,6},{3,7},{3,8},{3,9},{3,10},{4,13},{4,14},{5,7},{5,8},{5,9},{5,10},{6,11},{6,13},{7,12},{7,14},{8,11},{8,14},{9,12},{9,13}}

Cousin 727: {{1,4},{1,9},{1,10},{1,11},{2,4},{2,5},{2,6},{2,8},{2,12},{3,6},{3,7},{3,8},{3,9},{3,10},{4,7},{4,8},{4,13},{5,9},{5,10},{5,14},{6,11},{6,13},{7,12},{7,14},{8,11},{8,14},{9,12},{9,13}}

Cousin 728: {{1,4},{1,9},{1,10},{1,11},{2,4},{2,5},{2,6},{2,7},{2,8},{2,9},{3,10},{3,12},{3,13},{4,6},{4,8},{4,14},{5,7},{5,8},{5,9},{5,10},{6,11},{6,12},{7,13},{7,14},{8,11},{8,13},{9,12},{9,14}}

Cousin 729: {{1,4},{1,9},{1,10},{1,11},{2,4},{2,5},{2,6},{2,7},{2,8},{2,9},{3,10},{3,12},{3,13},{4,6},{4,7},{4,8},{4,9},{5,8},{5,10},{5,14},{6,11},{6,12},{7,13},{7,14},{8,11},{8,13},{9,12},{9,14}}

Cousin 730: {{1,4},{1,9},{1,10},{1,11},{2,4},{2,5},{2,6},{2,7},{2,8},{2,9},{3,7},{3,8},{3,10},{3,12},{4,6},{4,7},{4,8},{4,9},{5,7},{5,8},{5,9},{5,10},{6,11},{6,12},{7,9},{8,11},{9,12},{10,12}}

Cousin 731: {{1,4},{1,9},{1,10},{1,11},{2,4},{2,5},{2,6},{2,7},{2,8},{2,9},{3,6},{3,8},{3,10},{3,12},{4,13},{4,14},{5,7},{5,8},{5,9},{5,10},{6,11},{6,13},{7,12},{7,14},{8,11},{8,14},{9,12},{9,13}}

Cousin 732: {{1,4},{1,6},{1,8},{1,9},{1,10},{2,5},{2,7},{2,11},{2,12},{3,10},{3,13},{3,14},{4,6},{4,7},{4,9},{4,11},{5,7},{5,8},{5,9},{5,10},{6,12},{6,13},{7,8},{7,14},{8,11},{8,13},{9,12},{9,14}}

Cousin 733: {{1,4},{1,6},{1,8},{1,9},{1,10},{2,5},{2,7},{2,11},{2,12},{3,7},{3,9},{3,10},{3,13},{4,6},{4,11},{4,14},{5,7},{5,8},{5,9},{5,10},{6,12},{6,13},{7,8},{7,14},{8,11},{8,13},{9,12},{9,14}}

Cousin 734: {{1,4},{1,6},{1,8},{1,9},{1,10},{2,5},{2,6},{2,11},{2,12},{3,7},{3,9},{3,10},{3,13},{4,7},{4,11},{4,14},{5,7},{5,8},{5,9},{5,10},{6,13},{6,14},{7,8},{7,12},{8,11},{8,13},{9,12},{9,14}}

Cousin 735: {{1,4},{1,6},{1,8},{1,9},{1,10},{2,5},{2,6},{2,11},{2,12},{3,10},{3,13},{3,14},{4,6},{4,7},{4,9},{4,11},{5,7},{5,8},{5,9},{5,10},{6,8},{6,13},{7,12},{7,14},{8,11},{8,14},{9,12},{9,13}}

Cousin 736: {{1,4},{1,6},{1,8},{1,9},{1,10},{2,5},{2,6},{2,7},{2,9},{2,11},{3,7},{3,9},{3,10},{3,12},{4,6},{4,7},{4,9},{4,11},{5,7},{5,8},{5,9},{5,10},{6,9},{6,12},{7,8},{8,11},{8,12},{10,12}}

Cousin 737: {{1,4},{1,6},{1,8},{1,9},{1,10},{2,4},{2,5},{2,11},{2,12},{3,10},{3,13},{3,14},{4,6},{4,7},{4,8},{4,9},{5,7},{5,8},{5,9},{5,10},{6,11},{6,13},{7,12},{7,14},{8,11},{8,14},{9,12},{9,13}}

Cousin 738: {{1,4},{1,6},{1,8},{1,9},{1,10},{2,4},{2,5},{2,11},{2,12},{3,7},{3,8},{3,10},{3,13},{4,6},{4,9},{4,14},{5,7},{5,8},{5,9},{5,10},{6,11},{6,13},{7,12},{7,14},{8,11},{8,14},{9,12},{9,13}}

Cousin 739: {{1,4},{1,6},{1,8},{1,9},{1,10},{2,4},{2,5},{2,11},{2,12},{3,6},{3,9},{3,10},{3,13},{4,7},{4,8},{4,14},{5,7},{5,8},{5,9},{5,10},{6,11},{6,14},{7,12},{7,13},{8,11},{8,13},{9,12},{9,14}}

Cousin 740: {{1,4},{1,6},{1,8},{1,9},{1,10},{2,4},{2,5},{2,11},{2,12},{3,6},{3,7},{3,8},{3,9},{3,10},{4,13},{4,14},{5,7},{5,8},{5,9},{5,10},{6,11},{6,13},{7,12},{7,14},{8,11},{8,14},{9,12},{9,13}}

Cousin 741: {{1,4},{1,6},{1,8},{1,9},{1,10},{2,4},{2,5},{2,7},{2,9},{2,11},{3,10},{3,12},{3,13},{4,6},{4,8},{4,14},{5,7},{5,8},{5,9},{5,10},{6,11},{6,12},{7,13},{7,14},{8,11},{8,13},{9,12},{9,14}}

Cousin 742: {{1,4},{1,6},{1,8},{1,9},{1,10},{2,4},{2,5},{2,7},{2,9},{2,11},{3,7},{3,8},{3,10},{3,12},{4,6},{4,7},{4,8},{4,9},{5,7},{5,8},{5,9},{5,10},{6,11},{6,12},{7,9},{8,11},{9,12},{10,12}}

Cousin 743: {{1,4},{1,6},{1,8},{1,9},{1,10},{2,4},{2,5},{2,6},{2,9},{2,11},{3,10},{3,12},{3,13},{4,7},{4,8},{4,14},{5,7},{5,8},{5,9},{5,10},{6,12},{6,14},{7,11},{7,13},{8,11},{8,12},{9,13},{9,14}}

Cousin 744: {{1,4},{1,6},{1,8},{1,9},{1,10},{2,4},{2,5},{2,6},{2,9},{2,11},{3,7},{3,9},{3,10},{3,12},{4,6},{4,7},{4,8},{4,9},{5,7},{5,8},{5,9},{5,10},{6,9},{6,12},{7,11},{8,11},{8,12},{10,12}}

Cousin 745: {{1,5},{1,6},{1,10},{1,11},{2,6},{2,7},{2,12},{2,13},{3,5},{3,7},{3,10},{3,14},{4,6},{4,7},{4,11},{4,12},{5,7},{5,8},{5,13},{6,8},{6,14},{7,8},{7,9},{8,10},{8,12},{9,11},{9,13},{9,14}}

Cousin 746: {{1,5},{1,6},{1,10},{1,11},{2,6},{2,7},{2,12},{2,13},{3,5},{3,6},{3,10},{3,14},{4,6},{4,7},{4,11},{4,12},{5,7},{5,8},{5,13},{6,8},{6,9},{7,8},{7,14},{8,10},{8,12},{9,11},{9,13},{9,14}}

Cousin 747: {{1,5},{1,6},{1,10},{1,11},{2,6},{2,7},{2,12},{2,13},{3,5},{3,6},{3,7},{3,9},{3,10},{4,6},{4,7},{4,11},{4,12},{5,13},{5,14},{6,8},{6,9},{7,9},{7,14},{8,10},{8,12},{8,14},{9,11},{9,13}}

Cousin 748: {{1,5},{1,6},{1,10},{1,11},{2,5},{2,7},{2,12},{2,13},{3,6},{3,7},{3,10},{3,14},{4,6},{4,7},{4,11},{4,12},{5,7},{5,8},{5,14},{6,8},{6,13},{7,8},{7,9},{8,10},{8,12},{9,11},{9,13},{9,14}}

Cousin 749: {{1,5},{1,6},{1,10},{1,11},{2,5},{2,7},{2,12},{2,13},{3,5},{3,6},{3,7},{3,9},{3,10},{4,6},{4,7},{4,11},{4,12},{5,9},{5,14},{6,8},{6,13},{7,9},{7,14},{8,10},{8,12},{8,14},{9,11},{9,13}}

Cousin 750: {{1,5},{1,6},{1,10},{1,11},{2,5},{2,7},{2,12},{2,13},{3,5},{3,6},{3,7},{3,9},{3,10},{4,6},{4,7},{4,11},{4,12},{5,8},{5,14},{6,8},{6,13},{7,8},{7,14},{8,10},{8,12},{9,11},{9,13},{9,14}}

Cousin 751: {{1,5},{1,6},{1,10},{1,11},{2,5},{2,6},{2,12},{2,13},{3,6},{3,7},{3,10},{3,14},{4,6},{4,7},{4,11},{4,12},{5,7},{5,8},{5,14},{6,8},{6,9},{7,8},{7,13},{8,10},{8,12},{9,11},{9,13},{9,14}}

Cousin 752: {{1,5},{1,6},{1,10},{1,11},{2,5},{2,6},{2,12},{2,13},{3,5},{3,6},{3,7},{3,9},{3,10},{4,6},{4,7},{4,11},{4,12},{5,9},{5,14},{6,8},{6,9},{7,13},{7,14},{8,10},{8,12},{8,14},{9,11},{9,13}}

Cousin 753: {{1,5},{1,6},{1,10},{1,11},{2,4},{2,7},{2,12},{2,13},{3,6},{3,7},{3,10},{3,14},{4,6},{4,7},{4,8},{4,11},{5,7},{5,12},{5,14},{6,8},{6,13},{7,8},{7,9},{8,10},{8,12},{9,11},{9,13},{9,14}}

Cousin 754: {{1,5},{1,6},{1,10},{1,11},{2,4},{2,7},{2,12},{2,13},{3,5},{3,6},{3,10},{3,14},{4,6},{4,7},{4,8},{4,11},{5,7},{5,9},{5,12},{6,8},{6,13},{7,8},{7,14},{8,10},{8,12},{9,11},{9,13},{9,14}}

Cousin 755: {{1,5},{1,6},{1,10},{1,11},{2,4},{2,7},{2,12},{2,13},{3,5},{3,6},{3,7},{3,9},{3,10},{4,7},{4,11},{4,14},{5,7},{5,9},{5,12},{6,13},{6,14},{7,8},{7,9},{8,10},{8,12},{8,14},{9,11},{9,13}}

Cousin 756: {{1,5},{1,6},{1,10},{1,11},{2,4},{2,7},{2,12},{2,13},{3,5},{3,6},{3,7},{3,9},{3,10},{4,6},{4,11},{4,14},{5,7},{5,9},{5,12},{6,8},{6,13},{7,9},{7,14},{8,10},{8,12},{8,14},{9,11},{9,13}}

Cousin 757: {{1,5},{1,6},{1,10},{1,11},{2,4},{2,7},{2,12},{2,13},{3,5},{3,6},{3,7},{3,9},{3,10},{4,6},{4,7},{4,8},{4,11},{5,12},{5,14},{6,8},{6,13},{7,8},{7,14},{8,10},{8,12},{9,11},{9,13},{9,14}}

Cousin 758: {{1,5},{1,6},{1,10},{1,11},{2,4},{2,6},{2,12},{2,13},{3,6},{3,7},{3,10},{3,14},{4,6},{4,7},{4,8},{4,11},{5,7},{5,12},{5,14},{6,8},{6,9},{7,8},{7,13},{8,10},{8,12},{9,11},{9,13},{9,14}}

{8,12},{9,11},{9,13},{9,14}}

Cousin 759: {{1,5},{1,6},{1,10},{1,11},{2,4},{2,6},{2,12},{2,13},{3,5},{3,7},{3,10},{3,14},{4,6},{4,7},{4,8},{4,11},{5,7},{5,9},{5,12},{6,8},{6,14},{7,8},{7,13},{8,10},{8,12},{9,11},{9,13},{9,14}}

Cousin 760: {{1,5},{1,6},{1,10},{1,11},{2,4},{2,6},{2,12},{2,13},{3,5},{3,6},{3,7},{3,9},{3,10},{4,7},{4,11},{4,14},{5,7},{5,9},{5,12},{6,9},{6,14},{7,8},{7,13},{8,10},{8,12},{8,14},{9,11},{9,13}}

Cousin 761: {{1,5},{1,6},{1,10},{1,11},{2,4},{2,6},{2,12},{2,13},{3,5},{3,6},{3,7},{3,9},{3,10},{4,6},{4,11},{4,14},{5,7},{5,9},{5,12},{6,8},{6,9},{7,13},{7,14},{8,10},{8,12},{8,14},{9,11},{9,13}}

Cousin 762: {{1,5},{1,6},{1,10},{1,11},{2,4},{2,6},{2,7},{2,9},{2,12},{3,5},{3,7},{3,10},{3,13},{4,7},{4,11},{4,14},{5,7},{5,9},{5,12},{6,13},{6,14},{7,8},{7,9},{8,10},{8,12},{8,14},{9,11},{9,13}}

Cousin 763: {{1,5},{1,6},{1,10},{1,11},{2,4},{2,6},{2,7},{2,9},{2,12},{3,5},{3,7},{3,10},{3,13},{4,6},{4,11},{4,14},{5,7},{5,9},{5,12},{6,8},{6,13},{7,9},{7,14},{8,10},{8,12},{8,14},{9,11},{9,13}}

Cousin 764: {{1,5},{1,6},{1,10},{1,11},{2,4},{2,6},{2,7},{2,9},{2,12},{3,5},{3,7},{3,10},{3,13},{4,6},{4,7},{4,8},{4,11},{5,12},{5,14},{6,8},{6,13},{7,8},{7,14},{8,10},{8,12},{9,11},{9,13},{9,14}}

Cousin 765: {{1,5},{1,6},{1,10},{1,11},{2,4},{2,6},{2,7},{2,9},{2,12},{3,5},{3,6},{3,10},{3,13},{4,7},{4,11},{4,14},{5,7},{5,9},{5,12},{6,9},{6,14},{7,8},{7,13},{8,10},{8,12},{8,14},{9,11},{9,13}}

Cousin 766: {{1,5},{1,6},{1,10},{1,11},{2,4},{2,6},{2,7},{2,9},{2,12},{3,5},{3,6},{3,10},{3,13},{4,6},{4,11},{4,14},{5,7},{5,9},{5,12},{6,8},{6,9},{7,13},{7,14},{8,10},{8,12},{8,14},{9,11},{9,13}}

Cousin 767: {{1,5},{1,6},{1,10},{1,11},{2,4},{2,6},{2,7},{2,9},{2,12},{3,5},{3,6},{3,7},{3,9},{3,10},{4,7},{4,11},{4,13},{5,12},{5,14},{6,9},{6,13},{7,8},{7,14},{8,10},{8,12},{8,13},{9,11},{9,14}}

Cousin 768: {{1,5},{1,6},{1,10},{1,11},{2,4},{2,6},{2,7},{2,9},{2,12},{3,5},{3,6},{3,7},{3,9},{3,10},{4,6},{4,11},{4,13},{5,12},{5,14},{6,8},{6,9},{7,13},{7,14},{8,10},{8,12},{8,13},{9,11},{9,14}}

Cousin 769: {{1,5},{1,6},{1,10},{1,11},{2,4},{2,7},{2,12},{2,13},{3,5},{3,7},{3,10},{3,14},{4,6},{4,7},{4,8},{4,11},{5,7},{5,8},{5,12},{6,13},{6,14},{7,8},{7,9},{8,10},{8,13},{9,11},{9,12},{9,14}}

Cousin 770: {{1,5},{1,6},{1,10},{1,11},{2,4},{2,7},{2,12},{2,13},{3,5},{3,6},{3,7},{3,9},{3,10},{4,6},{4,11},{4,14},{5,7},{5,8},{5,12},{6,9},{6,13},{7,9},{7,14},{8,10},{8,13},{8,14},{9,11},{9,12}}

Cousin 771: {{1,5},{1,6},{1,10},{1,11},{2,4},{2,7},{2,12},{2,13},{3,5},{3,6},{3,7},{3,9},{3,10},{4,6},{4,7},{4,8},{4,11},{5,12},{5,14},{6,9},{6,13},{7,9},{7,14},{8,10},{8,13},{8,14},{9,11},{9,12}}

Cousin 772: {{1,5},{1,6},{1,10},{1,11},{2,4},{2,6},{2,12},{2,13},{3,5},{3,7},{3,10},{3,14},{4,6},{4,7},{4,8},{4,11},{5,7},{5,8},{5,12},{6,8},{6,14},{7,9},{7,13},{8,10},{8,13},{9,11},{9,12},{9,14}}

Cousin 773: {{1,5},{1,6},{1,10},{1,11},{2,4},{2,6},{2,12},{2,13},{3,5},{3,6},{3,7},{3,9},{3,10},{4,7},{4,11},{4,14},{5,7},{5,8},{5,12},{6,9},{6,14},{7,9},{7,13},{8,10},{8,13},{8,14},{9,11},{9,12}}

Cousin 774: {{1,5},{1,6},{1,10},{1,11},{2,4},{2,6},{2,7},{2,8},{2,12},{3,5},{3,7},{3,10},{3,13},{4,7},{4,11},{4,14},{5,7},{5,8},{5,12},{6,13},{6,14},{7,8},{7,9},{8,10},{8,14},{9,11},{9,12},{9,13}}

Cousin 775: {{1,5},{1,6},{1,10},{1,11},{2,4},{2,6},{2,7},{2,8},{2,12},{3,5},{3,7},{3,10},{3,13},{4,6},{4,11},{4,14},{5,7},{5,8},{5,12},{6,8},{6,13},{7,9},{7,14},{8,10},{8,14},{9,11},{9,12},{9,13}}

Cousin 776: {{1,5},{1,6},{1,10},{1,11},{2,4},{2,6},{2,7},{2,8},{2,12},{3,5},{3,7},{3,10},{3,13},{4,6},{4,7},{4,8},{4,11},{5,12},{5,14},{6,8},{6,13},{7,9},{7,14},{8,10},{8,14},{9,11},{9,12},{9,13}}

Cousin 777: {{1,5},{1,6},{1,10},{1,11},{2,4},{2,6},{2,7},{2,8},{2,12},{3,5},{3,6},{3,10},{3,13},{4,7},{4,11},{4,14},{5,7},{5,8},{5,12},{6,9},{6,14},{7,8},{7,13},{8,10},{8,14},{9,11},{9,12},{9,13}}

Cousin 778: {{1,5},{1,6},{1,10},{1,11},{2,4},{2,6},{2,7},{2,8},{2,12},{3,5},{3,6},{3,10},{3,13},{4,6},{4,11},{4,14},{5,7},{5,8},{5,12},{6,8},{6,9},{7,13},{7,14},{8,10},{8,14},{9,11},{9,12},{9,13}}

Cousin 779: {{1,5},{1,6},{1,10},{1,11},{2,4},{2,6},{2,7},{2,8},{2,12},{3,5},{3,6},{3,10},{3,13},{4,6},{4,7},{4,8},{4,11},{5,12},{5,14},{6,8},{6,9},{7,13},{7,14},{8,10},{8,14},{9,11},{9,12},{9,13}}

Cousin 780: {{1,5},{1,6},{1,10},{1,11},{2,4},{2,6},{2,7},{2,8},{2,12},{3,5},{3,6},{3,7},{3,9},{3,10},{4,7},{4,11},{4,13},{5,12},{5,14},{6,9},{6,13},{7,9},{7,14},{8,10},{8,13},{8,14},{9,11},{9,12}}

Cousin 781: {{1,5},{1,6},{1,10},{1,11},{2,4},{2,5},{2,12},{2,13},{3,6},{3,7},{3,10},{3,14},{4,6},{4,7},{4,8},{4,11},{5,7},{5,8},{5,14},{6,9},{6,12},{7,8},{7,13},{8,10},{8,12},{9,11},{9,13},{9,14}}

Cousin 782: {{1,5},{1,6},{1,10},{1,11},{2,4},{2,5},{2,12},{2,13},{3,5},{3,7},{3,10},{3,14},{4,6},{4,7},{4,8},{4,11},{5,7},{5,8},{5,9},{6,12},{6,14},{7,8},{7,13},{8,10},{8,12},{9,11},{9,13},{9,14}}

Cousin 783: {{1,5},{1,6},{1,10},{1,11},{2,4},{2,5},{2,7},{2,9},{2,12},{3,6},{3,7},{3,10},{3,13},{4,6},{4,11},{4,14},{5,7},{5,8},{5,13},{6,9},{6,12},{7,9},{7,14},{8,10},{8,12},{8,14},{9,11},{9,13}}

Cousin 784: {{1,5},{1,6},{1,10},{1,11},{2,4},{2,5},{2,7},{2,9},{2,12},{3,6},{3,7},{3,10},{3,13},{4,6},{4,7},{4,8},{4,11},{5,13},{5,14},{6,9},{6,12},{7,9},{7,14},{8,10},{8,12},{8,14},{9,11},{9,13}}

Cousin 785: {{1,5},{1,6},{1,10},{1,11},{2,4},{2,5},{2,7},{2,9},{2,12},{3,5},{3,7},{3,10},{3,13},{4,6},{4,11},{4,14},{5,7},{5,8},{5,9},{6,12},{6,13},{7,9},{7,14},{8,10},{8,12},{8,14},{9,11},{9,13}}

Cousin 786: {{1,5},{1,6},{1,10},{1,11},{2,4},{2,5},{2,7},{2,9},{2,12},{3,5},{3,7},{3,10},{3,13},{4,6},{4,7},{4,8},{4,11},{5,9},{5,14},{6,12},{6,13},{7,9},{7,14},{8,10},{8,12},{8,14},{9,11},{9,13}}

Cousin 787: {{1,5},{1,6},{1,10},{1,11},{2,4},{2,5},{2,7},{2,9},{2,12},{3,5},{3,7},{3,10},{3,13},{4,6},{4,7},{4,8},{4,11},{5,8},{5,14},{6,12},{6,13},{7,8},{7,14},{8,10},{8,12},{9,11},{9,13},{9,14}}

Cousin 788: {{1,5},{1,6},{1,10},{1,11},{2,4},{2,5},{2,7},{2,9},{2,12},{3,5},{3,6},{3,7},{3,9},{3,10},{4,6},{4,11},{4,13},{5,8},{5,14},{6,9},{6,12},{7,13},{7,14},{8,10},{8,12},{8,13},{9,11},{9,14}}

Cousin 789: {{1,5},{1,6},{1,10},{1,11},{2,4},{2,5},{2,12},{2,13},{3,6},{3,7},{3,10},{3,14},{4,6},{4,7},{4,8},{4,11},{5,7},{5,8},{5,14},{6,8},{6,12},{7,9},{7,13},{8,10},{8,13},{9,11},{9,12},{9,14}}

Cousin 790: {{1,5},{1,6},{1,10},{1,11},{2,4},{2,5},{2,12},{2,13},{3,5},{3,6},{3,7},{3,9},{3,10},{4,7},{4,11},{4,14},{5,7},{5,8},{5,9},{6,12},{6,14},{7,9},{7,13},{8,10},{8,13},{8,14},{9,11},{9,12}}

Cousin 791: {{1,5},{1,6},{1,10},{1,11},{2,4},{2,5},{2,7},{2,8},{2,12},{3,6},{3,7},{3,10},{3,13},{4,7},{4,11},{4,14},{5,7},{5,8},{5,13},{6,12},{6,14},{7,8},{7,9},{8,10},{8,14},{9,11},{9,12},{9,13}}

Cousin 792: {{1,5},{1,6},{1,10},{1,11},{2,4},{2,5},{2,7},{2,8},{2,12},{3,6},{3,7},{3,10},{3,13},{4,6},{4,11},{4,14},{5,7},{5,8},{5,13},{6,8},{6,12},{7,9},{7,14},{8,10},{8,14},{9,11},{9,12},{9,13}}

Cousin 793: {{1,5},{1,6},{1,10},{1,11},{2,4},{2,5},{2,7},{2,8},{2,12},{3,6},{3,7},{3,10},{3,13},{4,6},{4,7},{4,8},{4,11},{5,13},{5,14},{6,8},{6,12},{7,9},{7,14},{8,10},{8,14},{9,11},{9,12},{9,13}}

Cousin 794: {{1,5},{1,6},{1,10},{1,11},{2,4},{2,5},{2,7},{2,8},{2,12},{3,5},{3,6},{3,7},{3,9},{3,10},{4,7},{4,11},{4,13},{5,9},{5,14},{6,12},{6,13},{7,9},{7,14},{8,10},{8,13},{8,14},{9,11},{9,12}}

Cousin 795: {{1,5},{1,6},{1,10},{1,11},{2,4},{2,5},{2,7},{2,8},{2,12},{3,5},{3,6},{3,7},{3,9},{3,10},{4,7},{4,11},{4,13},{5,8},{5,14},{6,12},{6,13},{7,8},{7,14},{8,10},{8,13},{9,11},{9,12},{9,14}}

Cousin 796: {{1,5},{1,6},{1,10},{1,11},{2,4},{2,5},{2,6},{2,9},{2,12},{3,6},{3,7},{3,10},{3,13},{4,7},{4,11},{4,14},{5,7},{5,8},{5,13},{6,9},{6,14},{7,9},{7,12},{8,10},{8,12},{8,14},{9,11},{9,13}}

Cousin 797: {{1,5},{1,6},{1,10},{1,11},{2,4},{2,5},{2,6},{2,9},{2,12},{3,5},{3,7},{3,10},{3,13},{4,7},{4,11},{4,14},{5,7},{5,8},{5,9},{6,13},{6,14},{7,9},{7,12},{8,10},{8,12},{8,14},{9,11},{9,13}}

Cousin 798: {{1,5},{1,6},{1,10},{1,11},{2,4},{2,5},{2,6},{2,9},{2,12},{3,5},{3,7},{3,10},{3,13},{4,6},{4,7},{4,8},{4,11},{5,8},{5,14},{6,8},{6,13},{7,12},{7,14},{8,10},{8,12},{9,11},{9,13},{9,14}}

Cousin 799: {{1,5},{1,6},{1,10},{1,11},{2,4},{2,5},{2,6},{2,9},{2,12},{3,5},{3,6},{3,7},{3,9},{3,10},{4,7},{4,11},{4,13},{5,8},{5,14},{6,9},{6,13},{7,12},{7,14},{8,10},{8,12},{8,13},{9,11},{9,14}}

Cousin 800: {{1,5},{1,6},{1,10},{1,11},{2,4},{2,5},{2,6},{2,8},{2,12},{3,6},{3,7},{3,10},{3,13},{4,7},{4,11},{4,14},{5,7},{5,8},{5,13},{6,9},{6,14},{7,8},{7,12},{8,10},{8,14},{9,11},{9,12},{9,13}}

Cousin 801: {{1,5},{1,6},{1,10},{1,11},{2,4},{2,5},{2,6},{2,8},{2,12},{3,6},{3,7},{3,10},{3,13},{4,6},{4,11},{4,14},{5,7},{5,8},{5,13},{6,8},{6,9},{7,12},{7,14},{8,10},{8,14},{9,11},{9,12},{9,13}}

Cousin 802: {{1,5},{1,6},{1,10},{1,11},{2,4},{2,5},{2,6},{2,8},{2,12},{3,6},{3,7},{3,10},{3,13},{4,6},{4,7},{4,8},{4,11},{5,13},{5,14},{6,8},{6,9},{7,12},{7,14},{8,10},{8,14},{9,11},{9,12},{9,13}}

Cousin 803: {{1,5},{1,6},{1,10},{1,11},{2,4},{2,5},{2,6},{2,8},{2,12},{3,5},{3,7},{3,10},{3,13},{4,7},{4,11},{4,14},{5,7},{5,8},{5,9},{6,13},{6,14},{7,8},{7,12},{8,10},{8,14},{9,11},{9,12},{9,13}}

Cousin 804: {{1,5},{1,6},{1,10},{1,11},{2,4},{2,5},{2,6},{2,8},{2,12},{3,5},{3,7},{3,10},{3,13},{4,6},{4,11},{4,14},{5,7},{5,8},{5,9},{6,8},{6,13},{7,12},{7,14},{8,10},{8,14},{9,11},{9,12},{9,13}}

Cousin 805: {{1,5},{1,6},{1,10},{1,11},{2,4},{2,5},{2,6},{2,8},{2,12},{3,5},{3,7},{3,10},{3,13},{4,6},{4,7},{4,8},{4,11},{5,9},{5,14},{6,8},{6,13},{7,12},{7,14},{8,10},{8,14},{9,11},{9,12},{9,13}}

Cousin 806: {{1,5},{1,6},{1,10},{1,11},{2,4},{2,5},{2,6},{2,8},{2,12},{3,5},{3,6},{3,7},{3,9},{3,10},{4,7},{4,11},{4,13},{5,9},{5,14},{6,9},{6,13},{7,12},{7,14},{8,10},{8,13},{8,14},{9,11},{9,12}}

Cousin 807: {{1,5},{1,6},{1,10},{1,11},{2,4},{2,5},{2,6},{2,7},{2,8},{2,9},{3,6},{3,7},{3,10},{3,12},{4,7},{4,11},{4,13},{5,12},{5,14},{6,9},{6,13},{7,9},{7,14},{8,10},{8,13},{8,14},{9,11},{9,12}}

Cousin 808: {{1,5},{1,6},{1,10},{1,11},{2,4},{2,5},{2,6},{2,7},{2,8},{2,9},{3,5},{3,6},{3,10},{3,12},{4,7},{4,11},{4,13},{5,9},{5,14},{6,9},{6,13},{7,12},{7,14},{8,10},{8,13},{8,14},{9,11},{9,12}}

Cousin 809: {{1,4},{1,6},{1,10},{1,11},{2,5},{2,7},{2,12},{2,13},{3,5},{3,6},{3,7},{3,9},{3,10},{4,6},{4,12},{4,14},{5,7},{5,8},{5,11},{6,8},{6,13},{7,8},{7,14},{8,10},{8,12},{9,11},{9,13},{9,14}}

Cousin 810: {{1,4},{1,6},{1,10},{1,11},{2,5},{2,6},{2,12},{2,13},{3,5},{3,7},{3,10},{3,14},{4,6},{4,7},{4,9},{4,12},{5,7},{5,8},{5,11},{6,8},{6,14},{7,8},{7,13},{8,10},{8,12},{9,11},{9,13},{9,14}}

Cousin 811: {{1,4},{1,6},{1,10},{1,11},{2,5},{2,6},{2,12},{2,13},{3,5},{3,6},{3,7},{3,9},{3,10},{4,7},{4,12},{4,14},{5,7},{5,8},{5,11},{6,8},{6,14},{7,8},{7,13},{8,10},{8,12},{9,11},{9,13},{9,14}}

Cousin 812: {{1,4},{1,6},{1,10},{1,11},{2,5},{2,7},{2,12},{2,13},{3,5},{3,7},{3,10},{3,14},{4,6},{4,7},{4,8},{4,12},{5,7},{5,8},{5,11},{6,13},{6,14},{7,8},{7,9},{8,10},{8,13},{9,11},{9,12},{9,14}}

Cousin 813: {{1,4},{1,6},{1,10},{1,11},{2,5},{2,7},{2,12},{2,13},{3,5},{3,6},{3,7},{3,9},{3,10},{4,6},{4,12},{4,14},{5,7},{5,8},{5,11},{6,9},{6,13},{7,9},{7,14},{8,10},{8,13},{8,14},{9,11},{9,12}}

Cousin 814: {{1,4},{1,6},{1,10},{1,11},{2,5},{2,6},{2,12},{2,13},{3,5},{3,6},{3,7},{3,9},{3,10},{4,7},{4,12},{4,14},{5,7},{5,8},{5,11},{6,9},{6,14},{7,9},{7,13},{8,10},{8,13},{8,14},{9,11},{9,12}}

Cousin 815: {{1,4},{1,6},{1,10},{1,11},{2,4},{2,7},{2,12},{2,13},{3,5},{3,6},{3,7},{3,9},{3,10},{4,7},{4,9},{4,14},{5,7},{5,11},{5,12},{6,13},{6,14},{7,8},{7,9},{8,10},{8,12},{8,14},{9,11},{9,13}}

Cousin 816: {{1,4},{1,6},{1,10},{1,11},{2,4},{2,7},{2,12},{2,13},{3,5},{3,6},{3,7},{3,9},{3,10},{4,6},{4,9},{4,14},{5,7},{5,11},{5,12},{6,8},{6,13},{7,9},{7,14},{8,10},{8,12},{8,14},{9,11},{9,13}}

Cousin 817: {{1,4},{1,6},{1,10},{1,11},{2,4},{2,7},{2,12},{2,13},{3,5},{3,6},{3,7},{3,9},{3,10},{4,6},{4,8},{4,14},{5,7},{5,11},{5,12},{6,8},{6,13},{7,8},{7,14},{8,10},{8,12},{9,11},{9,13},{9,14}}

Cousin 818: {{1,4},{1,6},{1,10},{1,11},{2,4},{2,6},{2,12},{2,13},{3,5},{3,6},{3,7},{3,9},{3,10},{4,7},{4,9},{4,14},{5,7},{5,11},{5,12},{6,9},{6,14},{7,8},{7,13},{8,10},{8,12},{8,14},{9,11},{9,13}}

Cousin 819: {{1,4},{1,6},{1,10},{1,11},{2,4},{2,6},{2,7},{2,9},{2,12},{3,5},{3,7},{3,10},{3,13},{4,6},{4,9},{4,14},{5,7},{5,11},{5,12},{6,8},{6,13},{7,9},{7,14},{8,10},{8,12},{8,14},{9,11},{9,13}}

Cousin 820: {{1,4},{1,6},{1,10},{1,11},{2,4},{2,6},{2,7},{2,9},{2,12},{3,5},{3,7},{3,10},{3,13},{4,6},{4,8},{4,14},{5,7},{5,11},{5,12},{6,8},{6,13},{7,8},{7,14},{8,10},{8,12},{9,11},{9,13},{9,14}}

Cousin 821: {{1,4},{1,5},{1,10},{1,11},{2,5},{2,6},{2,12},{2,13},{3,6},{3,7},{3,10},{3,14},{4,6},{4,7},{4,9},{4,12},{5,7},{5,8},{5,14},{6,8},{6,11},{7,8},{7,13},{8,10},{8,12},{9,11},{9,13},{9,14}}

Cousin 822: {{1,4},{1,5},{1,10},{1,11},{2,5},{2,6},{2,7},{2,9},{2,12},{3,6},{3,7},{3,10},{3,13},{4,6},{4,7},{4,9},{4,12},{5,13},{5,14},{6,8},{6,11},{7,9},{7,14},{8,10},{8,12},{8,14},{9,11},{9,13}}

Cousin 823: {{1,4},{1,5},{1,10},{1,11},{2,5},{2,6},{2,12},{2,13},{3,5},{3,6},{3,7},{3,9},{3,10},{4,7},{4,12},{4,14},{5,7},{5,8},{5,9},{6,11},{6,14},{7,9},{7,13},{8,10},{8,13},{8,14},{9,11},{9,12}}

Cousin 824: {{1,3},{1,6},{1,10},{1,11},{2,4},{2,7},{2,12},{2,13},{3,5},{3,7},{3,9},{3,14},{4,6},{4,7},{4,9},{4,10},{5,7},{5,11},{5,12},{6,13},{6,14},{7,8},{7,9},{8,10},{8,12},{8,14},{9,11},{9,13}}

Cousin 825: {{1,3},{1,6},{1,10},{1,11},{2,4},{2,7},{2,12},{2,13},{3,5},{3,6},{3,9},{3,14},{4,6},{4,7},{4,9},{4,10},{5,7},{5,11},{5,12},{6,8},{6,13},{7,9},{7,14},{8,10},{8,12},{8,14},{9,11},{9,13}}

Cousin 826: {{1,3},{1,6},{1,10},{1,11},{2,4},{2,6},{2,7},{2,9},{2,12},{3,5},{3,13},{3,14},{4,6},{4,7},{4,9},{4,10},{5,7},{5,11},{5,12},{6,9},{6,13},{7,8},{7,14},{8,10},{8,12},{8,13},{9,11},{9,14}}

Cousin 827: {{1,8},{1,9},{1,10},{1,11},{2,12},{2,13},{2,14},{3,7},{3,9},{3,10},{3,15},{4,8},{4,9},{4,11},{4,12},{5,7},{5,9},{5,10},{5,13},{6,11},{6,14},{6,15},{7,8},{7,9},{7,12},{8,13},{8,15},{9,14}}

Cousin 828: {{1,8},{1,9},{1,10},{1,11},{2,12},{2,13},{2,14},{3,6},{3,9},{3,10},{3,15},{4,8},{4,9},{4,11},{4,12},{5,7},{5,9},{5,10},{5,13},{6,8},{6,11},{6,14},{7,9},{7,12},{7,15},{8,13},{8,15},{9,14}}

Cousin 829: {{1,8},{1,9},{1,10},{1,11},{2,12},{2,13},{2,14},{3,6},{3,8},{3,10},{3,15},{4,8},{4,9},{4,11},{4,12},{5,7},{5,9},{5,10},{5,13},{6,8},{6,11},{6,14},{7,8},{7,12},{7,15},{8,13},{9,14},{9,15}}

Cousin 830: {{1,8},{1,9},{1,10},{1,11},{2,12},{2,13},{2,14},{3,6},{3,7},{3,8},{3,9},{3,10},{4,8},{4,9},{4,11},{4,12},{5,10},{5,13},{5,15},{6,8},{6,11},{6,14},{7,8},{7,12},{7,15},{8,13},{9,14},{9,15}}

Cousin 831: {{1,8},{1,9},{1,10},{1,11},{2,6},{2,9},{2,12},{2,13},{3,6},{3,7},{3,8},{3,9},{3,10},{4,8},{4,9},{4,11},{4,12},{5,7},{5,9},{5,10},{5,13},{6,8},{6,11},{7,8},{7,9},{7,12},{8,13},{12,13}}

Cousin 832: {{1,8},{1,9},{1,10},{1,11},{2,6},{2,9},{2,12},{2,13},{3,7},{3,9},{3,10},{3,14},{4,8},{4,9},{4,11},{4,12},{5,10},{5,13},{5,15},{6,9},{6,11},{6,14},{7,8},{7,12},{7,15},{8,13},{8,14},{9,15}}

Cousin 833: {{1,8},{1,9},{1,10},{1,11},{2,6},{2,9},{2,12},{2,13},{3,7},{3,8},{3,10},{3,14},{4,8},{4,9},{4,11},{4,12},{5,10},{5,13},{5,15},{6,8},{6,11},{6,14},{7,8},{7,12},{7,15},{8,13},{9,14},{9,15}}

Cousin 834: {{1,8},{1,9},{1,10},{1,11},{2,6},{2,9},{2,12},{2,13},{3,6},{3,9},{3,10},{3,14},{4,8},{4,9},{4,11},{4,12},{5,10},{5,13},{5,15},{6,8},{6,9},{6,11},{7,12},{

{7,14},{7,15},{8,13},{8,14},{9,15}}

Cousin 835: {{1,8},{1,9},{1,10},{1,11},{2,6},{2,9},{2,12},{2,13},{3,6},{3,7},{3,8},{3,9},{3,10},{4,8},{4,9},{4,11},{4,12},{5,7},{5,9},{5,10},{5,13},{6,8},{6,9},{6,11},{7,8},{7,12},{8,13},{10,13}}

Cousin 836: {{1,8},{1,9},{1,10},{1,11},{2,5},{2,9},{2,12},{2,13},{3,7},{3,8},{3,10},{3,14},{4,8},{4,9},{4,11},{4,12},{5,9},{5,10},{5,15},{6,11},{6,13},{6,14},{7,9},{7,12},{7,15},{8,13},{8,15},{9,14}}

Cousin 837: {{1,8},{1,9},{1,10},{1,11},{2,5},{2,9},{2,12},{2,13},{3,6},{3,7},{3,8},{3,10},{4,8},{4,9},{4,11},{4,12},{5,7},{5,8},{5,9},{5,10},{6,9},{6,11},{6,13},{7,8},{7,9},{7,12},{8,13},{11,13}}

Cousin 838: {{1,8},{1,9},{1,10},{1,11},{2,6},{2,7},{2,12},{2,13},{3,10},{3,14},{3,15},{4,7},{4,9},{4,11},{4,12},{5,7},{5,8},{5,10},{5,13},{6,9},{6,11},{6,14},{7,8},{7,15},{8,12},{8,14},{9,13},{9,15}}

Cousin 839: {{1,8},{1,9},{1,10},{1,11},{2,6},{2,7},{2,12},{2,13},{3,7},{3,9},{3,10},{3,14},{4,11},{4,12},{4,15},{5,7},{5,8},{5,10},{5,13},{6,9},{6,11},{6,14},{7,8},{7,15},{8,12},{8,14},{9,13},{9,15}}

Cousin 840: {{1,8},{1,9},{1,10},{1,11},{2,6},{2,7},{2,12},{2,13},{3,7},{3,9},{3,10},{3,14},{4,7},{4,9},{4,11},{4,12},{5,10},{5,13},{5,15},{6,9},{6,11},{6,14},{7,9},{7,15},{8,12},{8,14},{8,15},{9,13}}

Cousin 841: {{1,8},{1,9},{1,10},{1,11},{2,6},{2,7},{2,12},{2,13},{3,10},{3,14},{3,15},{4,7},{4,9},{4,11},{4,12},{5,7},{5,8},{5,10},{5,13},{6,8},{6,11},{6,14},{7,9},{7,15},{8,12},{8,15},{9,13},{9,14}}

Cousin 842: {{1,8},{1,9},{1,10},{1,11},{2,6},{2,7},{2,12},{2,13},{3,7},{3,8},{3,10},{3,14},{4,11},{4,12},{4,15},{5,7},{5,8},{5,10},{5,13},{6,8},{6,11},{6,14},{7,8},{7,15},{8,12},{9,13},{9,14},{9,15}}

Cousin 843: {{1,8},{1,9},{1,10},{1,11},{2,6},{2,7},{2,12},{2,13},{3,7},{3,8},{3,10},{3,14},{4,7},{4,9},{4,11},{4,12},{5,10},{5,13},{5,15},{6,8},{6,11},{6,14},{7,9},{7,15},{8,12},{8,15},{9,13},{9,14}}

Cousin 844: {{1,8},{1,9},{1,10},{1,11},{2,6},{2,7},{2,12},{2,13},{3,6},{3,9},{3,10},{3,14},{4,11},{4,12},{4,15},{5,7},{5,8},{5,10},{5,13},{6,8},{6,9},{6,11},{7,14},{7,15},{8,12},{8,14},{9,13},{9,15}}

Cousin 845: {{1,8},{1,9},{1,10},{1,11},{2,6},{2,7},{2,12},{2,13},{3,6},{3,8},{3,10},{3,14},{4,7},{4,9},{4,11},{4,12},{5,10},{5,13},{5,15},{6,8},{6,9},{6,11},{7,14},{7,15},{8,12},{8,15},{9,13},{9,14}}

Cousin 846: {{1,8},{1,9},{1,10},{1,11},{2,6},{2,7},{2,12},{2,13},{3,6},{3,7},{3,8},{3,9},{3,10},{4,11},{4,12},{4,14},{5,10},{5,13},{5,15},{6,8},{6,9},{6,11},{7,14},{7,15},{8,12},{8,15},{9,13},{9,14}}

Cousin 847: {{1,8},{1,9},{1,10},{1,11},{2,6},{2,7},{2,12},{2,13},{3,6},{3,7},{3,8},{3,9},{3,10},{4,7},{4,9},{4,11},{4,12},{5,7},{5,8},{5,10},{5,13},{6,8},{6,9},{6,11},{7,8},{8,12},{9,13},{11,12}}

Cousin 848: {{1,8},{1,9},{1,10},{1,11},{2,6},{2,7},{2,12},{2,13},{3,6},{3,7},{3,8},{3,9},{3,10},{4,7},{4,9},{4,11},{4,12},{5,7},{5,8},{5,10},{5,13},{6,8},{6,9},{6,11},{7,9},{8,12},{9,13},{10,13}}

Cousin 849: {{1,8},{1,9},{1,10},{1,11},{2,5},{2,7},{2,12},{2,13},{3,10},{3,14},{3,15},{4,7},{4,9},{4,11},{4,12},{5,7},{5,8},{5,9},{5,10},{6,11},{6,13},{6,14},{7,8},{7,15},{8,12},{8,14},{9,13},{9,15}}

Cousin 850: {{1,8},{1,9},{1,10},{1,11},{2,5},{2,7},{2,12},{2,13},{3,7},{3,9},{3,10},{3,14},{4,11},{4,12},{4,15},{5,7},{5,8},{5,9},{5,10},{6,11},{6,13},{6,14},{7,8},{7,15},{8,12},{8,14},{9,13},{9,15}}

Cousin 851: {{1,8},{1,9},{1,10},{1,11},{2,5},{2,7},{2,12},{2,13},{3,7},{3,9},{3,10},{3,14},{4,7},{4,9},{4,11},{4,12},{5,9},{5,10},{5,15},{6,11},{6,13},{6,14},{7,9},{7,15},{8,12},{8,14},{8,15},{9,13}}

Cousin 852: {{1,8},{1,9},{1,10},{1,11},{2,5},{2,7},{2,12},{2,13},{3,7},{3,9},{3,10},{3,14},{4,7},{4,9},{4,11},{4,12},{5,8},{5,10},{5,15},{6,11},{6,13},{6,14},{7,8},{7,15},{8,12},{8,14},{9,13},{9,15}}

Cousin 853: {{1,8},{1,9},{1,10},{1,11},{2,5},{2,7},{2,12},{2,13},{3,6},{3,7},{3,9},{3,10},{4,7},{4,9},{4,11},{4,12},{5,7},{5,8},{5,9},{5,10},{6,8},{6,11},{6,13},{7,8},{7,9},{8,12},{9,13},{11,13}}

Cousin 854: {{1,8},{1,9},{1,10},{1,11},{2,5},{2,7},{2,12},{2,13},{3,6},{3,9},{3,10},{3,14},{4,11},{4,12},{4,15},{5,7},{5,8},{5,9},{5,10},{6,8},{6,11},{6,13},{7,14},{7,15},{8,12},{8,14},{9,13},{9,15}}

Cousin 855: {{1,8},{1,9},{1,10},{1,11},{2,5},{2,7},{2,12},{2,13},{3,6},{3,9},{3,10},{3,14},{4,7},{4,9},{4,11},{4,12},{5,8},{5,10},{5,15},{6,8},{6,11},{6,13},{7,14},{7,15},{8,12},{8,14},{9,13},{9,15}}

Cousin 856: {{1,8},{1,9},{1,10},{1,11},{2,5},{2,7},{2,12},{2,13},{3,6},{3,8},{3,10},{3,14},{4,7},{4,9},{4,11},{4,12},{5,9},{5,10},{5,15},{6,8},{6,11},{6,13},{7,14},{7,15},{8,12},{8,15},{9,13},{9,14}}

Cousin 857: {{1,8},{1,9},{1,10},{1,11},{2,5},{2,7},{2,12},{2,13},{3,6},{3,7},{3,8},{3,9},{3,10},{4,7},{4,9},{4,11},{4,12},{5,7},{5,8},{5,9},{5,10},{6,8},{6,11},{6,13},{7,8},{8,12},{9,13},{11,12}}

Cousin 858: {{1,8},{1,9},{1,10},{1,11},{2,5},{2,6},{2,12},{2,13},{3,7},{3,9},{3,10},{3,14},{4,7},{4,9},{4,11},{4,12},{5,9},{5,10},{5,15},{6,9},{6,11},{6,14},{7,13},{7,15},{8,12},{8,14},{8,15},{9,13}}

Cousin 859: {{1,8},{1,9},{1,10},{1,11},{2,5},{2,6},{2,12},{2,13},{3,10},{3,14},{3,15},{4,7},{4,9},{4,11},{4,12},{5,7},{5,8},{5,9},{5,10},{6,8},{6,11},{6,14},{7,13},{7,15},{8,12},{8,15},{9,13},{9,14}}

Cousin 860: {{1,8},{1,9},{1,10},{1,11},{2,5},{2,6},{2,12},{2,13},{3,7},{3,8},{3,10},{3,14},{4,7},{4,9},{4,11},{4,12},{5,9},{5,10},{5,15},{6,8},{6,11},{6,14},{7,13},{7,15},{8,12},{8,15},{9,13},{9,14}}

Cousin 861: {{1,8},{1,9},{1,10},{1,11},{2,5},{2,6},{2,7},{2,9},{2,12},{3,7},{3,9},{3,10},{3,13},{4,7},{4,9},{4,11},{4,12},{5,7},{5,8},{5,9},{5,10},{6,9},{6,11},{6,13},{7,8},{8,12},{8,13},{10,13}}

Cousin 862: {{1,8},{1,9},{1,10},{1,11},{2,5},{2,6},{2,7},{2,9},{2,12},{3,7},{3,9},{3,10},{3,13},{4,7},{4,9},{4,11},{4,12},{5,7},{5,8},{5,9},{5,10},{6,9},{6,11},{6,13},{7,8},{8,12},{8,13},{11,12}}

Cousin 863: {{1,8},{1,9},{1,10},{1,11},{2,5},{2,6},{2,7},{2,9},{2,12},{3,10},{3,13},{3,14},{4,11},{4,12},{4,15},{5,7},{5,8},{5,9},{5,10},{6,8},{6,11},{6,13},{7,14},{7,15},{8,12},{8,14},{9,13},{9,15}}

Cousin 864: {{1,8},{1,9},{1,10},{1,11},{2,5},{2,6},{2,7},{2,9},{2,12},{3,7},{3,8},{3,10},{3,13},{4,7},{4,9},{4,11},{4,12},{5,7},{5,8},{5,9},{5,10},{6,8},{6,11},{6,13},{7,9},{8,12},{9,13},{10,13}}

Cousin 865: {{1,8},{1,9},{1,10},{1,11},{2,5},{2,6},{2,7},{2,9},{2,12},{3,7},{3,8},{3,10},{3,13},{4,7},{4,9},{4,11},{4,12},{5,7},{5,8},{5,9},{5,10},{6,8},{6,11},{6,13},{7,8},{8,12},{9,13},{11,12}}

Cousin 866: {{1,8},{1,9},{1,10},{1,11},{2,5},{2,6},{2,7},{2,9},{2,12},{3,6},{3,9},{3,10},{3,13},{4,7},{4,9},{4,11},{4,12},{5,7},{5,8},{5,9},{5,10},{6,8},{6,9},{6,11},{7,13},{8,12},{8,13},{11,12}}

Cousin 867: {{1,8},{1,9},{1,10},{1,11},{2,4},{2,7},{2,12},{2,13},{3,10},{3,14},{3,15},{4,7},{4,8},{4,9},{4,11},{5,7},{5,9},{5,10},{5,12},{6,11},{6,13},{6,14},{7,8},{7,15},{8,12},{8,14},{9,13},{9,15}}

Cousin 868: {{1,8},{1,9},{1,10},{1,11},{2,4},{2,7},{2,12},{2,13},{3,7},{3,9},{3,10},{3,14},{4,9},{4,11},{4,15},{5,7},{5,9},{5,10},{5,12},{6,11},{6,13},{6,14},{7,9},{7,15},{8,12},{8,14},{8,15},{9,13}}

Cousin 869: {{1,8},{1,9},{1,10},{1,11},{2,4},{2,7},{2,12},{2,13},{3,7},{3,9},{3,10},{3,14},{4,8},{4,11},{4,15},{5,7},{5,9},{5,10},{5,12},{6,11},{6,13},{6,14},{7,8},{7,15},{8,12},{8,14},{9,13},{9,15}}

Cousin 870: {{1,8},{1,9},{1,10},{1,11},{2,4},{2,7},{2,12},{2,13},{3,6},{3,7},{3,9},{3,10},{4,7},{4,8},{4,9},{4,11},{5,7},{5,9},{5,10},{5,12},{6,8},{6,11},{6,13},{7,8},{7,9},{8,12},{9,13},{11,13}}

Cousin 871: {{1,8},{1,9},{1,10},{1,11},{2,4},{2,7},{2,12},{2,13},{3,6},{3,9},{3,10},{3,14},{4,8},{4,11},{4,15},{5,7},{5,9},{5,10},{5,12},{6,8},{6,11},{6,13},{7,14},{7,15},{8,12},{8,14},{9,13},{9,15}}

Cousin 872: {{1,8},{1,9},{1,10},{1,11},{2,4},{2,7},{2,12},{2,13},{3,6},{3,8},{3,10},{3,14},{4,9},{4,11},{4,15},{5,7},{5,9},{5,10},{5,12},{6,8},{6,11},{6,13},{7,14},{7,15},{8,12},{8,15},{9,13},{9,14}}

Cousin 873: {{1,8},{1,9},{1,10},{1,11},{2,4},{2,6},{2,12},{2,13},{3,7},{3,9},{3,10},{3,14},{4,9},{4,11},{4,15},{5,7},{5,9},{5,10},{5,12},{6,9},{6,11},{6,14},{7,13},{7,15},{8,12},{8,14},{8,15},{9,13}}

Cousin 874: {{1,8},{1,9},{1,10},{1,11},{2,4},{2,6},{2,12},{2,13},{3,10},{3,14},{3,15},{4,7},{4,8},{4,9},{4,11},{5,7},{5,9},{5,10},{5,12},{6,8},{6,11},{6,14},{7,13},{7,15},{8,12},{8,15},{9,13},{9,14}}

Cousin 875: {{1,8},{1,9},{1,10},{1,11},{2,4},{2,6},{2,12},{2,13},{3,7},{3,8},{3,10},{3,14},{4,9},{4,11},{4,15},{5,7},{5,9},{5,10},{5,12},{6,8},{6,11},{6,14},{7,13},{7,15},{8,12},{8,15},{9,13},{9,14}}

Cousin 876: {{1,8},{1,9},{1,10},{1,11},{2,4},{2,6},{2,7},{2,9},{2,12},{3,7},{3,9},{3,10},{3,13},{4,7},{4,8},{4,9},{4,11},{5,7},{5,9},{5,10},{5,12},{6,9},{6,11},{6,13},{7,8},{8,12},{8,13},{10,13}}

Cousin 877: {{1,8},{1,9},{1,10},{1,11},{2,4},{2,6},{2,7},{2,9},{2,12},{3,7},{3,8},{3,10},{3,13},{4,7},{4,8},{4,9},{4,11},{5,7},{5,9},{5,10},{5,12},{6,8},{6,11},{6,13},{7,9},{8,12},{9,13},{10,13}}

Cousin 878: {{1,8},{1,9},{1,10},{1,11},{2,4},{2,5},{2,12},{2,13},{3,10},{3,14},{3,15},{4,7},{4,8},{4,9},{4,11},{5,7},{5,8},{5,9},{5,10},{6,11},{6,12},{6,14},{7,13},{7,15},{8,12},{8,15},{9,13},{9,14}}

Cousin 879: {{1,8},{1,9},{1,10},{1,11},{2,4},{2,5},{2,12},{2,13},{3,6},{3,7},{3,8},{3,10},{4,7},{4,8},{4,9},{4,11},{5,7},{5,8},{5,9},{5,10},{6,9},{6,11},{6,12},{7,8},{7,13},{8,12},{9,13},{11,12}}

Cousin 880: {{1,8},{1,9},{1,10},{1,11},{2,4},{2,5},{2,7},{2,9},{2,12},{3,7},{3,8},{3,10},{3,13},{4,7},{4,8},{4,9},{4,11},{5,7},{5,8},{5,9},{5,10},{6,11},{6,12},{6,13},{7,9},{8,12},{9,13},{10,13}}

Cousin 881: {{1,10},{1,11},{1,12},{2,13},{2,14},{2,15},{3,6},{3,7},{3,8},{3,9},{3,10},{4,7},{4,9},{4,11},{4,13},{5,7},{5,9},{5,10},{5,14},{6,8},{6,12},{6,13},{7,8},{7,15},{8,11},{8,14},{9,12},{9,15}}

Cousin 882: {{1,10},{1,11},{1,12},{2,7},{2,9},{2,13},{2,14},{3,7},{3,9},{3,10},{3,15},{4,7},{4,9},{4,11},{4,13},{5,7},{5,9},{5,10},{5,14},{6,12},{6,13},{6,15},{7,8},{7,9},{8,11},{8,14},{8,15},{9,12}}

Cousin 883: {{1,10},{1,11},{1,12},{2,7},{2,9},{2,13},{2,14},{3,6},{3,9},{3,10},{3,15},{4,7},{4,9},{4,11},{4,13},{5,7},{5,9},{5,10},{5,14},{6,8},{6,12},{6,13},{7,9},{7,15},{8,11},{8,14},{8,15},{9,12}}

Cousin 884: {{1,10},{1,11},{1,12},{2,7},{2,9},{2,13},{2,14},{3,6},{3,8},{3,10},{3,15},{4,7},{4,9},{4,11},{4,13},{5,7},{5,9},{5,10},{5,14},{6,8},{6,12},{6,13},{7,8},{7,15},{8,11},{8,14},{9,12},{9,15}}



Cousin 885: {{1,10},{1,11},{1,12},{2,7},{2,9},{2,13},{2,14},{3,6},{3,7},{3,8},{3,9},{3,10},{4,11},{4,13},{4,15},{5,7},{5,9},{5,10},{5,14},{6,8},{6,12},{6,13},{7,8},{7,15},{8,11},{8,14},{9,12},{9,15}}

Cousin 886: {{1,10},{1,11},{1,12},{2,7},{2,9},{2,13},{2,14},{3,6},{3,7},{3,8},{3,9},{3,10},{4,7},{4,9},{4,11},{4,13},{5,10},{5,14},{5,15},{6,8},{6,12},{6,13},{7,8},{7,15},{8,11},{8,14},{9,12},{9,15}}

Cousin 887: {{1,2},{1,5},{1,8},{2,7},{2,9},{2,13},{3,6},{3,7},{3,8},{3,9},{3,10},{4,7},{4,9},{4,11},{4,13},{5,7},{5,9},{5,10},{6,8},{6,12},{6,13},{7,8},{7,9},{8,11},{9,12},{10,11},{10,12},{11,12}}

Cousin 888: {{1,10},{1,11},{1,12},{2,13},{2,14},{2,15},{3,6},{3,7},{3,8},{3,9},{3,10},{4,7},{4,9},{4,11},{4,13},{5,7},{5,8},{5,10},{5,14},{6,8},{6,12},{6,13},{7,9},{7,15},{8,11},{8,15},{9,12},{9,14}}

Cousin 889: {{1,10},{1,11},{1,12},{2,7},{2,8},{2,13},{2,14},{3,7},{3,9},{3,10},{3,15},{4,7},{4,9},{4,11},{4,13},{5,7},{5,8},{5,10},{5,14},{6,12},{6,13},{6,15},{7,8},{7,9},{8,11},{8,15},{9,12},{9,14}}

Cousin 890: {{1,10},{1,11},{1,12},{2,7},{2,8},{2,13},{2,14},{3,6},{3,9},{3,10},{3,15},{4,7},{4,9},{4,11},{4,13},{5,7},{5,8},{5,10},{5,14},{6,8},{6,12},{6,13},{7,9},{7,15},{8,11},{8,15},{9,12},{9,14}}

Cousin 891: {{1,10},{1,11},{1,12},{2,7},{2,8},{2,13},{2,14},{3,6},{3,8},{3,10},{3,15},{4,7},{4,9},{4,11},{4,13},{5,7},{5,8},{5,10},{5,14},{6,8},{6,12},{6,13},{7,8},{7,15},{8,11},{9,12},{9,14},{9,15}}

Cousin 892: {{1,10},{1,11},{1,12},{2,7},{2,8},{2,13},{2,14},{3,6},{3,7},{3,8},{3,9},{3,10},{4,11},{4,13},{4,15},{5,7},{5,8},{5,10},{5,14},{6,8},{6,12},{6,13},{7,8},{7,15},{8,11},{9,12},{9,14},{9,15}}

Cousin 893: {{1,10},{1,11},{1,12},{2,7},{2,8},{2,13},{2,14},{3,6},{3,7},{3,8},{3,9},{3,10},{4,7},{4,9},{4,11},{4,13},{5,10},{5,14},{5,15},{6,8},{6,12},{6,13},{7,9},{7,15},{8,11},{8,15},{9,12},{9,14}}

Cousin 894: {{1,2},{1,5},{1,9},{2,7},{2,8},{2,13},{3,6},{3,7},{3,8},{3,9},{3,10},{4,7},{4,9},{4,11},{4,13},{5,7},{5,8},{5,10},{6,8},{6,12},{6,13},{7,8},{7,9},{8,11},{9,12},{10,11},{10,12},{11,12}}

Cousin 895: {{1,10},{1,11},{1,12},{2,5},{2,9},{2,13},{2,14},{3,7},{3,9},{3,10},{3,15},{4,7},{4,9},{4,11},{4,13},{5,7},{5,8},{5,9},{5,10},{6,12},{6,13},{6,15},{7,9},{7,14},{8,11},{8,14},{8,15},{9,12}}

Cousin 896: {{1,10},{1,11},{1,12},{2,5},{2,9},{2,13},{2,14},{3,6},{3,8},{3,10},{3,15},{4,7},{4,9},{4,11},{4,13},{5,7},{5,8},{5,9},{5,10},{6,8},{6,12},{6,13},{7,14},{7,15},{8,11},{8,14},{9,12},{9,15}}

Cousin 897: {{1,10},{1,11},{1,12},{2,5},{2,9},{2,13},{2,14},{3,6},{3,7},{3,8},{3,9},{3,10},{4,11},{4,13},{4,15},{5,7},{5,8},{5,9},{5,10},{6,8},{6,12},{6,13},{7,14},{7,15},{8,11},{8,14},{9,12},{9,15}}

Cousin 898: {{1,10},{1,11},{1,12},{2,5},{2,9},{2,13},{2,14},{3,6},{3,7},{3,8},{3,9},{3,10},{4,7},{4,9},{4,11},{4,13},{5,8},{5,10},{5,15},{6,8},{6,12},{6,13},{7,14},{7,15},{8,11},{8,14},{9,12},{9,15}}

Cousin 899: {{1,2},{1,7},{1,8},{2,5},{2,9},{2,13},{3,6},{3,7},{3,8},{3,9},{3,10},{4,7},{4,9},{4,11},{4,13},{5,7},{5,8},{5,9},{5,10},{6,8},{6,12},{6,13},{7,9},{8,11},{9,12},{10,11},{10,12},{11,12}}

Cousin 900: {{1,10},{1,11},{1,12},{2,5},{2,8},{2,13},{2,14},{3,7},{3,9},{3,10},{3,15},{4,7},{4,9},{4,11},{4,13},{5,7},{5,8},{5,9},{5,10},{6,12},{6,13},{6,15},{7,8},{7,14},{8,11},{8,15},{9,12},{9,14}}

Cousin 901: {{1,10},{1,11},{1,12},{2,5},{2,8},{2,13},{2,14},{3,6},{3,9},{3,10},{3,15},{4,7},{4,9},{4,11},{4,13},{5,7},{5,8},{5,9},{5,10},{6,8},{6,12},{6,13},{7,14},{7,15},{8,11},{8,15},{9,12},{9,14}}

Cousin 902: {{1,10},{1,11},{1,12},{2,5},{2,8},{2,13},{2,14},{3,6},{3,7},{3,8},{3,9},{3,10},{4,7},{4,9},{4,11},{4,13},{5,9},{5,10},{5,15},{6,8},{6,12},{6,13},{7,14},{7,15},{8,11},{8,15},{9,12},{9,14}}

Cousin 903: {{1,2},{1,7},{1,9},{2,5},{2,8},{2,13},{3,6},{3,7},{3,8},{3,9},{3,10},{4,7},{4,9},{4,11},{4,13},{5,7},{5,8},{5,9},{5,10},{6,8},{6,12},{6,13},{7,8},{8,11},{9,12},{10,11},{10,12},{11,12}}

Cousin 904: {{1,10},{1,11},{1,12},{2,5},{2,7},{2,8},{2,9},{2,13},{3,10},{3,14},{3,15},{4,7},{4,9},{4,11},{4,13},{5,7},{5,8},{5,9},{5,10},{6,12},{6,13},{6,14},{7,8},{7,15},{8,11},{8,14},{9,12},{9,15}}

Cousin 905: {{1,3},{1,6},{1,8},{2,5},{2,7},{2,8},{2,9},{2,13},{3,7},{3,9},{3,10},{4,7},{4,9},{4,11},{4,13},{5,7},{5,8},{5,9},{5,10},{6,12},{6,13},{7,8},{7,9},{8,11},{9,12},{10,11},{10,12},{11,12}}

Cousin 906: {{1,10},{1,11},{1,12},{2,5},{2,7},{2,8},{2,9},{2,13},{3,6},{3,9},{3,10},{3,14},{4,11},{4,13},{4,15},{5,7},{5,8},{5,9},{5,10},{6,8},{6,12},{6,13},{7,14},{7,15},{8,11},{8,14},{9,12},{9,15}}

Cousin 907: {{1,10},{1,11},{1,12},{2,5},{2,7},{2,8},{2,9},{2,13},{3,6},{3,9},{3,10},{3,14},{4,7},{4,9},{4,11},{4,13},{5,8},{5,10},{5,15},{6,8},{6,12},{6,13},{7,14},{7,15},{8,11},{8,14},{9,12},{9,15}}

Cousin 908: {{1,3},{1,7},{1,8},{2,5},{2,7},{2,8},{2,9},{2,13},{3,6},{3,9},{3,10},{4,7},{4,9},{4,11},{4,13},{5,7},{5,8},{5,9},{5,10},{6,8},{6,12},{6,13},{7,9},{8,11},{9,12},{10,11},{10,12},{11,12}}

Cousin 909: {{1,10},{1,11},{1,12},{2,5},{2,7},{2,8},{2,9},{2,13},{3,6},{3,8},{3,10},{3,14},{4,7},{4,9},{4,11},{4,13},{5,9},{5,10},{5,15},{6,8},{6,12},{6,13},{7,14},{7,15},{8,11},{8,15},{9,12},{9,14}}

Cousin 910: {{1,3},{1,7},{1,9},{2,5},{2,7},{2,8},{2,9},{2,13},{3,6},{3,8},{3,10},{4,7},{4,9},{4,11},{4,13},{5,7},{5,8},{5,9},{5,10},{6,8},{6,12},{6,13},{7,8},{8,11},{9,12},{10,11},{10,12},{11,12}}

{9,12},{10,11},{10,12},{11,12}}

Cousin 911: {{1,10},{1,11},{1,12},{2,5},{2,7},{2,8},{2,9},{2,13},{3,6},{3,7},{3,8},{3,9},{3,10},{4,11},{4,13},{4,14},{5,9},{5,10},{5,15},{6,8},{6,12},{6,13},{7,14},{7,15},{8,11},{8,15},{9,12},{9,14}}

Cousin 912: {{1,4},{1,7},{1,9},{2,5},{2,7},{2,8},{2,9},{2,13},{3,6},{3,7},{3,8},{3,9},{3,10},{4,11},{4,13},{5,7},{5,8},{5,9},{5,10},{6,8},{6,12},{6,13},{7,8},{8,11},{9,12},{10,11},{10,12},{11,12}}

Cousin 913: {{1,10},{1,11},{1,12},{2,5},{2,7},{2,8},{2,9},{2,13},{3,6},{3,7},{3,8},{3,9},{3,10},{4,7},{4,9},{4,11},{4,13},{5,7},{5,8},{5,9},{5,10},{6,8},{6,12},{6,13},{7,8},{8,11},{9,12},{11,13}}

Cousin 914: {{1,5},{1,7},{1,8},{2,5},{2,7},{2,8},{2,9},{2,13},{3,6},{3,7},{3,8},{3,9},{3,10},{4,7},{4,9},{4,11},{4,13},{5,9},{5,10},{6,8},{6,12},{6,13},{7,9},{8,11},{9,12},{10,11},{10,12},{11,12}}

Cousin 915: {{1,5},{1,7},{1,9},{2,5},{2,7},{2,8},{2,9},{2,13},{3,6},{3,7},{3,8},{3,9},{3,10},{4,7},{4,9},{4,11},{4,13},{5,8},{5,10},{6,8},{6,12},{6,13},{7,8},{8,11},{9,12},{10,11},{10,12},{11,12}}

Cousin 916: {{1,10},{1,11},{1,12},{2,6},{2,9},{2,13},{2,14},{3,7},{3,9},{3,10},{3,15},{4,6},{4,9},{4,11},{4,13},{5,7},{5,9},{5,10},{5,14},{6,12},{6,15},{7,8},{7,9},{7,13},{8,11},{8,14},{8,15},{9,12}}

Cousin 917: {{1,10},{1,11},{1,12},{2,6},{2,9},{2,13},{2,14},{3,6},{3,9},{3,10},{3,15},{4,6},{4,9},{4,11},{4,13},{5,7},{5,9},{5,10},{5,14},{6,8},{6,12},{7,9},{7,13},{7,15},{8,11},{8,14},{8,15},{9,12}}

Cousin 918: {{1,10},{1,11},{1,12},{2,6},{2,9},{2,13},{2,14},{3,6},{3,8},{3,10},{3,15},{4,6},{4,9},{4,11},{4,13},{5,7},{5,9},{5,10},{5,14},{6,8},{6,12},{7,8},{7,13},{7,15},{8,11},{8,14},{9,12},{9,15}}

Cousin 919: {{1,2},{1,5},{1,8},{2,6},{2,9},{2,13},{3,6},{3,7},{3,8},{3,9},{3,10},{4,6},{4,9},{4,11},{4,13},{5,7},{5,9},{5,10},{6,8},{6,12},{7,8},{7,9},{7,13},{8,11},{9,12},{10,11},{10,12},{11,12}}

Cousin 920: {{1,10},{1,11},{1,12},{2,13},{2,14},{2,15},{3,6},{3,7},{3,8},{3,9},{3,10},{4,6},{4,9},{4,11},{4,13},{5,7},{5,8},{5,10},{5,14},{6,12},{6,15},{7,8},{7,9},{7,13},{8,11},{8,15},{9,12},{9,14}}

Cousin 921: {{1,10},{1,11},{1,12},{2,6},{2,8},{2,13},{2,14},{3,7},{3,9},{3,10},{3,15},{4,6},{4,9},{4,11},{4,13},{5,7},{5,8},{5,10},{5,14},{6,12},{6,15},{7,8},{7,9},{7,13},{8,11},{8,15},{9,12},{9,14}}

Cousin 922: {{1,10},{1,11},{1,12},{2,6},{2,8},{2,13},{2,14},{3,6},{3,9},{3,10},{3,15},{4,6},{4,9},{4,11},{4,13},{5,7},{5,8},{5,10},{5,14},{6,8},{6,12},{7,9},{7,13},{7,15},{8,11},{8,15},{9,12},{9,14}}

Cousin 923: {{1,10},{1,11},{1,12},{2,6},{2,8},{2,13},{2,14},{3,6},{3,8},{3,10},{3,15},{4,6},{4,9},{4,11},{4,13},{5,7},{5,8},{5,10},{5,14},{6,8},{6,12},{7,8},{7,13},{7,15},{8,11},{9,12},{9,14},{9,15}}

Cousin 924: {{1,2},{1,5},{1,9},{2,6},{2,8},{2,13},{3,6},{3,7},{3,8},{3,9},{3,10},{4,6},{4,9},{4,11},{4,13},{5,7},{5,8},{5,10},{6,8},{6,12},{7,8},{7,9},{7,13},{8,11},{9,12},{10,11},{10,12},{11,12}}

Cousin 925: {{1,10},{1,11},{1,12},{2,5},{2,9},{2,13},{2,14},{3,6},{3,9},{3,10},{3,15},{4,6},{4,9},{4,11},{4,13},{5,7},{5,8},{5,9},{5,10},{6,12},{6,14},{7,9},{7,13},{7,15},{8,11},{8,14},{8,15},{9,12}}

Cousin 926: {{1,10},{1,11},{1,12},{2,5},{2,9},{2,13},{2,14},{3,6},{3,8},{3,10},{3,15},{4,6},{4,9},{4,11},{4,13},{5,7},{5,8},{5,9},{5,10},{6,12},{6,14},{7,8},{7,13},{7,15},{8,11},{8,14},{9,12},{9,15}}

Cousin 927: {{1,10},{1,11},{1,12},{2,5},{2,9},{2,13},{2,14},{3,6},{3,7},{3,8},{3,9},{3,10},{4,6},{4,9},{4,11},{4,13},{5,9},{5,10},{5,15},{6,12},{6,14},{7,9},{7,13},{7,15},{8,11},{8,14},{8,15},{9,12}}

Cousin 928: {{1,10},{1,11},{1,12},{2,5},{2,9},{2,13},{2,14},{3,6},{3,7},{3,8},{3,9},{3,10},{4,6},{4,9},{4,11},{4,13},{5,8},{5,10},{5,15},{6,12},{6,14},{7,8},{7,13},{7,15},{8,11},{8,14},{9,12},{9,15}}

Cousin 929: {{1,2},{1,6},{1,8},{2,5},{2,9},{2,13},{3,6},{3,7},{3,8},{3,9},{3,10},{4,6},{4,9},{4,11},{4,13},{5,7},{5,8},{5,9},{5,10},{6,12},{7,8},{7,9},{7,13},{8,11},{9,12},{10,11},{10,12},{11,12}}

Cousin 930: {{1,10},{1,11},{1,12},{2,5},{2,6},{2,8},{2,9},{2,13},{3,10},{3,14},{3,15},{4,6},{4,9},{4,11},{4,13},{5,7},{5,8},{5,9},{5,10},{6,12},{6,14},{7,8},{7,13},{7,15},{8,11},{8,14},{9,12},{9,15}}

Cousin 931: {{1,10},{1,11},{1,12},{2,5},{2,6},{2,8},{2,9},{2,13},{3,7},{3,9},{3,10},{3,14},{4,6},{4,9},{4,11},{4,13},{5,9},{5,10},{5,15},{6,12},{6,14},{7,9},{7,13},{7,15},{8,11},{8,14},{8,15},{9,12}}

Cousin 932: {{1,10},{1,11},{1,12},{2,5},{2,6},{2,8},{2,9},{2,13},{3,7},{3,9},{3,10},{3,14},{4,6},{4,9},{4,11},{4,13},{5,8},{5,10},{5,15},{6,12},{6,14},{7,8},{7,13},{7,15},{8,11},{8,14},{9,12},{9,15}}

Cousin 933: {{1,3},{1,6},{1,8},{2,5},{2,6},{2,8},{2,9},{2,13},{3,7},{3,9},{3,10},{4,6},{4,9},{4,11},{4,13},{5,7},{5,8},{5,9},{5,10},{6,12},{7,8},{7,9},{7,13},{8,11},{9,12},{10,11},{10,12},{11,12}}

Cousin 934: {{1,3},{1,7},{1,8},{2,5},{2,6},{2,8},{2,9},{2,13},{3,6},{3,9},{3,10},{4,6},{4,9},{4,11},{4,13},{5,7},{5,8},{5,9},{5,10},{6,8},{6,12},{7,9},{7,13},{8,11},{9,12},{10,11},{10,12},{11,12}}

Cousin 935: {{1,3},{1,7},{1,9},{2,5},{2,6},{2,8},{2,9},{2,13},{3,6},{3,8},{3,10},{4,6},{4,9},{4,11},{4,13},{5,7},{5,8},{5,9},{5,10},{6,8},{6,12},{7,8},{7,13},{8,11},{9,12},{10,11},{10,12},{11,12}}

Cousin 936: {{1,5},{1,7},{1,8},{2,5},{2,6},{2,8},{2,9},{2,13},{3,6},{3,7},{3,8},{3,9},{3,10},{4,6},{4,9},{4,11},{4,13},{5,9},{5,10},{6,8},{6,12},{7,9},{7,13},{8,11},{9,12},{10,11},{10,12},{11,12}}

Cousin 937: {{1,5},{1,7},{1,9},{2,5},{2,6},{2,8},{2,9},{2,13},{3,6},{3,7},{3,8},{3,9},{3,10},{4,6},{4,9},{4,11},{4,13},{5,8},{5,10},{6,8},{6,12},{7,8},{7,13},{8,11},{9,12},{10,11},{10,12},{11,12}}

Cousin 938: {{1,10},{1,11},{1,12},{2,6},{2,7},{2,13},{2,14},{3,7},{3,9},{3,10},{3,15},{4,6},{4,7},{4,11},{4,13},{5,7},{5,9},{5,10},{5,14},{6,12},{6,15},{7,8},{7,9},{8,11},{8,14},{8,15},{9,12},{9,13}}

Cousin 939: {{1,10},{1,11},{1,12},{2,6},{2,7},{2,13},{2,14},{3,6},{3,9},{3,10},{3,15},{4,6},{4,7},{4,11},{4,13},{5,7},{5,9},{5,10},{5,14},{6,8},{6,12},{7,9},{7,15},{8,11},{8,14},{8,15},{9,12},{9,13}}

Cousin 940: {{1,10},{1,11},{1,12},{2,6},{2,7},{2,13},{2,14},{3,6},{3,8},{3,10},{3,15},{4,6},{4,7},{4,11},{4,13},{5,7},{5,9},{5,10},{5,14},{6,8},{6,12},{7,8},{7,15},{8,11},{8,14},{9,12},{9,13},{9,15}}

Cousin 941: {{1,10},{1,11},{1,12},{2,6},{2,7},{2,13},{2,14},{3,6},{3,7},{3,8},{3,9},{3,10},{4,6},{4,7},{4,11},{4,13},{5,10},{5,14},{5,15},{6,8},{6,12},{7,8},{7,15},{8,11},{8,14},{9,12},{9,13},{9,15}}

Cousin 942: {{1,2},{1,5},{1,8},{2,6},{2,7},{2,13},{3,6},{3,7},{3,8},{3,9},{3,10},{4,6},{4,7},{4,11},{4,13},{5,7},{5,9},{5,10},{6,8},{6,12},{7,8},{7,9},{8,11},{9,12},{9,13},{10,11},{10,12},{11,12}}

Cousin 943: {{1,10},{1,11},{1,12},{2,5},{2,7},{2,13},{2,14},{3,6},{3,9},{3,10},{3,15},{4,6},{4,7},{4,11},{4,13},{5,7},{5,8},{5,9},{5,10},{6,12},{6,14},{7,9},{7,15},{8,11},{8,14},{8,15},{9,12},{9,13}}

Cousin 944: {{1,10},{1,11},{1,12},{2,5},{2,7},{2,13},{2,14},{3,6},{3,8},{3,10},{3,15},{4,6},{4,7},{4,11},{4,13},{5,7},{5,8},{5,9},{5,10},{6,12},{6,14},{7,8},{7,15},{8,11},{8,14},{9,12},{9,13},{9,15}}

Cousin 945: {{1,10},{1,11},{1,12},{2,5},{2,7},{2,13},{2,14},{3,6},{3,7},{3,8},{3,9},{3,10},{4,6},{4,7},{4,11},{4,13},{5,9},{5,10},{5,15},{6,12},{6,14},{7,9},{7,15},{8,11},{8,14},{8,15},{9,12},{9,13}}

Cousin 946: {{1,10},{1,11},{1,12},{2,5},{2,7},{2,13},{2,14},{3,6},{3,7},{3,8},{3,9},{3,10},{4,6},{4,7},{4,11},{4,13},{5,8},{5,10},{5,15},{6,12},{6,14},{7,8},{7,15},{8,11},{8,14},{9,12},{9,13},{9,15}}

Cousin 947: {{1,2},{1,6},{1,8},{2,5},{2,7},{2,13},{3,6},{3,7},{3,8},{3,9},{3,10},{4,6},{4,7},{4,11},{4,13},{5,7},{5,8},{5,9},{5,10},{6,12},{7,8},{7,9},{8,11},{9,12},{9,13},{10,11},{10,12},{11,12}}

Cousin 948: {{1,10},{1,11},{1,12},{2,5},{2,6},{2,13},{2,14},{3,7},{3,9},{3,10},{3,15},{4,6},{4,7},{4,11},{4,13},{5,7},{5,8},{5,9},{5,10},{6,12},{6,15},{7,9},{7,14},{8,11},{8,14},{8,15},{9,12},{9,13}}

Cousin 949: {{1,10},{1,11},{1,12},{2,5},{2,6},{2,13},{2,14},{3,6},{3,8},{3,10},{3,15},{4,6},{4,7},{4,11},{4,13},{5,7},{5,8},{5,9},{5,10},{6,8},{6,12},{7,14},{7,15},{8,11},{8,14},{9,12},{9,13},{9,15}}

Cousin 950: {{1,10},{1,11},{1,12},{2,5},{2,6},{2,13},{2,14},{3,6},{3,7},{3,8},{3,9},{3,10},{4,6},{4,7},{4,11},{4,13},{5,8},{5,10},{5,15},{6,8},{6,12},{7,14},{7,15},{8,11},{8,14},{9,12},{9,13},{9,15}}

Cousin 951: {{1,2},{1,7},{1,8},{2,5},{2,6},{2,13},{3,6},{3,7},{3,8},{3,9},{3,10},{4,6},{4,7},{4,11},{4,13},{5,7},{5,8},{5,9},{5,10},{6,8},{6,12},{7,9},{8,11},{9,12},{9,13},{10,11},{10,12},{11,12}}

Cousin 952: {{1,10},{1,11},{1,12},{2,5},{2,6},{2,7},{2,8},{2,13},{3,10},{3,14},{3,15},{4,6},{4,7},{4,11},{4,13},{5,7},{5,8},{5,9},{5,10},{6,12},{6,14},{7,8},{7,15},{8,11},{8,14},{9,12},{9,13},{9,15}}

Cousin 953: {{1,10},{1,11},{1,12},{2,5},{2,6},{2,7},{2,8},{2,13},{3,7},{3,9},{3,10},{3,14},{4,6},{4,7},{4,11},{4,13},{5,9},{5,10},{5,15},{6,12},{6,14},{7,9},{7,15},{8,11},{8,14},{8,15},{9,12},{9,13}}

Cousin 954: {{1,10},{1,11},{1,12},{2,5},{2,6},{2,7},{2,8},{2,13},{3,7},{3,9},{3,10},{3,14},{4,6},{4,7},{4,11},{4,13},{5,8},{5,10},{5,15},{6,12},{6,14},{7,8},{7,15},{8,11},{8,14},{9,12},{9,13},{9,15}}

Cousin 955: {{1,3},{1,6},{1,8},{2,5},{2,6},{2,7},{2,8},{2,13},{3,7},{3,9},{3,10},{4,6},{4,7},{4,11},{4,13},{5,7},{5,8},{5,9},{5,10},{6,12},{7,8},{7,9},{8,11},{9,12},{9,13},{10,11},{10,12},{11,12}}

Cousin 956: {{1,10},{1,11},{1,12},{2,5},{2,6},{2,7},{2,8},{2,13},{3,6},{3,9},{3,10},{3,14},{4,6},{4,7},{4,11},{4,13},{5,8},{5,10},{5,15},{6,8},{6,12},{7,14},{7,15},{8,11},{8,14},{9,12},{9,13},{9,15}}

Cousin 957: {{1,3},{1,7},{1,8},{2,5},{2,6},{2,7},{2,8},{2,13},{3,6},{3,9},{3,10},{4,6},{4,7},{4,11},{4,13},{5,7},{5,8},{5,9},{5,10},{6,8},{6,12},{7,9},{8,11},{9,12},{9,13},{10,11},{10,12},{11,12}}

Cousin 958: {{1,10},{1,11},{1,12},{2,5},{2,6},{2,7},{2,8},{2,13},{3,6},{3,8},{3,10},{3,14},{4,6},{4,7},{4,11},{4,13},{5,9},{5,10},{5,15},{6,8},{6,12},{7,14},{7,15},{8,11},{8,15},{9,12},{9,13},{9,14}}

Cousin 959: {{1,3},{1,7},{1,9},{2,5},{2,6},{2,7},{2,8},{2,13},{3,6},{3,8},{3,10},{4,6},{4,7},{4,11},{4,13},{5,7},{5,8},{5,9},{5,10},{6,8},{6,12},{7,8},{8,11},{9,12},{9,13},{10,11},{10,12},{11,12}}

Cousin 960: {{1,5},{1,7},{1,8},{2,5},{2,6},{2,7},{2,8},{2,13},{3,6},{3,7},{3,8},{3,9},{3,10},{4,6},{4,7},{4,11},{4,13},{5,9},{5,10},{6,8},{6,12},{7,9},{8,11},{9,12},{9,13},{10,11},{10,12},{11,12}}

Cousin 961: {{1,5},{1,7},{1,9},{2,5},{2,6},{2,7},{2,8},{2,13},{3,6},{3,7},{3,8},{3,9},{3,10},{4,6},{4,7},{4,11},{4,13},{5,8},{5,10},{6,8},{6,12},{7,8},{8,11},{9,12},{9,13},{10,11},{10,12},{11,12}}

Cousin 962: {{1,10},{1,11},{1,12},{2,4},{2,6},{2,13},{2,14},{3,7},{3,9},{3,10},{3,15},{4,6},{4,7},{4,9},{4,11},{5,7},{5,9},{5,10},{5,13},{6,12},{6,15},{7,8},{7,14},{8,11},{8,13},{8,15},{9,12},{9,14}}

Cousin 963: {{1,10},{1,11},{1,12},{2,4},{2,6},{2,13},{2,14},{3,6},{3,9},{3,10},{3,15},{4,6},{4,7},{4,9},{4,11},{5,7},{5,9},{5,10},{5,13},{6,8},{6,12},{7,14},{7,15},{8,11},{8,13},{8,15},{9,12},{9,14}}

Cousin 964: {{1,2},{1,7},{1,9},{2,4},{2,6},{2,13},{3,6},{3,7},{3,8},{3,9},{3,10},{4,6},{4,7},{4,9},{4,11},{5,7},{5,9},{5,10},{5,13},{6,8},{6,12},{7,8},{8,11},{8,13},{9,12},{10,11},{10,12},{11,12}}

Cousin 965: {{1,10},{1,11},{1,12},{2,4},{2,6},{2,7},{2,9},{2,13},{3,10},{3,14},{3,15},{4,6},{4,7},{4,9},{4,11},{5,7},{5,9},{5,10},{5,13},{6,12},{6,14},{7,8},{7,15},{8,11},{8,13},{8,14},{9,12},{9,15}}

Cousin 966: {{1,10},{1,11},{1,12},{2,4},{2,6},{2,7},{2,9},{2,13},{3,7},{3,9},{3,10},{3,14},{4,6},{4,11},{4,15},{5,7},{5,9},{5,10},{5,13},{6,12},{6,14},{7,8},{7,15},{8,11},{8,13},{8,14},{9,12},{9,15}}

Cousin 967: {{1,10},{1,11},{1,12},{2,4},{2,6},{2,7},{2,9},{2,13},{3,7},{3,9},{3,10},{3,14},{4,6},{4,7},{4,9},{4,11},{5,10},{5,13},{5,15},{6,12},{6,14},{7,8},{7,15},{8,11},{8,13},{8,14},{9,12},{9,15}}

Cousin 968: {{1,3},{1,6},{1,8},{2,4},{2,6},{2,7},{2,9},{2,13},{3,7},{3,9},{3,10},{4,6},{4,7},{4,9},{4,11},{5,7},{5,9},{5,10},{5,13},{6,12},{7,8},{7,9},{8,11},{8,13},{9,12},{10,11},{10,12},{11,12}}

Cousin 969: {{1,10},{1,11},{1,12},{2,4},{2,6},{2,7},{2,9},{2,13},{3,6},{3,9},{3,10},{3,14},{4,6},{4,11},{4,15},{5,7},{5,9},{5,10},{5,13},{6,8},{6,12},{7,14},{7,15},{8,11},{8,13},{8,14},{9,12},{9,15}}

Cousin 970: {{1,3},{1,7},{1,8},{2,4},{2,6},{2,7},{2,9},{2,13},{3,6},{3,9},{3,10},{4,6},{4,7},{4,9},{4,11},{5,7},{5,9},{5,10},{5,13},{6,8},{6,12},{7,9},{8,11},{8,13},{9,12},{10,11},{10,12},{11,12}}

Cousin 971: {{1,3},{1,7},{1,9},{2,4},{2,6},{2,7},{2,9},{2,13},{3,6},{3,8},{3,10},{4,6},{4,7},{4,9},{4,11},{5,7},{5,9},{5,10},{5,13},{6,8},{6,12},{7,8},{8,11},{8,13},{9,12},{10,11},{10,12},{11,12}}

Cousin 972: {{1,4},{1,7},{1,9},{2,4},{2,6},{2,7},{2,9},{2,13},{3,6},{3,7},{3,8},{3,9},{3,10},{4,6},{4,11},{5,7},{5,9},{5,10},{5,13},{6,8},{6,12},{7,8},{8,11},{8,13},{9,12},{10,11},{10,12},{11,12}}

Cousin 973: {{1,5},{1,7},{1,9},{2,4},{2,6},{2,7},{2,9},{2,13},{3,6},{3,7},{3,8},{3,9},{3,10},{4,6},{4,7},{4,9},{4,11},{5,10},{5,13},{6,8},{6,12},{7,8},{8,11},{8,13},{9,12},{10,11},{10,12},{11,12}}

Cousin 974: {{1,10},{1,11},{1,12},{2,4},{2,7},{2,13},{2,14},{3,6},{3,9},{3,10},{3,15},{4,6},{4,7},{4,9},{4,11},{5,7},{5,8},{5,10},{5,13},{6,12},{6,14},{7,9},{7,15},{8,11},{8,14},{8,15},{9,12},{9,13}}

Cousin 975: {{1,10},{1,11},{1,12},{2,4},{2,7},{2,13},{2,14},{3,6},{3,8},{3,10},{3,15},{4,6},{4,7},{4,9},{4,11},{5,7},{5,8},{5,10},{5,13},{6,12},{6,14},{7,8},{7,15},{8,11},{8,14},{9,12},{9,13},{9,15}}

Cousin 976: {{1,10},{1,11},{1,12},{2,4},{2,7},{2,13},{2,14},{3,6},{3,7},{3,8},{3,9},{3,10},{4,6},{4,11},{4,15},{5,7},{5,8},{5,10},{5,13},{6,12},{6,14},{7,8},{7,15},{8,11},{8,14},{9,12},{9,13},{9,15}}

Cousin 977: {{1,10},{1,11},{1,12},{2,4},{2,7},{2,13},{2,14},{3,6},{3,7},{3,8},{3,9},{3,10},{4,6},{4,7},{4,9},{4,11},{5,10},{5,13},{5,15},{6,12},{6,14},{7,9},{7,15},{8,11},{8,14},{8,15},{9,12},{9,13}}

Cousin 978: {{1,2},{1,6},{1,8},{2,4},{2,7},{2,13},{3,6},{3,7},{3,8},{3,9},{3,10},{4,6},{4,7},{4,9},{4,11},{5,7},{5,8},{5,10},{5,13},{6,12},{7,8},{7,9},{8,11},{9,12},{9,13},{10,11},{10,12},{11,12}}

Cousin 979: {{1,10},{1,11},{1,12},{2,4},{2,6},{2,13},{2,14},{3,7},{3,9},{3,10},{3,15},{4,6},{4,7},{4,9},{4,11},{5,7},{5,8},{5,10},{5,13},{6,12},{6,15},{7,9},{7,14},{8,11},{8,14},{8,15},{9,12},{9,13}}

Cousin 980: {{1,10},{1,11},{1,12},{2,4},{2,6},{2,13},{2,14},{3,6},{3,8},{3,10},{3,15},{4,6},{4,7},{4,9},{4,11},{5,7},{5,8},{5,10},{5,13},{6,8},{6,12},{7,14},{7,15},{8,11},{8,14},{9,12},{9,13},{9,15}}

Cousin 981: {{1,10},{1,11},{1,12},{2,4},{2,6},{2,13},{2,14},{3,6},{3,7},{3,8},{3,9},{3,10},{4,6},{4,11},{4,15},{5,7},{5,8},{5,10},{5,13},{6,8},{6,12},{7,14},{7,15},{8,11},{8,14},{9,12},{9,13},{9,15}}

Cousin 982: {{1,2},{1,7},{1,8},{2,4},{2,6},{2,13},{3,6},{3,7},{3,8},{3,9},{3,10},{4,6},{4,7},{4,9},{4,11},{5,7},{5,8},{5,10},{5,13},{6,8},{6,12},{7,9},{8,11},{9,12},{9,13},{10,11},{10,12},{11,12}}

Cousin 983: {{1,10},{1,11},{1,12},{2,4},{2,6},{2,7},{2,8},{2,13},{3,10},{3,14},{3,15},{4,6},{4,7},{4,9},{4,11},{5,7},{5,8},{5,10},{5,13},{6,12},{6,14},{7,8},{7,15},{8,11},{8,14},{9,12},{9,13},{9,15}}

Cousin 984: {{1,10},{1,11},{1,12},{2,4},{2,6},{2,7},{2,8},{2,13},{3,7},{3,9},{3,10},{3,14},{4,6},{4,11},{4,15},{5,7},{5,8},{5,10},{5,13},{6,12},{6,14},{7,8},{7,15},{8,11},{8,14},{9,12},{9,13},{9,15}}

Cousin 985: {{1,10},{1,11},{1,12},{2,4},{2,6},{2,7},{2,8},{2,13},{3,7},{3,9},{3,10},{3,14},{4,6},{4,7},{4,9},{4,11},{5,10},{5,13},{5,15},{6,12},{6,14},{7,9},{7,15},{8,11},{8,14},{8,15},{9,12},{9,13}}

Cousin 986: {{1,3},{1,6},{1,8},{2,4},{2,6},{2,7},{2,8},{2,13},{3,7},{3,9},{3,10},{4,6},{4,7},{4,9},{4,11},{5,7},{5,8},{5,10},{5,13},{6,12},{7,8},{7,9},{8,11},{9,12},{9,13},{10,11},{10,12},{11,12}}

{9,13},{10,11},{10,12},{11,12}}

Cousin 987: {{1,10},{1,11},{1,12},{2,4},{2,6},{2,7},{2,8},{2,13},{3,6},{3,9},{3,10},{3,14},{4,6},{4,11},{4,15},{5,7},{5,8},{5,10},{5,13},{6,8},{6,12},{7,14},{7,15},{8,11},{8,14},{9,12},{9,13},{9,15}}

Cousin 988: {{1,3},{1,7},{1,8},{2,4},{2,6},{2,7},{2,8},{2,13},{3,6},{3,9},{3,10},{4,6},{4,7},{4,9},{4,11},{5,7},{5,8},{5,10},{5,13},{6,8},{6,12},{7,9},{8,11},{9,12},{9,13},{10,11},{10,12},{11,12}}

Cousin 989: {{1,3},{1,7},{1,9},{2,4},{2,6},{2,7},{2,8},{2,13},{3,6},{3,8},{3,10},{4,6},{4,7},{4,9},{4,11},{5,7},{5,8},{5,10},{5,13},{6,8},{6,12},{7,8},{8,11},{9,12},{9,13},{10,11},{10,12},{11,12}}

Cousin 990: {{1,4},{1,7},{1,9},{2,4},{2,6},{2,7},{2,8},{2,13},{3,6},{3,7},{3,8},{3,9},{3,10},{4,6},{4,11},{5,7},{5,8},{5,10},{5,13},{6,8},{6,12},{7,8},{8,11},{9,12},{9,13},{10,11},{10,12},{11,12}}

Cousin 991: {{1,5},{1,7},{1,8},{2,4},{2,6},{2,7},{2,8},{2,13},{3,6},{3,7},{3,8},{3,9},{3,10},{4,6},{4,7},{4,9},{4,11},{5,10},{5,13},{6,8},{6,12},{7,9},{8,11},{9,12},{9,13},{10,11},{10,12},{11,12}}

Cousin 992: {{1,10},{1,11},{1,12},{2,4},{2,5},{2,13},{2,14},{3,6},{3,9},{3,10},{3,15},{4,6},{4,7},{4,9},{4,11},{5,7},{5,8},{5,9},{5,10},{6,12},{6,13},{7,14},{7,15},{8,11},{8,13},{8,15},{9,12},{9,14}}

Cousin 993: {{1,10},{1,11},{1,12},{2,4},{2,5},{2,13},{2,14},{3,6},{3,7},{3,8},{3,9},{3,10},{4,6},{4,7},{4,9},{4,11},{5,9},{5,10},{5,15},{6,12},{6,13},{7,14},{7,15},{8,11},{8,13},{8,15},{9,12},{9,14}}

Cousin 994: {{1,2},{1,7},{1,9},{2,4},{2,5},{2,13},{3,6},{3,7},{3,8},{3,9},{3,10},{4,6},{4,7},{4,9},{4,11},{5,7},{5,8},{5,9},{5,10},{6,12},{6,13},{7,8},{8,11},{8,13},{9,12},{10,11},{10,12},{11,12}}

Cousin 995: {{1,10},{1,11},{1,12},{2,4},{2,5},{2,7},{2,9},{2,13},{3,6},{3,9},{3,10},{3,14},{4,6},{4,11},{4,15},{5,7},{5,8},{5,9},{5,10},{6,12},{6,13},{7,14},{7,15},{8,11},{8,13},{8,14},{9,12},{9,15}}

Cousin 996: {{1,10},{1,11},{1,12},{2,4},{2,5},{2,7},{2,9},{2,13},{3,6},{3,9},{3,10},{3,14},{4,6},{4,7},{4,9},{4,11},{5,8},{5,10},{5,15},{6,12},{6,13},{7,14},{7,15},{8,11},{8,13},{8,14},{9,12},{9,15}}

Cousin 997: {{1,3},{1,7},{1,8},{2,4},{2,5},{2,7},{2,9},{2,13},{3,6},{3,9},{3,10},{4,6},{4,7},{4,9},{4,11},{5,7},{5,8},{5,9},{5,10},{6,12},{6,13},{7,9},{8,11},{8,13},{9,12},{10,11},{10,12},{11,12}}

Cousin 998: {{1,10},{1,11},{1,12},{2,4},{2,5},{2,7},{2,9},{2,13},{3,6},{3,8},{3,10},{3,14},{4,6},{4,7},{4,9},{4,11},{5,9},{5,10},{5,15},{6,12},{6,13},{7,14},{7,15},{8,11},{8,13},{8,15},{9,12},{9,14}}

Cousin 999: {{1,3},{1,7},{1,9},{2,4},{2,5},{2,7},{2,9},{2,13},{3,6},{3,8},{3,10},{4,6},{4,7},{4,9},{4,11},{5,7},{5,8},{5,9},{5,10},{6,12},{6,13},{7,8},{8,11},{8,13},{9,12},{10,11},{10,12},{11,12}}

Cousin 1000: {{1,10},{1,11},{1,12},{2,4},{2,5},{2,7},{2,9},{2,13},{3,6},{3,7},{3,8},{3,9},{3,10},{4,6},{4,11},{4,14},{5,9},{5,10},{5,15},{6,12},{6,13},{7,14},{7,15},{8,11},{8,13},{8,15},{9,12},{9,14}}

Cousin 1001: {{1,4},{1,7},{1,9},{2,4},{2,5},{2,7},{2,9},{2,13},{3,6},{3,7},{3,8},{3,9},{3,10},{4,6},{4,11},{5,7},{5,8},{5,9},{5,10},{6,12},{6,13},{7,8},{8,11},{8,13},{9,12},{10,11},{10,12},{11,12}}

Cousin 1002: {{1,5},{1,7},{1,8},{2,4},{2,5},{2,7},{2,9},{2,13},{3,6},{3,7},{3,8},{3,9},{3,10},{4,6},{4,7},{4,9},{4,11},{5,9},{5,10},{6,12},{6,13},{7,9},{8,11},{8,13},{9,12},{10,11},{10,12},{11,12}}

Cousin 1003: {{1,5},{1,7},{1,9},{2,4},{2,5},{2,7},{2,9},{2,13},{3,6},{3,7},{3,8},{3,9},{3,10},{4,6},{4,7},{4,9},{4,11},{5,8},{5,10},{6,12},{6,13},{7,8},{8,11},{8,13},{9,12},{10,11},{10,12},{11,12}}

Cousin 1004: {{1,10},{1,11},{1,12},{2,4},{2,5},{2,6},{2,9},{2,13},{3,10},{3,14},{3,15},{4,6},{4,7},{4,9},{4,11},{5,7},{5,8},{5,9},{5,10},{6,12},{6,14},{7,13},{7,15},{8,11},{8,13},{8,14},{9,12},{9,15}}

Cousin 1005: {{1,10},{1,11},{1,12},{2,4},{2,5},{2,6},{2,9},{2,13},{3,7},{3,9},{3,10},{3,14},{4,6},{4,11},{4,15},{5,7},{5,8},{5,9},{5,10},{6,12},{6,14},{7,13},{7,15},{8,11},{8,13},{8,14},{9,12},{9,15}}

Cousin 1006: {{1,10},{1,11},{1,12},{2,4},{2,5},{2,6},{2,9},{2,13},{3,7},{3,9},{3,10},{3,14},{4,6},{4,7},{4,9},{4,11},{5,8},{5,10},{5,15},{6,12},{6,14},{7,13},{7,15},{8,11},{8,13},{8,14},{9,12},{9,15}}

Cousin 1007: {{1,3},{1,6},{1,8},{2,4},{2,5},{2,6},{2,9},{2,13},{3,7},{3,9},{3,10},{4,6},{4,7},{4,9},{4,11},{5,7},{5,8},{5,9},{5,10},{6,12},{7,9},{7,13},{8,11},{8,13},{9,12},{10,11},{10,12},{11,12}}

Cousin 1008: {{1,3},{1,7},{1,9},{2,4},{2,5},{2,6},{2,9},{2,13},{3,6},{3,8},{3,10},{4,6},{4,7},{4,9},{4,11},{5,7},{5,8},{5,9},{5,10},{6,8},{6,12},{7,13},{8,11},{8,13},{9,12},{10,11},{10,12},{11,12}}

Cousin 1009: {{1,4},{1,7},{1,9},{2,4},{2,5},{2,6},{2,9},{2,13},{3,6},{3,7},{3,8},{3,9},{3,10},{4,6},{4,11},{5,7},{5,8},{5,9},{5,10},{6,8},{6,12},{7,13},{8,11},{8,13},{9,12},{10,11},{10,12},{11,12}}

Cousin 1010: {{1,5},{1,7},{1,9},{2,4},{2,5},{2,6},{2,9},{2,13},{3,6},{3,7},{3,8},{3,9},{3,10},{4,6},{4,7},{4,9},{4,11},{5,8},{5,10},{6,8},{6,12},{7,13},{8,11},{8,13},{9,12},{10,11},{10,12},{11,12}}

Cousin 1011: {{1,10},{1,11},{1,12},{2,4},{2,5},{2,6},{2,8},{2,13},{3,7},{3,9},{3,10},{3,14},{4,6},{4,7},{4,9},{4,11},{5,9},{5,10},{5,15},{6,12},{6,14},{7,13},{7,15},{8,11},{8,14},{8,15},{9,12},{9,13}}

Cousin 1012: {{1,3},{1,6},{1,8},{2,4},{2,5},{2,6},{2,8},{2,13},{3,7},{3,9},{3,10},{4,6},{4,7},{4,9},{4,11},{5,7},{5,8},{5,9},{5,10},{6,12},{7,8},{7,13},{8,11},{9,12},{9,13},{10,11},{10,12},{11,12}}

Cousin 1013: {{1,3},{1,7},{1,8},{2,4},{2,5},{2,6},{2,8},{2,13},{3,6},{3,9},{3,10},{4,6},{4,7},{4,9},{4,11},{5,7},{5,8},{5,9},{5,10},{6,8},{6,12},{7,13},{8,11},{9,12},{9,13},{10,11},{10,12},{11,12}}

Cousin 1014: {{1,5},{1,7},{1,8},{2,4},{2,5},{2,6},{2,8},{2,13},{3,6},{3,7},{3,8},{3,9},{3,10},{4,6},{4,7},{4,9},{4,11},{5,9},{5,10},{6,8},{6,12},{7,13},{8,11},{9,12},{9,13},{10,11},{10,12},{11,12}}

Cousin 1015: {{1,10},{1,11},{1,12},{2,4},{2,5},{2,6},{2,7},{2,8},{2,9},{3,10},{3,13},{3,14},{4,6},{4,7},{4,9},{4,11},{5,9},{5,10},{5,15},{6,12},{6,13},{7,14},{7,15},{8,11},{8,13},{8,15},{9,12},{9,14}}

Cousin 1016: {{1,3},{1,7},{1,9},{2,4},{2,5},{2,6},{2,7},{2,8},{2,9},{3,10},{3,13},{4,6},{4,7},{4,9},{4,11},{5,7},{5,8},{5,9},{5,10},{6,12},{6,13},{7,8},{8,11},{8,13},{9,12},{10,11},{10,12},{11,12}}

Cousin 1017: {{1,10},{1,11},{1,12},{2,4},{2,5},{2,6},{2,7},{2,8},{2,9},{3,7},{3,9},{3,10},{3,13},{4,6},{4,7},{4,9},{4,11},{5,7},{5,8},{5,9},{5,10},{6,12},{6,13},{7,8},{8,11},{8,13},{9,12},{10,13}}

Cousin 1018: {{1,10},{1,11},{1,12},{2,4},{2,5},{2,6},{2,7},{2,8},{2,9},{3,7},{3,9},{3,10},{3,13},{4,6},{4,11},{4,14},{5,9},{5,10},{5,15},{6,12},{6,13},{7,14},{7,15},{8,11},{8,13},{8,15},{9,12},{9,14}}

Cousin 1019: {{1,4},{1,7},{1,9},{2,4},{2,5},{2,6},{2,7},{2,8},{2,9},{3,7},{3,9},{3,10},{3,13},{4,6},{4,11},{5,7},{5,8},{5,9},{5,10},{6,12},{6,13},{7,8},{8,11},{8,13},{9,12},{10,11},{10,12},{11,12}}

Cousin 1020: {{1,5},{1,7},{1,8},{2,4},{2,5},{2,6},{2,7},{2,8},{2,9},{3,7},{3,9},{3,10},{3,13},{4,6},{4,7},{4,9},{4,11},{5,9},{5,10},{6,12},{6,13},{7,9},{8,11},{8,13},{9,12},{10,11},{10,12},{11,12}}

Cousin 1021: {{1,5},{1,7},{1,9},{2,4},{2,5},{2,6},{2,7},{2,8},{2,9},{3,7},{3,9},{3,10},{3,13},{4,6},{4,7},{4,9},{4,11},{5,8},{5,10},{6,12},{6,13},{7,8},{8,11},{8,13},{9,12},{10,11},{10,12},{11,12}}

Cousin 1022: {{1,4},{1,7},{1,9},{2,4},{2,5},{2,6},{2,7},{2,8},{2,9},{3,6},{3,9},{3,10},{3,13},{4,6},{4,11},{5,7},{5,8},{5,9},{5,10},{6,8},{6,12},{7,13},{8,11},{8,13},{9,12},{10,11},{10,12},{11,12}}

Cousin 1023: {{1,5},{1,7},{1,9},{2,4},{2,5},{2,6},{2,7},{2,8},{2,9},{3,6},{3,9},{3,10},{3,13},{4,6},{4,7},{4,9},{4,11},{5,8},{5,10},{6,8},{6,12},{7,13},{8,11},{8,13},{9,12},{10,11},{10,12},{11,12}}

Cousin 1024: {{1,5},{1,7},{1,8},{2,4},{2,5},{2,6},{2,7},{2,8},{2,9},{3,6},{3,8},{3,10},{3,13},{4,6},{4,7},{4,9},{4,11},{5,9},{5,10},{6,8},{6,12},{7,13},{8,11},{9,12},{9,13},{10,11},{10,12},{11,12}}

Cousin 1025: {{1,5},{1,7},{1,8},{2,4},{2,5},{2,6},{2,7},{2,8},{2,9},{3,6},{3,7},{3,8},{3,9},{3,10},{4,6},{4,11},{4,13},{5,9},{5,10},{6,8},{6,12},{7,13},{8,11},{9,12},{9,13},{10,11},{10,12},{11,12}}

Cousin 1026: {{1,6},{1,9},{1,10},{1,11},{2,7},{2,9},{2,12},{2,13},{3,10},{3,14},{3,15},{4,7},{4,9},{4,11},{4,12},{5,7},{5,9},{5,10},{5,13},{6,9},{6,12},{6,14},{7,8},{7,15},{8,11},{8,13},{8,14},{9,15}}

Cousin 1027: {{1,6},{1,9},{1,10},{1,11},{2,7},{2,9},{2,12},{2,13},{3,10},{3,14},{3,15},{4,7},{4,9},{4,11},{4,12},{5,7},{5,9},{5,10},{5,13},{6,8},{6,12},{6,14},{7,9},{7,15},{8,11},{8,13},{8,15},{9,14}}

Cousin 1028: {{1,6},{1,9},{1,10},{1,11},{2,7},{2,9},{2,12},{2,13},{3,7},{3,8},{3,10},{3,14},{4,11},{4,12},{4,15},{5,7},{5,9},{5,10},{5,13},{6,8},{6,12},{6,14},{7,8},{7,15},{8,11},{8,13},{9,14},{9,15}}

Cousin 1029: {{1,6},{1,9},{1,10},{1,11},{2,7},{2,9},{2,12},{2,13},{3,6},{3,9},{3,10},{3,14},{4,11},{4,12},{4,15},{5,7},{5,9},{5,10},{5,13},{6,8},{6,9},{6,12},{7,14},{7,15},{8,11},{8,13},{8,14},{9,15}}

Cousin 1030: {{1,6},{1,9},{1,10},{1,11},{2,7},{2,9},{2,12},{2,13},{3,6},{3,7},{3,8},{3,9},{3,10},{4,7},{4,9},{4,11},{4,12},{5,7},{5,9},{5,10},{5,13},{6,8},{6,9},{6,12},{7,8},{8,11},{8,13},{11,12}}

Cousin 1031: {{1,6},{1,9},{1,10},{1,11},{2,7},{2,8},{2,12},{2,13},{3,10},{3,14},{3,15},{4,7},{4,9},{4,11},{4,12},{5,7},{5,8},{5,10},{5,13},{6,9},{6,12},{6,14},{7,8},{7,15},{8,11},{8,14},{9,13},{9,15}}

Cousin 1032: {{1,6},{1,9},{1,10},{1,11},{2,7},{2,8},{2,12},{2,13},{3,6},{3,9},{3,10},{3,14},{4,11},{4,12},{4,15},{5,7},{5,8},{5,10},{5,13},{6,8},{6,9},{6,12},{7,14},{7,15},{8,11},{8,14},{9,13},{9,15}}

Cousin 1033: {{1,6},{1,9},{1,10},{1,11},{2,7},{2,8},{2,12},{2,13},{3,6},{3,7},{3,8},{3,9},{3,10},{4,7},{4,9},{4,11},{4,12},{5,7},{5,8},{5,10},{5,13},{6,8},{6,9},{6,12},{7,8},{8,11},{9,13},{11,12}}

Cousin 1034: {{1,6},{1,9},{1,10},{1,11},{2,5},{2,9},{2,12},{2,13},{3,10},{3,14},{3,15},{4,7},{4,9},{4,11},{4,12},{5,7},{5,8},{5,9},{5,10},{6,9},{6,12},{6,14},{7,13},{7,15},{8,11},{8,13},{8,14},{9,15}}

Cousin 1035: {{1,6},{1,9},{1,10},{1,11},{2,5},{2,9},{2,12},{2,13},{3,7},{3,9},{3,10},{3,14},{4,11},{4,12},{4,15},{5,7},{5,8},{5,9},{5,10},{6,9},{6,12},{6,14},{7,13},{7,15},{8,11},{8,13},{8,14},{9,15}}

Cousin 1036: {{1,6},{1,9},{1,10},{1,11},{2,5},{2,9},{2,12},{2,13},{3,7},{3,9},{3,10},{3,14},{4,7},{4,9},{4,11},{4,12},{5,8},{5,10},{5,15},{6,9},{6,12},{6,14},{7,13},{7,15},{8,11},{8,13},{8,14},{9,15}}

Cousin 1037: {{1,6},{1,9},{1,10},{1,11},{2,5},{2,9},{2,12},{2,13},{3,7},{3,8},{3,10},{3,14},{4,11},{4,12},{4,15},{5,7},{5,8},{5,9},{5,10},{6,8},{6,12},{6,14},{7,13},{7,15},{8,11},{8,13},{9,14},{9,15}}

Cousin 1038: {{1,6},{1,9},{1,10},{1,11},{2,5},{2,9},{2,12},{2,13},{3,7},{3,8},{3,10},{3,14},{4,7},{4,9},{4,11},{4,12},{5,8},{5,10},{5,15},{6,8},{6,12},{6,14},{7,13},{7,15},{8,11},{8,13},{9,14},{9,15}}

Cousin 1039: {{1,6},{1,9},{1,10},{1,11},{2,5},{2,9},{2,12},{2,13},{3,6},{3,7},{3,8},{3,9},{3,10},{4,7},{4,9},{4,11},{4,12},{5,7},{5,8},{5,9},{5,10},{6,8},{6,9},{6,12},{7,13},{8,11},{8,13},{11,12}}

Cousin 1040: {{1,6},{1,9},{1,10},{1,11},{2,5},{2,8},{2,12},{2,13},{3,10},{3,14},{3,15},{4,7},{4,9},{4,11},{4,12},{5,7},{5,8},{5,9},{5,10},{6,8},{6,12},{6,14},{7,13},{7,15},{8,11},{8,15},{9,13},{9,14}}

Cousin 1041: {{1,6},{1,9},{1,10},{1,11},{2,5},{2,8},{2,12},{2,13},{3,7},{3,8},{3,10},{3,14},{4,7},{4,9},{4,11},{4,12},{5,9},{5,10},{5,15},{6,8},{6,12},{6,14},{7,13},{7,15},{8,11},{8,15},{9,13},{9,14}}

Cousin 1042: {{1,6},{1,9},{1,10},{1,11},{2,5},{2,7},{2,8},{2,9},{2,12},{3,7},{3,9},{3,10},{3,13},{4,7},{4,9},{4,11},{4,12},{5,7},{5,8},{5,9},{5,10},{6,9},{6,12},{6,13},{7,8},{8,11},{8,13},{10,13}}

Cousin 1043: {{1,6},{1,9},{1,10},{1,11},{2,5},{2,7},{2,8},{2,9},{2,12},{3,10},{3,13},{3,14},{4,11},{4,12},{4,15},{5,7},{5,8},{5,9},{5,10},{6,8},{6,12},{6,13},{7,14},{7,15},{8,11},{8,14},{9,13},{9,15}}

Cousin 1044: {{1,6},{1,9},{1,10},{1,11},{2,5},{2,7},{2,8},{2,9},{2,12},{3,7},{3,8},{3,10},{3,13},{4,7},{4,9},{4,11},{4,12},{5,7},{5,8},{5,9},{5,10},{6,8},{6,12},{6,13},{7,9},{8,11},{9,13},{10,13}}

Cousin 1045: {{1,6},{1,9},{1,10},{1,11},{2,5},{2,7},{2,8},{2,9},{2,12},{3,6},{3,9},{3,10},{3,13},{4,7},{4,9},{4,11},{4,12},{5,7},{5,8},{5,9},{5,10},{6,8},{6,9},{6,12},{7,13},{8,11},{8,13},{11,12}}

Cousin 1046: {{1,6},{1,9},{1,10},{1,11},{2,5},{2,7},{2,8},{2,9},{2,12},{3,6},{3,7},{3,8},{3,9},{3,10},{4,5},{4,7},{4,8},{5,9},{5,10},{6,8},{6,9},{6,12},{7,13},{8,11},{9,13},{11,12},{11,13},{12,13}}

Cousin 1047: {{1,6},{1,9},{1,10},{1,11},{2,5},{2,9},{2,12},{2,13},{3,7},{3,8},{3,10},{3,14},{4,6},{4,9},{4,11},{4,12},{5,9},{5,10},{5,15},{6,13},{6,14},{7,9},{7,12},{7,15},{8,11},{8,13},{8,15},{9,14}}

Cousin 1048: {{1,6},{1,9},{1,10},{1,11},{2,5},{2,9},{2,12},{2,13},{3,7},{3,8},{3,10},{3,14},{4,6},{4,9},{4,11},{4,12},{5,8},{5,10},{5,15},{6,13},{6,14},{7,8},{7,12},{7,15},{8,11},{8,13},{9,14},{9,15}}

Cousin 1049: {{1,6},{1,9},{1,10},{1,11},{2,6},{2,7},{2,12},{2,13},{3,10},{3,14},{3,15},{4,6},{4,7},{4,11},{4,12},{5,7},{5,9},{5,10},{5,13},{6,9},{6,14},{7,8},{7,15},{8,11},{8,13},{8,14},{9,12},{9,15}}

Cousin 1050: {{1,6},{1,9},{1,10},{1,11},{2,5},{2,7},{2,12},{2,13},{3,10},{3,14},{3,15},{4,6},{4,7},{4,11},{4,12},{5,7},{5,8},{5,9},{5,10},{6,13},{6,14},{7,9},{7,15},{8,11},{8,13},{8,15},{9,12},{9,14}}

Cousin 1051: {{1,6},{1,9},{1,10},{1,11},{2,5},{2,7},{2,12},{2,13},{3,7},{3,8},{3,10},{3,14},{4,6},{4,7},{4,11},{4,12},{5,9},{5,10},{5,15},{6,13},{6,14},{7,9},{7,15},{8,11},{8,13},{8,15},{9,12},{9,14}}

Cousin 1052: {{1,6},{1,9},{1,10},{1,11},{2,5},{2,7},{2,12},{2,13},{3,7},{3,8},{3,10},{3,14},{4,6},{4,7},{4,11},{4,12},{5,8},{5,10},{5,15},{6,13},{6,14},{7,8},{7,15},{8,11},{8,13},{9,12},{9,14},{9,15}}

Cousin 1053: {{1,6},{1,9},{1,10},{1,11},{2,5},{2,7},{2,12},{2,13},{3,6},{3,9},{3,10},{3,14},{4,6},{4,7},{4,11},{4,12},{5,8},{5,10},{5,15},{6,9},{6,13},{7,14},{7,15},{8,11},{8,13},{8,14},{9,12},{9,15}}

Cousin 1054: {{1,6},{1,9},{1,10},{1,11},{2,5},{2,7},{2,12},{2,13},{3,6},{3,8},{3,10},{3,14},{4,6},{4,7},{4,11},{4,12},{5,9},{5,10},{5,15},{6,9},{6,13},{7,14},{7,15},{8,11},{8,13},{8,15},{9,12},{9,14}}

Cousin 1055: {{1,6},{1,9},{1,10},{1,11},{2,5},{2,6},{2,12},{2,13},{3,10},{3,14},{3,15},{4,6},{4,7},{4,11},{4,12},{5,7},{5,8},{5,9},{5,10},{6,9},{6,14},{7,13},{7,15},{8,11},{8,13},{8,14},{9,12},{9,15}}

Cousin 1056: {{1,6},{1,9},{1,10},{1,11},{2,5},{2,6},{2,12},{2,13},{3,7},{3,9},{3,10},{3,14},{4,6},{4,7},{4,11},{4,12},{5,8},{5,10},{5,15},{6,9},{6,14},{7,13},{7,15},{8,11},{8,13},{8,14},{9,12},{9,15}}

Cousin 1057: {{1,6},{1,9},{1,10},{1,11},{2,5},{2,6},{2,12},{2,13},{3,7},{3,8},{3,10},{3,14},{4,6},{4,7},{4,11},{4,12},{5,8},{5,10},{5,15},{6,8},{6,14},{7,13},{7,15},{8,11},{8,13},{9,12},{9,14},{9,15}}

Cousin 1058: {{1,6},{1,9},{1,10},{1,11},{2,5},{2,6},{2,7},{2,8},{2,12},{3,10},{3,13},{3,14},{4,6},{4,7},{4,11},{4,12},{5,9},{5,10},{5,15},{6,9},{6,13},{7,14},{7,15},{8,11},{8,13},{8,15},{9,12},{9,14}}

Cousin 1059: {{1,6},{1,9},{1,10},{1,11},{2,5},{2,6},{2,7},{2,8},{2,12},{3,7},{3,9},{3,10},{3,13},{4,6},{4,7},{4,11},{4,12},{5,7},{5,8},{5,9},{5,10},{6,9},{6,13},{7,8},{8,11},{8,13},{9,12},{10,13}}

Cousin 1060: {{1,6},{1,9},{1,10},{1,11},{2,5},{2,6},{2,7},{2,8},{2,12},{3,10},{3,13},{3,14},{4,6},{4,7},{4,11},{4,12},{5,8},{5,10},{5,15},{6,8},{6,13},{7,14},{7,15},{8,11},{8,14},{9,12},{9,13},{9,15}}

Cousin 1061: {{1,6},{1,9},{1,10},{1,11},{2,5},{2,6},{2,7},{2,8},{2,12},{3,7},{3,8},{3,10},{3,13},{4,6},{4,7},{4,11},{4,12},{5,7},{5,8},{5,9},{5,10},{6,8},{6,13},{7,9},{8,11},{9,12},{9,13},{10,13}}

Cousin 1062: {{1,6},{1,9},{1,10},{1,11},{2,4},{2,7},{2,12},{2,13},{3,10},{3,14},{3,15},{4,6},{4,7},{4,9},{4,11},{5,7},{5,9},{5,10},{5,12},{6,13},{6,14},{7,8},{7,15},{8,11},{8,13},{8,15},{9,12},{9,14},{9,15}}

{8,11},{8,12},{8,14},{9,13},{9,15}}

Cousin 1063: {{1,6},{1,9},{1,10},{1,11},{2,4},{2,7},{2,12},{2,13},{3,7},{3,9},{3,10},{3,14},{4,6},{4,11},{4,15},{5,7},{5,9},{5,10},{5,12},{6,13},{6,14},{7,8},{7,15},{8,11},{8,12},{8,14},{9,13},{9,15}}

Cousin 1064: {{1,6},{1,9},{1,10},{1,11},{2,4},{2,6},{2,12},{2,13},{3,7},{3,9},{3,10},{3,14},{4,7},{4,11},{4,15},{5,7},{5,9},{5,10},{5,12},{6,14},{6,15},{7,8},{7,13},{8,11},{8,12},{8,14},{9,13},{9,15}}

Cousin 1065: {{1,6},{1,9},{1,10},{1,11},{2,4},{2,6},{2,12},{2,13},{3,10},{3,14},{3,15},{4,6},{4,7},{4,9},{4,11},{5,7},{5,9},{5,10},{5,12},{6,8},{6,14},{7,13},{7,15},{8,11},{8,12},{8,15},{9,13},{9,14}}

Cousin 1066: {{1,6},{1,9},{1,10},{1,11},{2,4},{2,6},{2,7},{2,9},{2,12},{3,7},{3,9},{3,10},{3,13},{4,6},{4,7},{4,9},{4,11},{5,7},{5,9},{5,10},{5,12},{6,9},{6,13},{7,8},{8,11},{8,12},{8,13},{10,13}}

Cousin 1067: {{1,6},{1,9},{1,10},{1,11},{2,4},{2,7},{2,12},{2,13},{3,10},{3,14},{3,15},{4,6},{4,7},{4,9},{4,11},{5,7},{5,8},{5,10},{5,12},{6,13},{6,14},{7,9},{7,15},{8,11},{8,13},{8,15},{9,12},{9,14}}

Cousin 1068: {{1,6},{1,9},{1,10},{1,11},{2,4},{2,7},{2,12},{2,13},{3,7},{3,8},{3,10},{3,14},{4,6},{4,11},{4,15},{5,7},{5,8},{5,10},{5,12},{6,13},{6,14},{7,8},{7,15},{8,11},{8,13},{9,12},{9,14},{9,15}}

Cousin 1069: {{1,6},{1,9},{1,10},{1,11},{2,4},{2,7},{2,12},{2,13},{3,6},{3,9},{3,10},{3,14},{4,7},{4,11},{4,15},{5,7},{5,8},{5,10},{5,12},{6,13},{6,15},{7,9},{7,14},{8,11},{8,13},{8,14},{9,12},{9,15}}

Cousin 1070: {{1,6},{1,9},{1,10},{1,11},{2,4},{2,7},{2,12},{2,13},{3,6},{3,8},{3,10},{3,14},{4,7},{4,11},{4,15},{5,7},{5,8},{5,10},{5,12},{6,13},{6,15},{7,8},{7,14},{8,11},{8,13},{9,12},{9,14},{9,15}}

Cousin 1071: {{1,6},{1,9},{1,10},{1,11},{2,4},{2,6},{2,12},{2,13},{3,10},{3,14},{3,15},{4,6},{4,7},{4,9},{4,11},{5,7},{5,8},{5,10},{5,12},{6,9},{6,14},{7,13},{7,15},{8,11},{8,13},{8,14},{9,12},{9,15}}

Cousin 1072: {{1,6},{1,9},{1,10},{1,11},{2,4},{2,6},{2,12},{2,13},{3,7},{3,9},{3,10},{3,14},{4,7},{4,11},{4,15},{5,7},{5,8},{5,10},{5,12},{6,14},{6,15},{7,9},{7,13},{8,11},{8,13},{8,14},{9,12},{9,15}}

Cousin 1073: {{1,6},{1,9},{1,10},{1,11},{2,4},{2,6},{2,7},{2,8},{2,12},{3,7},{3,9},{3,10},{3,13},{4,6},{4,7},{4,9},{4,11},{5,7},{5,8},{5,10},{5,12},{6,9},{6,13},{7,8},{8,11},{8,13},{9,12},{10,13}}

Cousin 1074: {{1,6},{1,9},{1,10},{1,11},{2,4},{2,6},{2,7},{2,8},{2,12},{3,7},{3,8},{3,10},{3,13},{4,6},{4,7},{4,9},{4,11},{5,7},{5,8},{5,10},{5,12},{6,8},{6,13},{7,9},{8,11},{9,12},{9,13},{10,13}}

Cousin 1075: {{1,6},{1,9},{1,10},{1,11},{2,4},{2,5},{2,12},{2,13},{3,10},{3,14},{3,15},{4,6},{4,7},{4,9},{4,11},{5,7},{5,8},{5,9},{5,10},{6,12},{6,14},{7,13},{7,15},{8,11},{8,12},{8,15},{9,13},{9,14}}

Cousin 1076: {{1,6},{1,9},{1,10},{1,11},{2,4},{2,5},{2,12},{2,13},{3,7},{3,8},{3,10},{3,14},{4,6},{4,7},{4,9},{4,11},{5,9},{5,10},{5,15},{6,12},{6,14},{7,13},{7,15},{8,11},{8,12},{8,15},{9,13},{9,14}}

Cousin 1077: {{1,6},{1,9},{1,10},{1,11},{2,4},{2,5},{2,12},{2,13},{3,6},{3,9},{3,10},{3,14},{4,7},{4,11},{4,15},{5,7},{5,8},{5,9},{5,10},{6,12},{6,15},{7,13},{7,14},{8,11},{8,12},{8,14},{9,13},{9,15}}

Cousin 1078: {{1,6},{1,9},{1,10},{1,11},{2,4},{2,5},{2,12},{2,13},{3,6},{3,7},{3,8},{3,9},{3,10},{4,7},{4,11},{4,14},{5,9},{5,10},{5,15},{6,12},{6,14},{7,13},{7,15},{8,11},{8,12},{8,15},{9,13},{9,14}}

Cousin 1079: {{1,6},{1,9},{1,10},{1,11},{2,4},{2,5},{2,7},{2,9},{2,12},{3,10},{3,13},{3,14},{4,6},{4,11},{4,15},{5,7},{5,8},{5,9},{5,10},{6,12},{6,13},{7,14},{7,15},{8,11},{8,12},{8,14},{9,13},{9,15}}

Cousin 1080: {{1,6},{1,9},{1,10},{1,11},{2,4},{2,5},{2,7},{2,9},{2,12},{3,10},{3,13},{3,14},{4,6},{4,7},{4,9},{4,11},{5,8},{5,10},{5,15},{6,12},{6,13},{7,14},{7,15},{8,11},{8,12},{8,14},{9,13},{9,15}}

Cousin 1081: {{1,6},{1,9},{1,10},{1,11},{2,4},{2,5},{2,7},{2,9},{2,12},{3,7},{3,8},{3,10},{3,13},{4,6},{4,7},{4,9},{4,11},{5,7},{5,8},{5,9},{5,10},{6,12},{6,13},{7,9},{8,11},{8,12},{9,13},{10,13}}

Cousin 1082: {{1,6},{1,9},{1,10},{1,11},{2,4},{2,5},{2,7},{2,9},{2,12},{3,7},{3,8},{3,10},{3,13},{4,6},{4,11},{4,14},{5,9},{5,10},{5,15},{6,12},{6,13},{7,14},{7,15},{8,11},{8,12},{8,15},{9,13},{9,14}}

Cousin 1083: {{1,6},{1,9},{1,10},{1,11},{2,4},{2,5},{2,7},{2,9},{2,12},{3,6},{3,9},{3,10},{3,13},{4,7},{4,11},{4,14},{5,8},{5,10},{5,15},{6,12},{6,14},{7,13},{7,15},{8,11},{8,12},{8,13},{9,14},{9,15}}

Cousin 1084: {{1,6},{1,9},{1,10},{1,11},{2,4},{2,5},{2,7},{2,9},{2,12},{3,6},{3,8},{3,10},{3,13},{4,7},{4,11},{4,14},{5,9},{5,10},{5,15},{6,12},{6,14},{7,13},{7,15},{8,11},{8,12},{8,15},{9,13},{9,14}}

Cousin 1085: {{1,6},{1,9},{1,10},{1,11},{2,4},{2,5},{2,12},{2,13},{3,10},{3,14},{3,15},{4,6},{4,7},{4,9},{4,11},{5,7},{5,8},{5,9},{5,10},{6,12},{6,14},{7,13},{7,15},{8,11},{8,13},{8,14},{9,12},{9,15}}

Cousin 1086: {{1,6},{1,9},{1,10},{1,11},{2,4},{2,5},{2,12},{2,13},{3,7},{3,9},{3,10},{3,14},{4,6},{4,11},{4,15},{5,7},{5,8},{5,9},{5,10},{6,12},{6,14},{7,13},{7,15},{8,11},{8,13},{8,14},{9,12},{9,15}}

Cousin 1087: {{1,6},{1,9},{1,10},{1,11},{2,4},{2,5},{2,12},{2,13},{3,7},{3,9},{3,10},{3,14},{4,6},{4,7},{4,9},{4,11},{5,8},{5,10},{5,15},{6,12},{6,14},{7,13},{7,15},{8,11},{8,13},{8,14},{9,12},{9,15}}



Cousin 1088: {{1,6},{1,9},{1,10},{1,11},{2,4},{2,5},{2,7},{2,8},{2,12},{3,10},{3,13},{3,14},{4,6},{4,7},{4,9},{4,11},{5,9},{5,10},{5,15},{6,12},{6,13},{7,14},{7,15},{8,11},{8,13},{8,15},{9,12},{9,14}}}

Cousin 1089: {{1,6},{1,9},{1,10},{1,11},{2,4},{2,5},{2,7},{2,8},{2,12},{3,7},{3,9},{3,10},{3,13},{4,6},{4,7},{4,9},{4,11},{5,7},{5,8},{5,9},{5,10},{6,12},{6,13},{7,8},{8,11},{8,13},{9,12},{10,13}}}

Cousin 1090: {{1,6},{1,9},{1,10},{1,11},{2,4},{2,5},{2,7},{2,8},{2,12},{3,7},{3,9},{3,10},{3,13},{4,6},{4,11},{4,14},{5,9},{5,10},{5,15},{6,12},{6,13},{7,14},{7,15},{8,11},{8,13},{8,15},{9,12},{9,14}}}

Cousin 1091: {{1,6},{1,9},{1,10},{1,11},{2,4},{2,5},{2,6},{2,9},{2,12},{3,10},{3,13},{3,14},{4,7},{4,11},{4,15},{5,7},{5,8},{5,9},{5,10},{6,13},{6,15},{7,12},{7,14},{8,11},{8,12},{8,13},{9,14},{9,15}}}

Cousin 1092: {{1,6},{1,9},{1,10},{1,11},{2,4},{2,5},{2,6},{2,9},{2,12},{3,7},{3,9},{3,10},{3,13},{4,6},{4,7},{4,9},{4,11},{5,7},{5,8},{5,9},{5,10},{6,9},{6,13},{7,12},{8,11},{8,12},{8,13},{10,13}}}

Cousin 1093: {{1,6},{1,9},{1,10},{1,11},{2,4},{2,5},{2,6},{2,9},{2,12},{3,7},{3,9},{3,10},{3,13},{4,7},{4,11},{4,14},{5,8},{5,10},{5,15},{6,13},{6,14},{7,12},{7,15},{8,11},{8,12},{8,13},{9,14},{9,15}}}

Cousin 1094: {{1,6},{1,9},{1,10},{1,11},{2,4},{2,5},{2,6},{2,8},{2,12},{3,7},{3,9},{3,10},{3,13},{4,7},{4,11},{4,14},{5,9},{5,10},{5,15},{6,13},{6,14},{7,12},{7,15},{8,11},{8,13},{8,15},{9,12},{9,14}}}

Cousin 1095: {{1,6},{1,9},{1,10},{1,11},{2,4},{2,5},{2,6},{2,8},{2,12},{3,7},{3,8},{3,10},{3,13},{4,6},{4,7},{4,9},{4,11},{5,7},{5,8},{5,9},{5,10},{6,8},{6,13},{7,12},{8,11},{9,12},{9,13},{10,13}}}

Cousin 1096: {{1,6},{1,9},{1,10},{1,11},{2,4},{2,5},{2,6},{2,7},{2,8},{2,9},{3,10},{3,12},{3,13},{4,7},{4,11},{4,14},{5,9},{5,10},{5,15},{6,12},{6,14},{7,13},{7,15},{8,11},{8,12},{8,15},{9,13},{9,14}}}

Cousin 1097: {{1,6},{1,9},{1,10},{1,11},{2,4},{2,5},{2,6},{2,7},{2,8},{2,9},{3,4},{3,6},{3,9},{4,7},{4,11},{5,7},{5,8},{5,9},{5,10},{6,12},{7,8},{7,13},{8,11},{8,12},{9,13},{10,12},{10,13},{12,13}}}

Cousin 1098: {{1,6},{1,9},{1,10},{1,11},{2,4},{2,5},{2,6},{2,7},{2,8},{2,9},{3,5},{3,7},{3,8},{4,6},{4,7},{4,9},{4,11},{5,9},{5,10},{6,9},{6,12},{7,13},{8,11},{8,12},{9,13},{10,12},{10,13},{12,13}}}

Cousin 1099: {{1,6},{1,9},{1,10},{1,11},{2,4},{2,5},{2,6},{2,7},{2,8},{2,9},{3,4},{3,7},{3,9},{4,6},{4,11},{5,7},{5,8},{5,9},{5,10},{6,8},{6,12},{7,13},{8,11},{8,13},{9,12},{10,12},{10,13},{12,13}}}

Cousin 1100: {{1,6},{1,9},{1,10},{1,11},{2,4},{2,5},{2,6},{2,7},{2,8},{2,9},{3,5},{3,7},{3,9},{4,6},{4,7},{4,9},{4,11},{5,8},{5,10},{6,8},{6,12},{7,13},{8,11},{8,13},{9,12},{10,12},{10,13},{12,13}}}

Cousin 1101: {{1,4},{1,9},{1,10},{1,11},{2,5},{2,7},{2,12},{2,13},{3,6},{3,9},{3,10},{3,14},{4,6},{4,12},{4,15},{5,7},{5,8},{5,9},{5,10},{6,11},{6,13},{7,14},{7,15},{8,11},{8,12},{8,14},{9,13},{9,15}}}

Cousin 1102: {{1,4},{1,9},{1,10},{1,11},{2,5},{2,7},{2,12},{2,13},{3,6},{3,9},{3,10},{3,14},{4,6},{4,7},{4,9},{4,12},{5,8},{5,10},{5,15},{6,11},{6,13},{7,14},{7,15},{8,11},{8,12},{8,14},{9,13},{9,15}}}

Cousin 1103: {{1,4},{1,9},{1,10},{1,11},{2,5},{2,7},{2,12},{2,13},{3,6},{3,8},{3,10},{3,14},{4,6},{4,7},{4,9},{4,12},{5,9},{5,10},{5,15},{6,11},{6,13},{7,14},{7,15},{8,11},{8,12},{8,15},{9,13},{9,14}}}

Cousin 1104: {{1,4},{1,9},{1,10},{1,11},{2,5},{2,7},{2,12},{2,13},{3,6},{3,7},{3,8},{3,9},{3,10},{4,6},{4,12},{4,14},{5,9},{5,10},{5,15},{6,11},{6,13},{7,14},{7,15},{8,11},{8,12},{8,15},{9,13},{9,14}}}

Cousin 1105: {{1,4},{1,9},{1,10},{1,11},{2,5},{2,6},{2,12},{2,13},{3,10},{3,14},{3,15},{4,6},{4,7},{4,9},{4,12},{5,7},{5,8},{5,9},{5,10},{6,11},{6,14},{7,13},{7,15},{8,11},{8,12},{8,15},{9,13},{9,14}}}

Cousin 1106: {{1,4},{1,9},{1,10},{1,11},{2,5},{2,6},{2,12},{2,13},{3,7},{3,8},{3,10},{3,14},{4,6},{4,7},{4,9},{4,12},{5,9},{5,10},{5,15},{6,11},{6,14},{7,13},{7,15},{8,11},{8,12},{8,15},{9,13},{9,14}}}

Cousin 1107: {{1,4},{1,9},{1,10},{1,11},{2,5},{2,6},{2,12},{2,13},{3,6},{3,9},{3,10},{3,14},{4,7},{4,12},{4,15},{5,7},{5,8},{5,9},{5,10},{6,11},{6,15},{7,13},{7,14},{8,11},{8,12},{8,14},{9,13},{9,15}}}

Cousin 1108: {{1,4},{1,9},{1,10},{1,11},{2,5},{2,6},{2,12},{2,13},{3,6},{3,7},{3,8},{3,9},{3,10},{4,7},{4,12},{4,14},{5,9},{5,10},{5,15},{6,11},{6,14},{7,13},{7,15},{8,11},{8,12},{8,15},{9,13},{9,14}}}

Cousin 1109: {{1,4},{1,9},{1,10},{1,11},{2,5},{2,6},{2,7},{2,9},{2,12},{3,10},{3,13},{3,14},{4,6},{4,12},{4,15},{5,7},{5,8},{5,9},{5,10},{6,11},{6,13},{7,14},{7,15},{8,11},{8,12},{8,14},{9,13},{9,15}}}

Cousin 1110: {{1,4},{1,9},{1,10},{1,11},{2,5},{2,6},{2,7},{2,9},{2,12},{3,10},{3,13},{3,14},{4,6},{4,7},{4,9},{4,12},{5,8},{5,10},{5,15},{6,11},{6,13},{7,14},{7,15},{8,11},{8,12},{8,14},{9,13},{9,15}}}

Cousin 1111: {{1,4},{1,9},{1,10},{1,11},{2,5},{2,6},{2,7},{2,9},{2,12},{3,7},{3,8},{3,10},{3,13},{4,6},{4,7},{4,9},{4,12},{5,7},{5,8},{5,9},{5,10},{6,11},{6,13},{7,9},{8,11},{8,12},{9,13},{10,13}}}

Cousin 1112: {{1,4},{1,9},{1,10},{1,11},{2,5},{2,6},{2,7},{2,9},{2,12},{3,6},{3,9},{3,10},{3,13},{4,7},{4,12},{4,14},{5,8},{5,10},{5,15},{6,11},{6,14},{7,13},{7,15},{8,11},{8,12},{8,13},{9,14},{9,15}}}

Cousin 1113: {{1,4},{1,9},{1,10},{1,11},{2,5},{2,6},{2,7},{2,8},{2,12},{3,7},{3,8},{3,10},{3,13},{4,6},{4,7},{4,8},{4,12},{5,7},{5,8},{5,9},{5,10},{6,11},{6,13},{7,9},{8,11},{9,12},{9,13},{10,13}}

Cousin 1114: {{1,4},{1,9},{1,10},{1,11},{2,4},{2,5},{2,6},{2,8},{2,12},{3,7},{3,8},{3,10},{3,13},{4,6},{4,7},{4,8},{4,9},{5,7},{5,8},{5,9},{5,10},{6,11},{6,13},{7,12},{8,11},{9,12},{9,13},{10,13}}

Cousin 1115: {{1,4},{1,9},{1,10},{1,11},{2,4},{2,5},{2,6},{2,7},{2,8},{2,9},{3,4},{3,7},{3,9},{4,6},{4,8},{5,7},{5,8},{5,9},{5,10},{6,11},{6,12},{7,13},{8,11},{8,13},{9,12},{10,12},{10,13},{12,13}}

Cousin 1116: {{1,4},{1,9},{1,10},{1,11},{2,4},{2,5},{2,6},{2,7},{2,8},{2,9},{3,5},{3,7},{3,9},{4,6},{4,7},{4,8},{4,9},{5,8},{5,10},{6,11},{6,12},{7,13},{8,11},{8,13},{9,12},{10,12},{10,13},{12,13}}

Cousin 1117: {{1,4},{1,6},{1,8},{1,9},{1,10},{2,5},{2,7},{2,11},{2,12},{3,7},{3,9},{3,10},{3,13},{4,6},{4,7},{4,9},{4,11},{5,7},{5,8},{5,9},{5,10},{6,12},{6,13},{7,8},{8,11},{8,13},{9,12},{10,13}}

Cousin 1118: {{1,4},{1,6},{1,8},{1,9},{1,10},{2,5},{2,6},{2,11},{2,12},{3,7},{3,8},{3,10},{3,13},{4,6},{4,7},{4,9},{4,11},{5,7},{5,8},{5,9},{5,10},{6,8},{6,13},{7,12},{8,11},{9,12},{9,13},{10,13}}

Cousin 1119: {{1,4},{1,6},{1,8},{1,9},{1,10},{2,4},{2,5},{2,11},{2,12},{3,7},{3,8},{3,10},{3,13},{4,6},{4,7},{4,8},{4,9},{5,7},{5,8},{5,9},{5,10},{6,11},{6,13},{7,12},{8,11},{9,12},{9,13},{10,13}}

Cousin 1120: {{1,4},{1,6},{1,8},{1,9},{1,10},{2,4},{2,5},{2,7},{2,9},{2,11},{3,4},{3,7},{3,9},{4,6},{4,8},{5,7},{5,8},{5,9},{5,10},{6,11},{6,12},{7,13},{8,11},{8,13},{9,12},{10,12},{10,13},{12,13}}

Cousin 1121: {{1,4},{1,6},{1,8},{1,9},{1,10},{2,4},{2,5},{2,6},{2,9},{2,11},{3,4},{3,6},{3,9},{4,7},{4,8},{5,7},{5,8},{5,9},{5,10},{6,12},{7,11},{7,13},{8,11},{8,12},{9,13},{10,12},{10,13},{12,13}}

Cousin 1122: {{1,5},{1,6},{1,10},{1,11},{2,6},{2,7},{2,12},{2,13},{3,5},{3,7},{3,10},{3,14},{4,6},{4,7},{4,11},{4,12},{5,13},{5,15},{6,8},{6,14},{7,9},{7,15},{8,10},{8,12},{8,15},{9,11},{9,13},{9,14}}

Cousin 1123: {{1,5},{1,6},{1,10},{1,11},{2,6},{2,7},{2,12},{2,13},{3,5},{3,6},{3,10},{3,14},{4,6},{4,7},{4,11},{4,12},{5,13},{5,15},{6,8},{6,9},{7,14},{7,15},{8,10},{8,12},{8,15},{9,11},{9,13},{9,14}}

Cousin 1124: {{1,5},{1,6},{1,10},{1,11},{2,5},{2,7},{2,12},{2,13},{3,6},{3,7},{3,10},{3,14},{4,6},{4,7},{4,11},{4,12},{5,14},{5,15},{6,8},{6,13},{7,9},{7,15},{8,10},{8,12},{8,15},{9,11},{9,13},{9,14}}

Cousin 1125: {{1,5},{1,6},{1,10},{1,11},{2,5},{2,6},{2,12},{2,13},{3,6},{3,7},{3,10},{3,14},{4,6},{4,7},{4,11},{4,12},{5,14},{5,15},{6,8},{6,9},{7,13},{7,15},{8,10},{8,12},{8,15},{9,11},{9,13},{9,14}}

Cousin 1126: {{1,5},{1,6},{1,10},{1,11},{2,4},{2,7},{2,12},{2,13},{3,6},{3,7},{3,10},{3,14},{4,7},{4,11},{4,15},{5,7},{5,12},{5,14},{6,13},{6,15},{7,8},{7,9},{8,10},{8,12},{8,15},{9,11},{9,13},{9,14}}

Cousin 1127: {{1,5},{1,6},{1,10},{1,11},{2,4},{2,7},{2,12},{2,13},{3,6},{3,7},{3,10},{3,14},{4,6},{4,11},{4,15},{5,7},{5,12},{5,14},{6,8},{6,13},{7,9},{7,15},{8,10},{8,12},{8,15},{9,11},{9,13},{9,14}}

Cousin 1128: {{1,5},{1,6},{1,10},{1,11},{2,4},{2,7},{2,12},{2,13},{3,5},{3,6},{3,10},{3,14},{4,7},{4,11},{4,15},{5,7},{5,9},{5,12},{6,13},{6,15},{7,8},{7,14},{8,10},{8,12},{8,15},{9,11},{9,13},{9,14}}

Cousin 1129: {{1,5},{1,6},{1,10},{1,11},{2,4},{2,7},{2,12},{2,13},{3,5},{3,6},{3,10},{3,14},{4,6},{4,11},{4,15},{5,7},{5,9},{5,12},{6,8},{6,13},{7,14},{7,15},{8,10},{8,12},{8,15},{9,11},{9,13},{9,14}}

Cousin 1130: {{1,5},{1,6},{1,10},{1,11},{2,4},{2,7},{2,12},{2,13},{3,5},{3,6},{3,7},{3,9},{3,10},{4,7},{4,11},{4,14},{5,12},{5,15},{6,13},{6,14},{7,8},{7,15},{8,10},{8,12},{8,14},{9,11},{9,13},{9,15}}

Cousin 1131: {{1,5},{1,6},{1,10},{1,11},{2,4},{2,7},{2,12},{2,13},{3,5},{3,6},{3,7},{3,9},{3,10},{4,6},{4,11},{4,14},{5,12},{5,15},{6,8},{6,13},{7,14},{7,15},{8,10},{8,12},{8,14},{9,11},{9,13},{9,15}}

Cousin 1132: {{1,5},{1,6},{1,10},{1,11},{2,4},{2,6},{2,12},{2,13},{3,6},{3,7},{3,10},{3,14},{4,7},{4,11},{4,15},{5,7},{5,12},{5,14},{6,9},{6,15},{7,8},{7,13},{8,10},{8,12},{8,15},{9,11},{9,13},{9,14}}

Cousin 1133: {{1,5},{1,6},{1,10},{1,11},{2,4},{2,6},{2,12},{2,13},{3,5},{3,7},{3,10},{3,14},{4,7},{4,11},{4,15},{5,7},{5,9},{5,12},{6,14},{6,15},{7,8},{7,13},{8,10},{8,12},{8,15},{9,11},{9,13},{9,14}}

Cousin 1134: {{1,5},{1,6},{1,10},{1,11},{2,4},{2,6},{2,12},{2,13},{3,5},{3,7},{3,10},{3,14},{4,6},{4,11},{4,15},{5,7},{5,9},{5,12},{6,8},{6,14},{7,13},{7,15},{8,10},{8,12},{8,15},{9,11},{9,13},{9,14}}

Cousin 1135: {{1,5},{1,6},{1,10},{1,11},{2,4},{2,6},{2,7},{2,9},{2,12},{3,5},{3,7},{3,10},{3,13},{4,6},{4,11},{4,14},{5,12},{5,15},{6,8},{6,13},{7,14},{7,15},{8,10},{8,12},{8,14},{9,11},{9,13},{9,15}}

Cousin 1136: {{1,5},{1,6},{1,10},{1,11},{2,4},{2,7},{2,12},{2,13},{3,5},{3,7},{3,10},{3,14},{4,6},{4,11},{4,15},{5,7},{5,8},{5,12},{6,13},{6,14},{7,9},{7,15},{8,10},{8,13},{8,15},{9,11},{9,12},{9,14}}

Cousin 1137: {{1,5},{1,6},{1,10},{1,11},{2,4},{2,7},{2,12},{2,13},{3,5},{3,7},{3,10},{3,14},{4,6},{4,7},{4,8},{4,11},{5,12},{5,15},{6,13},{6,14},{7,9},{7,15},{8,10},{8,13},{8,15},{9,11},{9,12},{9,14}}

Cousin 1138: {{1,5},{1,6},{1,10},{1,11},{2,4},{2,6},{2,12},{2,13},{3,5},{3,7},{3,10},{3,14},{4,7},{4,11},{4,15},{5,7},{5,8},{5,12},{6,14},{6,15},{7,9},{7,13},{8,10},{8,12},{8,15},{9,11},{9,13},{9,14}}

{8,13},{8,15},{9,11},{9,12},{9,14}}

Cousin 1139: {{1,5},{1,6},{1,10},{1,11},{2,4},{2,6},{2,7},{2,8},{2,12},{3,5},{3,6},{3,10},{3,13},{4,7},{4,11},{4,14},{5,12},{5,15},{6,9},{6,14},{7,13},{7,15},{8,10},{8,14},{8,15},{9,11},{9,12},{9,13}}

Cousin 1140: {{1,5},{1,6},{1,10},{1,11},{2,4},{2,5},{2,12},{2,13},{3,6},{3,7},{3,10},{3,14},{4,6},{4,11},{4,15},{5,7},{5,8},{5,14},{6,9},{6,12},{7,13},{7,15},{8,10},{8,12},{8,15},{9,11},{9,13},{9,14}}

Cousin 1141: {{1,5},{1,6},{1,10},{1,11},{2,4},{2,5},{2,12},{2,13},{3,6},{3,7},{3,10},{3,14},{4,6},{4,7},{4,8},{4,11},{5,14},{5,15},{6,9},{6,12},{7,13},{7,15},{8,10},{8,12},{8,15},{9,11},{9,13},{9,14}}

Cousin 1142: {{1,5},{1,6},{1,10},{1,11},{2,4},{2,5},{2,12},{2,13},{3,5},{3,7},{3,10},{3,14},{4,6},{4,11},{4,15},{5,7},{5,8},{5,9},{6,12},{6,14},{7,13},{7,15},{8,10},{8,12},{8,15},{9,11},{9,13},{9,14}}

Cousin 1143: {{1,5},{1,6},{1,10},{1,11},{2,4},{2,5},{2,12},{2,13},{3,6},{3,7},{3,10},{3,14},{4,7},{4,11},{4,15},{5,7},{5,8},{5,14},{6,12},{6,15},{7,9},{7,13},{8,10},{8,13},{8,15},{9,11},{9,12},{9,14}}

Cousin 1144: {{1,5},{1,6},{1,10},{1,11},{2,4},{2,5},{2,7},{2,8},{2,12},{3,6},{3,7},{3,10},{3,13},{4,7},{4,11},{4,14},{5,13},{5,15},{6,12},{6,14},{7,9},{7,15},{8,10},{8,14},{8,15},{9,11},{9,12},{9,13}}

Cousin 1145: {{1,5},{1,6},{1,10},{1,11},{2,4},{2,5},{2,6},{2,9},{2,12},{3,5},{3,7},{3,10},{3,13},{4,7},{4,11},{4,14},{5,8},{5,15},{6,13},{6,14},{7,12},{7,15},{8,10},{8,12},{8,14},{9,11},{9,13},{9,15}}

Cousin 1146: {{1,5},{1,6},{1,10},{1,11},{2,4},{2,5},{2,6},{2,8},{2,12},{3,6},{3,7},{3,10},{3,13},{4,7},{4,11},{4,14},{5,13},{5,15},{6,9},{6,14},{7,12},{7,15},{8,10},{8,14},{8,15},{9,11},{9,12},{9,13}}

Cousin 1147: {{1,4},{1,6},{1,10},{1,11},{2,5},{2,7},{2,12},{2,13},{3,5},{3,7},{3,10},{3,14},{4,6},{4,12},{4,15},{5,7},{5,8},{5,11},{6,13},{6,14},{7,9},{7,15},{8,10},{8,13},{8,15},{9,11},{9,12},{9,14}}

Cousin 1148: {{1,4},{1,5},{1,10},{1,11},{2,5},{2,6},{2,12},{2,13},{3,6},{3,7},{3,10},{3,14},{4,6},{4,7},{4,9},{4,12},{5,14},{5,15},{6,8},{6,11},{7,13},{7,15},{8,10},{8,12},{8,15},{9,11},{9,13},{9,14}}

Cousin 1149: {{1,3},{1,6},{1,10},{1,11},{2,4},{2,7},{2,12},{2,13},{3,5},{3,14},{3,15},{4,6},{4,7},{4,9},{4,10},{5,7},{5,11},{5,12},{6,13},{6,14},{7,8},{7,15},{8,10},{8,12},{8,14},{9,11},{9,13},{9,15}}

Cousin 1150: {{1,8},{1,9},{1,10},{1,11},{2,12},{2,13},{2,14},{3,10},{3,15},{3,16},{4,8},{4,9},{4,11},{4,12},{5,7},{5,9},{5,10},{5,13},{6,11},{6,14},{6,15},{7,8},{7,12},{7,16},{8,13},{8,15},{9,14},{9,16}}

Cousin 1151: {{1,8},{1,9},{1,10},{1,11},{2,12},{2,13},{2,14},{3,7},{3,9},{3,10},{3,15},{4,8},{4,9},{4,11},{4,12},{5,10},{5,13},{5,16},{6,11},{6,14},{6,15},{7,8},{7,12},{7,16},{8,13},{8,15},{9,14},{9,16}}

Cousin 1152: {{1,8},{1,9},{1,10},{1,11},{2,3},{2,6},{2,8},{3,7},{3,9},{3,10},{4,8},{4,9},{4,11},{4,12},{5,7},{5,9},{5,10},{5,13},{6,11},{6,14},{7,8},{7,9},{7,12},{8,13},{9,14},{12,13},{12,14},{13,14}}

Cousin 1153: {{1,8},{1,9},{1,10},{1,11},{2,12},{2,13},{2,14},{3,6},{3,7},{3,9},{3,10},{4,8},{4,9},{4,11},{4,12},{5,7},{5,9},{5,10},{5,13},{6,8},{6,11},{6,14},{7,8},{7,9},{7,12},{8,13},{9,14},{11,14}}

Cousin 1154: {{1,8},{1,9},{1,10},{1,11},{2,12},{2,13},{2,14},{3,6},{3,9},{3,10},{3,15},{4,8},{4,9},{4,11},{4,12},{5,10},{5,13},{5,16},{6,8},{6,11},{6,14},{7,12},{7,15},{7,16},{8,13},{8,15},{9,14},{9,16}}

Cousin 1155: {{1,8},{1,9},{1,10},{1,11},{2,3},{2,7},{2,8},{3,6},{3,9},{3,10},{4,8},{4,9},{4,11},{4,12},{5,7},{5,9},{5,10},{5,13},{6,8},{6,11},{6,14},{7,9},{7,12},{8,13},{9,14},{12,13},{12,14},{13,14}}

Cousin 1156: {{1,8},{1,9},{1,10},{1,11},{2,3},{2,7},{2,9},{3,6},{3,8},{3,10},{4,8},{4,9},{4,11},{4,12},{5,7},{5,9},{5,10},{5,13},{6,8},{6,11},{6,14},{7,8},{7,12},{8,13},{9,14},{12,13},{12,14},{13,14}}

Cousin 1157: {{1,8},{1,9},{1,10},{1,11},{2,5},{2,7},{2,9},{3,6},{3,7},{3,8},{3,9},{3,10},{4,8},{4,9},{4,11},{4,12},{5,10},{5,13},{6,8},{6,11},{6,14},{7,8},{7,12},{8,13},{9,14},{12,13},{12,14},{13,14}}

Cousin 1158: {{1,8},{1,9},{1,10},{1,11},{2,12},{2,13},{2,14},{3,6},{3,7},{3,8},{3,9},{3,10},{4,8},{4,9},{4,11},{4,12},{5,7},{5,9},{5,10},{5,13},{6,8},{6,11},{6,14},{7,8},{7,12},{8,13},{9,14},{10,13}}

Cousin 1159: {{1,8},{1,9},{1,10},{1,11},{2,6},{2,9},{2,12},{2,13},{3,7},{3,9},{3,10},{3,14},{4,8},{4,9},{4,11},{4,12},{5,7},{5,9},{5,10},{5,13},{6,9},{6,11},{6,14},{7,8},{7,12},{8,13},{8,14},{10,13}}

Cousin 1160: {{1,8},{1,9},{1,10},{1,11},{2,6},{2,9},{2,12},{2,13},{3,7},{3,8},{3,10},{3,14},{4,8},{4,9},{4,11},{4,12},{5,7},{5,9},{5,10},{5,13},{6,8},{6,11},{6,14},{7,8},{7,12},{8,13},{9,14},{10,13}}

Cousin 1161: {{1,8},{1,9},{1,10},{1,11},{2,6},{2,9},{2,12},{2,13},{3,6},{3,9},{3,10},{3,14},{4,8},{4,9},{4,11},{4,12},{5,7},{5,9},{5,10},{5,13},{6,8},{6,9},{6,11},{7,12},{7,14},{8,13},{8,14},{10,13}}

Cousin 1162: {{1,8},{1,9},{1,10},{1,11},{2,5},{2,9},{2,12},{2,13},{3,7},{3,8},{3,10},{3,14},{4,8},{4,9},{4,11},{4,12},{5,6},{5,9},{5,10},{6,7},{6,8},{7,9},{7,12},{8,13},{9,14},{11,13},{11,14},{13,14}}

Cousin 1163: {{1,8},{1,9},{1,10},{1,11},{2,6},{2,7},{2,12},{2,13},{3,10},{3,14},{3,15},{4,7},{4,9},{4,11},{4,12},{5,10},{5,13},{5,16},{6,9},{6,11},{6,14},{7,15},{7,16},{8,12},{8,14},{8,16},{9,13},{9,15}}

Cousin 1164: {{1,8},{1,9},{1,10},{1,11},{2,6},{2,7},{2,12},{2,13},{3,7},{3,9},{3,10},{3,14},{4,7},{4,9},{4,11},{4,12},{5,7},{5,8},{5,10},{5,13},{6,9},{6,11},{6,14},{7,8},{8,12},{8,14},{9,13},{10,14}}

Cousin 1165: {{1,8},{1,9},{1,10},{1,11},{2,6},{2,7},{2,12},{2,13},{3,7},{3,9},{3,10},{3,14},{4,11},{4,12},{4,15},{5,10},{5,13},{5,16},{6,9},{6,11},{6,14},{7,15},{7,16},{8,12},{8,14},{8,16},{9,13},{9,15}}

Cousin 1166: {{1,8},{1,9},{1,10},{1,11},{2,6},{2,7},{2,12},{2,13},{3,7},{3,9},{3,10},{3,14},{4,7},{4,9},{4,11},{4,12},{5,7},{5,8},{5,10},{5,13},{6,9},{6,11},{6,14},{7,8},{8,12},{8,14},{9,13},{11,12}}

Cousin 1167: {{1,8},{1,9},{1,10},{1,11},{2,6},{2,7},{2,12},{2,13},{3,7},{3,9},{3,10},{3,14},{4,7},{4,9},{4,11},{4,12},{5,7},{5,8},{5,10},{5,13},{6,9},{6,11},{6,14},{7,9},{8,12},{8,14},{9,13},{10,13}}

Cousin 1168: {{1,8},{1,9},{1,10},{1,11},{2,6},{2,7},{2,12},{2,13},{3,10},{3,14},{3,15},{4,11},{4,12},{4,16},{5,7},{5,8},{5,10},{5,13},{6,8},{6,11},{6,14},{7,15},{7,16},{8,12},{8,15},{9,13},{9,14},{9,16}}

Cousin 1169: {{1,8},{1,9},{1,10},{1,11},{2,6},{2,7},{2,12},{2,13},{3,7},{3,8},{3,10},{3,14},{4,7},{4,9},{4,11},{4,12},{5,7},{5,8},{5,10},{5,13},{6,8},{6,11},{6,14},{7,9},{8,12},{9,13},{9,14},{10,14}}

Cousin 1170: {{1,8},{1,9},{1,10},{1,11},{2,6},{2,7},{2,12},{2,13},{3,7},{3,8},{3,10},{3,14},{4,11},{4,12},{4,15},{5,10},{5,13},{5,16},{6,8},{6,11},{6,14},{7,15},{7,16},{8,12},{8,16},{9,13},{9,14},{9,15}}

Cousin 1171: {{1,8},{1,9},{1,10},{1,11},{2,6},{2,7},{2,12},{2,13},{3,7},{3,8},{3,10},{3,14},{4,7},{4,9},{4,11},{4,12},{5,7},{5,8},{5,10},{5,13},{6,8},{6,11},{6,14},{7,8},{8,12},{9,13},{9,14},{11,12}}

Cousin 1172: {{1,8},{1,9},{1,10},{1,11},{2,6},{2,7},{2,12},{2,13},{3,7},{3,8},{3,10},{3,14},{4,7},{4,9},{4,11},{4,12},{5,7},{5,8},{5,10},{5,13},{6,8},{6,11},{6,14},{7,9},{8,12},{9,13},{9,14},{10,13}}

Cousin 1173: {{1,8},{1,9},{1,10},{1,11},{2,6},{2,7},{2,12},{2,13},{3,6},{3,9},{3,10},{3,14},{4,7},{4,9},{4,11},{4,12},{5,7},{5,8},{5,10},{5,13},{6,8},{6,9},{6,11},{7,14},{8,12},{8,14},{9,13},{11,12}}

Cousin 1174: {{1,8},{1,9},{1,10},{1,11},{2,6},{2,7},{2,12},{2,13},{3,6},{3,8},{3,10},{3,14},{4,7},{4,9},{4,11},{4,12},{5,7},{5,8},{5,10},{5,13},{6,8},{6,9},{6,11},{7,14},{8,12},{9,13},{9,14},{10,13}}

Cousin 1175: {{1,8},{1,9},{1,10},{1,11},{2,6},{2,7},{2,12},{2,13},{3,6},{3,7},{3,8},{3,9},{3,10},{4,5},{4,7},{4,8},{5,10},{5,13},{6,8},{6,9},{6,11},{7,14},{8,12},{9,13},{9,14},{11,12},{11,14},{12,14}}

Cousin 1176: {{1,8},{1,9},{1,10},{1,11},{2,5},{2,7},{2,12},{2,13},{3,10},{3,14},{3,15},{4,7},{4,9},{4,11},{4,12},{5,9},{5,10},{5,16},{6,11},{6,13},{6,14},{7,15},{7,16},{8,12},{8,14},{8,16},{9,13},{9,15}}

Cousin 1177: {{1,8},{1,9},{1,10},{1,11},{2,5},{2,7},{2,12},{2,13},{3,7},{3,9},{3,10},{3,14},{4,7},{4,9},{4,11},{4,12},{5,7},{5,8},{5,9},{5,10},{6,11},{6,13},{6,14},{7,8},{8,12},{8,14},{9,13},{10,14}}

Cousin 1178: {{1,8},{1,9},{1,10},{1,11},{2,5},{2,7},{2,12},{2,13},{3,6},{3,10},{3,14},{4,7},{4,9},{4,11},{4,12},{5,7},{5,8},{5,9},{5,10},{6,7},{6,9},{7,8},{8,12},{8,14},{9,13},{11,13},{11,14},{13,14}}

Cousin 1179: {{1,8},{1,9},{1,10},{1,11},{2,5},{2,7},{2,12},{2,13},{3,7},{3,9},{3,10},{3,14},{4,7},{4,9},{4,11},{4,12},{5,7},{5,8},{5,9},{5,10},{6,11},{6,13},{6,14},{7,8},{8,12},{8,14},{9,13},{11,12}}

Cousin 1180: {{1,8},{1,9},{1,10},{1,11},{2,5},{2,7},{2,12},{2,13},{3,7},{3,9},{3,10},{3,14},{4,6},{4,11},{4,12},{5,7},{5,8},{5,9},{5,10},{6,7},{6,9},{7,8},{8,12},{8,14},{9,13},{11,13},{11,14},{13,14}}

Cousin 1181: {{1,8},{1,9},{1,10},{1,11},{2,5},{2,7},{2,12},{2,13},{3,7},{3,9},{3,10},{3,14},{4,7},{4,9},{4,11},{4,12},{5,6},{5,9},{5,10},{6,7},{6,8},{7,9},{8,12},{8,14},{9,13},{11,13},{11,14},{13,14}}

Cousin 1182: {{1,8},{1,9},{1,10},{1,11},{2,5},{2,7},{2,12},{2,13},{3,7},{3,9},{3,10},{3,14},{4,7},{4,9},{4,11},{4,12},{5,6},{5,8},{5,10},{6,7},{6,9},{7,8},{8,12},{8,14},{9,13},{11,13},{11,14},{13,14}}

Cousin 1183: {{1,8},{1,9},{1,10},{1,11},{2,5},{2,7},{2,12},{2,13},{3,6},{3,9},{3,10},{3,14},{4,7},{4,9},{4,11},{4,12},{5,7},{5,8},{5,9},{5,10},{6,8},{6,11},{6,13},{7,14},{8,12},{8,14},{9,13},{11,12}}

Cousin 1184: {{1,8},{1,9},{1,10},{1,11},{2,5},{2,6},{2,12},{2,13},{3,7},{3,8},{3,10},{3,14},{4,7},{4,9},{4,11},{4,12},{5,7},{5,8},{5,9},{5,10},{6,8},{6,11},{6,14},{7,13},{8,12},{9,13},{9,14},{10,14}}

Cousin 1185: {{1,8},{1,9},{1,10},{1,11},{2,5},{2,6},{2,7},{2,9},{2,12},{3,4},{3,7},{3,9},{4,11},{4,12},{5,7},{5,8},{5,9},{5,10},{6,8},{6,11},{6,13},{7,14},{8,12},{8,14},{9,13},{10,13},{10,14},{13,14}}

Cousin 1186: {{1,8},{1,9},{1,10},{1,11},{2,5},{2,6},{2,7},{2,9},{2,12},{3,10},{3,13},{3,14},{4,7},{4,9},{4,11},{4,12},{5,7},{5,8},{5,9},{5,10},{6,8},{6,11},{6,13},{7,14},{8,12},{8,14},{9,13},{11,12}}

Cousin 1187: {{1,8},{1,9},{1,10},{1,11},{2,4},{2,7},{2,12},{2,13},{3,10},{3,14},{3,15},{4,9},{4,11},{4,16},{5,7},{5,9},{5,10},{5,12},{6,11},{6,13},{6,14},{7,15},{7,16},{8,12},{8,14},{8,16},{9,13},{9,15}}

Cousin 1188: {{1,8},{1,9},{1,10},{1,11},{2,4},{2,7},{2,12},{2,13},{3,7},{3,9},{3,10},{3,14},{4,7},{4,8},{4,9},{4,11},{5,7},{5,9},{5,10},{5,12},{6,11},{6,13},{6,14},{7,8},{8,12},{8,14},{9,13},{10,14}}

Cousin 1189: {{1,8},{1,9},{1,10},{1,11},{2,4},{2,7},{2,12},{2,13},{3,6},{3,10},{3,14},{4,7},{4,8},{4,9},{4,11},{5,7},{5,9},{5,10},{5,12},{6,7},{6,9},{7,8},{8,12},{8,14},{9,13},{11,13},{11,14},{13,14}}

Cousin 1190: {{1,8},{1,9},{1,10},{1,11},{2,4},{2,7},{2,12},{2,13},{3,7},{3,9},{3,10},{3,14},{4,6},{4,9},{4,11},{5,7},{5,9},{5,10},{5,12},{6,7},{6,8},{7,9},{8,12},{8,14},{9,13},{11,13},{11,14},{13,14}}

Cousin 1191: {{1,8},{1,9},{1,10},{1,11},{2,4},{2,7},{2,12},{2,13},{3,7},{3,9},{3,10},{3,14},{4,6},{4,8},{4,11},{5,7},{5,9},{5,10},{5,12},{6,7},{6,9},{7,8},{8,12},{8,14},{9,13},{11,13},{11,14},{13,14}}

Cousin 1192: {{1,8},{1,9},{1,10},{1,11},{2,4},{2,6},{2,12},{2,13},{3,7},{3,8},{3,10},{3,14},{4,7},{4,8},{4,9},{4,11},{5,7},{5,9},{5,10},{5,12},{6,8},{6,11},{6,14},{7,13},{8,12},{9,13},{9,14},{10,14}}

Cousin 1193: {{1,8},{1,9},{1,10},{1,11},{2,4},{2,5},{2,12},{2,13},{3,7},{3,8},{3,10},{3,14},{4,7},{4,8},{4,9},{4,11},{5,7},{5,8},{5,9},{5,10},{6,11},{6,12},{6,14},{7,13},{8,12},{9,13},{9,14},{10,14}}

Cousin 1194: {{1,8},{1,9},{1,10},{1,11},{2,4},{2,5},{2,7},{2,9},{2,12},{3,6},{3,7},{3,8},{3,10},{4,7},{4,8},{4,9},{4,11},{5,7},{5,8},{5,9},{5,10},{6,9},{6,10},{6,11},{6,12},{7,9},{8,12},{11,12}}

Cousin 1195: {{1,10},{1,11},{1,12},{2,13},{2,14},{2,15},{3,7},{3,9},{3,10},{3,16},{4,7},{4,9},{4,11},{4,13},{5,7},{5,9},{5,10},{5,14},{6,12},{6,13},{6,16},{7,8},{7,15},{8,11},{8,14},{8,16},{9,12},{9,15}}

Cousin 1196: {{1,10},{1,11},{1,12},{2,13},{2,14},{2,15},{3,6},{3,9},{3,10},{3,16},{4,7},{4,9},{4,11},{4,13},{5,7},{5,9},{5,10},{5,14},{6,8},{6,12},{6,13},{7,15},{7,16},{8,11},{8,14},{8,16},{9,12},{9,15}}

Cousin 1197: {{1,2},{1,7},{1,9},{2,13},{2,14},{3,6},{3,7},{3,8},{3,9},{3,10},{4,7},{4,9},{4,11},{4,13},{5,7},{5,9},{5,10},{5,14},{6,8},{6,12},{6,13},{7,8},{8,11},{8,14},{9,12},{10,11},{10,12},{11,12}}

Cousin 1198: {{1,10},{1,11},{1,12},{2,7},{2,9},{2,13},{2,14},{3,6},{3,7},{3,8},{3,9},{3,10},{4,7},{4,9},{4,11},{4,13},{5,7},{5,9},{5,10},{5,14},{6,8},{6,12},{6,13},{7,8},{8,11},{8,14},{9,12},{13,14}}

Cousin 1199: {{1,10},{1,11},{1,12},{2,7},{2,9},{2,13},{2,14},{3,10},{3,15},{3,16},{4,7},{4,9},{4,11},{4,13},{5,7},{5,9},{5,10},{5,14},{6,12},{6,13},{6,15},{7,8},{7,16},{8,11},{8,14},{8,15},{9,12},{9,16}}

Cousin 1200: {{1,3},{1,6},{1,8},{2,7},{2,9},{2,13},{2,14},{3,7},{3,9},{3,10},{4,7},{4,9},{4,11},{4,13},{5,7},{5,9},{5,10},{5,14},{6,12},{6,13},{7,8},{7,9},{8,11},{8,14},{9,12},{10,11},{10,12},{11,12}}

Cousin 1201: {{1,10},{1,11},{1,12},{2,7},{2,9},{2,13},{2,14},{3,6},{3,9},{3,10},{3,15},{4,11},{4,13},{4,16},{5,7},{5,9},{5,10},{5,14},{6,8},{6,12},{6,13},{7,15},{7,16},{8,11},{8,14},{8,15},{9,12},{9,16}}

Cousin 1202: {{1,10},{1,11},{1,12},{2,7},{2,9},{2,13},{2,14},{3,6},{3,9},{3,10},{3,15},{4,7},{4,9},{4,11},{4,13},{5,10},{5,14},{5,16},{6,8},{6,12},{6,13},{7,15},{7,16},{8,11},{8,14},{8,15},{9,12},{9,16}}

Cousin 1203: {{1,3},{1,7},{1,8},{2,7},{2,9},{2,13},{2,14},{3,6},{3,9},{3,10},{4,7},{4,9},{4,11},{4,13},{5,7},{5,9},{5,10},{5,14},{6,8},{6,12},{6,13},{7,9},{8,11},{8,14},{9,12},{10,11},{10,12},{11,12}}

Cousin 1204: {{1,3},{1,7},{1,9},{2,7},{2,9},{2,13},{2,14},{3,6},{3,8},{3,10},{4,7},{4,9},{4,11},{4,13},{5,7},{5,9},{5,10},{5,14},{6,8},{6,12},{6,13},{7,8},{8,11},{8,14},{9,12},{10,11},{10,12},{11,12}}

Cousin 1205: {{1,4},{1,7},{1,9},{2,7},{2,9},{2,13},{2,14},{3,6},{3,7},{3,8},{3,9},{3,10},{4,11},{4,13},{5,7},{5,9},{5,10},{5,14},{6,8},{6,12},{6,13},{7,8},{8,11},{8,14},{9,12},{10,11},{10,12},{11,12}}

Cousin 1206: {{1,10},{1,11},{1,12},{2,7},{2,9},{2,13},{2,14},{3,6},{3,7},{3,8},{3,9},{3,10},{4,7},{4,9},{4,11},{4,13},{5,7},{5,9},{5,10},{5,14},{6,8},{6,12},{6,13},{7,8},{8,11},{8,14},{9,12},{11,13}}

Cousin 1207: {{1,5},{1,7},{1,9},{2,7},{2,9},{2,13},{2,14},{3,6},{3,7},{3,8},{3,9},{3,10},{4,7},{4,9},{4,11},{4,13},{5,10},{5,14},{6,8},{6,12},{6,13},{7,8},{8,11},{8,14},{9,12},{10,11},{10,12},{11,12}}

Cousin 1208: {{1,10},{1,11},{1,12},{2,7},{2,9},{2,13},{2,14},{3,6},{3,7},{3,8},{3,9},{3,10},{4,7},{4,9},{4,11},{4,13},{5,7},{5,9},{5,10},{5,14},{6,8},{6,12},{6,13},{7,8},{8,11},{8,14},{9,12},{10,14}}

Cousin 1209: {{1,10},{1,11},{1,12},{2,13},{2,14},{2,15},{3,7},{3,9},{3,10},{3,16},{4,7},{4,9},{4,11},{4,13},{5,7},{5,8},{5,10},{5,14},{6,12},{6,13},{6,16},{7,9},{7,15},{8,11},{8,15},{8,16},{9,12},{9,14}}

Cousin 1210: {{1,10},{1,11},{1,12},{2,13},{2,14},{2,15},{3,6},{3,8},{3,10},{3,16},{4,7},{4,9},{4,11},{4,13},{5,7},{5,8},{5,10},{5,14},{6,8},{6,12},{6,13},{7,15},{7,16},{8,11},{8,15},{9,12},{9,14},{9,16}}

Cousin 1211: {{1,10},{1,11},{1,12},{2,13},{2,14},{2,15},{3,6},{3,7},{3,8},{3,9},{3,10},{4,11},{4,13},{4,16},{5,7},{5,8},{5,10},{5,14},{6,8},{6,12},{6,13},{7,15},{7,16},{8,11},{8,15},{9,12},{9,14},{9,16}}

Cousin 1212: {{1,2},{1,7},{1,8},{2,13},{2,14},{3,6},{3,7},{3,8},{3,9},{3,10},{4,7},{4,9},{4,11},{4,13},{5,7},{5,8},{5,10},{5,14},{6,8},{6,12},{6,13},{7,9},{8,11},{9,12},{9,14},{10,11},{10,12},{11,12}}

Cousin 1213: {{1,10},{1,11},{1,12},{2,7},{2,8},{2,13},{2,14},{3,6},{3,7},{3,8},{3,9},{3,10},{4,7},{4,9},{4,11},{4,13},{5,7},{5,8},{5,10},{5,14},{6,8},{6,12},{6,13},{7,9},{8,11},{9,12},{9,14},{13,14}}

Cousin 1214: {{1,10},{1,11},{1,12},{2,7},{2,8},{2,13},{2,14},{3,10},{3,15},{3,16},{4,7},{4,9},{4,11},{4,13},{5,7},{5,8},{5,10},{5,14},{6,12},{6,13},{6,15},{7,8},{7,16},{8,11},{8,15},{9,12},{9,14},{9,16}}

{8,11},{8,15},{9,12},{9,14},{9,16}}

Cousin 1215: {{1,3},{1,6},{1,8},{2,7},{2,8},{2,13},{2,14},{3,7},{3,9},{3,10},{4,7},{4,9},{4,11},{4,13},{5,7},{5,8},{5,10},{5,14},{6,12},{6,13},{7,8},{7,9},{8,11},{9,12},{9,14},{10,11},{10,12},{11,12}}

Cousin 1216: {{1,10},{1,11},{1,12},{2,7},{2,8},{2,13},{2,14},{3,6},{3,9},{3,10},{3,15},{4,11},{4,13},{4,16},{5,7},{5,8},{5,10},{5,14},{6,8},{6,12},{6,13},{7,15},{7,16},{8,11},{8,15},{9,12},{9,14},{9,16}}

Cousin 1217: {{1,3},{1,7},{1,8},{2,7},{2,8},{2,13},{2,14},{3,6},{3,9},{3,10},{4,7},{4,9},{4,11},{4,13},{5,7},{5,8},{5,10},{5,14},{6,8},{6,12},{6,13},{7,9},{8,11},{9,12},{9,14},{10,11},{10,12},{11,12}}

Cousin 1218: {{1,10},{1,11},{1,12},{2,7},{2,8},{2,13},{2,14},{3,6},{3,8},{3,10},{3,15},{4,7},{4,9},{4,11},{4,13},{5,10},{5,14},{5,16},{6,8},{6,12},{6,13},{7,15},{7,16},{8,11},{8,16},{9,12},{9,14},{9,15}}

Cousin 1219: {{1,3},{1,7},{1,9},{2,7},{2,8},{2,13},{2,14},{3,6},{3,8},{3,10},{4,7},{4,9},{4,11},{4,13},{5,7},{5,8},{5,10},{5,14},{6,8},{6,12},{6,13},{7,8},{8,11},{9,12},{9,14},{10,11},{10,12},{11,12}}

Cousin 1220: {{1,10},{1,11},{1,12},{2,7},{2,8},{2,13},{2,14},{3,6},{3,7},{3,8},{3,9},{3,10},{4,11},{4,13},{4,15},{5,10},{5,14},{5,16},{6,8},{6,12},{6,13},{7,15},{7,16},{8,11},{8,16},{9,12},{9,14},{9,15}}

Cousin 1221: {{1,4},{1,7},{1,9},{2,7},{2,8},{2,13},{2,14},{3,6},{3,7},{3,8},{3,9},{3,10},{4,11},{4,13},{5,7},{5,8},{5,10},{5,14},{6,8},{6,12},{6,13},{7,8},{8,11},{9,12},{9,14},{10,11},{10,12},{11,12}}

Cousin 1222: {{1,10},{1,11},{1,12},{2,7},{2,8},{2,13},{2,14},{3,6},{3,7},{3,8},{3,9},{3,10},{4,7},{4,9},{4,11},{4,13},{5,7},{5,8},{5,10},{5,14},{6,8},{6,12},{6,13},{7,8},{8,11},{9,12},{9,14},{11,13}}

Cousin 1223: {{1,5},{1,7},{1,8},{2,7},{2,8},{2,13},{2,14},{3,6},{3,7},{3,8},{3,9},{3,10},{4,7},{4,9},{4,11},{4,13},{5,10},{5,14},{6,8},{6,12},{6,13},{7,9},{8,11},{9,12},{9,14},{10,11},{10,12},{11,12}}

Cousin 1224: {{1,10},{1,11},{1,12},{2,7},{2,8},{2,13},{2,14},{3,6},{3,7},{3,8},{3,9},{3,10},{4,7},{4,9},{4,11},{4,13},{5,7},{5,8},{5,10},{5,14},{6,8},{6,12},{6,13},{7,9},{8,11},{9,12},{9,14},{10,14}}

Cousin 1225: {{1,10},{1,11},{1,12},{2,5},{2,9},{2,13},{2,14},{3,10},{3,15},{3,16},{4,7},{4,9},{4,11},{4,13},{5,7},{5,8},{5,9},{5,10},{6,12},{6,13},{6,15},{7,14},{7,16},{8,11},{8,14},{8,15},{9,12},{9,16}}

Cousin 1226: {{1,10},{1,11},{1,12},{2,5},{2,9},{2,13},{2,14},{3,7},{3,9},{3,10},{3,15},{4,11},{4,13},{4,16},{5,7},{5,8},{5,9},{5,10},{6,12},{6,13},{6,15},{7,14},{7,16},{8,11},{8,14},{8,15},{9,12},{9,16}}

Cousin 1227: {{1,10},{1,11},{1,12},{2,5},{2,9},{2,13},{2,14},{3,7},{3,9},{3,10},{3,15},{4,7},{4,9},{4,11},{4,13},{5,8},{5,10},{5,16},{6,12},{6,13},{6,15},{7,14},{7,16},{8,11},{8,14},{8,15},{9,12},{9,16}}

Cousin 1228: {{1,3},{1,6},{1,8},{2,5},{2,9},{2,13},{2,14},{3,7},{3,9},{3,10},{4,7},{4,9},{4,11},{4,13},{5,7},{5,8},{5,9},{5,10},{6,12},{6,13},{7,9},{7,14},{8,11},{8,14},{9,12},{10,11},{10,12},{11,12}}

Cousin 1229: {{1,10},{1,11},{1,12},{2,5},{2,9},{2,13},{2,14},{3,6},{3,7},{3,9},{3,10},{4,7},{4,9},{4,11},{4,13},{5,7},{5,8},{5,9},{5,10},{6,8},{6,12},{6,13},{7,9},{7,14},{8,11},{8,14},{9,12},{12,13}}

Cousin 1230: {{1,3},{1,7},{1,9},{2,5},{2,9},{2,13},{2,14},{3,6},{3,8},{3,10},{4,7},{4,9},{4,11},{4,13},{5,7},{5,8},{5,9},{5,10},{6,8},{6,12},{6,13},{7,14},{8,11},{8,14},{9,12},{10,11},{10,12},{11,12}}

Cousin 1231: {{1,4},{1,7},{1,9},{2,5},{2,9},{2,13},{2,14},{3,6},{3,7},{3,8},{3,9},{3,10},{4,11},{4,13},{5,7},{5,8},{5,9},{5,10},{6,8},{6,12},{6,13},{7,14},{8,11},{8,14},{9,12},{10,11},{10,12},{11,12}}

Cousin 1232: {{1,10},{1,11},{1,12},{2,5},{2,9},{2,13},{2,14},{3,6},{3,7},{3,8},{3,9},{3,10},{4,7},{4,9},{4,11},{4,13},{5,7},{5,8},{5,9},{5,10},{6,8},{6,12},{6,13},{7,14},{8,11},{8,14},{9,12},{11,13}}

Cousin 1233: {{1,5},{1,7},{1,9},{2,5},{2,9},{2,13},{2,14},{3,6},{3,7},{3,8},{3,9},{3,10},{4,7},{4,9},{4,11},{4,13},{5,8},{5,10},{6,8},{6,12},{6,13},{7,14},{8,11},{8,14},{9,12},{10,11},{10,12},{11,12}}

Cousin 1234: {{1,3},{1,6},{1,8},{2,5},{2,8},{2,13},{2,14},{3,7},{3,9},{3,10},{4,7},{4,9},{4,11},{4,13},{5,7},{5,8},{5,9},{5,10},{6,12},{6,13},{7,8},{7,14},{8,11},{9,12},{9,14},{10,11},{10,12},{11,12}}

Cousin 1235: {{1,10},{1,11},{1,12},{2,5},{2,8},{2,13},{2,14},{3,6},{3,7},{3,9},{3,10},{4,7},{4,9},{4,11},{4,13},{5,7},{5,8},{5,9},{5,10},{6,8},{6,12},{6,13},{7,8},{7,14},{8,11},{9,12},{9,14},{12,13}}

Cousin 1236: {{1,3},{1,7},{1,8},{2,5},{2,8},{2,13},{2,14},{3,6},{3,9},{3,10},{4,7},{4,9},{4,11},{4,13},{5,7},{5,8},{5,9},{5,10},{6,8},{6,12},{6,13},{7,14},{8,11},{9,12},{9,14},{10,11},{10,12},{11,12}}

Cousin 1237: {{1,5},{1,7},{1,8},{2,5},{2,8},{2,13},{2,14},{3,6},{3,7},{3,8},{3,9},{3,10},{4,7},{4,9},{4,11},{4,13},{5,9},{5,10},{6,8},{6,12},{6,13},{7,14},{8,11},{9,12},{9,14},{10,11},{10,12},{11,12}}

Cousin 1238: {{1,3},{1,7},{1,9},{2,5},{2,7},{2,8},{2,9},{2,13},{3,10},{3,14},{4,7},{4,9},{4,11},{4,13},{5,7},{5,8},{5,9},{5,10},{6,12},{6,13},{6,14},{7,8},{8,11},{8,14},{9,12},{10,11},{10,12},{11,12}}

Cousin 1239: {{1,10},{1,11},{1,12},{2,5},{2,7},{2,8},{2,9},{2,13},{3,7},{3,9},{3,10},{3,14},{4,7},{4,9},{4,11},{4,13},{5,7},{5,8},{5,9},{5,10},{6,12},{6,13},{6,14},{7,8},{8,11},{8,14},{9,12},{10,14}}

Cousin 1240: {{1,10},{1,11},{1,12},{2,5},{2,7},{2,8},{2,9},{2,13},{3,6},{3,10},{3,14},{4,7},{4,9},{4,11},{4,13},{5,7},{5,8},{5,9},{5,10},{6,7},{6,9},{7,8},{8,11},{8,14},{9,12},{12,13},{12,14},{13,14}}

Cousin 1241: {{1,3},{1,6},{1,8},{1,12},{2,5},{2,6},{2,7},{2,8},{2,9},{3,7},{3,9},{3,10},{4,6},{4,7},{4,9},{4,11},{5,7},{5,8},{5,9},{5,10},{6,12},{7,8},{7,9},{8,11},{9,12},{10,11},{10,12},{11,12}}

Cousin 1242: {{1,4},{1,7},{1,9},{2,5},{2,7},{2,8},{2,9},{2,13},{3,6},{3,9},{3,10},{3,14},{4,11},{4,13},{5,7},{5,8},{5,9},{5,10},{6,8},{6,12},{6,13},{7,14},{8,11},{8,14},{9,12},{10,11},{10,12},{11,12}}

Cousin 1243: {{1,10},{1,11},{1,12},{2,5},{2,7},{2,8},{2,9},{2,13},{3,6},{3,9},{3,10},{3,14},{4,7},{4,9},{4,11},{4,13},{5,7},{5,8},{5,9},{5,10},{6,8},{6,12},{6,13},{7,14},{8,11},{8,14},{9,12},{11,13}}

Cousin 1244: {{1,5},{1,7},{1,9},{2,5},{2,7},{2,8},{2,9},{2,13},{3,6},{3,9},{3,10},{3,14},{4,7},{4,9},{4,11},{4,13},{5,8},{5,10},{6,8},{6,12},{6,13},{7,14},{8,11},{8,14},{9,12},{10,11},{10,12},{11,12}}

Cousin 1245: {{1,5},{1,7},{1,8},{2,5},{2,7},{2,8},{2,9},{2,13},{3,6},{3,8},{3,10},{3,14},{4,7},{4,9},{4,11},{4,13},{5,9},{5,10},{6,8},{6,12},{6,13},{7,14},{8,11},{9,12},{9,14},{10,11},{10,12},{11,12}}

Cousin 1246: {{1,5},{1,7},{1,8},{2,5},{2,7},{2,8},{2,9},{2,13},{3,6},{3,7},{3,8},{3,9},{3,10},{4,11},{4,13},{4,14},{5,9},{5,10},{6,8},{6,12},{6,13},{7,14},{8,11},{9,12},{9,14},{10,11},{10,12},{11,12}}

Cousin 1247: {{1,10},{1,11},{1,12},{2,5},{2,7},{2,8},{2,9},{2,13},{3,6},{3,7},{3,8},{3,9},{3,10},{4,5},{4,7},{4,8},{5,9},{5,10},{6,8},{6,12},{6,13},{7,14},{8,11},{9,12},{9,14},{11,13},{11,14},{13,14}}

Cousin 1248: {{1,4},{1,7},{1,9},{1,11},{2,4},{2,5},{2,7},{2,8},{2,9},{3,6},{3,7},{3,8},{3,9},{3,10},{4,6},{4,11},{5,7},{5,8},{5,9},{5,10},{6,8},{6,12},{7,8},{8,11},{9,12},{10,11},{10,12},{11,12}}

Cousin 1249: {{1,10},{1,11},{1,12},{2,6},{2,9},{2,13},{2,14},{3,10},{3,15},{3,16},{4,6},{4,9},{4,11},{4,13},{5,7},{5,9},{5,10},{5,14},{6,12},{6,15},{7,8},{7,13},{7,16},{8,11},{8,14},{8,15},{9,12},{9,16}}

Cousin 1250: {{1,3},{1,6},{1,8},{2,6},{2,9},{2,13},{2,14},{3,7},{3,9},{3,10},{4,6},{4,9},{4,11},{4,13},{5,7},{5,9},{5,10},{5,14},{6,12},{7,8},{7,9},{7,13},{8,11},{8,14},{9,12},{10,11},{10,12},{11,12}}

Cousin 1251: {{1,3},{1,7},{1,8},{2,6},{2,9},{2,13},{2,14},{3,6},{3,9},{3,10},{4,6},{4,9},{4,11},{4,13},{5,7},{5,9},{5,10},{5,14},{6,8},{6,12},{7,9},{7,13},{8,11},{8,14},{9,12},{10,11},{10,12},{11,12}}

Cousin 1252: {{1,3},{1,7},{1,9},{2,6},{2,9},{2,13},{2,14},{3,6},{3,8},{3,10},{4,6},{4,9},{4,11},{4,13},{5,7},{5,9},{5,10},{5,14},{6,8},{6,12},{7,8},{7,13},{8,11},{8,14},{9,12},{10,11},{10,12},{11,12}}

Cousin 1253: {{1,10},{1,11},{1,12},{2,13},{2,14},{2,15},{3,6},{3,9},{3,10},{3,16},{4,6},{4,9},{4,11},{4,13},{5,7},{5,8},{5,10},{5,14},{6,12},{6,15},{7,9},{7,13},{7,16},{8,11},{8,15},{8,16},{9,12},{9,14}}

Cousin 1254: {{1,10},{1,11},{1,12},{2,13},{2,14},{2,15},{3,6},{3,8},{3,10},{3,16},{4,6},{4,9},{4,11},{4,13},{5,7},{5,8},{5,10},{5,14},{6,12},{6,15},{7,8},{7,13},{7,16},{8,11},{8,15},{9,12},{9,14},{9,16}}

Cousin 1255: {{1,2},{1,6},{1,8},{2,13},{2,14},{3,6},{3,7},{3,8},{3,9},{3,10},{4,6},{4,9},{4,11},{4,13},{5,7},{5,8},{5,10},{5,14},{6,12},{7,8},{7,9},{7,13},{8,11},{9,12},{9,14},{10,11},{10,12},{11,12}}

Cousin 1256: {{1,10},{1,11},{1,12},{2,6},{2,8},{2,13},{2,14},{3,6},{3,7},{3,8},{3,9},{3,10},{4,6},{4,9},{4,11},{4,13},{5,7},{5,8},{5,10},{5,14},{6,12},{7,8},{7,9},{7,13},{8,11},{9,12},{9,14},{13,14}}

Cousin 1257: {{1,10},{1,11},{1,12},{2,6},{2,8},{2,13},{2,14},{3,10},{3,15},{3,16},{4,6},{4,9},{4,11},{4,13},{5,7},{5,8},{5,10},{5,14},{6,12},{6,15},{7,8},{7,13},{7,16},{8,11},{8,15},{9,12},{9,14},{9,16}}

Cousin 1258: {{1,3},{1,6},{1,8},{2,6},{2,8},{2,13},{2,14},{3,7},{3,9},{3,10},{4,6},{4,9},{4,11},{4,13},{5,7},{5,8},{5,10},{5,14},{6,12},{7,8},{7,9},{7,13},{8,11},{9,12},{9,14},{10,11},{10,12},{11,12}}

Cousin 1259: {{1,3},{1,7},{1,8},{2,6},{2,8},{2,13},{2,14},{3,6},{3,9},{3,10},{4,6},{4,9},{4,11},{4,13},{5,7},{5,8},{5,10},{5,14},{6,8},{6,12},{7,9},{7,13},{8,11},{9,12},{9,14},{10,11},{10,12},{11,12}}

Cousin 1260: {{1,3},{1,7},{1,9},{2,6},{2,8},{2,13},{2,14},{3,6},{3,8},{3,10},{4,6},{4,9},{4,11},{4,13},{5,7},{5,8},{5,10},{5,14},{6,8},{6,12},{7,8},{7,13},{8,11},{9,12},{9,14},{10,11},{10,12},{11,12}}

Cousin 1261: {{1,3},{1,7},{1,8},{2,5},{2,9},{2,13},{2,14},{3,6},{3,9},{3,10},{4,6},{4,9},{4,11},{4,13},{5,7},{5,8},{5,9},{5,10},{6,12},{6,14},{7,9},{7,13},{8,11},{8,14},{9,12},{10,11},{10,12},{11,12}}

Cousin 1262: {{1,3},{1,7},{1,9},{2,5},{2,9},{2,13},{2,14},{3,6},{3,8},{3,10},{4,6},{4,9},{4,11},{4,13},{5,7},{5,8},{5,9},{5,10},{6,12},{6,14},{7,8},{7,13},{8,11},{8,14},{9,12},{10,11},{10,12},{11,12}}

Cousin 1263: {{1,5},{1,7},{1,8},{2,5},{2,9},{2,13},{2,14},{3,6},{3,7},{3,8},{3,9},{3,10},{4,6},{4,9},{4,11},{4,13},{5,9},{5,10},{6,12},{6,14},{7,9},{7,13},{8,11},{8,14},{9,12},{10,11},{10,12},{11,12}}

Cousin 1264: {{1,5},{1,7},{1,9},{2,5},{2,9},{2,13},{2,14},{3,6},{3,7},{3,8},{3,9},{3,10},{4,6},{4,9},{4,11},{4,13},{5,8},{5,10},{6,12},{6,14},{7,8},{7,13},{8,11},{8,14},{9,12},{10,11},{10,12},{11,12}}

Cousin 1265: {{1,3},{1,7},{1,9},{2,5},{2,6},{2,8},{2,9},{2,13},{3,10},{3,14},{4,6},{4,9},{4,11},{4,13},{5,7},{5,8},{5,9},{5,10},{6,12},{6,14},{7,8},{7,13},{8,11},{8,14},{9,12},{10,11},{10,12},{11,12}}

Cousin 1266: {{1,10},{1,11},{1,12},{2,5},{2,6},{2,8},{2,9},{2,13},{3,7},{3,9},{3,10},{3,14},{4,6},{4,9},{4,11},{4,13},{5,7},{5,8},{5,9},{5,10},{6,12},{6,14},{7,8},{7,13},{8,11},{8,14},{9,12},{10,14}}

Cousin 1267: {{1,5},{1,7},{1,8},{2,5},{2,6},{2,8},{2,9},{2,13},{3,7},{3,9},{3,10},{3,14},{4,6},{4,9},{4,11},{4,13},{5,9},{5,10},{6,12},{6,14},{7,9},{7,13},{8,11},{8,14},{9,12},{10,11},{10,12},{11,12}}

Cousin 1268: {{1,5},{1,7},{1,9},{2,5},{2,6},{2,8},{2,9},{2,13},{3,7},{3,9},{3,10},{3,14},{4,6},{4,9},{4,11},{4,13},{5,8},{5,10},{6,12},{6,14},{7,8},{7,13},{8,11},{8,14},{9,12},{10,11},{10,12},{11,12}}

Cousin 1269: {{1,10},{1,11},{1,12},{2,6},{2,7},{2,13},{2,14},{3,10},{3,15},{3,16},{4,6},{4,7},{4,11},{4,13},{5,7},{5,9},{5,10},{5,14},{6,12},{6,15},{7,8},{7,16},{8,11},{8,14},{8,15},{9,12},{9,13},{9,16}}

Cousin 1270: {{1,10},{1,11},{1,12},{2,6},{2,7},{2,13},{2,14},{3,7},{3,9},{3,10},{3,15},{4,6},{4,7},{4,11},{4,13},{5,10},{5,14},{5,16},{6,12},{6,15},{7,8},{7,16},{8,11},{8,14},{8,15},{9,12},{9,13},{9,16}}

Cousin 1271: {{1,3},{1,6},{1,8},{2,6},{2,7},{2,13},{2,14},{3,7},{3,9},{3,10},{4,6},{4,7},{4,11},{4,13},{5,7},{5,9},{5,10},{5,14},{6,12},{7,8},{7,9},{8,11},{8,14},{9,12},{9,13},{10,11},{10,12},{11,12}}

Cousin 1272: {{1,3},{1,7},{1,8},{2,6},{2,7},{2,13},{2,14},{3,6},{3,9},{3,10},{4,6},{4,7},{4,11},{4,13},{5,7},{5,9},{5,10},{5,14},{6,8},{6,12},{7,9},{8,11},{8,14},{9,12},{9,13},{10,11},{10,12},{11,12}}

Cousin 1273: {{1,3},{1,7},{1,9},{2,6},{2,7},{2,13},{2,14},{3,6},{3,8},{3,10},{4,6},{4,7},{4,11},{4,13},{5,7},{5,9},{5,10},{5,14},{6,8},{6,12},{7,8},{8,11},{8,14},{9,12},{9,13},{10,11},{10,12},{11,12}}

Cousin 1274: {{1,5},{1,7},{1,9},{2,6},{2,7},{2,13},{2,14},{3,6},{3,7},{3,8},{3,9},{3,10},{4,6},{4,7},{4,11},{4,13},{5,10},{5,14},{6,8},{6,12},{7,8},{8,11},{8,14},{9,12},{9,13},{10,11},{10,12},{11,12}}

Cousin 1275: {{1,10},{1,11},{1,12},{2,5},{2,7},{2,13},{2,14},{3,6},{3,9},{3,10},{3,15},{4,6},{4,7},{4,11},{4,13},{5,8},{5,10},{5,16},{6,12},{6,14},{7,15},{7,16},{8,11},{8,14},{8,15},{9,12},{9,13},{9,16}}

Cousin 1276: {{1,3},{1,7},{1,8},{2,5},{2,7},{2,13},{2,14},{3,6},{3,9},{3,10},{4,6},{4,7},{4,11},{4,13},{5,7},{5,8},{5,9},{5,10},{6,12},{6,14},{7,9},{8,11},{8,14},{9,12},{9,13},{10,11},{10,12},{11,12}}

Cousin 1277: {{1,10},{1,11},{1,12},{2,5},{2,7},{2,13},{2,14},{3,6},{3,8},{3,10},{3,15},{4,6},{4,7},{4,11},{4,13},{5,9},{5,10},{5,16},{6,12},{6,14},{7,15},{7,16},{8,11},{8,14},{8,16},{9,12},{9,13},{9,15}}

Cousin 1278: {{1,3},{1,7},{1,9},{2,5},{2,7},{2,13},{2,14},{3,6},{3,8},{3,10},{4,6},{4,7},{4,11},{4,13},{5,7},{5,8},{5,9},{5,10},{6,12},{6,14},{7,8},{8,11},{8,14},{9,12},{9,13},{10,11},{10,12},{11,12}}

Cousin 1279: {{1,5},{1,7},{1,8},{2,5},{2,7},{2,13},{2,14},{3,6},{3,7},{3,8},{3,9},{3,10},{4,6},{4,7},{4,11},{4,13},{5,9},{5,10},{6,12},{6,14},{7,9},{8,11},{8,14},{9,12},{9,13},{10,11},{10,12},{11,12}}

Cousin 1280: {{1,5},{1,7},{1,9},{2,5},{2,7},{2,13},{2,14},{3,6},{3,7},{3,8},{3,9},{3,10},{4,6},{4,7},{4,11},{4,13},{5,8},{5,10},{6,12},{6,14},{7,8},{8,11},{8,14},{9,12},{9,13},{10,11},{10,12},{11,12}}

Cousin 1281: {{1,10},{1,11},{1,12},{2,5},{2,6},{2,13},{2,14},{3,10},{3,15},{3,16},{4,6},{4,7},{4,11},{4,13},{5,7},{5,8},{5,9},{5,10},{6,12},{6,15},{7,14},{7,16},{8,11},{8,14},{8,15},{9,12},{9,13},{9,16}}

Cousin 1282: {{1,10},{1,11},{1,12},{2,5},{2,6},{2,13},{2,14},{3,7},{3,9},{3,10},{3,15},{4,6},{4,7},{4,11},{4,13},{5,8},{5,10},{5,16},{6,12},{6,15},{7,14},{7,16},{8,11},{8,14},{8,15},{9,12},{9,13},{9,16}}

Cousin 1283: {{1,3},{1,6},{1,8},{2,5},{2,6},{2,13},{2,14},{3,7},{3,9},{3,10},{4,6},{4,7},{4,11},{4,13},{5,7},{5,8},{5,9},{5,10},{6,12},{7,9},{7,14},{8,11},{8,14},{9,12},{9,13},{10,11},{10,12},{11,12}}

Cousin 1284: {{1,3},{1,7},{1,9},{2,5},{2,6},{2,13},{2,14},{3,6},{3,8},{3,10},{4,6},{4,7},{4,11},{4,13},{5,7},{5,8},{5,9},{5,10},{6,8},{6,12},{7,14},{8,11},{8,14},{9,12},{9,13},{10,11},{10,12},{11,12}}

Cousin 1285: {{1,5},{1,7},{1,9},{2,5},{2,6},{2,13},{2,14},{3,6},{3,7},{3,8},{3,9},{3,10},{4,6},{4,7},{4,11},{4,13},{5,8},{5,10},{6,8},{6,12},{7,14},{8,11},{8,14},{9,12},{9,13},{10,11},{10,12},{11,12}}

Cousin 1286: {{1,10},{1,11},{1,12},{2,5},{2,6},{2,7},{2,8},{2,13},{3,10},{3,14},{3,15},{4,6},{4,7},{4,11},{4,13},{5,9},{5,10},{5,16},{6,12},{6,14},{7,15},{7,16},{8,11},{8,14},{8,16},{9,12},{9,13},{9,15}}

Cousin 1287: {{1,3},{1,7},{1,9},{2,5},{2,6},{2,7},{2,8},{2,13},{3,10},{3,14},{4,6},{4,7},{4,11},{4,13},{5,7},{5,8},{5,9},{5,10},{6,12},{6,14},{7,8},{8,11},{8,14},{9,12},{9,13},{10,11},{10,12},{11,12}}

Cousin 1288: {{1,10},{1,11},{1,12},{2,5},{2,6},{2,7},{2,8},{2,13},{3,7},{3,9},{3,10},{3,14},{4,6},{4,7},{4,11},{4,13},{5,7},{5,8},{5,9},{5,10},{6,12},{6,14},{7,8},{8,11},{8,14},{9,12},{9,13},{10,14}}

Cousin 1289: {{1,5},{1,7},{1,8},{2,5},{2,6},{2,7},{2,8},{2,13},{3,7},{3,9},{3,10},{3,14},{4,6},{4,7},{4,11},{4,13},{5,9},{5,10},{6,12},{6,14},{7,9},{8,11},{8,14},{9,12},{9,13},{10,11},{10,12},{11,12}}

Cousin 1290: {{1,5},{1,7},{1,9},{2,5},{2,6},{2,7},{2,8},{2,13},{3,7},{3,9},{3,10},{3,14},{4,6},{4,7},{4,11},{4,13},{5,8},{5,10},{6,12},{6,14},{7,8},{8,11},{8,14},{9,12},{9,13},{10,11},{10,12},{11,12}}



{9,13},{10,11},{10,12},{11,12}}

Cousin 1291: {{1,5},{1,7},{1,9},{2,5},{2,6},{2,7},{2,8},{2,13},{3,6},{3,9},{3,10},{3,14},{4,6},{4,7},{4,11},{4,13},{5,8},{5,10},{6,8},{6,12},{7,14},{8,11},{8,14},{9,12},{9,13},{10,11},{10,12},{11,12}}

Cousin 1292: {{1,5},{1,7},{1,8},{2,5},{2,6},{2,7},{2,8},{2,13},{3,6},{3,8},{3,10},{3,14},{4,6},{4,7},{4,11},{4,13},{5,9},{5,10},{6,8},{6,12},{7,14},{8,11},{9,12},{9,13},{9,14},{10,11},{10,12},{11,12}}

Cousin 1293: {{1,3},{1,6},{1,8},{2,4},{2,6},{2,13},{2,14},{3,7},{3,9},{3,10},{4,6},{4,7},{4,9},{4,11},{5,7},{5,9},{5,10},{5,13},{6,12},{7,8},{7,14},{8,11},{8,13},{9,12},{9,14},{10,11},{10,12},{11,12}}

Cousin 1294: {{1,3},{1,7},{1,8},{2,4},{2,6},{2,13},{2,14},{3,6},{3,9},{3,10},{4,6},{4,7},{4,9},{4,11},{5,7},{5,9},{5,10},{5,13},{6,8},{6,12},{7,14},{8,11},{8,13},{9,12},{9,14},{10,11},{10,12},{11,12}}

Cousin 1295: {{1,3},{1,7},{1,9},{2,4},{2,6},{2,7},{2,9},{2,13},{3,10},{3,14},{4,6},{4,7},{4,9},{4,11},{5,7},{5,9},{5,10},{5,13},{6,12},{6,14},{7,8},{8,11},{8,13},{8,14},{9,12},{10,11},{10,12},{11,12}}

Cousin 1296: {{1,10},{1,11},{1,12},{2,4},{2,6},{2,7},{2,9},{2,13},{3,7},{3,9},{3,10},{3,14},{4,6},{4,7},{4,9},{4,11},{5,7},{5,9},{5,10},{5,13},{6,12},{6,14},{7,8},{8,11},{8,13},{8,14},{9,12},{10,14}}

Cousin 1297: {{1,4},{1,7},{1,9},{2,4},{2,6},{2,7},{2,9},{2,13},{3,7},{3,9},{3,10},{3,14},{4,6},{4,11},{5,7},{5,9},{5,10},{5,13},{6,12},{6,14},{7,8},{8,11},{8,13},{8,14},{9,12},{10,11},{10,12},{11,12}}

Cousin 1298: {{1,5},{1,7},{1,9},{2,4},{2,6},{2,7},{2,9},{2,13},{3,7},{3,9},{3,10},{3,14},{4,6},{4,7},{4,9},{4,11},{5,10},{5,13},{6,12},{6,14},{7,8},{8,11},{8,13},{8,14},{9,12},{10,11},{10,12},{11,12}}

Cousin 1299: {{1,10},{1,11},{1,12},{2,4},{2,6},{2,7},{2,9},{2,13},{3,7},{3,9},{3,10},{3,14},{4,6},{4,7},{4,9},{4,11},{5,7},{5,9},{5,10},{5,13},{6,12},{6,14},{7,8},{8,11},{8,13},{8,14},{9,12},{10,13}}

Cousin 1300: {{1,4},{1,7},{1,9},{2,4},{2,6},{2,7},{2,9},{2,13},{3,6},{3,9},{3,10},{3,14},{4,6},{4,11},{5,7},{5,9},{5,10},{5,13},{6,8},{6,12},{7,14},{8,11},{8,13},{8,14},{9,12},{10,11},{10,12},{11,12}}

Cousin 1301: {{1,5},{1,7},{1,9},{1,10},{2,4},{2,5},{2,6},{2,7},{2,9},{3,6},{3,7},{3,8},{3,9},{3,10},{4,6},{4,7},{4,9},{4,11},{5,8},{5,10},{6,8},{6,12},{7,8},{8,11},{9,12},{10,11},{10,12},{11,12}}

Cousin 1302: {{1,10},{1,11},{1,12},{2,4},{2,7},{2,13},{2,14},{3,6},{3,9},{3,10},{3,15},{4,6},{4,11},{4,16},{5,7},{5,8},{5,10},{5,13},{6,12},{6,14},{7,15},{7,16},{8,11},{8,14},{8,15},{9,12},{9,13},{9,16}}

Cousin 1303: {{1,3},{1,7},{1,8},{2,4},{2,7},{2,13},{2,14},{3,6},{3,9},{3,10},{4,6},{4,7},{4,9},{4,11},{5,7},{5,8},{5,10},{5,13},{6,12},{6,14},{7,9},{8,11},{8,14},{9,12},{9,13},{10,11},{10,12},{11,12}}

Cousin 1304: {{1,10},{1,11},{1,12},{2,4},{2,7},{2,13},{2,14},{3,6},{3,8},{3,10},{3,15},{4,6},{4,7},{4,9},{4,11},{5,10},{5,13},{5,16},{6,12},{6,14},{7,15},{7,16},{8,11},{8,14},{8,16},{9,12},{9,13},{9,15}}

Cousin 1305: {{1,3},{1,7},{1,9},{2,4},{2,7},{2,13},{2,14},{3,6},{3,8},{3,10},{4,6},{4,7},{4,9},{4,11},{5,7},{5,8},{5,10},{5,13},{6,12},{6,14},{7,8},{8,11},{8,14},{9,12},{9,13},{10,11},{10,12},{11,12}}

Cousin 1306: {{1,10},{1,11},{1,12},{2,4},{2,7},{2,13},{2,14},{3,6},{3,7},{3,8},{3,9},{3,10},{4,6},{4,11},{4,15},{5,10},{5,13},{5,16},{6,12},{6,14},{7,15},{7,16},{8,11},{8,14},{8,16},{9,12},{9,13},{9,15}}

Cousin 1307: {{1,4},{1,7},{1,9},{2,4},{2,7},{2,13},{2,14},{3,6},{3,7},{3,8},{3,9},{3,10},{4,6},{4,11},{5,7},{5,8},{5,10},{5,13},{6,12},{6,14},{7,8},{8,11},{8,14},{9,12},{9,13},{10,11},{10,12},{11,12}}

Cousin 1308: {{1,5},{1,7},{1,8},{2,4},{2,7},{2,13},{2,14},{3,6},{3,7},{3,8},{3,9},{3,10},{4,6},{4,7},{4,9},{4,11},{5,10},{5,13},{6,12},{6,14},{7,9},{8,11},{8,14},{9,12},{9,13},{10,11},{10,12},{11,12}}

Cousin 1309: {{1,10},{1,11},{1,12},{2,4},{2,7},{2,13},{2,14},{3,6},{3,7},{3,8},{3,9},{3,10},{4,6},{4,7},{4,9},{4,11},{5,7},{5,8},{5,10},{5,13},{6,12},{6,14},{7,9},{8,11},{8,14},{9,12},{9,13},{10,13}}

Cousin 1310: {{1,10},{1,11},{1,12},{2,4},{2,6},{2,13},{2,14},{3,10},{3,15},{3,16},{4,6},{4,7},{4,9},{4,11},{5,7},{5,8},{5,10},{5,13},{6,12},{6,15},{7,14},{7,16},{8,11},{8,14},{8,15},{9,12},{9,13},{9,16}}

Cousin 1311: {{1,10},{1,11},{1,12},{2,4},{2,6},{2,13},{2,14},{3,7},{3,9},{3,10},{3,15},{4,6},{4,11},{4,16},{5,7},{5,8},{5,10},{5,13},{6,12},{6,15},{7,14},{7,16},{8,11},{8,14},{8,15},{9,12},{9,13},{9,16}}

Cousin 1312: {{1,3},{1,6},{1,8},{2,4},{2,6},{2,13},{2,14},{3,7},{3,9},{3,10},{4,6},{4,7},{4,9},{4,11},{5,7},{5,8},{5,10},{5,13},{6,12},{7,9},{7,14},{8,11},{8,14},{9,12},{9,13},{10,11},{10,12},{11,12}}

Cousin 1313: {{1,3},{1,7},{1,9},{2,4},{2,6},{2,13},{2,14},{3,6},{3,8},{3,10},{4,6},{4,7},{4,9},{4,11},{5,7},{5,8},{5,10},{5,13},{6,8},{6,12},{7,14},{8,11},{8,14},{9,12},{9,13},{10,11},{10,12},{11,12}}

Cousin 1314: {{1,4},{1,7},{1,9},{2,4},{2,6},{2,13},{2,14},{3,6},{3,7},{3,8},{3,9},{3,10},{4,6},{4,11},{5,7},{5,8},{5,10},{5,13},{6,8},{6,12},{7,14},{8,11},{8,14},{9,12},{9,13},{10,11},{10,12},{11,12}}

Cousin 1315: {{1,10},{1,11},{1,12},{2,4},{2,6},{2,7},{2,8},{2,13},{3,10},{3,14},{3,15},{4,6},{4,7},{4,9},{4,11},{5,10},{5,13},{5,16},{6,12},{6,14},{7,15},{7,16},{8,11},{8,14},{8,16},{9,12},{9,13},{9,15}}

Cousin 1316: {{1,3},{1,7},{1,9},{2,4},{2,6},{2,7},{2,8},{2,13},{3,10},{3,14},{4,6},{4,7},{4,9},{4,11},{5,7},{5,8},{5,10},{5,13},{6,12},{6,14},{7,8},{8,11},{8,14},{9,12},{9,13},{10,11},{10,12},{11,12}}

Cousin 1317: {{1,10},{1,11},{1,12},{2,4},{2,6},{2,7},{2,8},{2,13},{3,7},{3,9},{3,10},{3,14},{4,6},{4,7},{4,9},{4,11},{5,7},{5,8},{5,10},{5,13},{6,12},{6,14},{7,8},{8,11},{8,14},{9,12},{9,13},{10,11},{10,12},{11,12}}

Cousin 1318: {{1,4},{1,7},{1,9},{2,4},{2,6},{2,7},{2,8},{2,13},{3,7},{3,9},{3,10},{3,14},{4,6},{4,11},{5,7},{5,8},{5,10},{5,13},{6,12},{6,14},{7,8},{8,11},{8,14},{9,12},{9,13},{10,11},{10,12},{11,12}}

Cousin 1319: {{1,5},{1,7},{1,8},{2,4},{2,6},{2,7},{2,8},{2,13},{3,7},{3,9},{3,10},{3,14},{4,6},{4,7},{4,9},{4,11},{5,10},{5,13},{6,12},{6,14},{7,9},{8,11},{8,14},{9,12},{9,13},{10,11},{10,12},{11,12}}

Cousin 1320: {{1,10},{1,11},{1,12},{2,4},{2,6},{2,7},{2,8},{2,13},{3,7},{3,9},{3,10},{3,14},{4,6},{4,7},{4,9},{4,11},{5,7},{5,8},{5,10},{5,13},{6,12},{6,14},{7,9},{8,11},{8,14},{9,12},{9,13},{10,13}}

Cousin 1321: {{1,4},{1,7},{1,9},{2,4},{2,6},{2,7},{2,8},{2,13},{3,6},{3,9},{3,10},{3,14},{4,6},{4,11},{5,7},{5,8},{5,10},{5,13},{6,8},{6,12},{7,14},{8,11},{8,14},{9,12},{9,13},{10,11},{10,12},{11,12}}

Cousin 1322: {{1,5},{1,7},{1,8},{1,10},{2,4},{2,5},{2,6},{2,7},{2,8},{3,6},{3,7},{3,8},{3,9},{3,10},{4,6},{4,7},{4,9},{4,11},{5,9},{5,10},{6,8},{6,12},{7,9},{8,11},{9,12},{10,11},{10,12},{11,12}}

Cousin 1323: {{1,3},{1,7},{1,8},{2,4},{2,5},{2,13},{2,14},{3,6},{3,9},{3,10},{4,6},{4,7},{4,9},{4,11},{5,7},{5,8},{5,9},{5,10},{6,12},{6,13},{7,14},{8,11},{8,13},{9,12},{9,14},{10,11},{10,12},{11,12}}

Cousin 1324: {{1,5},{1,7},{1,8},{2,4},{2,5},{2,13},{2,14},{3,6},{3,7},{3,8},{3,9},{3,10},{4,6},{4,7},{4,9},{4,11},{5,9},{5,10},{6,12},{6,13},{7,14},{8,11},{8,13},{9,12},{9,14},{10,11},{10,12},{11,12}}

Cousin 1325: {{1,4},{1,7},{1,9},{2,4},{2,5},{2,7},{2,9},{2,13},{3,6},{3,9},{3,10},{3,14},{4,6},{4,11},{5,7},{5,8},{5,9},{5,10},{6,12},{6,13},{7,14},{8,11},{8,13},{8,14},{9,12},{10,11},{10,12},{11,12}}

Cousin 1326: {{1,5},{1,7},{1,9},{2,4},{2,5},{2,7},{2,9},{2,13},{3,6},{3,9},{3,10},{3,14},{4,6},{4,7},{4,9},{4,11},{5,8},{5,10},{6,12},{6,13},{7,14},{8,11},{8,13},{8,14},{9,12},{10,11},{10,12},{11,12}}

Cousin 1327: {{1,5},{1,7},{1,8},{2,4},{2,5},{2,7},{2,9},{2,13},{3,6},{3,8},{3,10},{3,14},{4,6},{4,7},{4,9},{4,11},{5,9},{5,10},{6,12},{6,13},{7,14},{8,11},{8,13},{9,12},{9,14},{10,11},{10,12},{11,12}}

Cousin 1328: {{1,5},{1,7},{1,8},{2,4},{2,5},{2,7},{2,9},{2,13},{3,6},{3,7},{3,8},{3,9},{3,10},{4,6},{4,11},{4,14},{5,9},{5,10},{6,12},{6,13},{7,14},{8,11},{8,13},{9,12},{9,14},{10,11},{10,12},{11,12}}

Cousin 1329: {{1,3},{1,7},{1,9},{2,4},{2,5},{2,6},{2,9},{2,13},{3,10},{3,14},{4,6},{4,7},{4,9},{4,11},{5,7},{5,8},{5,9},{5,10},{6,12},{6,14},{7,13},{8,11},{8,13},{8,14},{9,12},{10,11},{10,12},{11,12}}

Cousin 1330: {{1,10},{1,11},{1,12},{2,4},{2,5},{2,6},{2,9},{2,13},{3,7},{3,9},{3,10},{3,14},{4,6},{4,7},{4,9},{4,11},{5,7},{5,8},{5,9},{5,10},{6,12},{6,14},{7,13},{8,11},{8,13},{8,14},{9,12},{10,14}}

Cousin 1331: {{1,4},{1,7},{1,9},{2,4},{2,5},{2,6},{2,9},{2,13},{3,7},{3,9},{3,10},{3,14},{4,6},{4,11},{5,7},{5,8},{5,9},{5,10},{6,12},{6,14},{7,13},{8,11},{8,13},{8,14},{9,12},{10,11},{10,12},{11,12}}

Cousin 1332: {{1,5},{1,7},{1,9},{2,4},{2,5},{2,6},{2,9},{2,13},{3,7},{3,9},{3,10},{3,14},{4,6},{4,7},{4,9},{4,11},{5,8},{5,10},{6,12},{6,14},{7,13},{8,11},{8,13},{8,14},{9,12},{10,11},{10,12},{11,12}}

Cousin 1333: {{1,5},{1,7},{1,8},{2,4},{2,5},{2,6},{2,8},{2,13},{3,7},{3,9},{3,10},{3,14},{4,6},{4,7},{4,9},{4,11},{5,9},{5,10},{6,12},{6,14},{7,13},{8,11},{8,14},{9,12},{9,13},{10,11},{10,12},{11,12}}

Cousin 1334: {{1,5},{1,7},{1,8},{2,4},{2,5},{2,6},{2,7},{2,8},{2,9},{3,10},{3,13},{3,14},{4,6},{4,7},{4,9},{4,11},{5,9},{5,10},{6,12},{6,13},{7,14},{8,11},{8,13},{9,12},{9,14},{10,11},{10,12},{11,12}}

Cousin 1335: {{1,10},{1,11},{1,12},{2,4},{2,5},{2,6},{2,7},{2,8},{2,9},{3,5},{3,7},{3,8},{4,6},{4,7},{4,9},{4,11},{5,9},{5,10},{6,12},{6,13},{7,14},{8,11},{8,13},{9,12},{9,14},{10,13},{10,14},{13,14}}

Cousin 1336: {{1,3},{1,7},{1,9},{1,10},{2,4},{2,5},{2,6},{2,7},{2,8},{2,9},{3,6},{3,8},{3,10},{4,6},{4,7},{4,9},{4,11},{5,7},{5,8},{5,9},{5,10},{6,12},{7,8},{8,11},{9,12},{10,11},{10,12},{11,12}}

Cousin 1337: {{1,5},{1,7},{1,8},{2,4},{2,5},{2,6},{2,7},{2,8},{2,9},{3,7},{3,9},{3,10},{3,13},{4,6},{4,11},{4,14},{5,9},{5,10},{6,12},{6,13},{7,14},{8,11},{8,13},{9,12},{9,14},{10,11},{10,12},{11,12}}

Cousin 1338: {{1,6},{1,9},{1,10},{1,11},{2,7},{2,9},{2,12},{2,13},{3,7},{3,9},{3,10},{3,14},{4,7},{4,9},{4,11},{4,12},{5,7},{5,9},{5,10},{5,13},{6,9},{6,12},{6,14},{7,8},{8,11},{8,13},{8,14},{10,14}}

Cousin 1339: {{1,6},{1,9},{1,10},{1,11},{2,7},{2,9},{2,12},{2,13},{3,10},{3,14},{3,15},{4,11},{4,12},{4,16},{5,7},{5,9},{5,10},{5,13},{6,8},{6,12},{6,14},{7,15},{7,16},{8,11},{8,13},{8,15},{9,14},{9,16}}

Cousin 1340: {{1,6},{1,9},{1,10},{1,11},{2,7},{2,9},{2,12},{2,13},{3,7},{3,8},{3,10},{3,14},{4,7},{4,9},{4,11},{4,12},{5,7},{5,9},{5,10},{5,13},{6,8},{6,12},{6,14},{7,9},{8,11},{8,13},{9,14},{10,14}}

Cousin 1341: {{1,6},{1,9},{1,10},{1,11},{2,7},{2,9},{2,12},{2,13},{3,7},{3,8},{3,10},{3,14},{4,7},{4,9},{4,11},{4,12},{5,7},{5,9},{5,10},{5,13},{6,8},{6,12},{6,14},{7,8},{8,11},{8,13},{9,14},{11,12}}

Cousin 1342: {{1,6},{1,9},{1,10},{1,11},{2,7},{2,9},{2,12},{2,13},{3,6},{3,9},{3,10},{3,14},{4,7},{4,9},{4,11},{4,12},{5,7},{5,9},{5,10},{5,13},{6,8},{6,9},{6,12},{7,14},{8,11},{8,13},{8,14},{11,12}}

Cousin 1343: {{1,6},{1,9},{1,10},{1,11},{2,7},{2,8},{2,12},{2,13},{3,7},{3,9},{3,10},{3,14},{4,7},{4,9},{4,11},{4,12},{5,7},{5,8},{5,10},{5,13},{6,9},{6,12},{6,14},{7,8},{8,11},{8,14},{9,13},{10,14}}

Cousin 1344: {{1,6},{1,9},{1,10},{1,11},{2,7},{2,8},{2,12},{2,13},{3,6},{3,9},{3,10},{3,14},{4,7},{4,9},{4,11},{4,12},{5,7},{5,8},{5,10},{5,13},{6,8},{6,9},{6,12},{7,14},{8,11},{8,14},{9,13},{11,12}}

Cousin 1345: {{1,6},{1,9},{1,10},{1,11},{2,5},{2,9},{2,12},{2,13},{3,7},{3,9},{3,10},{3,14},{4,7},{4,9},{4,11},{4,12},{5,7},{5,8},{5,9},{5,10},{6,9},{6,12},{6,14},{7,13},{8,11},{8,13},{8,14},{10,14}}

Cousin 1346: {{1,6},{1,9},{1,10},{1,11},{2,5},{2,9},{2,12},{2,13},{3,7},{3,9},{3,10},{3,14},{4,7},{4,9},{4,11},{4,12},{5,7},{5,8},{5,9},{5,10},{6,9},{6,12},{6,14},{7,13},{8,11},{8,13},{8,14},{11,12}}

Cousin 1347: {{1,6},{1,9},{1,10},{1,11},{2,5},{2,9},{2,12},{2,13},{3,7},{3,8},{3,10},{3,14},{4,7},{4,9},{4,11},{4,12},{5,7},{5,8},{5,9},{5,10},{6,8},{6,12},{6,14},{7,13},{8,11},{8,13},{9,14},{11,12}}

Cousin 1348: {{1,6},{1,9},{1,10},{1,11},{2,5},{2,8},{2,12},{2,13},{3,7},{3,8},{3,10},{3,14},{4,7},{4,9},{4,11},{4,12},{5,7},{5,8},{5,9},{5,10},{6,8},{6,12},{6,14},{7,13},{8,11},{9,13},{9,14},{10,14}}

Cousin 1349: {{1,6},{1,9},{1,10},{1,11},{2,5},{2,7},{2,8},{2,9},{2,12},{3,4},{3,7},{3,9},{4,11},{4,12},{5,7},{5,8},{5,9},{5,10},{6,8},{6,12},{6,13},{7,14},{8,11},{8,14},{9,13},{10,13},{10,14},{13,14}}

Cousin 1350: {{1,6},{1,9},{1,10},{1,11},{2,6},{2,7},{2,12},{2,13},{3,7},{3,9},{3,10},{3,14},{4,6},{4,7},{4,11},{4,12},{5,7},{5,9},{5,10},{5,13},{6,9},{6,14},{7,8},{8,11},{8,13},{8,14},{9,12},{10,14}}

Cousin 1351: {{1,6},{1,9},{1,10},{1,11},{2,5},{2,7},{2,12},{2,13},{3,10},{3,14},{3,15},{4,6},{4,7},{4,11},{4,12},{5,8},{5,10},{5,16},{6,13},{6,14},{7,15},{7,16},{8,11},{8,13},{8,15},{9,12},{9,14},{9,16}}

Cousin 1352: {{1,6},{1,9},{1,10},{1,11},{2,5},{2,7},{2,12},{2,13},{3,7},{3,8},{3,10},{3,14},{4,6},{4,7},{4,11},{4,12},{5,7},{5,8},{5,9},{5,10},{6,13},{6,14},{7,9},{8,11},{8,13},{9,12},{9,14},{10,14}}

Cousin 1353: {{1,6},{1,9},{1,10},{1,11},{2,5},{2,6},{2,12},{2,13},{3,7},{3,9},{3,10},{3,14},{4,6},{4,7},{4,11},{4,12},{5,7},{5,8},{5,9},{5,10},{6,9},{6,14},{7,13},{8,11},{8,13},{8,14},{9,12},{10,14}}

Cousin 1354: {{1,6},{1,9},{1,10},{1,11},{2,5},{2,6},{2,7},{2,8},{2,12},{3,5},{3,7},{3,8},{4,6},{4,7},{4,11},{4,12},{5,9},{5,10},{6,9},{6,13},{7,14},{8,11},{8,13},{9,12},{9,14},{10,13},{10,14},{13,14}}

Cousin 1355: {{1,6},{1,9},{1,10},{1,11},{2,5},{2,6},{2,7},{2,8},{2,12},{3,5},{3,7},{3,9},{4,6},{4,7},{4,11},{4,12},{5,8},{5,10},{6,8},{6,13},{7,14},{8,11},{8,14},{9,12},{9,13},{10,13},{10,14},{13,14}}

Cousin 1356: {{1,6},{1,9},{1,10},{1,11},{2,4},{2,7},{2,12},{2,13},{3,7},{3,9},{3,10},{3,14},{4,6},{4,7},{4,9},{4,11},{5,7},{5,9},{5,10},{5,12},{6,13},{6,14},{7,8},{8,11},{8,12},{8,14},{9,13},{10,14}}

Cousin 1357: {{1,6},{1,9},{1,10},{1,11},{2,4},{2,6},{2,12},{2,13},{3,7},{3,8},{3,10},{3,14},{4,6},{4,7},{4,9},{4,11},{5,7},{5,9},{5,10},{5,12},{6,8},{6,14},{7,13},{8,11},{8,12},{9,13},{9,14},{10,14}}

Cousin 1358: {{1,6},{1,9},{1,10},{1,11},{2,4},{2,7},{2,12},{2,13},{3,10},{3,14},{3,15},{4,6},{4,11},{4,16},{5,7},{5,8},{5,10},{5,12},{6,13},{6,14},{7,15},{7,16},{8,11},{8,13},{8,15},{9,12},{9,14},{9,16}}

Cousin 1359: {{1,6},{1,9},{1,10},{1,11},{2,4},{2,7},{2,12},{2,13},{3,7},{3,8},{3,10},{3,14},{4,6},{4,7},{4,9},{4,11},{5,7},{5,8},{5,10},{5,12},{6,13},{6,14},{7,9},{8,11},{8,13},{9,12},{9,14},{10,14}}

Cousin 1360: {{1,6},{1,9},{1,10},{1,11},{2,4},{2,6},{2,12},{2,13},{3,10},{3,14},{3,15},{4,7},{4,11},{4,16},{5,7},{5,8},{5,10},{5,12},{6,14},{6,16},{7,13},{7,15},{8,11},{8,13},{8,14},{9,12},{9,15},{9,16}}

Cousin 1361: {{1,6},{1,9},{1,10},{1,11},{2,4},{2,6},{2,12},{2,13},{3,7},{3,9},{3,10},{3,14},{4,6},{4,7},{4,9},{4,11},{5,7},{5,8},{5,10},{5,12},{6,9},{6,14},{7,13},{8,11},{8,13},{8,14},{9,12},{10,14}}

Cousin 1362: {{1,6},{1,9},{1,10},{1,11},{2,4},{2,5},{2,12},{2,13},{3,7},{3,8},{3,10},{3,14},{4,6},{4,7},{4,9},{4,11},{5,7},{5,8},{5,9},{5,10},{6,12},{6,14},{7,13},{8,11},{8,12},{9,13},{9,14},{10,14}}

Cousin 1363: {{1,6},{1,9},{1,10},{1,11},{2,4},{2,5},{2,7},{2,9},{2,12},{3,4},{3,7},{3,9},{4,6},{4,11},{5,7},{5,8},{5,9},{5,10},{6,12},{6,13},{7,14},{8,11},{8,12},{8,14},{9,13},{10,13},{10,14},{13,14}}

Cousin 1364: {{1,6},{1,9},{1,10},{1,11},{2,4},{2,5},{2,7},{2,9},{2,12},{3,5},{3,7},{3,9},{4,6},{4,7},{4,9},{4,11},{5,8},{5,10},{6,12},{6,13},{7,14},{8,11},{8,12},{8,14},{9,13},{10,13},{10,14},{13,14}}

Cousin 1365: {{1,6},{1,9},{1,10},{1,11},{2,4},{2,5},{2,12},{2,13},{3,7},{3,9},{3,10},{3,14},{4,6},{4,7},{4,9},{4,11},{5,7},{5,8},{5,9},{5,10},{6,12},{6,14},{7,13},{8,11},{8,13},{8,14},{9,12},{10,14}}

Cousin 1366: {{1,6},{1,9},{1,10},{1,11},{2,4},{2,5},{2,7},{2,8},{2,12},{3,5},{3,7},{3,8},{4,6},{4,7},{4,9},{4,11},{5,9},{5,10},{6,12},{6,13},{7,14},{8,11},{8,13},{9,12},{9,13},{10,13},{10,14},{13,14}}

{9,14},{10,13},{10,14},{13,14}}

Cousin 1367: {{1,6},{1,9},{1,10},{1,11},{2,4},{2,5},{2,6},{2,9},{2,12},{3,4},{3,6},{3,9},{4,7},{4,11},{5,7},{5,8},{5,9},{5,10},{6,13},{7,12},{7,14},{8,11},{8,12},{8,13},{9,14},{10,13},{10,14},{13,14}}

Cousin 1368: {{1,6},{1,9},{1,10},{1,11},{2,4},{2,5},{2,6},{2,7},{2,8},{2,9},{3,5},{3,7},{3,8},{4,7},{4,11},{4,14},{5,9},{5,10},{6,12},{6,14},{7,13},{8,11},{8,12},{9,13},{9,14},{10,12},{10,13},{12,13}}

Cousin 1369: {{1,4},{1,9},{1,10},{1,11},{2,5},{2,6},{2,12},{2,13},{3,7},{3,8},{3,10},{3,14},{4,6},{4,7},{4,9},{4,12},{5,7},{5,8},{5,9},{5,10},{6,11},{6,14},{7,13},{8,11},{8,12},{9,13},{9,14},{10,14}}

Cousin 1370: {{1,4},{1,9},{1,10},{1,11},{2,5},{2,6},{2,7},{2,9},{2,12},{3,4},{3,7},{3,9},{4,6},{4,12},{5,7},{5,8},{5,9},{5,10},{6,11},{6,13},{7,14},{8,11},{8,12},{8,14},{9,13},{10,13},{10,14},{13,14}}

Cousin 1371: {{1,4},{1,9},{1,10},{1,11},{2,5},{2,6},{2,7},{2,9},{2,12},{3,5},{3,7},{3,9},{4,6},{4,7},{4,9},{4,12},{5,8},{5,10},{6,11},{6,13},{7,14},{8,11},{8,12},{8,14},{9,13},{10,13},{10,14},{13,14}}

Cousin 1372: {{1,8},{1,9},{1,10},{1,11},{2,3},{2,7},{2,9},{3,10},{3,15},{4,8},{4,9},{4,11},{4,12},{5,7},{5,9},{5,10},{5,13},{6,11},{6,14},{6,15},{7,8},{7,12},{8,13},{8,15},{9,14},{12,13},{12,14},{13,14}}

Cousin 1373: {{1,8},{1,9},{1,10},{1,11},{2,12},{2,13},{2,14},{3,6},{3,10},{3,15},{4,8},{4,9},{4,11},{4,12},{5,7},{5,9},{5,10},{5,13},{6,7},{6,9},{7,8},{7,12},{8,13},{8,15},{9,14},{11,14},{11,15},{14,15}}

Cousin 1374: {{1,8},{1,9},{1,10},{1,11},{2,5},{2,7},{2,9},{3,7},{3,9},{3,10},{3,15},{4,8},{4,9},{4,11},{4,12},{5,10},{5,13},{6,11},{6,14},{6,15},{7,8},{7,12},{8,13},{8,15},{9,14},{12,13},{12,14},{13,14}}

Cousin 1375: {{1,8},{1,9},{1,10},{1,11},{2,12},{2,13},{2,14},{3,7},{3,9},{3,10},{3,15},{4,8},{4,9},{4,11},{4,12},{5,7},{5,9},{5,10},{5,13},{6,11},{6,14},{6,15},{7,8},{7,12},{8,13},{8,15},{9,14},{10,13}}

Cousin 1376: {{1,8},{1,9},{1,10},{1,11},{2,12},{2,13},{2,14},{3,7},{3,9},{3,10},{3,15},{4,8},{4,9},{4,11},{4,12},{5,6},{5,10},{5,13},{6,7},{6,9},{7,8},{7,12},{8,13},{8,15},{9,14},{11,14},{11,15},{14,15}}

Cousin 1377: {{1,8},{1,9},{1,10},{1,11},{2,3},{2,6},{2,8},{2,11},{3,7},{3,9},{3,10},{4,8},{4,9},{4,11},{4,12},{5,7},{5,9},{5,10},{5,13},{6,9},{6,11},{6,12},{6,13},{7,8},{7,9},{7,12},{8,13},{12,13}}

Cousin 1378: {{1,8},{1,9},{1,10},{1,11},{2,5},{2,7},{2,9},{3,6},{3,9},{3,10},{3,15},{4,8},{4,9},{4,11},{4,12},{5,10},{5,13},{6,8},{6,11},{6,14},{7,12},{7,15},{8,13},{8,15},{9,14},{12,13},{12,14},{13,14}}

Cousin 1379: {{1,8},{1,9},{1,10},{1,11},{2,12},{2,13},{2,14},{3,6},{3,9},{3,10},{3,15},{4,8},{4,9},{4,11},{4,12},{5,7},{5,9},{5,10},{5,13},{6,8},{6,11},{6,14},{7,12},{7,15},{8,13},{8,15},{9,14},{10,13}}

Cousin 1380: {{1,8},{1,9},{1,10},{1,11},{2,12},{2,13},{2,14},{3,6},{3,9},{3,10},{3,15},{4,8},{4,9},{4,11},{4,12},{5,7},{5,10},{5,13},{6,8},{6,11},{6,14},{7,9},{7,12},{7,15},{8,13},{8,15},{9,14},{12,15}}

Cousin 1381: {{1,8},{1,9},{1,10},{1,11},{2,7},{2,9},{2,10},{2,13},{3,6},{3,7},{3,8},{3,9},{3,10},{4,8},{4,9},{4,11},{4,12},{5,6},{5,9},{5,12},{5,13},{6,8},{6,11},{7,8},{7,12},{8,13},{10,13},{12,13}}

Cousin 1382: {{1,8},{1,9},{1,10},{1,11},{2,6},{2,9},{2,12},{2,13},{3,6},{3,7},{3,9},{3,10},{4,8},{4,9},{4,11},{4,12},{5,7},{5,9},{5,10},{5,12},{5,13},{6,8},{6,9},{6,11},{7,8},{7,12},{8,13},{10,13}}

Cousin 1383: {{1,8},{1,9},{1,10},{1,11},{2,6},{2,7},{2,12},{2,13},{3,5},{3,7},{3,8},{4,7},{4,9},{4,11},{4,12},{5,10},{5,13},{6,9},{6,11},{6,14},{7,15},{8,12},{8,14},{9,13},{9,15},{10,14},{10,15},{14,15}}

Cousin 1384: {{1,8},{1,9},{1,10},{1,11},{2,6},{2,7},{2,12},{2,13},{3,10},{3,14},{3,15},{4,7},{4,9},{4,11},{4,12},{5,7},{5,8},{5,10},{5,13},{6,9},{6,11},{6,14},{7,15},{8,12},{8,14},{9,13},{9,15},{10,13}}

Cousin 1385: {{1,8},{1,9},{1,10},{1,11},{2,6},{2,7},{2,12},{2,13},{3,7},{3,9},{3,10},{3,14},{4,5},{4,7},{4,8},{5,10},{5,13},{6,9},{6,11},{6,14},{7,15},{8,12},{8,14},{9,13},{9,15},{11,12},{11,15},{12,15}}

Cousin 1386: {{1,8},{1,9},{1,10},{1,11},{2,6},{2,7},{2,12},{2,13},{3,4},{3,7},{3,9},{4,11},{4,12},{5,7},{5,8},{5,10},{5,13},{6,8},{6,11},{6,14},{7,15},{8,12},{8,15},{9,13},{9,14},{10,14},{10,15},{14,15}}

Cousin 1387: {{1,8},{1,9},{1,10},{1,11},{2,6},{2,7},{2,12},{2,13},{3,10},{3,14},{3,15},{4,7},{4,9},{4,11},{4,12},{5,7},{5,8},{5,10},{5,13},{6,8},{6,11},{6,14},{7,15},{8,12},{8,15},{9,13},{9,14},{11,12}}

Cousin 1388: {{1,8},{1,9},{1,10},{1,11},{2,6},{2,7},{2,12},{2,13},{3,7},{3,8},{3,10},{3,14},{4,5},{4,7},{4,8},{5,10},{5,13},{6,8},{6,11},{6,14},{7,15},{8,12},{9,13},{9,14},{9,15},{11,12},{11,15},{12,15}}

Cousin 1389: {{1,8},{1,9},{1,10},{1,11},{2,6},{2,7},{2,12},{2,13},{3,6},{3,7},{3,8},{3,9},{3,10},{4,7},{4,8},{4,10},{4,13},{5,7},{5,9},{5,11},{5,12},{6,8},{6,9},{6,11},{8,12},{9,13},{10,13},{11,12}}

Cousin 1390: {{1,8},{1,9},{1,10},{1,11},{2,5},{2,7},{2,12},{2,13},{3,5},{3,7},{3,8},{4,7},{4,9},{4,11},{4,12},{5,9},{5,10},{6,11},{6,13},{6,14},{7,15},{8,12},{8,14},{9,13},{9,15},{10,14},{10,15},{14,15}}

Cousin 1391: {{1,8},{1,9},{1,10},{1,11},{2,5},{2,7},{2,12},{2,13},{3,6},{3,7},{3,9},{3,10},{4,7},{4,9},{4,11},{4,12},{5,7},{5,8},{5,9},{5,10},{6,8},{6,10},{6,11},{6,13},{7,8},{8,12},{9,13},{11,13}}

Cousin 1392: {{1,8},{1,9},{1,10},{1,11},{2,5},{2,7},{2,12},{2,13},{3,6},{3,7},{3,9},{3,10},{4,7},{4,9},{4,11},{4,12},{5,7},{5,8},{5,9},{5,10},{6,8},{6,11},{6,13},{7,8},{8,12},{9,13},{11,12},{11,13}}

Cousin 1393: {{1,8},{1,9},{1,10},{1,11},{2,5},{2,6},{2,7},{2,9},{2,12},{3,7},{3,9},{3,11},{3,12},{4,7},{4,8},{4,10},{4,13},{5,7},{5,8},{5,9},{5,10},{6,8},{6,11},{6,13},{8,12},{9,13},{10,13},{11,12}}

Cousin 1394: {{1,8},{1,9},{1,10},{1,11},{2,4},{2,7},{2,12},{2,13},{3,4},{3,7},{3,8},{4,9},{4,11},{5,7},{5,9},{5,10},{5,12},{6,11},{6,13},{6,14},{7,15},{8,12},{8,14},{9,13},{9,15},{10,14},{10,15},{14,15}}

Cousin 1395: {{1,8},{1,9},{1,10},{1,11},{2,4},{2,7},{2,12},{2,13},{3,6},{3,7},{3,9},{3,10},{4,7},{4,8},{4,9},{4,11},{5,7},{5,9},{5,10},{5,12},{6,8},{6,10},{6,11},{6,13},{7,8},{8,12},{9,13},{11,13}}

Cousin 1396: {{1,8},{1,9},{1,10},{1,11},{2,4},{2,5},{2,12},{2,13},{3,6},{3,7},{3,8},{3,10},{4,7},{4,8},{4,9},{4,11},{5,7},{5,8},{5,9},{5,10},{6,9},{6,10},{6,11},{6,12},{7,13},{8,12},{9,13},{11,12}}

Cousin 1397: {{1,3},{1,6},{1,8},{2,13},{2,14},{2,15},{3,7},{3,9},{3,10},{4,7},{4,9},{4,11},{4,13},{5,7},{5,9},{5,10},{5,14},{6,12},{6,13},{7,8},{7,15},{8,11},{8,14},{9,12},{9,15},{10,11},{10,12},{11,12}}

Cousin 1398: {{1,10},{1,11},{1,12},{2,3},{2,6},{2,8},{3,7},{3,9},{3,10},{4,7},{4,9},{4,11},{4,13},{5,7},{5,9},{5,10},{5,14},{6,12},{6,13},{7,8},{7,15},{8,11},{8,14},{9,12},{9,15},{13,14},{13,15},{14,15}}

Cousin 1399: {{1,10},{1,11},{1,12},{2,13},{2,14},{2,15},{3,6},{3,7},{3,9},{3,10},{4,7},{4,9},{4,11},{4,13},{5,7},{5,9},{5,10},{5,14},{6,8},{6,12},{6,13},{7,8},{7,15},{8,11},{8,14},{9,12},{9,15},{12,13}}

Cousin 1400: {{1,3},{1,7},{1,8},{2,13},{2,14},{2,15},{3,6},{3,9},{3,10},{4,7},{4,9},{4,11},{4,13},{5,7},{5,9},{5,10},{5,14},{6,8},{6,12},{6,13},{7,15},{8,11},{8,14},{9,12},{9,15},{10,11},{10,12},{11,12}}

Cousin 1401: {{1,10},{1,11},{1,12},{2,3},{2,7},{2,8},{3,6},{3,9},{3,10},{4,7},{4,9},{4,11},{4,13},{5,7},{5,9},{5,10},{5,14},{6,8},{6,12},{6,13},{7,15},{8,11},{8,14},{9,12},{9,15},{13,14},{13,15},{14,15}}

Cousin 1402: {{1,2},{1,7},{1,9},{1,13},{2,5},{2,8},{2,13},{3,6},{3,7},{3,8},{3,9},{3,10},{4,7},{4,9},{4,11},{4,13},{5,7},{5,9},{5,10},{6,8},{6,12},{6,13},{7,8},{8,11},{9,12},{10,11},{10,12},{11,12}}

Cousin 1403: {{1,3},{1,7},{1,9},{2,7},{2,9},{2,13},{2,14},{3,10},{3,15},{4,7},{4,9},{4,11},{4,13},{5,7},{5,9},{5,10},{5,14},{6,12},{6,13},{6,15},{7,8},{8,11},{8,14},{8,15},{9,12},{10,11},{10,12},{11,12}}

Cousin 1404: {{1,10},{1,11},{1,12},{2,7},{2,9},{2,13},{2,14},{3,7},{3,9},{3,10},{3,15},{4,7},{4,9},{4,11},{4,13},{5,7},{5,9},{5,10},{5,14},{6,12},{6,13},{6,15},{7,8},{8,11},{8,14},{8,15},{9,12},{10,15}}

Cousin 1405: {{1,10},{1,11},{1,12},{2,7},{2,9},{2,13},{2,14},{3,6},{3,10},{3,15},{4,7},{4,9},{4,11},{4,13},{5,7},{5,9},{5,10},{5,14},{6,7},{6,9},{7,8},{8,11},{8,14},{8,15},{9,12},{12,13},{12,15},{13,15}}

Cousin 1406: {{1,3},{1,8},{1,12},{1,13},{2,6},{2,7},{2,9},{2,13},{3,7},{3,9},{3,10},{4,7},{4,9},{4,11},{4,13},{5,6},{5,7},{5,9},{5,10},{6,8},{7,8},{7,9},{8,11},{9,12},{10,11},{10,12},{11,12},{12,13}}

Cousin 1407: {{1,4},{1,7},{1,9},{2,7},{2,9},{2,13},{2,14},{3,6},{3,9},{3,10},{3,15},{4,11},{4,13},{5,7},{5,9},{5,10},{5,14},{6,8},{6,12},{6,13},{7,15},{8,11},{8,14},{8,15},{9,12},{10,11},{10,12},{11,12}}

Cousin 1408: {{1,10},{1,11},{1,12},{2,7},{2,9},{2,13},{2,14},{3,6},{3,9},{3,10},{3,15},{4,7},{4,9},{4,11},{4,13},{5,7},{5,9},{5,10},{5,14},{6,8},{6,12},{6,13},{7,15},{8,11},{8,14},{8,15},{9,12},{11,13}}

Cousin 1409: {{1,5},{1,7},{1,9},{2,7},{2,9},{2,13},{2,14},{3,6},{3,9},{3,10},{3,15},{4,7},{4,9},{4,11},{4,13},{5,10},{5,14},{6,8},{6,12},{6,13},{7,15},{8,11},{8,14},{8,15},{9,12},{10,11},{10,12},{11,12}}

Cousin 1410: {{1,10},{1,11},{1,12},{2,7},{2,9},{2,13},{2,14},{3,6},{3,9},{3,10},{3,15},{4,7},{4,9},{4,11},{4,13},{5,7},{5,9},{5,10},{5,14},{6,8},{6,12},{6,13},{7,15},{8,11},{8,14},{8,15},{9,12},{10,14}}

Cousin 1411: {{1,7},{1,9},{1,11},{1,13},{2,4},{2,7},{2,9},{2,13},{3,6},{3,7},{3,8},{3,9},{3,10},{4,5},{4,8},{5,7},{5,9},{5,10},{6,8},{6,12},{6,13},{7,8},{8,11},{9,12},{10,11},{10,12},{11,12},{11,13}}

Cousin 1412: {{1,5},{1,7},{1,9},{1,10},{2,5},{2,7},{2,9},{2,13},{3,6},{3,7},{3,8},{3,9},{3,10},{4,7},{4,9},{4,11},{4,13},{5,8},{5,10},{6,8},{6,12},{6,13},{7,8},{8,11},{9,12},{10,11},{10,12},{11,12}}

Cousin 1413: {{1,10},{1,11},{1,12},{2,13},{2,14},{2,15},{3,10},{3,16},{3,17},{4,7},{4,9},{4,11},{4,13},{5,7},{5,8},{5,10},{5,14},{6,12},{6,13},{6,16},{7,15},{7,17},{8,11},{8,15},{8,16},{9,12},{9,14},{9,17}}

Cousin 1414: {{1,10},{1,11},{1,12},{2,13},{2,14},{2,15},{3,7},{3,9},{3,10},{3,16},{4,11},{4,13},{4,17},{5,7},{5,8},{5,10},{5,14},{6,12},{6,13},{6,16},{7,15},{7,17},{8,11},{8,15},{8,16},{9,12},{9,14},{9,17}}

Cousin 1415: {{1,3},{1,6},{1,8},{2,13},{2,14},{2,15},{3,7},{3,9},{3,10},{4,7},{4,9},{4,11},{4,13},{5,7},{5,8},{5,10},{5,14},{6,12},{6,13},{7,9},{7,15},{8,11},{8,15},{9,12},{9,14},{10,11},{10,12},{11,12}}

Cousin 1416: {{1,10},{1,11},{1,12},{2,3},{2,6},{2,8},{3,7},{3,9},{3,10},{4,7},{4,9},{4,11},{4,13},{5,7},{5,8},{5,10},{5,14},{6,12},{6,13},{7,9},{7,15},{8,11},{8,15},{9,12},{9,14},{13,14},{13,15},{14,15}}

Cousin 1417: {{1,10},{1,11},{1,12},{2,13},{2,14},{2,15},{3,6},{3,7},{3,9},{3,10},{4,7},{4,9},{4,11},{4,13},{5,7},{5,8},{5,10},{5,14},{6,8},{6,12},{6,13},{7,9},{7,15},{8,11},{8,15},{9,12},{9,14},{12,13}}

Cousin 1418: {{1,3},{1,7},{1,9},{2,13},{2,14},{2,15},{3,6},{3,8},{3,10},{4,7},{4,9},{4,11},{4,13},{5,7},{5,8},{5,10},{5,14},{6,8},{6,12},{6,13},{7,15},{8,11},{8,15},{9,12},{9,14},{10,11},{10,12},{11,12}}

Cousin 1419: {{1,10},{1,11},{1,12},{2,3},{2,7},{2,9},{3,6},{3,8},{3,10},{4,7},{4,9},{4,11},{4,13},{5,7},{5,8},{5,10},{5,14},{6,8},{6,12},{6,13},{7,15},{8,11},{8,15},{9,12},{9,14},{13,14},{13,15},{14,15}}

Cousin 1420: {{1,4},{1,7},{1,9},{2,13},{2,14},{2,15},{3,6},{3,7},{3,8},{3,9},{3,10},{4,11},{4,13},{5,7},{5,8},{5,10},{5,14},{6,8},{6,12},{6,13},{7,15},{8,11},{8,15},{9,12},{9,14},{10,11},{10,12},{11,12}}

Cousin 1421: {{1,10},{1,11},{1,12},{2,4},{2,7},{2,9},{3,6},{3,7},{3,8},{3,9},{3,10},{4,11},{4,13},{5,7},{5,8},{5,10},{5,14},{6,8},{6,12},{6,13},{7,15},{8,11},{8,15},{9,12},{9,14},{13,14},{13,15},{14,15}}

Cousin 1422: {{1,10},{1,11},{1,12},{2,13},{2,14},{2,15},{3,6},{3,7},{3,8},{3,9},{3,10},{4,7},{4,9},{4,11},{4,13},{5,7},{5,8},{5,10},{5,14},{6,8},{6,12},{6,13},{7,15},{8,11},{8,15},{9,12},{9,14},{11,13}}

Cousin 1423: {{1,2},{1,7},{1,8},{1,13},{2,5},{2,9},{2,13},{3,6},{3,7},{3,8},{3,9},{3,10},{4,7},{4,9},{4,11},{4,13},{5,7},{5,8},{5,10},{6,8},{6,12},{6,13},{7,9},{8,11},{9,12},{10,11},{10,12},{11,12}}

Cousin 1424: {{1,3},{1,7},{1,9},{2,7},{2,8},{2,13},{2,14},{3,10},{3,15},{4,7},{4,9},{4,11},{4,13},{5,7},{5,8},{5,10},{5,14},{6,12},{6,13},{6,15},{7,8},{8,11},{8,15},{9,12},{9,14},{10,11},{10,12},{11,12}}

Cousin 1425: {{1,10},{1,11},{1,12},{2,7},{2,8},{2,13},{2,14},{3,7},{3,9},{3,10},{3,15},{4,7},{4,9},{4,11},{4,13},{5,7},{5,8},{5,10},{5,14},{6,12},{6,13},{6,15},{7,8},{8,11},{8,15},{9,12},{9,14},{10,15}}

Cousin 1426: {{1,10},{1,11},{1,12},{2,7},{2,8},{2,13},{2,14},{3,6},{3,10},{3,15},{4,7},{4,9},{4,11},{4,13},{5,7},{5,8},{5,10},{5,14},{6,7},{6,9},{7,8},{8,11},{8,15},{9,12},{9,14},{12,13},{12,15},{13,15}}

Cousin 1427: {{1,3},{1,8},{1,12},{1,13},{2,6},{2,7},{2,8},{2,13},{3,7},{3,9},{3,10},{4,7},{4,9},{4,11},{4,13},{5,6},{5,7},{5,8},{5,10},{6,9},{7,8},{7,9},{8,11},{9,12},{10,11},{10,12},{11,12},{12,13}}

Cousin 1428: {{1,4},{1,7},{1,9},{2,7},{2,8},{2,13},{2,14},{3,6},{3,9},{3,10},{3,15},{4,11},{4,13},{5,7},{5,8},{5,10},{5,14},{6,8},{6,12},{6,13},{7,15},{8,11},{8,15},{9,12},{9,14},{10,11},{10,12},{11,12}}

Cousin 1429: {{1,10},{1,11},{1,12},{2,7},{2,8},{2,13},{2,14},{3,6},{3,9},{3,10},{3,15},{4,7},{4,9},{4,11},{4,13},{5,7},{5,8},{5,10},{5,14},{6,8},{6,12},{6,13},{7,15},{8,11},{8,15},{9,12},{9,14},{11,13}}

Cousin 1430: {{1,5},{1,7},{1,8},{2,7},{2,8},{2,13},{2,14},{3,6},{3,8},{3,10},{3,15},{4,7},{4,9},{4,11},{4,13},{5,10},{5,14},{6,8},{6,12},{6,13},{7,15},{8,11},{9,12},{9,14},{9,15},{10,11},{10,12},{11,12}}

Cousin 1431: {{1,10},{1,11},{1,12},{2,7},{2,8},{2,13},{2,14},{3,6},{3,8},{3,10},{3,15},{4,7},{4,9},{4,11},{4,13},{5,7},{5,8},{5,10},{5,14},{6,8},{6,12},{6,13},{7,15},{8,11},{9,12},{9,14},{9,15},{10,14}}

Cousin 1432: {{1,5},{1,7},{1,8},{2,7},{2,8},{2,13},{2,14},{3,6},{3,7},{3,8},{3,9},{3,10},{4,11},{4,13},{4,15},{5,10},{5,14},{6,8},{6,12},{6,13},{7,15},{8,11},{9,12},{9,14},{9,15},{10,11},{10,12},{11,12}}

Cousin 1433: {{1,10},{1,11},{1,12},{2,7},{2,8},{2,13},{2,14},{3,6},{3,7},{3,8},{3,9},{3,10},{4,5},{4,7},{4,8},{5,10},{5,14},{6,8},{6,12},{6,13},{7,15},{8,11},{9,12},{9,14},{9,15},{11,13},{11,15},{13,15}}

Cousin 1434: {{1,10},{1,11},{1,12},{2,7},{2,8},{2,13},{2,14},{3,6},{3,7},{3,8},{3,9},{3,10},{4,11},{4,13},{4,15},{5,7},{5,8},{5,10},{5,14},{6,8},{6,12},{6,13},{7,15},{8,11},{9,12},{9,14},{9,15},{10,14}}

Cousin 1435: {{1,7},{1,9},{1,11},{1,13},{2,4},{2,7},{2,8},{2,13},{3,6},{3,7},{3,8},{3,9},{3,10},{4,5},{4,9},{5,7},{5,8},{5,10},{6,8},{6,12},{6,13},{7,8},{8,11},{9,12},{10,11},{10,12},{11,12},{11,13}}

Cousin 1436: {{1,5},{1,7},{1,8},{1,10},{2,5},{2,7},{2,8},{2,13},{3,6},{3,7},{3,8},{3,9},{3,10},{4,7},{4,9},{4,11},{4,13},{5,9},{5,10},{6,8},{6,12},{6,13},{7,9},{8,11},{9,12},{10,11},{10,12},{11,12}}

Cousin 1437: {{1,3},{1,7},{1,9},{2,5},{2,9},{2,13},{2,14},{3,10},{3,15},{4,7},{4,9},{4,11},{4,13},{5,7},{5,8},{5,9},{5,10},{6,12},{6,13},{6,15},{7,14},{8,11},{8,14},{8,15},{9,12},{10,11},{10,12},{11,12}}

Cousin 1438: {{1,10},{1,11},{1,12},{2,5},{2,9},{2,13},{2,14},{3,7},{3,9},{3,10},{3,15},{4,7},{4,9},{4,11},{4,13},{5,7},{5,8},{5,9},{5,10},{6,12},{6,13},{6,15},{7,14},{8,11},{8,14},{8,15},{9,12},{10,15}}

Cousin 1439: {{1,10},{1,11},{1,12},{2,5},{2,9},{2,13},{2,14},{3,6},{3,10},{3,15},{4,7},{4,9},{4,11},{4,13},{5,7},{5,8},{5,9},{5,10},{6,7},{6,9},{7,14},{8,11},{8,14},{8,15},{9,12},{12,13},{12,15},{13,15}}

Cousin 1440: {{1,4},{1,7},{1,9},{2,5},{2,9},{2,13},{2,14},{3,7},{3,9},{3,10},{3,15},{4,11},{4,13},{5,7},{5,8},{5,9},{5,10},{6,12},{6,13},{6,15},{7,14},{8,11},{8,14},{8,15},{9,12},{10,11},{10,12},{11,12}}

Cousin 1441: {{1,10},{1,11},{1,12},{2,5},{2,9},{2,13},{2,14},{3,7},{3,9},{3,10},{3,15},{4,7},{4,9},{4,11},{4,13},{5,7},{5,8},{5,9},{5,10},{6,12},{6,13},{6,15},{7,14},{8,11},{8,14},{8,15},{9,12},{11,13}}

Cousin 1442: {{1,10},{1,11},{1,12},{2,5},{2,9},{2,13},{2,14},{3,7},{3,9},{3,10},{3,15},{4,6},{4,11},{4,13},{5,7},{5,8},{5,9},{5,10},{6,7},{6,9},{7,14},{8,11},{8,14},

{8,15},{9,12},{12,13},{12,15},{13,15}}

Cousin 1443: {{1,5},{1,7},{1,9},{2,5},{2,9},{2,13},{2,14},{3,7},{3,9},{3,10},{3,15},{4,7},{4,9},{4,11},{4,13},{5,8},{5,10},{6,12},{6,13},{6,15},{7,14},{8,11},{8,14},{8,15},{9,12},{10,11},{10,12},{11,12}}

Cousin 1444: {{1,10},{1,11},{1,12},{2,5},{2,9},{2,13},{2,14},{3,7},{3,9},{3,10},{3,15},{4,7},{4,9},{4,11},{4,13},{5,6},{5,8},{5,10},{6,7},{6,9},{7,14},{8,11},{8,14},{8,15},{9,12},{12,13},{12,15},{13,15}}

Cousin 1445: {{1,3},{1,8},{1,12},{1,13},{2,5},{2,6},{2,9},{2,13},{3,7},{3,9},{3,10},{4,7},{4,9},{4,11},{4,13},{5,7},{5,8},{5,9},{5,10},{6,7},{6,8},{7,9},{8,11},{9,12},{10,11},{10,12},{11,12},{12,13}}

Cousin 1446: {{1,7},{1,9},{1,11},{1,13},{2,4},{2,5},{2,9},{2,13},{3,6},{3,7},{3,8},{3,9},{3,10},{4,7},{4,8},{5,7},{5,8},{5,9},{5,10},{6,8},{6,12},{6,13},{8,11},{9,12},{10,11},{10,12},{11,12},{11,13}}

Cousin 1447: {{1,3},{1,8},{1,12},{1,13},{2,5},{2,6},{2,8},{2,13},{3,7},{3,9},{3,10},{4,7},{4,9},{4,11},{4,13},{5,7},{5,8},{5,9},{5,10},{6,7},{6,9},{7,8},{8,11},{9,12},{10,11},{10,12},{11,12},{12,13}}

Cousin 1448: {{1,3},{1,7},{1,9},{1,10},{2,5},{2,7},{2,8},{2,9},{2,13},{3,6},{3,8},{3,10},{4,7},{4,9},{4,11},{4,13},{5,7},{5,8},{5,9},{5,10},{6,12},{6,13},{7,8},{8,11},{9,12},{10,11},{10,12},{11,12}}

Cousin 1449: {{1,3},{1,7},{1,9},{2,5},{2,7},{2,8},{2,9},{2,13},{3,6},{3,10},{4,7},{4,9},{4,11},{4,13},{5,7},{5,8},{5,9},{5,10},{6,8},{6,12},{6,13},{7,8},{8,11},{9,12},{10,11},{10,12},{11,12},{12,13}}

Cousin 1450: {{1,10},{1,11},{1,12},{2,5},{2,7},{2,8},{2,9},{2,13},{3,6},{3,7},{3,9},{3,10},{4,7},{4,9},{4,11},{4,13},{5,7},{5,8},{5,9},{5,10},{6,8},{6,10},{6,12},{6,13},{7,8},{8,11},{9,12},{12,13}}

Cousin 1451: {{1,7},{1,9},{1,11},{1,13},{2,5},{2,7},{2,8},{2,9},{2,13},{3,4},{3,6},{3,9},{3,10},{4,7},{4,8},{5,7},{5,8},{5,9},{5,10},{6,8},{6,12},{6,13},{8,11},{9,12},{10,11},{10,12},{11,12},{11,13}}

Cousin 1452: {{1,5},{1,7},{1,8},{2,5},{2,7},{2,8},{2,9},{2,13},{3,6},{3,7},{3,8},{3,9},{3,10},{4,7},{4,9},{4,11},{4,13},{5,9},{5,10},{6,8},{6,12},{6,13},{8,11},{9,12},{10,11},{10,12},{11,12},{11,13}}

Cousin 1453: {{1,3},{1,7},{1,9},{2,6},{2,9},{2,13},{2,14},{3,10},{3,15},{4,6},{4,9},{4,11},{4,13},{5,7},{5,9},{5,10},{5,14},{6,12},{6,15},{7,8},{7,13},{8,11},{8,14},{8,15},{9,12},{10,11},{10,12},{11,12}}

Cousin 1454: {{1,10},{1,11},{1,12},{2,6},{2,9},{2,13},{2,14},{3,7},{3,9},{3,10},{3,15},{4,6},{4,9},{4,11},{4,13},{5,7},{5,9},{5,10},{5,14},{6,12},{6,15},{7,8},{7,13},{8,11},{8,14},{8,15},{9,12},{10,15}}

Cousin 1455: {{1,3},{1,7},{1,8},{2,13},{2,14},{2,15},{3,6},{3,9},{3,10},{4,6},{4,9},{4,11},{4,13},{5,7},{5,8},{5,10},{5,14},{6,12},{6,15},{7,9},{7,13},{8,11},{8,15},{9,12},{9,14},{10,11},{10,12},{11,12}}

Cousin 1456: {{1,10},{1,11},{1,12},{2,3},{2,7},{2,8},{3,6},{3,9},{3,10},{4,6},{4,9},{4,11},{4,13},{5,7},{5,8},{5,10},{5,14},{6,12},{6,15},{7,9},{7,13},{8,11},{8,15},{9,12},{9,14},{13,14},{13,15},{14,15}}

Cousin 1457: {{1,3},{1,7},{1,9},{2,13},{2,14},{2,15},{3,6},{3,8},{3,10},{4,6},{4,9},{4,11},{4,13},{5,7},{5,8},{5,10},{5,14},{6,12},{6,15},{7,8},{7,13},{8,11},{8,15},{9,12},{9,14},{10,11},{10,12},{11,12}}

Cousin 1458: {{1,10},{1,11},{1,12},{2,3},{2,7},{2,9},{3,6},{3,8},{3,10},{4,6},{4,9},{4,11},{4,13},{5,7},{5,8},{5,10},{5,14},{6,12},{6,15},{7,8},{7,13},{8,11},{8,15},{9,12},{9,14},{13,14},{13,15},{14,15}}

Cousin 1459: {{1,2},{1,6},{1,8},{1,13},{2,5},{2,9},{2,13},{3,6},{3,7},{3,8},{3,9},{3,10},{4,6},{4,9},{4,11},{4,13},{5,7},{5,8},{5,10},{6,12},{7,8},{7,9},{7,13},{8,11},{9,12},{10,11},{10,12},{11,12}}

Cousin 1460: {{1,3},{1,7},{1,9},{2,6},{2,8},{2,13},{2,14},{3,10},{3,15},{4,6},{4,9},{4,11},{4,13},{5,7},{5,8},{5,10},{5,14},{6,12},{6,15},{7,8},{7,13},{8,11},{8,15},{9,12},{9,14},{10,11},{10,12},{11,12}}

Cousin 1461: {{1,10},{1,11},{1,12},{2,6},{2,8},{2,13},{2,14},{3,7},{3,9},{3,10},{3,15},{4,6},{4,9},{4,11},{4,13},{5,7},{5,8},{5,10},{5,14},{6,12},{6,15},{7,8},{7,13},{8,11},{8,15},{9,12},{9,14},{10,15}}

Cousin 1462: {{1,3},{1,7},{1,9},{1,10},{2,5},{2,6},{2,8},{2,9},{2,13},{3,6},{3,8},{3,10},{4,6},{4,9},{4,11},{4,13},{5,7},{5,8},{5,9},{5,10},{6,12},{7,8},{7,13},{8,11},{9,12},{10,11},{10,12},{11,12}}

Cousin 1463: {{1,3},{1,7},{1,9},{2,6},{2,7},{2,13},{2,14},{3,10},{3,15},{4,6},{4,7},{4,11},{4,13},{5,7},{5,9},{5,10},{5,14},{6,12},{6,15},{7,8},{8,11},{8,14},{8,15},{9,12},{9,13},{10,11},{10,12},{11,12}}

Cousin 1464: {{1,10},{1,11},{1,12},{2,6},{2,7},{2,13},{2,14},{3,7},{3,9},{3,10},{3,15},{4,6},{4,7},{4,11},{4,13},{5,7},{5,9},{5,10},{5,14},{6,12},{6,15},{7,8},{8,11},{8,14},{8,15},{9,12},{9,13},{10,15}}

Cousin 1465: {{1,5},{1,7},{1,9},{2,6},{2,7},{2,13},{2,14},{3,7},{3,9},{3,10},{3,15},{4,6},{4,7},{4,11},{4,13},{5,10},{5,14},{6,12},{6,15},{7,8},{8,11},{8,14},{8,15},{9,12},{9,13},{10,11},{10,12},{11,12}}

Cousin 1466: {{1,10},{1,11},{1,12},{2,6},{2,7},{2,13},{2,14},{3,7},{3,9},{3,10},{3,15},{4,6},{4,7},{4,11},{4,13},{5,7},{5,9},{5,10},{5,14},{6,12},{6,15},{7,8},{8,11},{8,14},{8,15},{9,12},{9,13},{10,14}}

Cousin 1467: {{1,5},{1,7},{1,9},{1,10},{2,5},{2,6},{2,7},{2,13},{3,6},{3,7},{3,8},{3,9},{3,10},{4,6},{4,7},{4,11},{4,13},{5,8},{5,10},{6,8},{6,12},{7,8},{8,11},{9,12},{9,13},{10,11},{10,12},{11,12}}

Cousin 1468: {{1,5},{1,7},{1,9},{2,5},{2,7},{2,13},{2,14},{3,6},{3,9},{3,10},{3,15},{4,6},{4,7},{4,11},{4,13},{5,8},{5,10},{6,12},{6,14},{7,15},{8,11},{8,14},{8,15},{9,12},{9,13},{10,11},{10,12},{11,12}}

Cousin 1469: {{1,5},{1,7},{1,8},{2,5},{2,7},{2,13},{2,14},{3,6},{3,8},{3,10},{3,15},{4,6},{4,7},{4,11},{4,13},{5,9},{5,10},{6,12},{6,14},{7,15},{8,11},{8,14},{9,12},{9,13},{9,15},{10,11},{10,12},{11,12}}

Cousin 1470: {{1,3},{1,7},{1,9},{2,5},{2,6},{2,13},{2,14},{3,10},{3,15},{4,6},{4,7},{4,11},{4,13},{5,7},{5,8},{5,9},{5,10},{6,12},{6,15},{7,14},{8,11},{8,14},{8,15},{9,12},{9,13},{10,11},{10,12},{11,12}}

Cousin 1471: {{1,10},{1,11},{1,12},{2,5},{2,6},{2,13},{2,14},{3,7},{3,9},{3,10},{3,15},{4,6},{4,7},{4,11},{4,13},{5,7},{5,8},{5,9},{5,10},{6,12},{6,15},{7,14},{8,11},{8,14},{8,15},{9,12},{9,13},{10,15}}

Cousin 1472: {{1,5},{1,7},{1,9},{2,5},{2,6},{2,13},{2,14},{3,7},{3,9},{3,10},{3,15},{4,6},{4,7},{4,11},{4,13},{5,8},{5,10},{6,12},{6,15},{7,14},{8,11},{8,14},{8,15},{9,12},{9,13},{10,11},{10,12},{11,12}}

Cousin 1473: {{1,5},{1,7},{1,8},{2,5},{2,6},{2,7},{2,8},{2,13},{3,10},{3,14},{3,15},{4,6},{4,7},{4,11},{4,13},{5,9},{5,10},{6,12},{6,14},{7,15},{8,11},{8,14},{9,12},{9,13},{9,15},{10,11},{10,12},{11,12}}

Cousin 1474: {{1,10},{1,11},{1,12},{2,5},{2,6},{2,7},{2,8},{2,13},{3,5},{3,7},{3,8},{4,6},{4,7},{4,11},{4,13},{5,9},{5,10},{6,12},{6,14},{7,15},{8,11},{8,14},{9,12},{9,13},{9,15},{10,14},{10,15},{14,15}}

Cousin 1475: {{1,3},{1,7},{1,9},{1,10},{2,5},{2,6},{2,7},{2,8},{2,13},{3,6},{3,8},{3,10},{4,6},{4,7},{4,11},{4,13},{5,7},{5,8},{5,9},{5,10},{6,12},{7,8},{8,11},{9,12},{9,13},{10,11},{10,12},{11,12}}

Cousin 1476: {{1,3},{1,7},{1,9},{1,10},{2,4},{2,6},{2,7},{2,9},{2,13},{3,6},{3,8},{3,10},{4,6},{4,7},{4,9},{4,11},{5,7},{5,9},{5,10},{5,13},{6,12},{7,8},{8,11},{8,13},{9,12},{10,11},{10,12},{11,12}}

Cousin 1477: {{1,7},{1,9},{1,10},{1,13},{2,4},{2,6},{2,7},{2,9},{2,13},{3,5},{3,7},{3,9},{3,10},{4,6},{4,7},{4,9},{4,11},{5,6},{5,8},{6,12},{7,8},{8,11},{8,13},{9,12},{10,11},{10,12},{10,13},{11,12}}

Cousin 1478: {{1,4},{1,7},{1,9},{2,4},{2,7},{2,13},{2,14},{3,6},{3,9},{3,10},{3,15},{4,6},{4,11},{5,7},{5,8},{5,10},{5,13},{6,12},{6,14},{7,15},{8,11},{8,14},{8,15},{9,12},{9,13},{10,11},{10,12},{11,12}}

Cousin 1479: {{1,5},{1,7},{1,8},{2,4},{2,7},{2,13},{2,14},{3,6},{3,8},{3,10},{3,15},{4,6},{4,7},{4,9},{4,11},{5,10},{5,13},{6,12},{6,14},{7,15},{8,11},{8,14},{9,12},{9,13},{9,15},{10,11},{10,12},{11,12}}

Cousin 1480: {{1,10},{1,11},{1,12},{2,4},{2,7},{2,13},{2,14},{3,6},{3,8},{3,10},{3,15},{4,6},{4,7},{4,9},{4,11},{5,7},{5,8},{5,10},{5,13},{6,12},{6,14},{7,15},{8,11},{8,14},{9,12},{9,13},{9,15},{10,13}}

Cousin 1481: {{1,5},{1,7},{1,8},{2,4},{2,7},{2,13},{2,14},{3,6},{3,7},{3,8},{3,9},{3,10},{4,6},{4,11},{4,15},{5,10},{5,13},{6,12},{6,14},{7,15},{8,11},{8,14},{9,12},{9,13},{9,15},{10,11},{10,12},{11,12}}

Cousin 1482: {{1,7},{1,8},{1,10},{1,13},{2,4},{2,5},{2,7},{2,13},{3,6},{3,7},{3,8},{3,9},{3,10},{4,6},{4,7},{4,9},{4,11},{5,6},{5,8},{6,12},{7,9},{8,11},{9,12},{9,13},{10,11},{10,12},{10,13},{11,12}}

Cousin 1483: {{1,3},{1,7},{1,9},{2,4},{2,6},{2,13},{2,14},{3,10},{3,15},{4,6},{4,7},{4,9},{4,11},{5,7},{5,8},{5,10},{5,13},{6,12},{6,15},{7,14},{8,11},{8,14},{8,15},{9,12},{9,13},{10,11},{10,12},{11,12}}

Cousin 1484: {{1,10},{1,11},{1,12},{2,4},{2,6},{2,13},{2,14},{3,7},{3,9},{3,10},{3,15},{4,6},{4,7},{4,9},{4,11},{5,7},{5,8},{5,10},{5,13},{6,12},{6,15},{7,14},{8,11},{8,14},{8,15},{9,12},{9,13},{10,15}}

Cousin 1485: {{1,4},{1,7},{1,9},{2,4},{2,6},{2,13},{2,14},{3,7},{3,9},{3,10},{3,15},{4,6},{4,11},{5,7},{5,8},{5,10},{5,13},{6,12},{6,15},{7,14},{8,11},{8,14},{8,15},{9,12},{9,13},{10,11},{10,12},{11,12}}

Cousin 1486: {{1,5},{1,7},{1,8},{2,4},{2,6},{2,7},{2,8},{2,13},{3,10},{3,14},{3,15},{4,6},{4,7},{4,9},{4,11},{5,10},{5,13},{6,12},{6,14},{7,15},{8,11},{8,14},{9,12},{9,13},{9,15},{10,11},{10,12},{11,12}}

Cousin 1487: {{1,10},{1,11},{1,12},{2,4},{2,6},{2,7},{2,8},{2,13},{3,5},{3,7},{3,8},{4,6},{4,7},{4,9},{4,11},{5,10},{5,13},{6,12},{6,14},{7,15},{8,11},{8,14},{9,12},{9,13},{9,15},{10,14},{10,15},{14,15}}

Cousin 1488: {{1,3},{1,7},{1,9},{1,10},{2,4},{2,6},{2,7},{2,8},{2,13},{3,6},{3,8},{3,10},{4,6},{4,7},{4,9},{4,11},{5,7},{5,8},{5,10},{5,13},{6,12},{7,8},{8,11},{9,12},{9,13},{10,11},{10,12},{11,12}}

Cousin 1489: {{1,7},{1,8},{1,10},{1,13},{2,4},{2,6},{2,7},{2,8},{2,13},{3,5},{3,7},{3,9},{3,10},{4,6},{4,7},{4,9},{4,11},{5,6},{5,8},{6,12},{7,9},{8,11},{9,12},{9,13},{10,11},{10,12},{10,13},{11,12}}

Cousin 1490: {{1,3},{1,7},{1,9},{1,10},{2,4},{2,5},{2,6},{2,9},{2,13},{3,6},{3,8},{3,10},{4,6},{4,7},{4,9},{4,11},{5,7},{5,8},{5,9},{5,10},{6,12},{7,13},{8,11},{8,13},{9,12},{10,11},{10,12},{11,12}}

Cousin 1491: {{1,5},{1,7},{1,8},{2,4},{2,5},{2,6},{2,7},{2,8},{2,9},{3,7},{3,9},{3,10},{3,13},{4,6},{4,7},{4,9},{4,11},{5,9},{5,10},{6,12},{6,13},{8,11},{8,13},{9,12},{10,11},{10,12},{10,13},{11,12}}

Cousin 1492: {{1,6},{1,9},{1,10},{1,11},{2,7},{2,9},{2,12},{2,13},{3,4},{3,7},{3,9},{4,11},{4,12},{5,7},{5,9},{5,10},{5,13},{6,8},{6,12},{6,14},{7,15},{8,11},{8,13},{8,15},{9,14},{10,14},{10,15},{14,15}}



Cousin 1493: {{1,6},{1,9},{1,10},{1,11},{2,7},{2,9},{2,12},{2,13},{3,10},{3,14},{3,15},{4,7},{4,9},{4,11},{4,12},{5,7},{5,9},{5,10},{5,13},{6,8},{6,12},{6,14},{7,15},{8,11},{8,13},{8,15},{9,14},{11,12}}

Cousin 1494: {{1,6},{1,9},{1,10},{1,11},{2,5},{2,7},{2,8},{2,9},{2,12},{3,7},{3,9},{3,11},{3,12},{4,7},{4,8},{4,10},{4,13},{5,7},{5,8},{5,9},{5,10},{6,8},{6,12},{6,13},{8,11},{9,13},{10,13},{11,12}}

Cousin 1495: {{1,6},{1,9},{1,10},{1,11},{2,5},{2,7},{2,12},{2,13},{3,5},{3,7},{3,9},{4,6},{4,7},{4,11},{4,12},{5,8},{5,10},{6,13},{6,14},{7,15},{8,11},{8,13},{8,15},{9,12},{9,14},{10,14},{10,15},{14,15}}

Cousin 1496: {{1,6},{1,9},{1,10},{1,11},{2,4},{2,7},{2,12},{2,13},{3,4},{3,7},{3,9},{4,6},{4,11},{5,7},{5,8},{5,10},{5,12},{6,13},{6,14},{7,15},{8,11},{8,13},{8,15},{9,12},{9,14},{10,14},{10,15},{14,15}}

Cousin 1497: {{1,6},{1,9},{1,10},{1,11},{2,4},{2,6},{2,12},{2,13},{3,4},{3,6},{3,9},{4,7},{4,11},{5,7},{5,8},{5,10},{5,12},{6,14},{7,13},{7,15},{8,11},{8,13},{8,14},{9,12},{9,15},{10,14},{10,15},{14,15}}

Cousin 1498: {{1,8},{1,9},{1,10},{1,11},{2,3},{2,7},{2,9},{2,10},{3,6},{3,8},{3,10},{4,8},{4,9},{4,11},{4,12},{5,7},{5,9},{5,10},{5,13},{6,11},{6,14},{7,8},{7,12},{8,13},{9,14},{12,13},{12,14},{13,14}}

Cousin 1499: {{1,8},{1,9},{1,10},{1,11},{2,3},{2,7},{2,9},{3,6},{3,10},{4,8},{4,9},{4,11},{4,12},{5,7},{5,9},{5,10},{5,13},{6,8},{6,11},{6,14},{7,8},{7,12},{8,13},{9,14},{11,14},{12,13},{12,14},{13,14}}

Cousin 1500: {{1,8},{1,9},{1,10},{1,11},{2,7},{2,9},{2,10},{2,13},{3,5},{3,7},{3,9},{3,10},{4,8},{4,9},{4,11},{4,12},{5,6},{5,8},{6,11},{6,14},{7,8},{7,12},{8,13},{9,14},{10,13},{12,13},{12,14},{13,14}}

Cousin 1501: {{1,8},{1,9},{1,10},{1,11},{2,5},{2,7},{2,9},{3,6},{3,7},{3,9},{3,10},{4,8},{4,9},{4,11},{4,12},{5,10},{5,13},{6,8},{6,11},{6,14},{7,8},{7,12},{8,13},{9,14},{11,14},{12,13},{12,14},{13,14}}

Cousin 1502: {{1,8},{1,9},{1,10},{1,11},{2,12},{2,13},{2,14},{3,6},{3,7},{3,9},{3,10},{4,8},{4,9},{4,11},{4,12},{5,7},{5,9},{5,10},{5,13},{6,8},{6,11},{6,14},{7,8},{7,12},{8,13},{9,14},{10,13},{11,14}}

Cousin 1503: {{1,8},{1,9},{1,10},{1,11},{2,7},{2,9},{2,10},{2,13},{3,5},{3,6},{3,9},{3,10},{4,8},{4,9},{4,11},{4,12},{5,7},{5,8},{6,8},{6,11},{6,14},{7,12},{8,13},{9,14},{10,13},{12,13},{12,14},{13,14}}

Cousin 1504: {{1,8},{1,9},{1,10},{1,11},{2,5},{2,7},{2,9},{2,12},{3,6},{3,7},{3,9},{3,10},{4,8},{4,9},{4,11},{4,12},{5,10},{5,13},{6,8},{6,11},{6,14},{7,8},{7,12},{8,13},{9,14},{12,13},{12,14},{13,14}}

Cousin 1505: {{1,8},{1,9},{1,10},{1,11},{2,12},{2,13},{2,14},{3,6},{3,7},{3,9},{3,10},{4,8},{4,9},{4,11},{4,12},{5,7},{5,9},{5,10},{5,12},{5,13},{6,8},{6,11},{6,14},{7,8},{7,12},{8,13},{9,14},{10,13}}

Cousin 1506: {{1,8},{1,9},{1,10},{1,11},{2,6},{2,7},{2,12},{2,13},{3,7},{3,8},{3,10},{3,13},{4,7},{4,9},{4,11},{4,12},{5,7},{5,9},{5,10},{5,14},{6,9},{6,11},{6,14},{8,12},{8,14},{9,13},{10,13},{10,14}}

Cousin 1507: {{1,8},{1,9},{1,10},{1,11},{2,6},{2,7},{2,12},{2,13},{3,7},{3,9},{3,10},{3,14},{4,7},{4,8},{4,10},{4,13},{5,7},{5,9},{5,11},{5,12},{6,9},{6,11},{6,14},{8,12},{8,14},{9,13},{10,13},{11,12}}

Cousin 1508: {{1,8},{1,9},{1,10},{1,11},{2,6},{2,7},{2,12},{2,13},{3,7},{3,9},{3,11},{3,12},{4,7},{4,8},{4,10},{4,14},{5,7},{5,8},{5,10},{5,13},{6,8},{6,11},{6,14},{8,12},{9,13},{9,14},{10,14},{11,12}}

Cousin 1509: {{1,8},{1,9},{1,10},{1,11},{2,6},{2,7},{2,12},{2,13},{3,7},{3,8},{3,10},{3,14},{4,7},{4,8},{4,10},{4,13},{5,7},{5,9},{5,11},{5,12},{6,8},{6,11},{6,14},{8,12},{9,13},{9,14},{10,13},{11,12}}

Cousin 1510: {{1,8},{1,9},{1,10},{1,11},{2,5},{2,7},{2,12},{2,13},{3,5},{3,7},{3,8},{4,7},{4,9},{4,11},{4,12},{5,9},{5,10},{6,7},{6,9},{6,10},{6,14},{8,12},{8,14},{9,13},{10,14},{11,13},{11,14},{13,14}}

Cousin 1511: {{1,8},{1,9},{1,10},{1,11},{2,4},{2,7},{2,12},{2,13},{3,4},{3,7},{3,8},{4,9},{4,11},{5,7},{5,9},{5,10},{5,12},{6,7},{6,9},{6,10},{6,14},{8,12},{8,14},{9,13},{10,14},{11,13},{11,14},{13,14}}

Cousin 1512: {{1,3},{1,6},{1,8},{2,7},{2,9},{2,13},{2,14},{3,7},{3,9},{3,10},{4,7},{4,9},{4,11},{4,13},{5,7},{5,9},{5,10},{5,14},{6,12},{6,13},{7,8},{8,11},{8,14},{9,12},{10,11},{10,12},{11,12},{13,14}}

Cousin 1513: {{1,3},{1,8},{1,12},{1,13},{2,6},{2,13},{2,14},{3,7},{3,9},{3,10},{4,7},{4,9},{4,11},{4,13},{5,7},{5,9},{5,10},{5,14},{6,7},{6,9},{7,8},{8,11},{8,14},{9,12},{10,11},{10,12},{11,12},{12,13}}

Cousin 1514: {{1,10},{1,11},{1,12},{2,3},{2,8},{2,12},{2,13},{3,7},{3,9},{3,10},{4,7},{4,9},{4,11},{4,13},{5,7},{5,9},{5,10},{5,14},{6,7},{6,9},{6,13},{6,14},{7,8},{8,11},{8,14},{9,12},{12,13},{13,14}}

Cousin 1515: {{1,3},{1,7},{1,8},{2,7},{2,9},{2,13},{2,14},{3,6},{3,9},{3,10},{4,7},{4,9},{4,11},{4,13},{5,7},{5,9},{5,10},{5,14},{6,8},{6,12},{6,13},{8,11},{8,14},{9,12},{10,11},{10,12},{11,12},{13,14}}

Cousin 1516: {{1,3},{1,7},{1,9},{1,10},{2,7},{2,9},{2,13},{2,14},{3,6},{3,8},{3,10},{4,7},{4,9},{4,11},{4,13},{5,7},{5,9},{5,10},{5,14},{6,12},{6,13},{7,8},{8,11},{8,14},{9,12},{10,11},{10,12},{11,12}}

Cousin 1517: {{1,3},{1,7},{1,9},{2,7},{2,9},{2,13},{2,14},{3,6},{3,10},{4,7},{4,9},{4,11},{4,13},{5,7},{5,9},{5,10},{5,14},{6,8},{6,12},{6,13},{7,8},{8,11},{8,14},{9,12},{10,11},{10,12},{11,12},{12,13}}

Cousin 1518: {{1,10},{1,11},{1,12},{2,7},{2,9},{2,13},{2,14},{3,6},{3,7},{3,9},{3,10},{4,7},{4,9},{4,11},{4,13},{5,7},{5,9},{5,10},{5,14},{6,8},{6,10},{6,12},{6,13},{

{7,8},{8,11},{8,14},{9,12},{12,13}}

Cousin 1519: {{1,7},{1,9},{1,11},{1,13},{2,7},{2,9},{2,13},{2,14},{3,4},{3,6},{3,9},{3,10},{4,7},{4,8},{5,7},{5,9},{5,10},{5,14},{6,8},{6,12},{6,13},{8,11},{8,14},{9,12},{10,11},{10,12},{11,12},{11,13}}

Cousin 1520: {{1,7},{1,9},{1,10},{1,14},{2,7},{2,9},{2,13},{2,14},{3,5},{3,6},{3,9},{3,10},{4,7},{4,9},{4,11},{4,13},{5,7},{5,8},{6,8},{6,12},{6,13},{8,11},{8,14},{9,12},{10,11},{10,12},{10,14},{11,12}}

Cousin 1521: {{1,3},{1,7},{1,9},{2,13},{2,14},{2,15},{3,10},{3,16},{4,7},{4,9},{4,11},{4,13},{5,7},{5,8},{5,10},{5,14},{6,12},{6,13},{6,16},{7,15},{8,11},{8,15},{8,16},{9,12},{9,14},{10,11},{10,12},{11,12}}

Cousin 1522: {{1,10},{1,11},{1,12},{2,3},{2,7},{2,9},{3,10},{3,16},{4,7},{4,9},{4,11},{4,13},{5,7},{5,8},{5,10},{5,14},{6,12},{6,13},{6,16},{7,15},{8,11},{8,15},{8,16},{9,12},{9,14},{13,14},{13,15},{14,15}}

Cousin 1523: {{1,10},{1,11},{1,12},{2,13},{2,14},{2,15},{3,7},{3,9},{3,10},{3,16},{4,7},{4,9},{4,11},{4,13},{5,7},{5,8},{5,10},{5,14},{6,12},{6,13},{6,16},{7,15},{8,11},{8,15},{8,16},{9,12},{9,14},{10,16}}

Cousin 1524: {{1,10},{1,11},{1,12},{2,13},{2,14},{2,15},{3,6},{3,10},{3,16},{4,7},{4,9},{4,11},{4,13},{5,7},{5,8},{5,10},{5,14},{6,7},{6,9},{7,15},{8,11},{8,15},{8,16},{9,12},{9,14},{12,13},{12,16},{13,16}}

Cousin 1525: {{1,4},{1,7},{1,9},{2,13},{2,14},{2,15},{3,7},{3,9},{3,10},{3,16},{4,11},{4,13},{5,7},{5,8},{5,10},{5,14},{6,12},{6,13},{6,16},{7,15},{8,11},{8,15},{8,16},{9,12},{9,14},{10,11},{10,12},{11,12}}

Cousin 1526: {{1,10},{1,11},{1,12},{2,4},{2,7},{2,9},{3,7},{3,9},{3,10},{3,16},{4,11},{4,13},{5,7},{5,8},{5,10},{5,14},{6,12},{6,13},{6,16},{7,15},{8,11},{8,15},{8,16},{9,12},{9,14},{13,14},{13,15},{14,15}}

Cousin 1527: {{1,10},{1,11},{1,12},{2,13},{2,14},{2,15},{3,7},{3,9},{3,10},{3,16},{4,7},{4,9},{4,11},{4,13},{5,7},{5,8},{5,10},{5,14},{6,12},{6,13},{6,16},{7,15},{8,11},{8,15},{8,16},{9,12},{9,14},{11,13}}

Cousin 1528: {{1,10},{1,11},{1,12},{2,13},{2,14},{2,15},{3,7},{3,9},{3,10},{3,16},{4,6},{4,11},{4,13},{5,7},{5,8},{5,10},{5,14},{6,7},{6,9},{7,15},{8,11},{8,15},{8,16},{9,12},{9,14},{12,13},{12,16},{13,16}}

Cousin 1529: {{1,3},{1,6},{1,8},{2,7},{2,8},{2,13},{2,14},{3,7},{3,9},{3,10},{4,7},{4,9},{4,11},{4,13},{5,7},{5,8},{5,10},{5,14},{6,12},{6,13},{7,9},{8,11},{9,12},{9,14},{10,11},{10,12},{11,12},{13,14}}

Cousin 1530: {{1,3},{1,8},{1,12},{1,13},{2,6},{2,13},{2,14},{3,7},{3,9},{3,10},{4,7},{4,9},{4,11},{4,13},{5,7},{5,8},{5,10},{5,14},{6,7},{6,8},{7,9},{8,11},{9,12},{9,14},{10,11},{10,12},{11,12},{12,13}}

Cousin 1531: {{1,10},{1,11},{1,12},{2,3},{2,8},{2,12},{2,13},{3,7},{3,9},{3,10},{4,7},{4,9},{4,11},{4,13},{5,7},{5,8},{5,10},{5,14},{6,7},{6,8},{6,13},{6,14},{7,9},{8,11},{9,12},{9,14},{12,13},{13,14}}

Cousin 1532: {{1,3},{1,7},{1,9},{2,7},{2,8},{2,13},{2,14},{3,6},{3,8},{3,10},{4,7},{4,9},{4,11},{4,13},{5,7},{5,8},{5,10},{5,14},{6,8},{6,12},{6,13},{8,11},{9,12},{9,14},{10,11},{10,12},{11,12},{13,14}}

Cousin 1533: {{1,4},{1,7},{1,9},{2,7},{2,8},{2,13},{2,14},{3,6},{3,7},{3,8},{3,9},{3,10},{4,11},{4,13},{5,7},{5,8},{5,10},{5,14},{6,8},{6,12},{6,13},{8,11},{9,12},{9,14},{10,11},{10,12},{11,12},{13,14}}

Cousin 1534: {{1,7},{1,9},{1,11},{1,13},{2,4},{2,13},{2,14},{3,6},{3,7},{3,8},{3,9},{3,10},{4,7},{4,8},{5,7},{5,8},{5,10},{5,14},{6,8},{6,12},{6,13},{8,11},{9,12},{9,14},{10,11},{10,12},{11,12},{11,13}}

Cousin 1535: {{1,10},{1,11},{1,12},{2,7},{2,9},{2,11},{2,13},{3,6},{3,7},{3,8},{3,9},{3,10},{4,7},{4,8},{4,13},{4,14},{5,7},{5,8},{5,10},{5,14},{6,8},{6,12},{6,13},{8,11},{9,12},{9,14},{11,13},{13,14}}

Cousin 1536: {{1,3},{1,7},{1,9},{1,10},{2,7},{2,8},{2,13},{2,14},{3,6},{3,8},{3,10},{4,7},{4,9},{4,11},{4,13},{5,7},{5,8},{5,10},{5,14},{6,12},{6,13},{7,8},{8,11},{9,12},{9,14},{10,11},{10,12},{11,12}}

Cousin 1537: {{1,3},{1,7},{1,9},{2,7},{2,8},{2,13},{2,14},{3,6},{3,10},{4,7},{4,9},{4,11},{4,13},{5,7},{5,8},{5,10},{5,14},{6,8},{6,12},{6,13},{7,8},{8,11},{9,12},{9,14},{10,11},{10,12},{11,12},{12,13}}

Cousin 1538: {{1,10},{1,11},{1,12},{2,7},{2,8},{2,13},{2,14},{3,6},{3,7},{3,9},{3,10},{4,7},{4,9},{4,11},{4,13},{5,7},{5,8},{5,10},{5,14},{6,8},{6,10},{6,12},{6,13},{7,8},{8,11},{9,12},{9,14},{12,13}}

Cousin 1539: {{1,7},{1,9},{1,11},{1,13},{2,7},{2,8},{2,13},{2,14},{3,4},{3,6},{3,9},{3,10},{4,7},{4,8},{5,7},{5,8},{5,10},{5,14},{6,8},{6,12},{6,13},{8,11},{9,12},{9,14},{10,11},{10,12},{11,12},{11,13}}

Cousin 1540: {{1,7},{1,8},{1,10},{1,14},{2,7},{2,8},{2,13},{2,14},{3,5},{3,6},{3,8},{3,10},{4,7},{4,9},{4,11},{4,13},{5,7},{5,9},{6,8},{6,12},{6,13},{8,11},{9,12},{9,14},{10,11},{10,12},{10,14},{11,12}}

Cousin 1541: {{1,5},{1,7},{1,8},{2,7},{2,8},{2,13},{2,14},{3,6},{3,7},{3,8},{3,9},{3,10},{4,7},{4,9},{4,11},{4,13},{5,10},{5,14},{6,8},{6,12},{6,13},{8,11},{9,12},{9,14},{10,11},{10,12},{11,12},{11,13}}

Cousin 1542: {{1,7},{1,8},{1,10},{1,14},{2,7},{2,8},{2,13},{2,14},{3,6},{3,7},{3,8},{3,9},{3,10},{4,5},{4,11},{4,13},{5,7},{5,9},{6,8},{6,12},{6,13},{8,11},{9,12},{9,14},{10,11},{10,12},{10,14},{11,12}}

Cousin 1543: {{1,10},{1,11},{1,12},{2,7},{2,8},{2,13},{2,14},{3,6},{3,7},{3,8},{3,9},{3,10},{4,7},{4,8},{4,10},{4,14},{5,7},{5,9},{5,11},{5,13},{6,8},{6,12},{6,13},{8,11},{9,12},{9,14},{10,14},{11,13}}

Cousin 1544: {{1,3},{1,7},{1,9},{1,10},{2,5},{2,9},{2,13},{2,14},{3,6},{3,8},{3,10},{4,7},{4,9},{4,11},{4,13},{5,7},{5,8},{5,9},{5,10},{6,12},{6,13},{7,14},{8,11},{8,14},{9,12},{10,11},{10,12},{11,12}}

Cousin 1545: {{1,3},{1,7},{1,9},{2,5},{2,9},{2,13},{2,14},{3,6},{3,10},{4,7},{4,9},{4,11},{4,13},{5,7},{5,8},{5,9},{5,10},{6,8},{6,12},{6,13},{7,14},{8,11},{8,14},{9,12},{10,11},{10,12},{11,12},{12,13}}

Cousin 1546: {{1,10},{1,11},{1,12},{2,5},{2,9},{2,13},{2,14},{3,6},{3,7},{3,9},{3,10},{4,7},{4,9},{4,11},{4,13},{5,7},{5,8},{5,9},{5,10},{6,8},{6,10},{6,12},{6,13},{7,14},{8,11},{8,14},{9,12},{12,13}}

Cousin 1547: {{1,7},{1,9},{1,11},{1,13},{2,5},{2,9},{2,13},{2,14},{3,4},{3,7},{3,9},{3,10},{4,6},{4,8},{5,7},{5,8},{5,9},{5,10},{6,12},{6,13},{7,14},{8,11},{8,14},{9,12},{10,11},{10,12},{11,12},{11,13}}

Cousin 1548: {{1,4},{1,7},{1,9},{2,5},{2,9},{2,13},{2,14},{3,6},{3,7},{3,9},{3,10},{4,11},{4,13},{5,7},{5,8},{5,9},{5,10},{6,8},{6,12},{6,13},{7,14},{8,11},{8,14},{9,12},{10,11},{10,12},{11,12},{12,13}}

Cousin 1549: {{1,10},{1,11},{1,12},{2,5},{2,9},{2,13},{2,14},{3,6},{3,7},{3,9},{3,10},{4,7},{4,9},{4,11},{4,13},{5,7},{5,8},{5,9},{5,10},{6,8},{6,12},{6,13},{7,14},{8,11},{8,14},{9,12},{11,13},{12,13}}

Cousin 1550: {{1,5},{1,7},{1,9},{2,5},{2,9},{2,13},{2,14},{3,6},{3,7},{3,9},{3,10},{4,7},{4,9},{4,11},{4,13},{5,8},{5,10},{6,8},{6,12},{6,13},{7,14},{8,11},{8,14},{9,12},{10,11},{10,12},{11,12},{12,13}}

Cousin 1551: {{1,3},{1,7},{1,9},{1,10},{2,5},{2,6},{2,7},{2,8},{2,9},{3,6},{3,8},{3,10},{3,12},{4,6},{4,7},{4,9},{4,11},{5,7},{5,8},{5,9},{5,10},{6,12},{7,8},{8,11},{9,12},{10,11},{10,12},{11,12}}

Cousin 1552: {{1,3},{1,7},{1,9},{1,10},{2,6},{2,9},{2,13},{2,14},{3,6},{3,8},{3,10},{4,6},{4,9},{4,11},{4,13},{5,7},{5,9},{5,10},{5,14},{6,12},{7,8},{7,13},{8,11},{8,14},{9,12},{10,11},{10,12},{11,12}}

Cousin 1553: {{1,3},{1,7},{1,8},{2,6},{2,8},{2,13},{2,14},{3,6},{3,9},{3,10},{4,6},{4,9},{4,11},{4,13},{5,7},{5,8},{5,10},{5,14},{6,12},{7,9},{7,13},{8,11},{9,12},{9,14},{10,11},{10,12},{11,12},{13,14}}

Cousin 1554: {{1,3},{1,7},{1,9},{2,6},{2,8},{2,13},{2,14},{3,6},{3,8},{3,10},{4,6},{4,9},{4,11},{4,13},{5,7},{5,8},{5,10},{5,14},{6,12},{7,8},{7,13},{8,11},{9,12},{9,14},{10,11},{10,12},{11,12},{13,14}}

Cousin 1555: {{1,3},{1,7},{1,9},{1,10},{2,6},{2,8},{2,13},{2,14},{3,6},{3,8},{3,10},{4,6},{4,9},{4,11},{4,13},{5,7},{5,8},{5,10},{5,14},{6,12},{7,8},{7,13},{8,11},{9,12},{9,14},{10,11},{10,12},{11,12}}

Cousin 1556: {{1,3},{1,7},{1,9},{1,10},{2,6},{2,7},{2,13},{2,14},{3,6},{3,8},{3,10},{4,6},{4,7},{4,11},{4,13},{5,7},{5,9},{5,10},{5,14},{6,12},{7,8},{8,11},{8,14},{9,12},{9,13},{10,11},{10,12},{11,12}}

Cousin 1557: {{1,7},{1,9},{1,10},{1,14},{2,6},{2,7},{2,13},{2,14},{3,5},{3,7},{3,9},{3,10},{4,6},{4,7},{4,11},{4,13},{5,6},{5,8},{6,12},{7,8},{8,11},{8,14},{9,12},{9,13},{10,11},{10,12},{10,14},{11,12}}

Cousin 1558: {{1,3},{1,7},{1,9},{1,10},{2,5},{2,6},{2,13},{2,14},{3,6},{3,8},{3,10},{4,6},{4,7},{4,11},{4,13},{5,7},{5,8},{5,9},{5,10},{6,12},{7,14},{8,11},{8,14},{9,12},{9,13},{10,11},{10,12},{11,12}}

Cousin 1559: {{1,5},{1,7},{1,8},{2,5},{2,6},{2,7},{2,8},{2,13},{3,7},{3,9},{3,10},{3,14},{4,6},{4,7},{4,11},{4,13},{5,9},{5,10},{6,12},{6,14},{8,11},{8,14},{9,12},{9,13},{10,11},{10,12},{10,14},{11,12}}

Cousin 1560: {{1,7},{1,8},{1,10},{1,13},{2,4},{2,7},{2,13},{2,14},{3,5},{3,6},{3,8},{3,10},{4,6},{4,7},{4,9},{4,11},{5,7},{5,9},{6,12},{6,14},{8,11},{8,14},{9,12},{9,13},{10,11},{10,12},{10,13},{11,12}}

Cousin 1561: {{1,7},{1,8},{1,10},{1,13},{2,4},{2,7},{2,13},{2,14},{3,6},{3,7},{3,8},{3,9},{3,10},{4,5},{4,6},{4,11},{5,7},{5,9},{6,12},{6,14},{8,11},{8,14},{9,12},{9,13},{10,11},{10,12},{10,13},{11,12}}

Cousin 1562: {{1,3},{1,7},{1,9},{1,10},{2,4},{2,6},{2,13},{2,14},{3,6},{3,8},{3,10},{4,6},{4,7},{4,9},{4,11},{5,7},{5,8},{5,10},{5,13},{6,12},{7,14},{8,11},{8,14},{9,12},{9,13},{10,11},{10,12},{11,12}}

Cousin 1563: {{1,5},{1,7},{1,8},{2,4},{2,6},{2,7},{2,8},{2,13},{3,7},{3,9},{3,10},{3,14},{4,6},{4,7},{4,9},{4,11},{5,10},{5,13},{6,12},{6,14},{8,11},{8,14},{9,12},{9,13},{10,11},{10,12},{10,14},{11,12}}

Cousin 1564: {{1,7},{1,8},{1,10},{1,13},{2,4},{2,6},{2,7},{2,8},{2,13},{3,5},{3,10},{3,14},{4,6},{4,7},{4,9},{4,11},{5,7},{5,9},{6,12},{6,14},{8,11},{8,14},{9,12},{9,13},{10,11},{10,12},{10,13},{11,12}}

Cousin 1565: {{1,6},{1,9},{1,10},{1,11},{2,7},{2,9},{2,12},{2,13},{3,7},{3,9},{3,11},{3,12},{4,7},{4,8},{4,10},{4,14},{5,7},{5,9},{5,10},{5,13},{6,8},{6,12},{6,14},{8,11},{8,13},{9,14},{10,14},{11,12}}

Cousin 1566: {{1,8},{1,9},{1,10},{1,11},{2,3},{2,7},{2,9},{2,10},{3,6},{3,8},{3,10},{3,11},{4,8},{4,9},{4,11},{4,12},{5,7},{5,9},{5,10},{5,13},{6,9},{6,11},{6,12},{6,13},{7,8},{7,12},{8,13},{12,13}}

Cousin 1567: {{1,8},{1,9},{1,10},{1,11},{2,7},{2,9},{2,10},{2,13},{3,5},{3,7},{3,9},{3,10},{4,8},{4,9},{4,11},{4,12},{5,6},{5,8},{5,11},{6,9},{6,11},{6,12},{6,13},{7,8},{7,12},{8,13},{10,13},{12,13}}

Cousin 1568: {{1,8},{1,9},{1,10},{1,11},{2,5},{2,9},{2,10},{2,12},{2,13},{3,5},{3,6},{3,9},{3,10},{4,8},{4,9},{4,11},{4,12},{5,8},{5,12},{6,7},{6,8},{6,11},{7,9},{7,12},{7,13},{8,13},{10,13},{12,13}}

Cousin 1569: {{1,3},{1,8},{1,12},{1,13},{2,6},{2,7},{2,9},{2,13},{3,7},{3,9},{3,10},{4,7},{4,9},{4,11},{4,13},{5,6},{5,7},{5,9},{5,10},{6,8},{6,13},{7,8},{8,11},{9,12},{10,11},{10,12},{11,12},{12,13}}

Cousin 1570: {{1,3},{1,7},{1,9},{1,10},{2,6},{2,7},{2,9},{2,13},{3,8},{3,10},{3,12},{3,13},{4,7},{4,9},{4,11},{4,13},{5,6},{5,7},{5,9},{5,10},{6,8},{7,8},{8,11},{9,12},{10,11},{10,12},{11,12},{12,13}}

Cousin 1571: {{1,3},{1,7},{1,9},{2,3},{2,6},{2,8},{3,10},{4,7},{4,9},{4,11},{4,13},{5,7},{5,8},{5,10},{5,14},{6,12},{6,13},{7,15},{8,11},{8,15},{9,12},{9,14},{10,11},{10,12},{11,12},{13,14},{13,15},{14,15}}

Cousin 1572: {{1,3},{1,7},{1,9},{1,10},{2,13},{2,14},{2,15},{3,6},{3,8},{3,10},{4,7},{4,9},{4,11},{4,13},{5,7},{5,8},{5,10},{5,14},{6,12},{6,13},{7,15},{8,11},{8,15},{9,12},{9,14},{10,11},{10,12},{11,12}}

Cousin 1573: {{1,3},{1,7},{1,9},{2,13},{2,14},{2,15},{3,6},{3,10},{4,7},{4,9},{4,11},{4,13},{5,7},{5,8},{5,10},{5,14},{6,8},{6,12},{6,13},{7,15},{8,11},{8,15},{9,12},{9,14},{10,11},{10,12},{11,12},{12,13}}

Cousin 1574: {{1,10},{1,11},{1,12},{2,3},{2,7},{2,9},{2,10},{3,6},{3,8},{3,10},{4,7},{4,9},{4,11},{4,13},{5,7},{5,8},{5,10},{5,14},{6,12},{6,13},{7,15},{8,11},{8,15},{9,12},{9,14},{13,14},{13,15},{14,15}}

Cousin 1575: {{1,10},{1,11},{1,12},{2,3},{2,7},{2,9},{3,6},{3,10},{4,7},{4,9},{4,11},{4,13},{5,7},{5,8},{5,10},{5,14},{6,8},{6,12},{6,13},{7,15},{8,11},{8,15},{9,12},{9,14},{12,13},{13,14},{13,15},{14,15}}

Cousin 1576: {{1,10},{1,11},{1,12},{2,13},{2,14},{2,15},{3,6},{3,7},{3,9},{3,10},{4,7},{4,9},{4,11},{4,13},{5,7},{5,8},{5,10},{5,14},{6,8},{6,10},{6,12},{6,13},{7,15},{8,11},{8,15},{9,12},{9,14},{12,13}}

Cousin 1577: {{1,4},{1,7},{1,9},{2,3},{2,6},{2,8},{3,7},{3,9},{3,10},{4,11},{4,13},{5,7},{5,8},{5,10},{5,14},{6,12},{6,13},{7,15},{8,11},{8,15},{9,12},{9,14},{10,11},{10,12},{11,12},{13,14},{13,15},{14,15}}

Cousin 1578: {{1,7},{1,9},{1,11},{1,13},{2,13},{2,14},{2,15},{3,4},{3,7},{3,9},{3,10},{4,6},{4,8},{5,7},{5,8},{5,10},{5,14},{6,12},{6,13},{7,15},{8,11},{8,15},{9,12},{9,14},{10,11},{10,12},{11,12},{11,13}}

Cousin 1579: {{1,4},{1,7},{1,9},{2,13},{2,14},{2,15},{3,6},{3,7},{3,9},{3,10},{4,11},{4,13},{5,7},{5,8},{5,10},{5,14},{6,8},{6,12},{6,13},{7,15},{8,11},{8,15},{9,12},{9,14},{10,11},{10,12},{11,12},{12,13}}

Cousin 1580: {{1,10},{1,11},{1,12},{2,7},{2,9},{2,11},{2,13},{3,4},{3,7},{3,9},{3,10},{4,6},{4,8},{5,7},{5,8},{5,10},{5,14},{6,12},{6,13},{7,15},{8,11},{8,15},{9,12},{9,14},{11,13},{13,14},{13,15},{14,15}}

Cousin 1581: {{1,10},{1,11},{1,12},{2,4},{2,7},{2,9},{3,6},{3,7},{3,9},{3,10},{4,11},{4,13},{5,7},{5,8},{5,10},{5,14},{6,8},{6,12},{6,13},{7,15},{8,11},{8,15},{9,12},{9,14},{12,13},{13,14},{13,15},{14,15}}

Cousin 1582: {{1,10},{1,11},{1,12},{2,13},{2,14},{2,15},{3,6},{3,7},{3,9},{3,10},{4,7},{4,9},{4,11},{4,13},{5,7},{5,8},{5,10},{5,14},{6,8},{6,12},{6,13},{7,15},{8,11},{8,15},{9,12},{9,14},{11,13},{12,13}}

Cousin 1583: {{1,3},{1,8},{1,12},{1,13},{2,6},{2,7},{2,8},{2,13},{3,7},{3,9},{3,10},{4,7},{4,9},{4,11},{4,13},{5,6},{5,7},{5,8},{5,10},{6,9},{6,13},{7,9},{8,11},{9,12},{10,11},{10,12},{11,12},{12,13}}

Cousin 1584: {{1,7},{1,9},{1,11},{1,13},{2,4},{2,7},{2,8},{2,13},{3,6},{3,7},{3,8},{3,9},{3,10},{4,5},{4,9},{4,13},{5,7},{5,8},{5,10},{6,8},{6,12},{6,13},{8,11},{9,12},{10,11},{10,12},{11,12},{11,13}}

Cousin 1585: {{1,3},{1,7},{1,9},{1,10},{2,6},{2,7},{2,8},{2,13},{3,8},{3,10},{3,12},{3,13},{4,7},{4,9},{4,11},{4,13},{5,6},{5,7},{5,8},{5,10},{6,9},{7,8},{8,11},{9,12},{10,11},{10,12},{11,12},{12,13}}

Cousin 1586: {{1,5},{1,7},{1,8},{1,10},{2,5},{2,7},{2,8},{2,13},{3,6},{3,7},{3,8},{3,9},{3,10},{4,7},{4,9},{4,11},{4,13},{5,9},{5,10},{6,8},{6,12},{6,13},{8,11},{9,12},{10,11},{10,12},{11,12},{11,13}}

Cousin 1587: {{1,3},{1,7},{1,9},{1,10},{2,5},{2,6},{2,9},{2,13},{3,8},{3,10},{3,12},{3,13},{4,7},{4,9},{4,11},{4,13},{5,7},{5,8},{5,9},{5,10},{6,7},{6,8},{8,11},{9,12},{10,11},{10,12},{11,12},{12,13}}

Cousin 1588: {{1,7},{1,9},{1,11},{1,13},{2,5},{2,6},{2,9},{2,13},{3,4},{3,7},{3,9},{3,10},{4,8},{4,12},{4,13},{5,7},{5,8},{5,9},{5,10},{6,7},{6,8},{8,11},{9,12},{10,11},{10,12},{11,12},{11,13},{12,13}}

Cousin 1589: {{1,3},{1,7},{1,9},{1,10},{2,5},{2,6},{2,7},{2,8},{2,9},{3,6},{3,8},{3,13},{4,6},{4,7},{4,9},{4,11},{5,7},{5,8},{5,9},{5,10},{6,12},{7,8},{8,11},{9,12},{10,11},{10,13},{11,12},{12,13}}

Cousin 1590: {{1,7},{1,8},{1,10},{1,13},{2,4},{2,6},{2,7},{2,8},{2,13},{3,5},{3,7},{3,9},{3,10},{4,6},{4,7},{4,9},{4,11},{5,6},{5,8},{5,10},{6,12},{8,11},{9,12},{9,13},{10,11},{10,12},{10,13},{11,12}}

Cousin 1591: {{1,8},{1,9},{1,10},{1,11},{2,5},{2,9},{2,10},{2,14},{3,5},{3,6},{3,9},{3,10},{4,8},{4,9},{4,11},{4,12},{5,8},{5,12},{6,7},{6,8},{6,11},{7,9},{7,12},{7,13},{8,13},{10,13},{12,14},{13,14}}

Cousin 1592: {{1,3},{1,7},{1,9},{1,10},{2,6},{2,7},{2,9},{2,13},{3,8},{3,13},{3,14},{4,7},{4,9},{4,11},{4,13},{5,6},{5,7},{5,9},{5,10},{6,8},{7,8},{8,11},{9,12},{10,11},{10,14},{11,12},{12,13},{12,14}}

Cousin 1593: {{1,2},{1,7},{1,9},{1,10},{2,6},{2,8},{2,10},{3,7},{3,8},{3,13},{3,14},{4,7},{4,9},{4,11},{4,13},{5,7},{5,8},{5,10},{5,14},{6,12},{6,13},{8,11},{9,12},{9,14},{10,11},{10,12},{11,12},{13,14}}

Cousin 1594: {{1,3},{1,7},{1,9},{2,3},{2,8},{2,12},{2,13},{3,10},{4,7},{4,9},{4,11},{4,13},{5,7},{5,8},{5,10},{5,14},{6,7},{6,8},{6,13},{6,14},{8,11},{9,12},{9,14},

{10,11},{10,12},{11,12},{12,13},{13,14}}

Cousin 1595: {{1,3},{1,7},{1,9},{1,10},{2,6},{2,13},{2,14},{3,8},{3,10},{3,12},{3,13},{4,7},{4,9},{4,11},{4,13},{5,7},{5,8},{5,10},{5,14},{6,7},{6,8},{8,11},{9,12},{9,14},{10,11},{10,12},{11,12},{12,13}}

Cousin 1596: {{1,10},{1,11},{1,12},{2,3},{2,7},{2,9},{2,10},{3,8},{3,10},{3,12},{3,13},{4,7},{4,9},{4,11},{4,13},{5,7},{5,8},{5,10},{5,14},{6,7},{6,8},{6,13},{6,14},{8,11},{9,12},{9,14},{12,13},{13,14}}

Cousin 1597: {{1,7},{1,9},{1,11},{1,13},{2,3},{2,6},{2,8},{3,7},{3,9},{3,10},{4,7},{4,8},{4,13},{4,14},{5,7},{5,8},{5,10},{5,14},{6,12},{6,13},{8,11},{9,12},{9,14},{10,11},{10,12},{11,12},{11,13},{13,14}}

Cousin 1598: {{1,4},{1,7},{1,9},{2,3},{2,8},{2,12},{2,13},{3,7},{3,9},{3,10},{4,11},{4,13},{5,7},{5,8},{5,10},{5,14},{6,7},{6,8},{6,13},{6,14},{8,11},{9,12},{9,14},{10,11},{10,12},{11,12},{12,13},{13,14}}

Cousin 1599: {{1,7},{1,9},{1,11},{1,13},{2,6},{2,13},{2,14},{3,4},{3,7},{3,9},{3,10},{4,8},{4,12},{4,13},{5,7},{5,8},{5,10},{5,14},{6,7},{6,8},{8,11},{9,12},{9,14},{10,11},{10,12},{11,12},{11,13},{12,13}}

Cousin 1600: {{1,10},{1,11},{1,12},{2,7},{2,9},{2,11},{2,13},{3,4},{3,7},{3,9},{3,10},{4,8},{4,12},{4,13},{5,7},{5,8},{5,10},{5,14},{6,7},{6,8},{6,13},{6,14},{8,11},{9,12},{9,14},{11,13},{12,13},{13,14}}

Cousin 1601: {{1,3},{1,7},{1,9},{1,10},{2,6},{2,7},{2,8},{2,13},{3,8},{3,13},{3,14},{4,7},{4,9},{4,11},{4,13},{5,6},{5,7},{5,8},{5,10},{6,9},{7,8},{8,11},{9,12},{10,11},{10,14},{11,12},{12,13},{12,14}}

Cousin 1602: {{1,3},{1,7},{1,9},{1,10},{2,5},{2,6},{2,9},{2,13},{3,8},{3,13},{3,14},{4,7},{4,9},{4,11},{4,13},{5,7},{5,8},{5,9},{5,10},{6,7},{6,8},{8,11},{9,12},{10,11},{10,14},{11,12},{12,13},{12,14}}

Cousin 1603: {{1,7},{1,9},{1,11},{1,13},{2,5},{2,6},{2,9},{2,13},{3,4},{3,7},{3,9},{3,10},{4,8},{4,12},{4,13},{5,7},{5,8},{5,9},{5,10},{6,7},{6,8},{8,11},{9,12},{10,11},{10,12},{11,14},{12,14},{13,14}}

Cousin 1604: {{1,2},{1,7},{1,9},{1,10},{2,8},{2,10},{2,12},{2,13},{3,6},{3,7},{3,8},{3,13},{4,7},{4,9},{4,11},{4,13},{5,6},{5,7},{5,8},{5,10},{6,9},{6,13},{8,11},{9,12},{10,11},{10,12},{11,12},{12,13}}

Cousin 1605: {{1,3},{1,7},{1,9},{1,10},{2,6},{2,13},{2,14},{3,8},{3,13},{3,15},{4,7},{4,9},{4,11},{4,13},{5,7},{5,8},{5,10},{5,14},{6,7},{6,8},{8,11},{9,12},{9,14},{10,11},{10,15},{11,12},{12,13},{12,15}}

Cousin 1606: {{1,7},{1,9},{1,11},{1,13},{2,8},{2,12},{2,13},{3,7},{3,9},{3,10},{4,6},{4,7},{4,8},{4,13},{5,6},{5,7},{5,8},{5,10},{6,9},{6,13},{8,11},{9,12},{10,11},{10,12},{11,12},{11,13},{12,13}}

Cousin 1607: {{1,7},{1,9},{1,11},{1,13},{2,6},{2,13},{2,14},{3,4},{3,7},{3,9},{3,10},{4,8},{4,12},{4,13},{5,7},{5,8},{5,10},{5,14},{6,7},{6,8},{8,11},{9,12},{9,14},{10,11},{10,12},{11,15},{12,15},{13,15}}

Cousin 1608: {{1,2},{1,7},{1,9},{1,10},{2,8},{2,13},{2,14},{3,6},{3,7},{3,8},{3,13},{4,7},{4,9},{4,11},{4,13},{5,6},{5,7},{5,8},{5,10},{6,9},{6,13},{8,11},{9,12},{10,11},{10,14},{11,12},{12,13},{12,14}}

Cousin 1609: {{1,7},{1,9},{1,11},{1,13},{2,3},{2,8},{2,12},{2,13},{3,7},{3,9},{3,10},{4,6},{4,7},{4,8},{4,13},{5,6},{5,7},{5,8},{5,10},{6,9},{6,13},{8,11},{9,12},{10,11},{10,12},{11,14},{12,14},{13,14}}

---

Cousin 1151 and its ancestors:

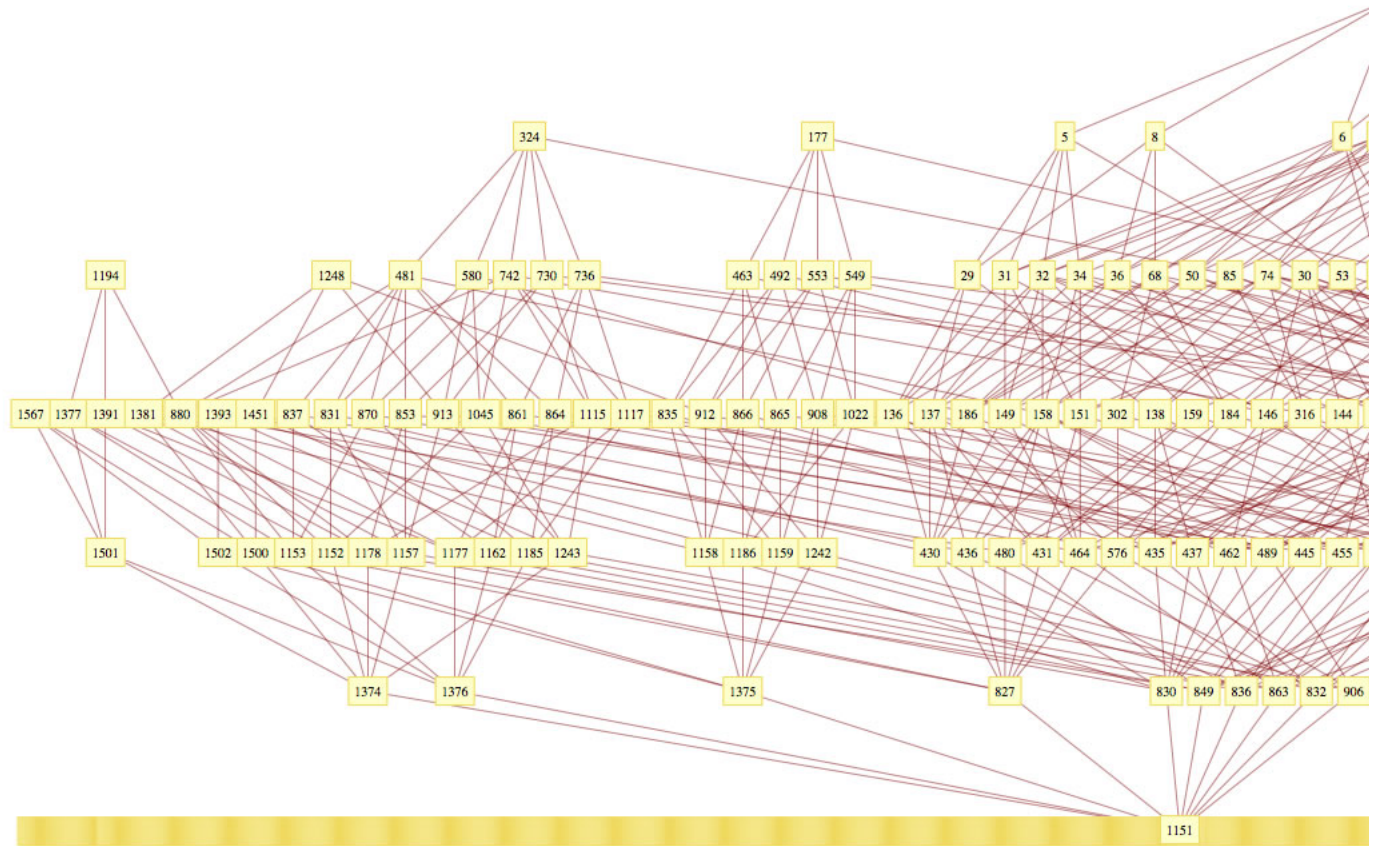

## Section 4.1:

### Lists of children of each graph in the $G_{\{9,28\}}$ family

The  $G_{9,28}$  family consists of 1609 graphs. Since this family is too large to give a family diagram for it here, we instead give a list of all children for each graph in the family. In this list, each Cousin  $C$  is followed by a list of pairs,  $\{c,v\}$ , where Cousin  $c$  is a child of Cousin  $C$  and vertex  $v$  of Cousin  $c$  is the new degree-3 vertex that is created by a triangle-Y move on Cousin  $C$ . For example, Cousin 5 is a child of Cousin 2 (see "Children of Cousin 2" below); the pairs  $\{5,10\}$  and  $\{5,11\}$  indicate that there are two ways of doing a triangle-Y move on Cousin 2 to obtain Cousin 5, one of which yields vertex 10, the other vertex 11, as the new degree-3 vertex in Cousin 5.

$G_{9,28}$  is Cousin 1.

Children of Cousin 1:  $\{\{2,10\},\{3,10\},\{4,10\}\}$

Children of Cousin 2:  $\{\{5,10\},\{5,11\},\{6,11\},\{7,11\},\{8,10\},\{8,11\},\{9,11\},\{10,11\},\{11,11\},\{12,11\}\}$

Children of Cousin 3:  $\{\{7,10\},\{9,10\},\{11,10\},\{13,11\},\{14,11\},\{15,10\},\{15,11\},\{16,10\},\{16,11\},\{17,10\},\{17,11\},\{18,11\},\{19,11\},\{20,10\},\{20,11\},\{21,10\},\{21,11\},\{22,11\},\{23,11\}\}$

Children of Cousin 4: {{6,10},{10,10},{12,10},{13,10},{14,10},{18,10},{19,10},{22,10},{23,10},{24,10},{24,11},{25,10},{25,11},{26,10},{26,11},{27,10},{27,11},{28,10},{28,11}}

Children of Cousin 5: {{29,10},{29,12},{30,12},{31,12},{32,12},{33,12},{34,12}}

Children of Cousin 6: {{31,11},{35,12},{36,12},{37,10},{37,12},{38,12},{39,11},{39,12},{40,11},{40,12},{41,12},{42,12},{43,12},{44,12},{45,12},{46,12},{47,12},{48,12},{49,12},{50,12},{51,12},{52,12}}

Children of Cousin 7: {{30,10},{35,11},{51,11},{52,11},{53,10},{53,12},{54,12},{55,12},{56,12},{57,12},{58,12},{59,12},{60,12},{61,12},{62,12},{63,12},{64,12},{65,12},{66,11},{66,12},{67,11},{67,12}}

Children of Cousin 8: {{29,11},{36,11},{37,11},{53,11},{54,11},{68,12}}

Children of Cousin 9: {{30,11},{38,11},{55,11},{56,11},{69,12},{70,12},{71,12},{72,12}}

Children of Cousin 10: {{31,10},{32,11},{41,11},{42,11},{50,11},{57,11},{64,11},{65,11},{68,10},{69,11},{73,12},{74,12},{75,12},{76,12},{77,12},{78,11},{78,12},{79,11},{79,12}}

Children of Cousin 11: {{33,10},{33,11},{43,11},{44,11},{49,11},{54,10},{58,11},{59,11},{63,11},{70,11},{73,11},{77,11},{80,12},{81,12},{82,12},{83,11},{83,12},{84,11},{84,12}}

Children of Cousin 12: {{32,10},{34,10},{34,11},{36,10},{45,11},{46,11},{47,11},{48,11},{60,11},{61,11},{62,11},{68,11},{71,11},{72,11},{74,11},{75,11},{76,11},{80,11},{81,11},{82,11},{85,11},{85,12}}

Children of Cousin 13: {{38,10},{57,10},{73,10},{82,10},{86,10},{86,12},{87,12},{88,12},{89,12},{90,12},{91,12},{92,12},{93,12},{94,12},{95,11},{95,12},{96,12},{97,12},{98,12},{99,12}}

Children of Cousin 14: {{35,10},{49,10},{60,10},{69,10},{77,10},{94,11},{96,10},{100,12},{101,12},{102,12},{103,12},{104,12},{105,12},{106,12},{107,11},{107,12},{108,12},{109,12},{110,12},{111,12}}

Children of Cousin 15: {{63,10},{70,10},{93,11},{112,12},{113,12},{114,12},{115,12},{116,12},{117,11},{117,12}}

Children of Cousin 16: {{58,10},{66,10},{86,11},{91,11},{100,11},{105,11},{112,11},{116,11},{118,12},{119,12}}

Children of Cousin 17: {{59,10},{67,10},{92,11},{101,11},{106,11},{113,11},{116,10},{120,12}}

Children of Cousin 18: {{43,10},{61,10},{64,10},{71,10},{87,11},{89,11},{92,10},{93,10},{102,11},{103,11},{106,10},{109,10},{114,11},{121,12},{122,10},{122,12},{123,12},{124,12},{125,12}}

Children of Cousin 19: {{44,10},{62,10},{65,10},{72,10},{88,11},{90,11},{91,10},{104,11},{105,10},{108,10},{115,11},{121,11},{123,10},{126,10},{126,12},{127,12},{128,12}}

Children of Cousin 20: {{55,10},{83,10},{96,11},{98,11},{108,11},{113,10},{117,10},{118,10},{118,11},{120,11},{122,11},{126,11}}

Children of Cousin 21: {{56,10},{84,10},{99,11},{109,11},{112,10},{119,10},{119,11},{120,10},{123,11}}

Children of Cousin 22: {{51,10},{80,10},{97,11},{99,10},{101,10},{110,11},{115,10},{124,11},{127,11}}

Children of Cousin 23: {{52,10},{81,10},{98,10},{100,10},{111,11},{114,10},{125,11},{128,11}}

Children of Cousin 24: {{50,10},{74,10},{85,10},{97,10},{102,10},{121,10},{129,10},{129,12},{130,12},{131,12},{132,12}}

Children of Cousin 25: {{39,10},{47,10},{75,10},{88,10},{95,10},{104,10},{111,10},{129,11},{131,10},{133,10},{133,12},{134,12}}

Children of Cousin 26: {{40,10},{48,10},{76,10},{87,10},{103,10},{110,10},{130,10},{134,10},{135,10},{135,12}}

Children of Cousin 27: {{41,10},{45,10},{78,10},{90,10},{94,10},{107,10},{124,10},{128,10},{130,11},{132,11},{133,11},{135,11}}

Children of Cousin 28: {{42,10},{46,10},{79,10},{89,10},{125,10},{127,10},{131,11},{132,10},{134,11}}

Children of Cousin 29: {{136,13},{137,13},{138,13}}

Children of Cousin 30: {{138,10},{138,12},{139,13},{140,13},{141,13},{142,13},{143,13},{144,13},{145,13},{146,13},{147,12},{147,13},{148,12},{148,13}}

Children of Cousin 31: {{136,12},{139,12},{146,12},{149,13},{150,13},{151,13},{152,13},{153,13},{154,13},{155,12},{155,13},{156,12},{156,13}}

Children of Cousin 32: {{136,10},{137,12},{140,12},{144,12},{145,12},{149,12},{153,12},{154,12},{157,13},{158,13},{159,12},{159,13},{160,12},{160,13}}

Children of Cousin 33: {{141,12},{150,12},{157,12},{161,13},{162,13}}

Children of Cousin 34: {{137,10},{142,12},{143,12},{151,12},{152,12},{158,12},{161,12},{162,12}}

Children of Cousin 35: {{146,10},{163,13},{164,13},{165,13},{166,13},{167,13},{168,13},{169,13},{170,13},{171,13},{172,13},{173,13},{174,13},{175,13},{176,13}}

Children of Cousin 36: {{136,11},{163,12},{178,13},{179,13},{180,13},{181,13},{182,11},{182,13},{183,11},{183,13},{184,13},{185,13},{186,13},{187,13},{188,13}}

Children of Cousin 37: {{164,12},{178,11},{179,11},{189,13},{190,13},{191,13},{192,13}}

Children of Cousin 38: {{139,11},{165,12},{193,11},{193,13},{194,13},{195,13},{196,13},{197,13},{198,13},{199,13},{200,13},{201,13}}

Children of Cousin 39: {{166,12},{178,12},{193,12},{202,13},{203,13},{204,13},{205,13}}

Children of Cousin 40: {{167,12},{179,12},{206,13},{207,13},{208,13},{209,13}}

Children of Cousin 41: {{155,10},{155,11},{168,12},{189,12},{194,12},{206,12},{210,13},{211,13},{212,13},{213,13},{214,13},{215,13},{216,13},{217,13}}

Children of Cousin 42: {{156,10},{156,11},{190,12},{202,12},{218,13},{219,13},{220,13},{221,13},{222,13},{223,13},{224,13}}

Children of Cousin 43: {{169,12},{180,12},{195,12},{207,12},{218,12},{225,13},{226,13},{227,13},{228,13},{229,13},{230,13}}

Children of Cousin 44: {{170,12},{181,12},{203,12},{210,12},{231,13},{232,13},{233,13},{234,13},{235,13}}

Children of Cousin 45: {{153,11},{171,12},{182,10},{182,12},{189,10},{196,12},{204,12},{208,12},{219,12},{225,12},{231,12},{236,13},{237,13},{238,13},{239,13},{240,13}}

Children of Cousin 46: {{154,11},{183,10},{183,12},{190,10},{197,12},{205,12},{209,12},{211,12},{226,12},{232,12},{241,13},{242,13},{243,13},{244,13}}

Children of Cousin 47: {{151,11},{172,12},{178,10},{184,12},{198,12},{204,11},{209,11},{212,12},{220,12},{233,12},{241,12},{245,13},{246,13},{247,13}}

Children of Cousin 48: {{152,11},{173,12},{179,10},{185,12},{199,12},{205,11},{208,11},{213,12},{221,12},{227,12},{236,12},{248,13},{249,13}}

Children of Cousin 49: {{150,11},{164,10},{203,11},{207,11},{214,12},{228,12},{234,12},{237,12},{245,12},{248,12},{250,13},{251,13}}

Children of Cousin 50: {{149,11},{174,12},{186,12},{202,11},{206,11},{215,12},{222,12},{229,12},{238,12},{242,12},{246,12},{252,13}}

Children of Cousin 51: {{167,11},{175,12},{187,12},{191,10},{191,12},{200,12},{216,12},{223,12},{235,12},{239,12},{243,12},{249,12},{250,12},{252,12}}

Children of Cousin 52: {{166,11},{176,12},{188,12},{192,10},{192,12},{201,12},{217,12},{224,12},{230,12},{240,12},{244,12},{247,12},{251,12}}

Children of Cousin 53: {{138,11},{163,11},{191,11},{192,11},{253,13},{254,13},{255,13},{256,13}}

Children of Cousin 54: {{164,11},{180,11},{181,11},{187,11},{188,11},{253,11},{254,11},{257,13},{258,13},{259,11},{259,13}}

Children of Cousin 55: {{147,10},{147,11},{165,11},{201,11},{260,13},{261,13},{262,13},{263,13},{264,13},{265,13},{266,13},{267,11},{267,13},{268,13}}

Children of Cousin 56: {{148,10},{148,11},{200,11},{268,11},{269,13},{270,13},{271,13},{272,13},{273,13},{274,11},{274,13}}

Children of Cousin 57: {{139,10},{168,11},{252,11},{257,12},{260,12},{275,13},{276,13},{277,13},{278,13},{279,13},{280,13},{281,13}}

Children of Cousin 58: {{170,11},{251,11},{253,12},{269,12},{275,12},{282,13},{283,13},{284,13},{285,13},{286,13}}

Children of Cousin 59: {{169,11},{250,11},{254,12},{261,12},{287,13},{288,13},{289,13},{290,13},{291,13}}

Children of Cousin 60: {{140,10},{163,10},{171,11},{247,11},{249,11},{258,12},{262,12},{270,12},{282,12},{287,12},{292,13},{293,13},{294,13},{295,13},{296,13}}

Children of Cousin 61: {{142,10},{173,11},{180,10},{239,11},{244,11},{255,12},{263,12},{271,12},{276,12},{288,12},{292,12},{296,11},{297,13},{298,13}}

Children of Cousin 62: {{143,10},{172,11},{181,10},{240,11},{243,11},{256,12},{264,12},{272,12},{277,12},{283,12},{295,11},{299,13},{300,13}}

Children of Cousin 63: {{141,10},{230,11},{235,11},{259,10},{259,12},{265,12},{284,12},{286,11},{289,12},{291,11},{297,12},{299,12},{301,13}}

Children of Cousin 64: {{144,10},{174,11},{216,11},{224,11},{255,10},{273,12},{278,12},{281,11},{290,12},{293,12},{300,12},{301,12}}

Children of Cousin 65: {{145,10},{217,11},{223,11},{256,10},{266,12},{279,12},{280,11},{285,12},{294,12},{298,12}}

Children of Cousin 66: {{176,11},{253,10},{267,12},{274,12},{280,12},{291,12},{295,12}}

Children of Cousin 67: {{175,11},{254,10},{268,12},{281,12},{286,12},{296,12}}

Children of Cousin 68: {{137,11},{184,11},{185,11},{186,11},{189,11},{190,11},{255,11},{256,11},{257,11},{258,11},{302,12},{302,13}}

Children of Cousin 69: {{140,11},{146,11},{194,11},{260,11},{266,11},{273,11},{303,13},{304,13},{305,13},{306,12},{306,13}}

Children of Cousin 70: {{141,11},{195,11},{261,11},{265,11},{269,11},{307,13},{308,13},{309,13},{310,12},{310,13}}

Children of Cousin 71: {{142,11},{144,11},{197,11},{199,11},{263,11},{270,11},{272,11},{303,12},{304,12},{307,12},{309,12},{311,13}}

Children of Cousin 72: {{143,11},{145,11},{196,11},{198,11},{262,11},{264,11},{271,11},{305,12},{308,12},{311,12}}

Children of Cousin 73: {{157,11},{210,11},{218,11},{275,11},{301,11},{312,13},{313,13},{314,13},{315,13}}



Children of Cousin 74: {{149,10},{158,11},{211,11},{219,11},{246,11},{298,11},{300,11},{302,10},{302,11},{303,11},{312,12},{316,13},{317,13},{318,13}}

Children of Cousin 75: {{151,10},{159,10},{159,11},{184,10},{212,11},{221,11},{242,11},{277,11},{294,11},{305,11},{313,12},{316,12},{318,11},{319,13}}

Children of Cousin 76: {{152,10},{160,10},{160,11},{185,10},{213,11},{220,11},{238,11},{276,11},{293,11},{304,11},{317,11},{320,13}}

Children of Cousin 77: {{150,10},{214,11},{229,11},{258,10},{285,11},{290,11},{314,12},{315,11},{319,12},{320,12}}

Children of Cousin 78: {{153,10},{222,11},{279,11},{306,11},{315,12},{317,12}}

Children of Cousin 79: {{154,10},{215,11},{278,11},{318,12}}

Children of Cousin 80: {{161,10},{161,11},{187,10},{225,11},{232,11},{248,11},{287,11},{299,11},{308,11},{312,11},{320,11},{321,13},{322,13}}

Children of Cousin 81: {{162,10},{162,11},{188,10},{226,11},{231,11},{245,11},{282,11},{297,11},{307,11},{319,11},{323,13}}

Children of Cousin 82: {{157,10},{227,11},{233,11},{237,11},{257,10},{283,11},{288,11},{309,11},{313,11},{321,12},{322,11},{323,11}}

Children of Cousin 83: {{234,11},{289,11},{310,11},{314,11},{323,12}}

Children of Cousin 84: {{228,11},{284,11},{322,12}}

Children of Cousin 85: {{158,10},{186,10},{236,11},{241,11},{292,11},{311,11},{316,11},{321,11}}

Children of Cousin 86: {{275,10},{325,13},{326,13},{327,13},{328,13},{329,13}}

Children of Cousin 87: {{199,10},{227,10},{276,10},{330,13},{331,13},{332,10},{332,13},{333,13},{334,13},{335,13},{336,13},{337,13}}

Children of Cousin 88: {{198,10},{233,10},{277,10},{325,12},{338,13},{339,13},{340,13},{341,13},{342,13},{343,13},{344,13}}

Children of Cousin 89: {{197,10},{218,10},{278,10},{334,11},{338,12},{345,10},{345,13},{346,13},{347,13},{348,13},{349,13},{350,13}}

Children of Cousin 90: {{196,10},{210,10},{279,10},{326,12},{330,12},{341,11},{351,10},{351,13},{352,13},{353,13},{354,13},{355,13},{356,13}}

Children of Cousin 91: {{280,10},{283,10},{325,11},{339,12},{351,11},{351,12},{357,13},{358,13},{359,13},{360,13}}

Children of Cousin 92: {{281,10},{288,10},{327,12},{331,12},{345,11},{345,12},{361,13},{362,13},{363,13},{364,13},{365,13}}

Children of Cousin 93: {{195,10},{301,10},{309,10},{327,10},{332,11},{332,12},{346,12},{352,12},{357,12},{361,12},{366,13},{367,13},{368,13}}

Children of Cousin 94: {{168,10},{194,10},{237,10},{315,10},{326,10},{333,12},{340,12},{347,12},{358,12},{362,12},{369,10},{369,13},{370,13},{371,13},{372,13}}

Children of Cousin 95: {{193,10},{313,10},{325,10},{334,12},{341,12},{373,13},{374,13}}

Children of Cousin 96: {{165,10},{260,10},{314,10},{335,12},{342,12},{353,12},{359,12},{363,12},{366,12},{369,11},{369,12},{373,12},{375,13},{376,13}}

Children of Cousin 97: {{252,10},{312,10},{321,10},{336,12},{343,12},{348,12},{354,12},{364,12},{367,12},{370,12},{374,11},{374,12},{377,10},{377,13}}

Children of Cousin 98: {{201,10},{323,10},{328,10},{328,12},{344,12},{349,12},{355,12},{365,12},{368,12},{371,12},{373,11},{375,12}}

Children of Cousin 99: {{200,10},{322,10},{329,10},{329,12},{337,12},{350,12},{356,12},{360,12},{372,12},{376,12},{377,11},{377,12}}

Children of Cousin 100: {{176,10},{251,10},{282,10},{358,11},{375,10},{378,13},{379,13},{380,13},{381,13},{382,11},{382,13}}

Children of Cousin 101: {{175,10},{250,10},{287,10},{362,11},{364,11},{376,10},{383,13},{384,13},{385,13},{386,13},{387,11},{387,13}}

Children of Cousin 102: {{174,10},{229,10},{292,10},{303,10},{347,11},{364,10},{388,13},{389,10},{389,13},{390,13},{391,13},{392,13},{393,13},{394,13}}

Children of Cousin 103: {{173,10},{207,10},{293,10},{304,10},{331,10},{333,11},{335,10},{383,12},{390,11},{395,10},{395,13},{396,13},{397,13}}

Children of Cousin 104: {{172,10},{203,10},{294,10},{305,10},{339,10},{340,11},{342,10},{378,12},{388,12},{398,10},{398,13},{399,13},{400,13}}

Children of Cousin 105: {{170,10},{285,10},{295,10},{326,11},{339,11},{378,11},{380,11},{384,12},{401,13},{402,13}}

Children of Cousin 106: {{169,10},{290,10},{296,10},{331,11},{366,10},{379,12},{383,11},{385,11},{389,11},{389,12},{403,13},{404,13}}

Children of Cousin 107: {{171,10},{214,10},{306,10},{353,10},{380,12},{385,12},{390,12},{405,13},{406,13}}

Children of Cousin 108: {{234,10},{262,10},{266,10},{344,11},{353,11},{359,10},{371,11},{386,12},{391,12},{398,11},{398,12},{401,12},{403,12}}

Children of Cousin 109: {{228,10},{270,10},{273,10},{337,11},{363,10},{372,11},{381,12},{392,12},{395,11},{395,12},{402,12},{404,12}}

Children of Cousin 110: {{167,10},{248,10},{249,10},{320,10},{337,10},{370,11},{383,10},{387,10},{387,12},{393,12},{396,12},{399,12},{405,11},{405,12}}

Children of Cousin 111: {{166,10},{245,10},{247,10},{319,10},{344,10},{373,10},{378,10},{382,10},{382,12},{394,12},{397,12},{400,12},{406,11},{406,12}}

Children of Cousin 112: {{269,10},{284,10},{357,11},{360,11},{381,11},{407,10},{407,13},{408,13},{409,13},{410,12},{410,13}}

Children of Cousin 113: {{261,10},{289,10},{361,11},{365,11},{366,11},{386,11},{409,12},{411,10},{411,13},{412,13},{413,11},{413,13},{414,12},{414,13}}

Children of Cousin 114: {{230,10},{297,10},{307,10},{346,11},{365,10},{368,10},{379,10},{381,10},{415,10},{415,13},{416,13},{417,12},{417,13}}

Children of Cousin 115: {{235,10},{299,10},{308,10},{352,11},{360,10},{367,11},{384,10},{386,10},{416,12},{418,10},{418,13},{419,12},{419,13}}

Children of Cousin 116: {{286,10},{291,10},{327,11},{379,11},{384,11},{407,11},{407,12},{408,11},{411,11},{411,12},{412,11}}

Children of Cousin 117: {{265,10},{310,10},{368,11},{408,12},{412,12},{413,10},{413,12},{415,12},{418,12}}

Children of Cousin 118: {{267,10},{328,11},{359,11},{375,11},{401,11},{409,11},{412,10}}

Children of Cousin 119: {{274,10},{329,11},{402,11},{410,10},{410,11}}

Children of Cousin 120: {{268,10},{363,11},{376,11},{403,11},{404,11},{408,10},{409,10},{414,10},{414,11}}

Children of Cousin 121: {{298,10},{300,10},{311,10},{330,11},{338,11},{367,10},{388,11},{391,10},{392,10},{420,13},{421,13}}

Children of Cousin 122: {{263,10},{335,11},{349,11},{361,10},{391,11},{404,10},{415,11}}

Children of Cousin 123: {{271,10},{272,10},{350,11},{356,11},{357,10},{392,11},{402,10},{403,10}}

Children of Cousin 124: {{216,10},{225,10},{239,10},{336,11},{348,11},{352,10},{356,10},{362,10},{372,10},{385,10},{393,11},{396,11},{416,11},{420,12}}

Children of Cousin 125: {{224,10},{226,10},{244,10},{346,10},{349,10},{394,11},{397,11},{417,10},{417,11},{421,12}}

Children of Cousin 126: {{264,10},{342,11},{355,11},{401,10},{418,11}}

Children of Cousin 127: {{223,10},{232,10},{243,10},{343,11},{350,10},{354,11},{399,11},{419,10},{419,11},{420,11}}

Children of Cousin 128: {{217,10},{231,10},{240,10},{355,10},{358,10},{371,10},{380,10},{400,11},{416,10},{421,11}}

Children of Cousin 129: {{246,10},{316,10},{374,10},{388,10},{422,10},{422,13},{423,13},{424,13}}

Children of Cousin 130: {{206,10},{236,10},{238,10},{317,10},{330,10},{336,10},{370,10},{390,10},{393,10},{424,10},{425,10},{425,13},{426,13},{427,12},{427,13}}

Children of Cousin 131: {{202,10},{241,10},{242,10},{318,10},{338,10},{343,10},{394,10},{422,11},{422,12},{423,10},{426,12},{428,10},{428,13},{429,12},{429,13}}

Children of Cousin 132: {{211,10},{215,10},{219,10},{222,10},{347,10},{348,10},{354,10},{420,10},{421,10},{423,12},{424,12},{425,11},{425,12},{428,11},{428,12}}

Children of Cousin 133: {{204,10},{212,10},{340,10},{341,10},{400,10},{406,10},{423,11},{426,11}}

Children of Cousin 134: {{205,10},{209,10},{220,10},{221,10},{334,10},{397,10},{399,10},{424,11},{426,10},{429,10},{429,11}}

Children of Cousin 135: {{208,10},{213,10},{333,10},{396,10},{405,10},{427,10},{427,11}}

Children of Cousin 136: {{430,14},{431,14},{432,14},{433,13},{433,14},{434,13},{434,14},{435,14}}

Children of Cousin 137: {{430,13},{431,13},{432,13},{436,13},{436,14},{437,14},{438,14}}

Children of Cousin 138: {{435,13},{437,13},{438,13}}

Children of Cousin 139: {{439,14},{440,14},{441,14},{442,14},{443,14},{444,14}}

Children of Cousin 140: {{435,10},{445,14},{446,14},{447,14},{448,14},{449,14},{450,14}}

Children of Cousin 141: {{451,14},{452,14},{453,14},{454,12},{454,14}}

Children of Cousin 142: {{437,10},{439,13},{445,13},{451,13},{455,14},{456,14},{457,12},{457,14},{458,14}}

Children of Cousin 143: {{438,10},{440,13},{452,13},{458,12},{459,14},{460,14},{461,12},{461,14}}

Children of Cousin 144: {{437,12},{441,13},{446,13},{450,12},{453,13},{459,13},{462,14}}

Children of Cousin 145: {{438,12},{442,13},{447,13},{449,12},{455,13}}

Children of Cousin 146: {{435,12},{443,13},{444,12},{448,13},{456,13},{460,13},{462,13}}

Children of Cousin 147: {{444,13},{449,13},{454,13},{457,13},{461,13}}

Children of Cousin 148: {{450,13},{458,13}}

Children of Cousin 149: {{430,12},{462,12},{464,14},{465,14},{466,14},{467,14},{468,14}}

Children of Cousin 150: {{469,14},{470,14},{471,14},{472,12},{472,14}}

Children of Cousin 151: {{431,12},{440,12},{460,12},{464,13},{469,13},{473,14},{474,12},{474,14},{475,14}}

Children of Cousin 152: {{432,12},{439,12},{456,12},{470,13},{475,12},{476,14},{477,12},{477,14}}

Children of Cousin 153: {{433,10},{433,12},{442,12},{448,12},{465,13},{468,12},{471,13},{476,13}}

Children of Cousin 154: {{434,10},{434,12},{441,12},{466,13},{467,12},{473,13}}

Children of Cousin 155: {{443,12},{467,13},{472,13},{474,13},{477,13}}

Children of Cousin 156: {{468,13},{475,13}}

Children of Cousin 157: {{453,12},{471,12},{478,14},{479,12},{479,14}}

Children of Cousin 158: {{430,10},{436,10},{436,12},{445,12},{455,12},{459,12},{464,12},{473,12},{476,12},{478,13},{480,12},{480,14}}

Children of Cousin 159: {{431,10},{447,12},{466,12},{479,13},{480,13}}

Children of Cousin 160: {{432,10},{446,12},{465,12}}

Children of Cousin 161: {{452,12},{470,12},{478,12}}

Children of Cousin 162: {{451,12},{469,12}}

Children of Cousin 163: {{435,11},{482,14},{483,14},{484,14},{485,14},{486,11},{486,14},{487,14},{488,14},{489,14},{490,14},{491,14}}

Children of Cousin 164: {{493,14},{494,14},{495,14},{496,14},{497,14},{498,14},{499,14},{500,14}}

Children of Cousin 165: {{444,11},{502,14},{503,14},{504,14},{505,14},{506,14},{507,14},{508,14},{509,14}}

Children of Cousin 166: {{482,13},{493,13},{502,13},{511,14},{512,14},{513,14},{514,14},{515,14},{516,12},{516,14}}

Children of Cousin 167: {{483,13},{494,13},{518,14},{519,14},{520,14},{521,14},{522,14},{523,14},{524,12},{524,14}}

Children of Cousin 168: {{443,10},{495,13},{503,13},{518,13},{526,14},{527,14},{528,14},{529,14},{530,14},{531,14}}

Children of Cousin 169: {{484,13},{504,13},{519,13},{533,14},{534,14},{535,14},{536,14}}

Children of Cousin 170: {{485,13},{511,13},{526,13},{538,14},{539,14},{540,14}}

Children of Cousin 171: {{448,10},{486,10},{486,13},{496,13},{505,13},{512,13},{520,13},{533,13},{538,13},{542,14},{543,14},{544,14},{545,14}}

Children of Cousin 172: {{460,10},{487,13},{497,13},{506,13},{513,13},{521,13},{527,13},{539,13},{547,14},{548,14}}

Children of Cousin 173: {{456,10},{488,13},{498,13},{507,13},{514,13},{522,13},{528,13},{534,13},{542,13},{550,14}}

Children of Cousin 174: {{462,10},{489,13},{515,13},{523,13},{529,13},{535,13},{543,13},{547,13},{552,14}}

Children of Cousin 175: {{490,13},{499,13},{508,13},{524,11},{524,13},{530,13},{540,13},{544,13},{550,13},{552,13}}

Children of Cousin 176: {{491,13},{500,13},{509,13},{516,11},{516,13},{531,13},{536,13},{545,13},{548,13}}

Children of Cousin 177: {{35,1},{463,10},{492,1},{501,1},{510,1},{517,1},{525,1},{532,1},{537,1},{541,1},{546,1},{549,1},{551,1},{553,1},{554,1},{555,1}}

Children of Cousin 178: {{482,12},{493,12},{497,12},{556,11},{556,14},{557,14},{558,14},{559,14},{560,14}}

Children of Cousin 179: {{483,12},{494,12},{498,12},{557,11},{561,11},{561,14},{562,14},{563,14},{564,14}}

Children of Cousin 180: {{484,12},{498,11},{565,14},{566,14},{567,14},{568,14},{569,14}}

Children of Cousin 181: {{485,12},{497,11},{570,14},{571,14},{572,14},{573,14}}

Children of Cousin 182: {{433,11},{486,12},{556,13},{561,13},{565,13},{570,13},{574,14}}

Children of Cousin 183: {{434,11},{557,13},{566,13},{571,13},{575,14}}

Children of Cousin 184: {{431,11},{487,12},{558,13},{562,13},{572,13},{575,13},{576,14},{577,14}}

Children of Cousin 185: {{432,11},{488,12},{559,13},{563,13},{567,13},{574,13},{578,14}}

Children of Cousin 186: {{430,11},{489,12},{560,13},{564,13},{568,13},{574,11},{575,11},{576,13},{579,14}}

Children of Cousin 187: {{490,12},{494,11},{565,11},{571,11},{573,13},{578,13},{579,13}}

Children of Cousin 188: {{491,12},{493,11},{566,11},{569,13},{570,11},{577,13}}

Children of Cousin 189: {{495,12},{496,12},{558,11},{563,11},{564,11},{581,14},{582,14},{583,14}}

Children of Cousin 190: {{559,11},{560,11},{562,11},{581,13},{584,14},{585,14}}

Children of Cousin 191: {{483,11},{499,12},{582,13},{584,13}}

Children of Cousin 192: {{482,11},{500,12},{583,13},{585,13}}

Children of Cousin 193: {{502,12},{586,14},{587,14}}

Children of Cousin 194: {{443,11},{503,12},{588,14},{589,14},{590,14},{591,14},{592,14}}

Children of Cousin 195: {{504,12},{593,14},{594,14},{595,14},{596,14}}

Children of Cousin 196: {{442,11},{505,12},{586,13},{593,13},{597,14},{598,14},{599,14}}

Children of Cousin 197: {{441,11},{587,13},{588,13},{594,13},{600,14},{601,14},{602,14}}

Children of Cousin 198: {{440,11},{506,12},{586,11},{589,13},{600,13},{603,14}}

Children of Cousin 199: {{439,11},{507,12},{587,11},{590,13},{595,13},{597,13},{604,14}}

Children of Cousin 200: {{508,12},{591,13},{598,13},{601,13},{604,13}}

Children of Cousin 201: {{502,11},{509,12},{592,13},{596,13},{599,13},{602,13},{603,13}}

Children of Cousin 202: {{515,12},{560,12},{605,14},{606,14},{607,14},{608,13},{608,14}}

Children of Cousin 203: {{497,10},{511,12},{609,14},{610,14},{611,14},{612,13},{612,14}}

Children of Cousin 204: {{512,12},{513,12},{556,10},{556,12},{558,12},{586,12},{605,13},{606,13},{609,13},{611,13},{613,14}}

Children of Cousin 205: {{514,12},{557,12},{559,12},{587,12},{607,13},{610,13},{613,13}}

Children of Cousin 206: {{518,12},{523,12},{564,12},{614,14},{615,14},{616,14},{617,14},{618,13},{618,14}}

Children of Cousin 207: {{498,10},{519,12},{617,13},{619,14},{620,14},{621,14},{622,13},{622,14}}

Children of Cousin 208: {{520,12},{522,12},{561,10},{561,12},{563,12},{616,13},{619,13},{621,13},{623,13},{623,14}}

Children of Cousin 209: {{521,12},{557,10},{562,12},{614,13},{615,13},{620,13},{624,13},{624,14}}

Children of Cousin 210: {{526,12},{625,14},{626,14},{627,14},{628,14}}

Children of Cousin 211: {{467,10},{581,12},{588,12},{614,12},{625,13},{629,14},{630,14},{631,14},{632,14}}

Children of Cousin 212: {{474,10},{474,11},{527,12},{558,10},{589,12},{615,12},{626,13},{629,13},{633,14},{634,14},{635,14}}

Children of Cousin 213: {{477,10},{477,11},{528,12},{563,10},{590,12},{616,12},{636,14},{637,14}}

Children of Cousin 214: {{472,10},{472,11},{496,10},{617,12},{627,13},{633,13},{636,13},{638,14},{639,14}}

Children of Cousin 215: {{467,11},{529,12},{618,11},{618,12},{630,13},{634,13},{640,14}}

Children of Cousin 216: {{523,11},{530,12},{582,12},{591,12},{628,13},{631,13},{637,13},{638,13},{640,13}}

Children of Cousin 217: {{531,12},{583,12},{592,12},{632,13},{635,13},{639,13}}

Children of Cousin 218: {{641,14},{642,14},{643,14},{644,14}}

Children of Cousin 219: {{468,10},{581,10},{605,12},{641,13},{645,14},{646,14},{647,14},{648,14}}

Children of Cousin 220: {{475,11},{559,10},{606,12},{649,14},{650,14}}

Children of Cousin 221: {{475,10},{562,10},{607,12},{642,13},{645,13},{651,14}}

Children of Cousin 222: {{468,11},{608,11},{608,12},{643,13},{646,13},{649,13},{652,14}}

Children of Cousin 223: {{584,12},{647,13},{651,13},{652,13}}

Children of Cousin 224: {{515,11},{585,12},{644,13},{648,13},{650,13}}

Children of Cousin 225: {{533,12},{565,12},{593,12},{619,12},{641,12},{653,14},{654,14},{655,14},{656,14}}

Children of Cousin 226: {{566,12},{594,12},{620,12},{657,14},{658,14}}

Children of Cousin 227: {{534,12},{567,12},{595,12},{621,12},{642,12},{653,13},{659,14}}

Children of Cousin 228: {{622,11},{622,12},{654,13},{659,13},{660,14}}

Children of Cousin 229: {{535,12},{568,12},{617,11},{643,12},{655,13},{657,13}}

Children of Cousin 230: {{536,12},{569,12},{596,12},{644,12},{656,13},{658,13},{660,13}}

Children of Cousin 231: {{538,12},{570,12},{609,12},{661,14},{662,14}}

Children of Cousin 232: {{571,12},{610,12},{625,12},{663,14},{664,14}}

Children of Cousin 233: {{539,12},{572,12},{611,12},{626,12},{663,13},{665,14}}

Children of Cousin 234: {{612,11},{612,12},{627,12},{661,13},{665,13},{666,14}}

Children of Cousin 235: {{540,12},{573,12},{628,12},{662,13},{664,13},{666,13}}

Children of Cousin 236: {{476,11},{542,12},{564,10},{574,12},{597,12},{613,12},{623,11},{623,12},{645,12},{653,12},{667,14},{668,14}}

Children of Cousin 237: {{471,11},{495,10},{611,11},{621,11},{654,12},{661,12},{667,13},{670,14},{671,14}}

Children of Cousin 238: {{465,11},{543,12},{574,10},{606,11},{616,11},{646,12},{655,12},{672,14}}

Children of Cousin 239: {{522,11},{544,12},{565,10},{582,10},{598,12},{647,12},{662,12},{668,13},{670,13},{672,13}}

Children of Cousin 240: {{513,11},{545,12},{570,10},{583,10},{599,12},{648,12},{656,12},{671,13}}

Children of Cousin 241: {{473,11},{560,10},{575,12},{600,12},{613,11},{624,11},{624,12},{629,12},{663,12},{673,14},{674,14}}

Children of Cousin 242: {{466,11},{575,10},{607,11},{615,11},{630,12},{657,12},{673,13},{676,14}}

Children of Cousin 243: {{521,11},{571,10},{584,10},{601,12},{631,12},{664,12},{676,13}}

Children of Cousin 244: {{514,11},{566,10},{585,10},{602,12},{632,12},{658,12},{674,13}}

Children of Cousin 245: {{469,11},{493,10},{609,11},{620,11},{633,12},{665,12},{677,14}}

Children of Cousin 246: {{464,11},{547,12},{576,12},{605,11},{614,11},{634,12},{649,12},{673,12}}

Children of Cousin 247: {{482,10},{512,11},{548,12},{577,12},{603,12},{635,12},{650,12},{674,12},{677,13}}

Children of Cousin 248: {{470,11},{494,10},{610,11},{619,11},{636,12},{659,12},{667,12},{678,14}}

Children of Cousin 249: {{483,10},{520,11},{550,12},{578,12},{604,12},{637,12},{651,12},{668,12},{678,13}}

Children of Cousin 250: {{499,10},{519,11},{638,12},{666,12},{670,12},{678,12}}

Children of Cousin 251: {{500,10},{511,11},{639,12},{660,12},{671,12},{677,12}}

Children of Cousin 252: {{518,11},{552,12},{579,12},{640,12},{652,12},{672,12},{676,12}}

Children of Cousin 253: {{485,11},{491,11},{500,11},{679,14},{680,14},{681,14}}

Children of Cousin 254: {{484,11},{490,11},{499,11},{681,13},{682,14},{683,14}}

Children of Cousin 255: {{437,11},{488,11},{489,11},{582,11},{585,11},{682,13},{683,13},{684,14}}

Children of Cousin 256: {{438,11},{487,11},{583,11},{584,11},{679,13},{680,13},{684,13}}

Children of Cousin 257: {{495,11},{567,11},{572,11},{579,11},{679,11},{682,11}}

Children of Cousin 258: {{496,11},{568,11},{577,11},{578,11},{680,11},{683,11}}

Children of Cousin 259: {{569,11},{573,11},{681,11}}

Children of Cousin 260: {{444,10},{503,11},{685,14},{686,14},{687,14},{688,14},{689,14}}

Children of Cousin 261: {{504,11},{690,14},{691,14},{692,14},{693,14}}

Children of Cousin 262: {{449,10},{505,11},{603,11},{690,13},{694,14},{695,14},{696,14},{697,14}}

Children of Cousin 263: {{457,10},{457,11},{507,11},{602,11},{685,13},{691,13},{694,13},{698,14},{699,14},{700,14}}

Children of Cousin 264: {{461,10},{461,11},{506,11},{599,11},{686,13},{696,11},{701,14}}

Children of Cousin 265: {{454,10},{454,11},{596,11},{692,13},{693,11},{698,13},{701,13},{702,14}}

Children of Cousin 266: {{449,11},{592,11},{687,13},{688,11},{695,13},{699,13}}

Children of Cousin 267: {{509,11},{688,13},{693,13},{696,13}}

Children of Cousin 268: {{508,11},{689,13},{697,13},{700,13},{702,13}}

Children of Cousin 269: {{702,11},{703,14},{704,14}}

Children of Cousin 270: {{450,10},{604,11},{700,11},{703,13},{705,14},{706,14},{707,14}}

Children of Cousin 271: {{458,10},{598,11},{697,11},{705,13}}

Children of Cousin 272: {{458,11},{601,11},{704,13},{707,11},{708,14}}

Children of Cousin 273: {{450,11},{591,11},{689,11},{706,13},{708,13}}

Children of Cousin 274: {{707,13}}

Children of Cousin 275: {{526,11},{709,14},{710,14},{711,14}}

Children of Cousin 276: {{439,10},{528,11},{567,10},{672,11},{685,12},{712,14},{713,14}}

Children of Cousin 277: {{440,10},{527,11},{572,10},{676,11},{686,12},{709,13},{714,14},{715,14}}

Children of Cousin 278: {{441,10},{529,11},{640,11},{714,13},{716,11},{716,14}}

Children of Cousin 279: {{442,10},{652,11},{687,12},{710,13},{712,13},{717,11},{717,14}}

Children of Cousin 280: {{531,11},{679,10},{688,12},{715,13},{717,12},{717,13}}

Children of Cousin 281: {{530,11},{552,11},{682,10},{689,12},{711,13},{713,13},{716,12},{716,13}}

Children of Cousin 282: {{491,10},{538,11},{677,11},{703,12},{718,14},{719,14}}

Children of Cousin 283: {{539,11},{671,11},{679,12},{704,12},{709,12},{720,14}}

Children of Cousin 284: {{660,11},{720,13},{721,11},{721,14}}

Children of Cousin 285: {{639,11},{680,12},{710,12},{718,13}}

Children of Cousin 286: {{540,11},{681,12},{702,12},{711,12},{719,13},{721,12},{721,13}}

Children of Cousin 287: {{490,10},{533,11},{678,11},{690,12},{722,14},{723,14},{724,14}}

Children of Cousin 288: {{534,11},{670,11},{682,12},{691,12},{722,13},{725,14}}

Children of Cousin 289: {{666,11},{692,12},{725,13},{726,14},{727,11},{727,14}}

Children of Cousin 290: {{535,11},{638,11},{683,12},{723,13},{726,13}}

Children of Cousin 291: {{536,11},{681,10},{693,12},{724,13},{727,12},{727,13}}

Children of Cousin 292: {{445,10},{489,10},{542,11},{568,10},{668,11},{674,11},{694,12},{705,12},{722,12},{728,14},{729,11},{729,14}}

Children of Cousin 293: {{446,10},{488,10},{543,11},{637,11},{650,11},{706,12},{713,11},{723,12}}

Children of Cousin 294: {{447,10},{487,10},{635,11},{651,11},{695,12},{715,11},{718,12},{728,13}}

Children of Cousin 295: {{485,10},{545,11},{548,11},{680,10},{696,12},{707,12},{715,12},{724,12}}

Children of Cousin 296: {{484,10},{544,11},{550,11},{683,10},{697,12},{700,12},{713,12},{719,12},{729,12},{729,13}}

Children of Cousin 297: {{451,10},{569,10},{658,11},{662,11},{698,12},{719,11},{725,12}}

Children of Cousin 298: {{455,10},{632,11},{647,11},{684,12},{699,12},{712,12},{728,12}}

Children of Cousin 299: {{452,10},{573,10},{656,11},{664,11},{701,12},{720,12},{724,11},{731,14}}

Children of Cousin 300: {{459,10},{547,11},{631,11},{648,11},{684,10},{708,12},{714,12},{731,13}}

Children of Cousin 301: {{453,10},{628,11},{644,11},{711,11},{726,12},{731,12}}

Children of Cousin 302:  $\{\{436,11\},\{576,11\},\{581,11\},\{684,11\}\}$

Children of Cousin 303:  $\{\{445,11\},\{462,11\},\{588,11\},\{699,11\},\{708,11\},\{732,14\},\{733,14\}\}$

Children of Cousin 304:  $\{\{446,11\},\{456,11\},\{590,11\},\{685,11\},\{706,11\},\{733,12\}\}$

Children of Cousin 305:  $\{\{447,11\},\{460,11\},\{589,11\},\{686,11\},\{695,11\},\{732,13\}\}$

Children of Cousin 306:  $\{\{448,11\},\{687,11\},\{733,13\}\}$

Children of Cousin 307:  $\{\{451,11\},\{594,11\},\{698,11\},\{703,11\},\{734,14\}\}$

Children of Cousin 308:  $\{\{452,11\},\{593,11\},\{690,11\},\{701,11\},\{735,14\}\}$

Children of Cousin 309:  $\{\{453,11\},\{595,11\},\{691,11\},\{704,11\},\{734,12\},\{735,13\}\}$

Children of Cousin 310:  $\{\{692,11\},\{734,13\}\}$

Children of Cousin 311:  $\{\{455,11\},\{459,11\},\{597,11\},\{600,11\},\{694,11\},\{705,11\},\{732,12\},\{735,12\}\}$

Children of Cousin 312:  $\{\{478,11\},\{625,11\},\{641,11\},\{731,11\},\{737,14\},\{738,14\}\}$

Children of Cousin 313:  $\{\{479,10\},\{479,11\},\{626,11\},\{642,11\},\{709,11\},\{737,13\},\{739,14\}\}$

Children of Cousin 314:  $\{\{627,11\},\{726,11\},\{739,13\},\{740,11\},\{740,14\}\}$

Children of Cousin 315:  $\{\{471,10\},\{643,11\},\{710,11\},\{738,13\},\{740,12\},\{740,13\}\}$

Children of Cousin 316:  $\{\{464,10\},\{480,10\},\{480,11\},\{576,10\},\{629,11\},\{645,11\},\{673,11\},\{728,11\},\{732,11\},\{737,12\},\{741,11\},\{741,14\}\}$

Children of Cousin 317:  $\{\{465,10\},\{476,10\},\{646,11\},\{649,11\},\{712,11\},\{733,11\},\{738,12\}\}$

Children of Cousin 318:  $\{\{466,10\},\{473,10\},\{630,11\},\{634,11\},\{714,11\},\{741,12\},\{741,13\}\}$

Children of Cousin 319:  $\{\{469,10\},\{577,10\},\{633,11\},\{657,11\},\{718,11\},\{739,12\}\}$

Children of Cousin 320:  $\{\{470,10\},\{578,10\},\{636,11\},\{655,11\},\{723,11\},\{738,11\}\}$

Children of Cousin 321:  $\{\{478,10\},\{579,10\},\{653,11\},\{663,11\},\{667,11\},\{722,11\},\{735,11\},\{737,11\},\{743,11\},\{743,14\}\}$

Children of Cousin 322:  $\{\{654,11\},\{659,11\},\{720,11\},\{743,12\},\{743,13\}\}$

Children of Cousin 323:  $\{\{661,11\},\{665,11\},\{725,11\},\{734,11\},\{739,11\}\}$

Children of Cousin 324:  $\{\{85,3\},\{481,10\},\{580,10\},\{669,11\},\{675,11\},\{730,11\},\{736,11\},\{742,11\},\{744,11\}\}$

Children of Cousin 325:  $\{\{709,10\},\{745,14\},\{746,13\},\{746,14\},\{747,14\}\}$

Children of Cousin 326:  $\{\{526,10\},\{710,10\},\{745,13\},\{748,14\},\{749,14\},\{750,14\}\}$

Children of Cousin 327:  $\{\{711,10\},\{748,13\},\{751,13\},\{751,14\},\{752,14\}\}$

Children of Cousin 328:  $\{\{747,13\},\{749,13\},\{752,13\}\}$

Children of Cousin 329:  $\{\{750,13\}\}$

Children of Cousin 330:  $\{\{597,10\},\{712,10\},\{753,14\},\{754,14\},\{755,14\},\{756,14\},\{757,14\}\}$

Children of Cousin 331:  $\{\{534,10\},\{713,10\},\{758,14\},\{759,14\},\{760,14\},\{761,14\}\}$

Children of Cousin 332:  $\{\{595,10\},\{753,13\},\{758,13\}\}$

Children of Cousin 333:  $\{\{528,10\},\{590,10\},\{621,10\},\{759,13\},\{762,10\},\{762,14\},\{763,14\},\{764,14\}\}$

Children of Cousin 334:  $\{\{587,10\},\{642,10\},\{754,13\},\{765,14\},\{766,14\}\}$

Children of Cousin 335:  $\{\{507,10\},\{685,10\},\{755,13\},\{758,10\},\{760,13\},\{762,11\},\{762,13\},\{765,13\},\{767,14\}\}$

Children of Cousin 336:  $\{\{653,10\},\{672,10\},\{753,10\},\{756,13\},\{761,13\},\{763,13\},\{766,13\},\{768,14\}\}$

Children of Cousin 337:  $\{\{604,10\},\{659,10\},\{757,13\},\{764,13\},\{767,13\},\{768,13\}\}$

Children of Cousin 338:  $\{\{600,10\},\{714,10\},\{754,11\},\{769,14\},\{770,14\},\{771,14\}\}$

Children of Cousin 339:  $\{\{539,10\},\{715,10\},\{745,11\},\{772,14\},\{773,14\}\}$

Children of Cousin 340: {{527,10},{589,10},{611,10},{745,12},{769,13},{772,13},{774,10},{774,14},{775,14},{776,14}}

Children of Cousin 341: {{586,10},{626,10},{745,10},{746,10},{746,12},{754,12},{777,14},{778,14},{779,14}}

Children of Cousin 342: {{506,10},{686,10},{773,13},{774,11},{774,13},{777,13},{780,14}}

Children of Cousin 343: {{663,10},{676,10},{770,13},{775,13},{778,13}}

Children of Cousin 344: {{603,10},{665,10},{747,12},{771,13},{776,13},{779,13},{780,13}}

Children of Cousin 345: {{716,10},{781,14},{782,14}}

Children of Cousin 346: {{594,10},{644,10},{781,13},{783,14},{784,14}}

Children of Cousin 347: {{529,10},{588,10},{643,10},{769,12},{782,13},{785,14},{786,14},{787,14}}

Children of Cousin 348: {{640,10},{641,10},{766,11},{770,12},{782,10},{783,13},{785,13},{788,14}}

Children of Cousin 349: {{602,10},{765,11},{771,12},{781,10},{784,13},{786,13}}

Children of Cousin 350: {{601,10},{787,13},{788,13}}

Children of Cousin 351: {{717,10},{746,11},{789,14},{790,14}}

Children of Cousin 352: {{593,10},{628,10},{748,12},{753,12},{789,13},{791,14},{792,14},{793,14}}

Children of Cousin 353: {{505,10},{627,10},{687,10},{755,12},{779,11},{790,10},{790,13},{791,13},{794,14},{795,14}}

Children of Cousin 354: {{625,10},{652,10},{756,12},{778,11},{788,10},{792,13}}

Children of Cousin 355: {{599,10},{749,12},{777,11},{793,13},{794,13}}

Children of Cousin 356: {{598,10},{750,12},{757,12},{788,11},{789,10},{795,13}}

Children of Cousin 357: {{704,10},{789,12},{796,14}}

Children of Cousin 358: {{531,10},{671,10},{772,12},{797,14},{798,14}}

Children of Cousin 359: {{688,10},{747,11},{773,12},{790,11},{790,12},{796,13},{797,13},{799,14}}

Children of Cousin 360: {{720,10},{789,11},{798,13},{799,13}}

Children of Cousin 361: {{691,10},{751,10},{751,12},{758,12},{781,12},{800,14},{801,14},{802,14}}

Children of Cousin 362: {{530,10},{670,10},{748,10},{759,12},{782,12},{803,14},{804,14},{805,14}}

Children of Cousin 363: {{689,10},{760,12},{800,13},{803,13},{806,14}}

Children of Cousin 364: {{552,10},{722,10},{761,12},{782,11},{801,13},{804,13}}

Children of Cousin 365: {{725,10},{752,12},{781,11},{802,13},{805,13},{806,13}}

Children of Cousin 366: {{504,10},{726,10},{758,11},{791,12},{796,12},{800,12},{807,14}}

Children of Cousin 367: {{731,10},{735,10},{753,11},{783,12},{792,12},{801,12}}

Children of Cousin 368: {{596,10},{734,10},{752,10},{784,12},{793,12},{802,12},{807,13}}

Children of Cousin 369: {{503,10},{740,10},{762,12},{774,12},{797,12},{803,12}}

Children of Cousin 370: {{518,10},{667,10},{738,10},{763,12},{768,10},{775,12},{785,12},{804,12}}

Children of Cousin 371: {{592,10},{661,10},{749,10},{776,12},{786,12},{797,10},{805,12}}

Children of Cousin 372: {{591,10},{654,10},{750,10},{764,12},{768,11},{787,12},{798,12},{803,10}}

Children of Cousin 373: {{502,10},{739,10},{747,10},{765,12},{777,12},{779,12},{808,13},{808,14}}

Children of Cousin 374: {{737,10},{766,12},{778,12}}

Children of Cousin 375: {{509,10},{780,12},{794,12},{797,11},{806,12},{807,12},{808,11},{808,12}}

Children of Cousin 376: {{508,10},{767,12},{795,12},{799,12},{803,11}}

Children of Cousin 377: {{743,10},{768,12},{788,12}}



Children of Cousin 378: {{511,10},{548,10},{718,10},{772,11},{780,10},{809,14}}

Children of Cousin 379: {{536,10},{719,10},{807,10},{810,14},{811,14}}

Children of Cousin 380: {{538,10},{545,10},{639,10},{794,10},{809,11},{810,13}}

Children of Cousin 381: {{660,10},{703,10},{798,11},{806,10},{811,13}}

Children of Cousin 382: {{516,10},{677,10},{808,10},{809,13}}

Children of Cousin 383: {{519,10},{550,10},{723,10},{759,11},{767,10},{812,14},{813,14}}

Children of Cousin 384: {{540,10},{724,10},{748,11},{810,11},{814,14}}

Children of Cousin 385: {{533,10},{544,10},{638,10},{761,11},{791,10},{795,10},{810,12},{812,13},{813,11}}

Children of Cousin 386: {{666,10},{690,10},{791,11},{799,10},{801,11},{805,11},{814,13}}

Children of Cousin 387: {{524,10},{678,10},{804,11},{813,13}}

Children of Cousin 388: {{547,10},{728,10},{732,10},{769,11},{815,10},{815,14},{816,14},{817,14}}

Children of Cousin 389: {{535,10},{729,10},{812,11},{818,14}}

Children of Cousin 390: {{542,10},{543,10},{617,10},{733,10},{755,10},{761,10},{812,12},{819,14},{820,14}}

Children of Cousin 391: {{694,10},{699,10},{755,11},{771,11},{786,11},{801,10},{815,11},{815,13},{818,13}}

Children of Cousin 392: {{705,10},{708,10},{757,11},{787,11},{818,10}}

Children of Cousin 393: {{523,10},{655,10},{668,10},{757,10},{785,11},{804,10},{812,10},{816,13},{819,13}}

Children of Cousin 394: {{515,10},{657,10},{674,10},{771,10},{817,13},{820,13}}

Children of Cousin 395: {{622,10},{706,10},{760,10},{764,11}}

Children of Cousin 396: {{522,10},{619,10},{637,10},{759,10},{763,11},{764,10},{813,12},{819,11}}

Children of Cousin 397: {{514,10},{620,10},{650,10},{765,10},{820,11}}

Children of Cousin 398: {{612,10},{695,10},{773,10},{776,11},{815,12}}

Children of Cousin 399: {{521,10},{610,10},{651,10},{775,11},{816,12}}

Children of Cousin 400: {{513,10},{609,10},{635,10},{772,10},{776,10},{777,10},{809,12},{817,12}}

Children of Cousin 401: {{696,10},{749,11},{773,11},{780,11},{794,11},{814,12}}

Children of Cousin 402: {{707,10},{750,11}}

Children of Cousin 403: {{697,10},{795,11},{796,10},{818,12}}

Children of Cousin 404: {{700,10},{760,11},{767,11},{800,10},{811,12},{818,11}}

Children of Cousin 405: {{520,10},{636,10},{813,10},{819,12}}

Children of Cousin 406: {{512,10},{633,10},{779,10},{809,10},{820,12}}

Children of Cousin 407: {{721,10},{821,14}}

Children of Cousin 408: {{702,10},{811,11},{821,13},{822,14}}

Children of Cousin 409: {{796,11},{799,11},{806,11},{821,10},{822,13}}

Children of Cousin 410: {}

Children of Cousin 411: {{727,10},{751,11},{821,11},{823,14}}

Children of Cousin 412: {{693,10},{752,11},{807,11},{814,11},{821,12},{822,11},{823,11},{823,12}}

Children of Cousin 413: {{692,10},{802,11},{822,12},{823,10},{823,13}}

Children of Cousin 414: {{800,11},{822,10}}

Children of Cousin 415: {{698,10},{784,11},{802,10},{811,10}}

Children of Cousin 416:  $\{\{656,10\},\{662,10\},\{783,11\},\{793,10\},\{798,10\},\{805,10\},\{810,10\}\}$

Children of Cousin 417:  $\{\{658,10\},\{784,10\}\}$

Children of Cousin 418:  $\{\{701,10\},\{793,11\},\{814,10\}\}$

Children of Cousin 419:  $\{\{664,10\},\{792,11\}\}$

Children of Cousin 420:  $\{\{631,10\},\{647,10\},\{756,11\},\{770,11\},\{787,10\},\{792,10\},\{816,11\}\}$

Children of Cousin 421:  $\{\{632,10\},\{648,10\},\{783,10\},\{786,10\},\{817,11\}\}$

Children of Cousin 422:  $\{\{673,10\},\{741,10\},\{824,10\},\{824,14\},\{825,14\}\}$

Children of Cousin 423:  $\{\{605,10\},\{629,10\},\{634,10\},\{769,10\},\{778,10\},\{817,10\},\{824,11\},\{824,13\},\{825,13\},\{826,14\}\}$

Children of Cousin 424:  $\{\{614,10\},\{645,10\},\{649,10\},\{766,10\},\{816,10\},\{825,10\},\{826,13\}\}$

Children of Cousin 425:  $\{\{618,10\},\{646,10\},\{756,10\},\{785,10\},\{826,12\}\}$

Children of Cousin 426:  $\{\{606,10\},\{613,10\},\{615,10\},\{754,10\},\{775,10\},\{820,10\},\{825,11\},\{826,11\}\}$

Children of Cousin 427:  $\{\{616,10\},\{623,10\},\{763,10\},\{819,10\}\}$

Children of Cousin 428:  $\{\{608,10\},\{630,10\},\{770,10\},\{824,12\},\{826,10\}\}$

Children of Cousin 429:  $\{\{607,10\},\{624,10\},\{825,12\}\}$

Children of Cousin 430:  $\{\{827,15\},\{828,15\},\{829,15\},\{830,15\}\}$

Children of Cousin 431:  $\{\{827,14\},\{829,13\},\{832,15\}\}$

Children of Cousin 432:  $\{\{828,13\},\{833,15\}\}$

Children of Cousin 433:  $\{\{828,14\},\{834,15\}\}$

Children of Cousin 434:  $\{\{829,14\}\}$

Children of Cousin 435:  $\{\{830,14\},\{832,14\},\{833,14\},\{834,13\},\{834,14\}\}$

Children of Cousin 436:  $\{\{827,13\},\{836,15\}\}$

Children of Cousin 437:  $\{\{830,13\},\{833,13\},\{836,14\}\}$

Children of Cousin 438:  $\{\{832,13\},\{836,13\}\}$

Children of Cousin 439:  $\{\{838,15\},\{839,15\},\{840,15\}\}$

Children of Cousin 440:  $\{\{841,15\},\{842,15\},\{843,15\}\}$

Children of Cousin 441:  $\{\{841,14\},\{844,15\}\}$

Children of Cousin 442:  $\{\{838,14\},\{845,15\}\}$

Children of Cousin 443:  $\{\{839,14\},\{842,14\},\{844,14\},\{846,12\},\{846,15\}\}$

Children of Cousin 444:  $\{\{840,14\},\{843,14\},\{845,14\},\{846,13\},\{846,14\}\}$

Children of Cousin 445:  $\{\{830,10\},\{849,15\},\{850,15\},\{851,15\},\{852,15\}\}$

Children of Cousin 446:  $\{\{833,10\},\{854,15\},\{855,12\},\{855,15\}\}$

Children of Cousin 447:  $\{\{832,10\},\{849,14\},\{856,12\},\{856,15\}\}$

Children of Cousin 448:  $\{\{834,10\},\{834,12\},\{845,12\},\{850,14\},\{854,14\}\}$

Children of Cousin 449:  $\{\{845,13\},\{851,14\},\{856,13\},\{856,14\}\}$

Children of Cousin 450:  $\{\{852,14\},\{855,13\},\{855,14\}\}$

Children of Cousin 451:  $\{\{858,12\},\{858,15\}\}$

Children of Cousin 452:  $\{\{859,15\},\{860,12\},\{860,15\}\}$

Children of Cousin 453:  $\{\{859,14\}\}$

Children of Cousin 454: {{858,14},{860,14}}

Children of Cousin 455: {{836,10},{838,13},{849,13},{851,12}}

Children of Cousin 456: {{833,12},{839,13},{840,12},{850,13}}

Children of Cousin 457: {{840,13},{851,13},{858,13}}

Children of Cousin 458: {{852,13}}

Children of Cousin 459: {{836,12},{841,13},{852,12},{859,13},{863,15}}

Children of Cousin 460: {{832,12},{842,13},{843,12},{863,14}}

Children of Cousin 461: {{843,13},{860,13}}

Children of Cousin 462: {{830,12},{844,13},{854,13},{863,13}}

Children of Cousin 463: {{146,4},{835,12},{847,13},{848,12},{857,13},{862,13},{865,13},{866,13}}

Children of Cousin 464: {{827,12},{863,12},{867,15},{868,15},{869,15}}

Children of Cousin 465: {{828,12},{854,12},{871,12},{871,15}}

Children of Cousin 466: {{829,12},{867,14},{872,12},{872,15}}

Children of Cousin 467: {{844,12},{868,14},{872,13},{872,14}}

Children of Cousin 468: {{869,14},{871,13},{871,14}}

Children of Cousin 469: {{873,12},{873,15}}

Children of Cousin 470: {{874,15},{875,12},{875,15}}

Children of Cousin 471: {{874,14}}

Children of Cousin 472: {{873,14},{875,14}}

Children of Cousin 473: {{829,10},{841,12},{867,13},{868,12}}

Children of Cousin 474: {{842,12},{868,13},{873,13}}

Children of Cousin 475: {{869,13}}

Children of Cousin 476: {{828,10},{838,12},{850,12},{869,12},{874,13}}

Children of Cousin 477: {{839,12},{875,13}}

Children of Cousin 478: {{859,12},{874,12},{878,12},{878,15}}

Children of Cousin 479: {{878,14}}

Children of Cousin 480: {{827,10},{849,12},{867,12},{878,13}}

Children of Cousin 481: {{158,6},{831,10},{837,10},{837,12},{853,12},{861,12},{864,12},{870,12},{876,12},{877,12},{879,13},{880,12}}

Children of Cousin 482: {{881,15},{882,11},{882,15},{883,15},{884,15},{885,15},{886,15}}

Children of Cousin 483: {{888,15},{889,11},{889,15},{890,15},{891,15},{892,15},{893,15}}

Children of Cousin 484: {{888,14},{895,15},{896,15},{897,15},{898,15}}

Children of Cousin 485: {{881,14},{900,15},{901,15},{902,15}}

Children of Cousin 486: {{834,11},{882,14},{889,14},{895,14},{900,14},{904,15}}

Children of Cousin 487: {{832,11},{883,14},{890,14},{901,14},{906,15},{907,15}}

Children of Cousin 488: {{833,11},{884,14},{891,14},{896,14},{904,14},{909,15}}

Children of Cousin 489: {{830,11},{885,14},{892,14},{897,14},{904,11},{906,14},{911,15}}

Children of Cousin 490: {{893,14},{895,11},{902,14},{909,14},{911,14}}

Children of Cousin 491: {{886,14},{898,14},{900,11},{907,14}}

Children of Cousin 492: {{163,1},{835,11},{887,1},{894,1},{899,1},{903,1},{905,1},{908,1},{910,1},{912,1},{914,1},{915,1}}

Children of Cousin 493: {{886,12},{916,15},{917,15},{918,15}}

Children of Cousin 494: {{893,12},{920,15},{921,15},{922,15},{923,15}}

Children of Cousin 495: {{920,14},{925,15},{926,15},{927,15},{928,15}}

Children of Cousin 496: {{916,14},{921,14},{930,15},{931,15},{932,15}}

Children of Cousin 497: {{881,12},{917,14},{922,14},{925,14}}

Children of Cousin 498: {{888,12},{918,14},{923,14},{926,14},{930,14}}

Children of Cousin 499: {{888,11},{893,11},{927,14},{931,14}}

Children of Cousin 500: {{881,11},{886,11},{928,14},{932,14}}

Children of Cousin 501: {{164,1},{919,1},{924,1},{929,1},{933,1},{934,1},{935,1},{936,1},{937,1}}

Children of Cousin 502: {{938,15},{939,15},{940,15},{941,12},{941,15}}

Children of Cousin 503: {{846,10},{846,11},{943,15},{944,15},{945,15},{946,15}}

Children of Cousin 504: {{948,15},{949,15},{950,15}}

Children of Cousin 505: {{845,11},{938,14},{948,14},{952,15},{953,15},{954,15}}

Children of Cousin 506: {{843,11},{939,14},{943,14},{956,15}}

Children of Cousin 507: {{840,11},{940,14},{944,14},{949,14},{952,14},{958,15}}

Children of Cousin 508: {{945,14},{953,14},{958,14}}

Children of Cousin 509: {{941,11},{941,14},{946,14},{950,14},{954,14},{956,14}}

Children of Cousin 510: {{165,1},{848,11},{942,1},{947,1},{951,1},{955,1},{957,1},{959,1},{960,1},{961,1}}

Children of Cousin 511: {{881,13},{962,15},{963,15}}

Children of Cousin 512: {{882,10},{882,13},{916,13},{938,13},{962,14},{965,15},{966,15},{967,15}}

Children of Cousin 513: {{883,13},{917,13},{939,13},{963,14},{967,12},{969,15}}

Children of Cousin 514: {{884,13},{918,13},{940,13},{965,14}}

Children of Cousin 515: {{885,13},{966,14},{969,14}}

Children of Cousin 516: {{886,13},{941,13},{967,14}}

Children of Cousin 517: {{166,1},{887,13},{919,13},{942,13},{964,1},{968,1},{970,1},{971,1},{972,1},{973,1}}

Children of Cousin 518: {{920,13},{974,15},{975,15},{976,15},{977,15}}

Children of Cousin 519: {{888,13},{979,15},{980,15},{981,15}}

Children of Cousin 520: {{889,10},{889,13},{921,13},{979,14},{983,15},{984,15},{985,15}}

Children of Cousin 521: {{890,13},{922,13},{974,14},{987,15}}

Children of Cousin 522: {{891,13},{923,13},{975,14},{980,14},{983,14},{985,12}}

Children of Cousin 523: {{892,13},{976,14},{977,12},{981,14},{984,14},{987,14}}

Children of Cousin 524: {{893,13},{977,14},{985,14}}

Children of Cousin 525: {{167,1},{894,13},{924,13},{978,1},{982,1},{986,1},{988,1},{989,1},{990,1},{991,1}}

Children of Cousin 526: {{992,15},{993,15}}

Children of Cousin 527: {{842,10},{925,13},{943,13},{974,13},{992,14},{995,15},{996,15}}

Children of Cousin 528: {{839,10},{926,13},{944,13},{975,13},{998,15}}

Children of Cousin 529: {{844,10},{976,13},{995,14},{1000,15}}

Children of Cousin 530: {{927,13},{945,13},{977,13},{993,14},{998,14},{1000,14}}

Children of Cousin 531: {{928,13},{946,13},{996,14}}

Children of Cousin 532: {{168,1},{847,10},{929,13},{947,13},{978,13},{994,1},{997,1},{999,1},{1001,1},{1002,1},{1003,1}}

Children of Cousin 533: {{895,13},{948,13},{979,13},{1004,15},{1005,15},{1006,15}}

Children of Cousin 534: {{896,13},{949,13},{980,13},{1004,14}}

Children of Cousin 535: {{897,13},{981,13},{1005,14}}

Children of Cousin 536: {{898,13},{950,13},{1006,14}}

Children of Cousin 537: {{169,1},{899,13},{951,13},{982,13},{1007,1},{1008,1},{1009,1},{1010,1}}

Children of Cousin 538: {{900,13},{962,13},{1011,15}}

Children of Cousin 539: {{901,13},{963,13},{992,13}}

Children of Cousin 540: {{902,13},{993,13},{1011,14}}

Children of Cousin 541: {{170,1},{903,13},{964,13},{994,13},{1012,1},{1013,1},{1014,1}}

Children of Cousin 542: {{850,10},{904,13},{930,13},{952,13},{965,13},{983,13},{1004,13},{1015,15}}

Children of Cousin 543: {{854,10},{904,10},{966,13},{984,13},{1005,13},{1018,15}}

Children of Cousin 544: {{895,10},{931,13},{953,13},{985,13},{1011,13},{1015,14},{1018,14}}

Children of Cousin 545: {{900,10},{932,13},{954,13},{967,13},{1006,13}}

Children of Cousin 546: {{171,1},{857,10},{905,13},{933,13},{955,13},{968,13},{986,13},{1007,13},{1012,13},{1016,1},{1019,1},{1020,1},{1021,1}}

Children of Cousin 547: {{863,10},{906,13},{969,13},{987,13},{995,13}}

Children of Cousin 548: {{881,10},{907,13},{956,13},{967,11},{996,13}}

Children of Cousin 549: {{172,1},{865,10},{908,13},{934,13},{957,13},{970,13},{988,13},{997,13},{1013,13},{1022,1},{1023,1}}

Children of Cousin 550: {{888,10},{909,13},{958,13},{985,11},{998,13},{1015,13}}

Children of Cousin 551: {{173,1},{862,10},{910,13},{935,13},{959,13},{971,13},{989,13},{999,13},{1008,13},{1016,13},{1024,1}}

Children of Cousin 552: {{911,13},{977,11},{1000,13},{1018,13}}

Children of Cousin 553: {{174,1},{866,10},{912,13},{972,13},{990,13},{1001,13},{1009,13},{1019,13},{1022,13},{1025,1}}

Children of Cousin 554: {{175,1},{914,13},{936,13},{960,13},{991,13},{1002,13},{1014,13},{1020,13},{1024,13},{1025,13}}

Children of Cousin 555: {{176,1},{915,13},{937,13},{961,13},{973,13},{1003,13},{1010,13},{1021,13},{1023,13}}

Children of Cousin 556: {{882,12},{917,12},{1026,15}}

Children of Cousin 557: {{918,12},{922,12},{1027,15},{1028,15}}

Children of Cousin 558: {{883,12},{916,12},{925,12},{1027,14},{1029,15}}

Children of Cousin 559: {{884,12},{1026,14}}

Children of Cousin 560: {{885,12},{1026,11},{1028,14},{1029,14}}

Children of Cousin 561: {{889,12},{923,12},{1031,15}}

Children of Cousin 562: {{890,12},{1028,11},{1032,15}}

Children of Cousin 563: {{891,12},{921,12},{926,12},{1031,14}}

Children of Cousin 564: {{892,12},{920,12},{930,12},{1027,11},{1031,11},{1032,14}}

Children of Cousin 565: {{895,12},{923,11},{1034,15},{1035,15},{1036,15}}

Children of Cousin 566: {{918,11},{1037,15},{1038,13},{1038,15}}

Children of Cousin 567: {{896,12},{926,11},{1034,14}}

Children of Cousin 568: {{897,12},{930,11},{1035,14},{1037,14}}

Children of Cousin 569: {{898,12},{1036,14},{1038,11},{1038,14}}

Children of Cousin 570: {{900,12},{917,11},{1036,13}}

Children of Cousin 571: {{922,11},{1040,15},{1041,13},{1041,15}}

Children of Cousin 572: {{901,12},{925,11},{1040,14}}

Children of Cousin 573: {{902,12},{1036,11},{1041,11},{1041,14}}

Children of Cousin 574: {{828,11},{904,12},{1026,13},{1031,13},{1034,13},{1035,13}}

Children of Cousin 575: {{829,11},{1027,13},{1028,13},{1037,13},{1040,13},{1043,14},{1043,15}}

Children of Cousin 576: {{827,11},{906,12},{1029,13},{1032,13},{1043,11},{1043,13}}

Children of Cousin 577: {{907,12},{916,11},{1037,11}}

Children of Cousin 578: {{909,12},{921,11},{1035,11}}

Children of Cousin 579: {{911,12},{920,11},{1034,11},{1040,11}}

Children of Cousin 580: {{186,4},{831,11},{913,12},{1030,13},{1033,13},{1039,13},{1042,11},{1044,11},{1045,13},{1046,4}}

Children of Cousin 581: {{1029,11},{1032,11},{1047,15},{1048,15}}

Children of Cousin 582: {{891,11},{892,11},{927,12},{931,12},{1047,14}}

Children of Cousin 583: {{883,11},{928,12},{932,12},{1048,14}}

Children of Cousin 584: {{890,11},{1047,13}}

Children of Cousin 585: {{884,11},{885,11},{1048,13}}

Children of Cousin 586: {{938,12},{939,12},{1049,15}}

Children of Cousin 587: {{940,12},{1049,14}}

Children of Cousin 588: {{844,11},{1050,15},{1051,15},{1052,15}}

Children of Cousin 589: {{842,11},{943,12},{1050,14},{1053,15}}

Children of Cousin 590: {{839,11},{944,12},{1054,15}}

Children of Cousin 591: {{945,12},{1051,14},{1054,14}}

Children of Cousin 592: {{946,12},{1052,14},{1053,14}}

Children of Cousin 593: {{948,12},{1055,15},{1056,15}}

Children of Cousin 594: {{1057,15}}

Children of Cousin 595: {{949,12},{1055,14}}

Children of Cousin 596: {{950,12},{1056,14},{1057,14}}

Children of Cousin 597: {{838,11},{952,12},{1049,13},{1055,13},{1058,15}}

Children of Cousin 598: {{953,12},{1058,14}}

Children of Cousin 599: {{939,11},{954,12},{1056,13}}

Children of Cousin 600: {{841,11},{1049,11},{1050,13},{1060,15}}

Children of Cousin 601: {{1051,13}}

Children of Cousin 602: {{940,11},{1052,13},{1057,13},{1060,14}}

Children of Cousin 603: {{938,11},{956,12},{1053,13},{1060,13}}

Children of Cousin 604: {{958,12},{1054,13},{1058,13}}

Children of Cousin 605: {{969,12},{1029,12},{1062,15},{1063,15}}

Children of Cousin 606:  $\{\{966,12\},\{1026,10\},\{1063,13\}\}$

Children of Cousin 607:  $\{\{1028,12\},\{1062,14\}\}$

Children of Cousin 608:  $\{\{1063,14\}\}$

Children of Cousin 609:  $\{\{917,10\},\{962,12\},\{1064,15\}\}$

Children of Cousin 610:  $\{\{922,10\},\{1065,15\}\}$

Children of Cousin 611:  $\{\{925,10\},\{963,12\},\{1064,13\},\{1065,14\}\}$

Children of Cousin 612:  $\{\{1064,14\}\}$

Children of Cousin 613:  $\{\{965,12\},\{1026,12\},\{1027,12\},\{1049,12\},\{1062,13\},\{1065,13\}\}$

Children of Cousin 614:  $\{\{987,12\},\{1032,12\},\{1067,15\},\{1068,15\}\}$

Children of Cousin 615:  $\{\{974,12\},\{1027,10\},\{1067,14\},\{1068,13\},\{1069,15\}\}$

Children of Cousin 616:  $\{\{975,12\},\{984,12\},\{1031,10\},\{1070,15\}\}$

Children of Cousin 617:  $\{\{930,10\},\{981,12\},\{1069,14\},\{1070,14\}\}$

Children of Cousin 618:  $\{\{976,12\},\{1068,14\}\}$

Children of Cousin 619:  $\{\{923,10\},\{979,12\},\{1070,13\},\{1071,15\},\{1072,15\}\}$

Children of Cousin 620:  $\{\{918,10\},\{1069,13\}\}$

Children of Cousin 621:  $\{\{926,10\},\{980,12\},\{1071,14\},\{1072,13\}\}$

Children of Cousin 622:  $\{\{1072,14\}\}$

Children of Cousin 623:  $\{\{983,12\},\{1031,12\},\{1071,13\}\}$

Children of Cousin 624:  $\{\{1028,10\},\{1067,13\}\}$

Children of Cousin 625:  $\{\{1075,15\},\{1076,15\}\}$

Children of Cousin 626:  $\{\{992,12\},\{1075,14\},\{1077,15\}\}$

Children of Cousin 627:  $\{\{1077,14\},\{1078,15\}\}$

Children of Cousin 628:  $\{\{993,12\},\{1076,14\},\{1078,14\}\}$

Children of Cousin 629:  $\{\{868,10\},\{1029,10\},\{1050,12\},\{1067,12\},\{1075,13\},\{1079,15\},\{1080,15\}\}$

Children of Cousin 630:  $\{\{872,10\},\{872,11\},\{1068,12\},\{1079,14\},\{1082,15\}\}$

Children of Cousin 631:  $\{\{987,11\},\{1047,12\},\{1051,12\},\{1076,13\},\{1082,14\}\}$

Children of Cousin 632:  $\{\{1048,12\},\{1052,12\},\{1080,14\}\}$

Children of Cousin 633:  $\{\{873,10\},\{873,11\},\{916,10\},\{1069,12\},\{1077,13\},\{1083,15\}\}$

Children of Cousin 634:  $\{\{868,11\},\{995,12\},\{1068,11\},\{1079,13\}\}$

Children of Cousin 635:  $\{\{883,10\},\{996,12\},\{1053,12\},\{1080,13\},\{1083,14\}\}$

Children of Cousin 636:  $\{\{875,10\},\{875,11\},\{921,10\},\{1070,12\},\{1084,15\}\}$

Children of Cousin 637:  $\{\{891,10\},\{984,11\},\{998,12\},\{1054,12\},\{1084,14\}\}$

Children of Cousin 638:  $\{\{931,10\},\{981,11\},\{1078,13\},\{1084,13\}\}$

Children of Cousin 639:  $\{\{932,10\},\{1083,13\}\}$

Children of Cousin 640:  $\{\{976,11\},\{1000,12\},\{1082,13\}\}$

Children of Cousin 641:  $\{\{1085,15\},\{1086,15\},\{1087,15\}\}$

Children of Cousin 642:  $\{\{1085,14\}\}$

Children of Cousin 643:  $\{\{1086,14\}\}$

Children of Cousin 644: {{1087,14}}

Children of Cousin 645: {{869,10},{1032,10},{1062,12},{1085,13},{1088,15}}

Children of Cousin 646: {{871,10},{871,11},{1063,12},{1086,13},{1090,15}}

Children of Cousin 647: {{1047,10},{1088,14},{1090,14}}

Children of Cousin 648: {{969,11},{1048,10},{1087,13}}

Children of Cousin 649: {{869,11},{1063,11}}

Children of Cousin 650: {{884,10},{966,11}}

Children of Cousin 651: {{890,10},{1088,13}}

Children of Cousin 652: {{1090,13}}

Children of Cousin 653: {{1004,12},{1034,12},{1055,12},{1071,12},{1085,12},{1091,15}}

Children of Cousin 654: {{1072,12},{1091,14},{1093,15}}

Children of Cousin 655: {{1005,12},{1035,12},{1070,11},{1086,12}}

Children of Cousin 656: {{1006,12},{1036,12},{1056,12},{1087,12},{1093,14}}

Children of Cousin 657: {{1037,12},{1069,11}}

Children of Cousin 658: {{1038,10},{1038,12},{1057,12}}

Children of Cousin 659: {{1072,11},{1091,13}}

Children of Cousin 660: {{1093,13}}

Children of Cousin 661: {{1064,12},{1094,15}}

Children of Cousin 662: {{1011,12},{1036,10},{1094,14}}

Children of Cousin 663: {{1040,12},{1065,12},{1075,12}}

Children of Cousin 664: {{1041,10},{1041,12},{1076,12}}

Children of Cousin 665: {{1064,11},{1077,12}}

Children of Cousin 666: {{1078,12},{1094,13}}

Children of Cousin 667: {{874,11},{920,10},{1065,11},{1071,11},{1091,12},{1096,15}}

Children of Cousin 668: {{892,10},{983,11},{1015,12},{1035,10},{1058,12},{1088,12},{1096,14}}

Children of Cousin 669: {{236,3},{877,11},{1017,12},{1033,10},{1042,12},{1059,12},{1066,12},{1073,11},{1073,12},{1089,12},{1092,12},{1097,3},{1098,3}}

Children of Cousin 670: {{927,10},{980,11},{1094,12},{1096,13}}

Children of Cousin 671: {{928,10},{963,11},{1093,12}}

Children of Cousin 672: {{975,11},{1018,12},{1034,10},{1090,12}}

Children of Cousin 673: {{867,11},{1043,10},{1043,12},{1062,11},{1067,11},{1079,12}}

Children of Cousin 674: {{885,10},{965,11},{1037,10},{1060,12},{1080,12}}

Children of Cousin 675: {{241,3},{876,11},{1030,10},{1044,12},{1061,12},{1066,11},{1074,11},{1074,12},{1081,12},{1095,12},{1099,3},{1100,3}}

Children of Cousin 676: {{974,11},{1040,10},{1082,12}}

Children of Cousin 677: {{886,10},{962,11},{1083,12}}

Children of Cousin 678: {{893,10},{979,11},{1084,12},{1096,12}}

Children of Cousin 679: {{901,11},{928,11}}

Children of Cousin 680: {{907,11},{932,11}}

Children of Cousin 681: {{898,11},{902,11}}



Children of Cousin 682:  $\{\{896,11\},\{911,11\},\{927,11\}\}$

Children of Cousin 683:  $\{\{897,11\},\{909,11\},\{931,11\}\}$

Children of Cousin 684:  $\{\{836,11\},\{906,11\},\{1047,11\},\{1048,11\}\}$

Children of Cousin 685:  $\{\{840,10\},\{944,11\},\{1101,15\},\{1102,15\}\}$

Children of Cousin 686:  $\{\{843,10\},\{943,11\},\{1103,15\}\}$

Children of Cousin 687:  $\{\{845,10\},\{1101,14\},\{1104,11\},\{1104,15\}\}$

Children of Cousin 688:  $\{\{946,11\},\{1103,14\},\{1104,13\},\{1104,14\}\}$

Children of Cousin 689:  $\{\{945,11\},\{1102,14\}\}$

Children of Cousin 690:  $\{\{948,11\},\{1105,15\},\{1106,15\}\}$

Children of Cousin 691:  $\{\{949,11\},\{1105,14\},\{1107,15\}\}$

Children of Cousin 692:  $\{\{1107,14\},\{1108,11\},\{1108,15\}\}$

Children of Cousin 693:  $\{\{950,11\},\{1106,14\},\{1108,13\},\{1108,14\}\}$

Children of Cousin 694:  $\{\{851,10\},\{952,11\},\{1060,11\},\{1105,13\},\{1109,15\},\{1110,15\}\}$

Children of Cousin 695:  $\{\{856,10\},\{856,11\},\{1053,11\},\{1103,11\},\{1109,14\}\}$

Children of Cousin 696:  $\{\{954,11\},\{956,11\},\{1103,13\},\{1106,13\}\}$

Children of Cousin 697:  $\{\{953,11\},\{1110,14\}\}$

Children of Cousin 698:  $\{\{858,10\},\{858,11\},\{1057,11\},\{1107,13\},\{1112,15\}\}$

Children of Cousin 699:  $\{\{851,11\},\{1052,11\},\{1101,13\},\{1109,13\}\}$

Children of Cousin 700:  $\{\{958,11\},\{1102,13\},\{1110,13\},\{1112,14\}\}$

Children of Cousin 701:  $\{\{860,10\},\{860,11\},\{1056,11\},\{1106,11\}\}$

Children of Cousin 702:  $\{\{1112,13\}\}$

Children of Cousin 703:  $\{\{1112,11\}\}$

Children of Cousin 704:  $\{\}$

Children of Cousin 705:  $\{\{852,10\},\{1058,11\},\{1110,11\}\}$

Children of Cousin 706:  $\{\{855,10\},\{855,11\},\{1054,11\},\{1102,11\}\}$

Children of Cousin 707:  $\{\}$

Children of Cousin 708:  $\{\{852,11\},\{1051,11\}\}$

Children of Cousin 709:  $\{\{992,11\}\}$

Children of Cousin 710:  $\{\}$

Children of Cousin 711:  $\{\{993,11\}\}$

Children of Cousin 712:  $\{\{838,10\},\{1090,11\},\{1101,12\}\}$

Children of Cousin 713:  $\{\{896,10\},\{998,11\},\{1018,11\},\{1102,12\}\}$

Children of Cousin 714:  $\{\{841,10\},\{995,11\},\{1082,11\}\}$

Children of Cousin 715:  $\{\{901,10\},\{996,11\},\{1103,12\}\}$

Children of Cousin 716:  $\{\{1000,11\}\}$

Children of Cousin 717:  $\{\{1104,12\}\}$

Children of Cousin 718:  $\{\{907,10\},\{1083,11\}\}$

Children of Cousin 719:  $\{\{898,10\},\{1011,11\},\{1112,12\}\}$

Children of Cousin 720: {{1093,11}}

Children of Cousin 721: {}

Children of Cousin 722: {{911,10},{1004,11},{1096,11},{1105,12}}

Children of Cousin 723: {{909,10},{1005,11},{1084,11}}

Children of Cousin 724: {{902,10},{1006,11},{1106,12}}

Children of Cousin 725: {{1094,11},{1107,12}}

Children of Cousin 726: {{1078,11}}

Children of Cousin 727: {{1108,12}}

Children of Cousin 728: {{849,10},{906,10},{1080,11},{1088,11},{1109,12}}

Children of Cousin 729: {{897,10},{1015,11},{1110,12}}

Children of Cousin 730: {{292,3},{853,10},{913,10},{1017,11},{1039,10},{1098,11},{1100,11},{1111,12},{1113,12},{1114,12},{1115,3},{1116,3},{1116,11}}

Children of Cousin 731: {{859,10},{1076,11},{1087,11}}

Children of Cousin 732: {{849,11},{863,11},{1050,11},{1109,11}}

Children of Cousin 733: {{850,11},{854,11},{1101,11}}

Children of Cousin 734: {{1107,11}}

Children of Cousin 735: {{859,11},{1055,11},{1105,11}}

Children of Cousin 736: {{311,3},{861,11},{864,11},{1059,11},{1061,11},{1111,11},{1113,11},{1117,12},{1118,12}}

Children of Cousin 737: {{878,10},{878,11},{1075,11},{1085,11}}

Children of Cousin 738: {{874,10},{1086,11}}

Children of Cousin 739: {{1077,11}}

Children of Cousin 740: {}

Children of Cousin 741: {{867,10},{1079,11}}

Children of Cousin 742: {{316,3},{870,10},{880,11},{1045,10},{1081,11},{1089,11},{1099,11},{1115,11},{1117,11},{1119,12},{1120,3},{1120,11}}

Children of Cousin 743: {{1091,11}}

Children of Cousin 744: {{321,3},{879,10},{1046,10},{1092,11},{1095,11},{1097,11},{1114,11},{1118,11},{1119,11},{1121,3},{1121,11}}

Children of Cousin 745: {{992,10},{1122,15}}

Children of Cousin 746: {{1123,15}}

Children of Cousin 747: {{1122,14},{1123,13},{1123,14}}

Children of Cousin 748: {{993,10},{1124,15}}

Children of Cousin 749: {{1122,13},{1124,14}}

Children of Cousin 750: {}

Children of Cousin 751: {{1125,15}}

Children of Cousin 752: {{1124,13},{1125,13},{1125,14}}

Children of Cousin 753: {{1055,10},{1126,15},{1127,13},{1127,15}}

Children of Cousin 754: {{1049,10},{1128,15},{1129,15}}

Children of Cousin 755: {{952,10},{1101,10},{1126,14},{1128,14},{1130,15}}

Children of Cousin 756: {{1090,10},{1127,10},{1127,14},{1129,14},{1131,15}}

Children of Cousin 757: {{1058,10},{1130,14},{1131,14}}

Children of Cousin 758: {{949,10},{1126,13},{1132,13},{1132,15}}

Children of Cousin 759: {{980,10},{998,10},{1133,15},{1134,15}}

Children of Cousin 760: {{1102,10},{1132,10},{1132,14},{1133,14}}

Children of Cousin 761: {{1004,10},{1018,10},{1126,10},{1134,14}}

Children of Cousin 762: {{944,10},{1133,13}}

Children of Cousin 763: {{975,10},{1071,10},{1134,13},{1135,10},{1135,15}}

Children of Cousin 764: {{1054,10},{1072,10},{1133,10},{1135,11},{1135,14}}

Children of Cousin 765: {{940,10},{1128,13}}

Children of Cousin 766: {{1085,10},{1129,13}}

Children of Cousin 767: {{958,10},{1130,13},{1133,11}}

Children of Cousin 768: {{1091,10},{1131,13},{1135,12},{1135,13}}

Children of Cousin 769: {{995,10},{1050,10},{1136,15},{1137,15}}

Children of Cousin 770: {{1082,10},{1129,11},{1136,14}}

Children of Cousin 771: {{1060,10},{1128,11},{1137,14}}

Children of Cousin 772: {{963,10},{996,10},{1138,15}}

Children of Cousin 773: {{1103,10},{1122,11},{1138,14}}

Children of Cousin 774: {{943,10},{1138,13}}

Children of Cousin 775: {{974,10},{1065,10},{1136,13}}

Children of Cousin 776: {{1053,10},{1064,10},{1122,12},{1137,13},{1138,10}}

Children of Cousin 777: {{939,10},{1122,10},{1139,15}}

Children of Cousin 778: {{1075,10},{1129,12}}

Children of Cousin 779: {{938,10},{1077,10},{1123,10},{1123,12},{1128,12},{1139,14}}

Children of Cousin 780: {{956,10},{1138,11},{1139,13}}

Children of Cousin 781: {{1140,15},{1141,14},{1141,15}}

Children of Cousin 782: {{1000,10},{1140,14},{1142,14},{1142,15}}

Children of Cousin 783: {{1087,10},{1140,13}}

Children of Cousin 784: {{1057,10},{1141,10},{1141,13}}

Children of Cousin 785: {{976,10},{1086,10},{1131,10},{1136,12},{1142,10},{1142,13}}

Children of Cousin 786: {{1052,10},{1137,12},{1140,10}}

Children of Cousin 787: {{1051,10},{1131,11}}

Children of Cousin 788: {{1131,12}}

Children of Cousin 789: {{1143,15}}

Children of Cousin 790: {{1104,10},{1123,11},{1143,14}}

Children of Cousin 791: {{948,10},{1078,10},{1126,12},{1143,13},{1144,15}}

Children of Cousin 792: {{1076,10},{1127,11},{1127,12}}

Children of Cousin 793: {{1056,10},{1124,12},{1144,14}}

Children of Cousin 794: {{954,10},{1139,11},{1144,13}}

Children of Cousin 795: {{953,10},{1130,12},{1143,10}}

Children of Cousin 796: {{1143,12}}

Children of Cousin 797: {{946,10},{1138,12},{1145,15}}

Children of Cousin 798: {{1093,10},{1145,14}}

Children of Cousin 799: {{1143,11},{1145,13}}

Children of Cousin 800: {{1132,11},{1132,12},{1146,15}}

Children of Cousin 801: {{1105,10},{1126,11},{1140,12}}

Children of Cousin 802: {{1107,10},{1125,10},{1125,12},{1141,11},{1141,12},{1146,14}}

Children of Cousin 803: {{945,10},{1133,12},{1145,12}}

Children of Cousin 804: {{977,10},{1096,10},{1134,12},{1142,11},{1142,12}}

Children of Cousin 805: {{1094,10},{1124,10},{1140,11},{1145,10}}

Children of Cousin 806: {{1145,11},{1146,13}}

Children of Cousin 807: {{950,10},{1144,12},{1146,12}}

Children of Cousin 808: {{941,10},{1139,12}}

Children of Cousin 809: {{962,10},{967,10},{1083,10},{1139,10}}

Children of Cousin 810: {{1006,10},{1011,10},{1144,10}}

Children of Cousin 811: {{1112,10},{1146,10}}

Children of Cousin 812: {{981,10},{1005,10},{1015,10},{1130,10},{1147,11},{1147,15}}

Children of Cousin 813: {{979,10},{985,10},{1084,10},{1134,11},{1147,13},{1147,14}}

Children of Cousin 814: {{1106,10},{1124,11},{1144,11}}

Children of Cousin 815: {{1109,10},{1137,11}}

Children of Cousin 816: {{987,10},{1088,10},{1136,11}}

Children of Cousin 817: {{969,10},{1080,10},{1137,10}}

Children of Cousin 818: {{1110,10},{1130,11}}

Children of Cousin 819: {{983,10},{984,10},{1070,10},{1134,10},{1147,10},{1147,12}}

Children of Cousin 820: {{965,10},{966,10},{1069,10},{1128,10}}

Children of Cousin 821: {{1148,14},{1148,15}}

Children of Cousin 822: {{1146,11},{1148,10},{1148,13}}

Children of Cousin 823: {{1108,10},{1125,11},{1148,11},{1148,12}}

Children of Cousin 824: {{1079,10},{1149,10},{1149,15}}

Children of Cousin 825: {{1062,10},{1067,10},{1149,11},{1149,14}}

Children of Cousin 826: {{1063,10},{1068,10},{1129,10},{1136,10},{1149,12},{1149,13}}

Children of Cousin 827: {{1150,13},{1150,16},{1151,16}}

Children of Cousin 828: {{1154,16}}

Children of Cousin 829: {{1150,14},{1150,15}}

Children of Cousin 830: {{1151,15},{1154,15}}

Children of Cousin 831: {{430,2},{1152,2},{1155,2},{1156,2},{1157,2}}

Children of Cousin 832: {{1151,14}}

Children of Cousin 833: {{1154,13}}

Children of Cousin 834: {{1154,14}}

Children of Cousin 835: {{435,5},{1158,14},{1159,14},{1160,14},{1161,14}}

Children of Cousin 836: {{1151,13}}

Children of Cousin 837: {{436,6},{1153,13},{1162,6}}

Children of Cousin 838: {{1163,16}}

Children of Cousin 839: {{1165,12},{1165,16}}

Children of Cousin 840: {{1163,15},{1165,13},{1165,15}}

Children of Cousin 841: {{1168,16}}

Children of Cousin 842: {{1168,15},{1170,12},{1170,16}}

Children of Cousin 843: {{1170,13},{1170,15}}

Children of Cousin 844: {{1168,14}}

Children of Cousin 845: {{1163,14}}

Children of Cousin 846: {{1165,14},{1170,14}}

Children of Cousin 847: {{443,4},{1166,14},{1171,14},{1173,14},{1175,4}}

Children of Cousin 848: {{444,5},{1167,14},{1172,14},{1174,14},{1175,13}}

Children of Cousin 849: {{1151,10},{1176,12},{1176,16}}

Children of Cousin 850: {{1154,10},{1163,12}}

Children of Cousin 851: {{1163,13},{1176,13},{1176,15}}

Children of Cousin 852: {}

Children of Cousin 853: {{445,6},{1157,10},{1178,6},{1180,6},{1181,6},{1182,6}}

Children of Cousin 854: {{1154,12}}

Children of Cousin 855: {}

Children of Cousin 856: {{1176,14}}

Children of Cousin 857: {{448,4},{1161,12},{1174,12},{1179,14},{1183,14}}

Children of Cousin 858: {}

Children of Cousin 859: {}

Children of Cousin 860: {}

Children of Cousin 861: {{455,3},{1162,10},{1164,13},{1177,13},{1181,12}}

Children of Cousin 862: {{456,4},{1160,12},{1166,13},{1167,12},{1179,13}}

Children of Cousin 863: {{1151,12},{1168,13}}

Children of Cousin 864: {{459,3},{1162,12},{1169,13},{1182,12},{1184,13},{1185,3}}

Children of Cousin 865: {{460,4},{1159,12},{1171,13},{1172,12},{1186,14}}

Children of Cousin 866: {{462,4},{1158,12},{1173,13},{1183,13},{1186,13}}

Children of Cousin 867: {{1150,10},{1150,12},{1187,12},{1187,16}}

Children of Cousin 868: {{1168,12},{1187,13},{1187,15}}

Children of Cousin 869: {}

Children of Cousin 870: {{464,6},{1153,12},{1185,12},{1189,6},{1190,6},{1191,6}}

Children of Cousin 871: {}

Children of Cousin 872: {{1187,14}}

Children of Cousin 873: {}

Children of Cousin 874: {}

Children of Cousin 875: {}

Children of Cousin 876: {{473,3},{1156,10},{1169,12},{1188,13},{1190,12}}

Children of Cousin 877: {{476,3},{1155,10},{1164,12},{1180,12},{1191,12},{1192,13}}

Children of Cousin 878: {}

Children of Cousin 879: {{478,6},{1184,12},{1192,12},{1193,12}}

Children of Cousin 880: {{480,3},{480,6},{1152,10},{1153,10},{1177,12},{1178,12},{1188,12},{1189,12},{1193,13}}

Children of Cousin 881: {{1195,16},{1196,16}}

Children of Cousin 882: {{1195,15},{1199,16}}

Children of Cousin 883: {{1196,15},{1201,16},{1202,16}}

Children of Cousin 884: {{1199,15}}

Children of Cousin 885: {{1199,11},{1201,15}}

Children of Cousin 886: {{1195,11},{1202,15}}

Children of Cousin 887: {{482,1},{1197,1},{1200,1},{1203,1},{1204,1},{1205,1},{1207,1}}

Children of Cousin 888: {{1209,16},{1210,16},{1211,16}}

Children of Cousin 889: {{1209,15},{1214,16}}

Children of Cousin 890: {{1216,16}}

Children of Cousin 891: {{1210,15},{1214,15},{1218,16}}

Children of Cousin 892: {{1211,15},{1214,11},{1216,15},{1220,16}}

Children of Cousin 893: {{1209,11},{1218,15},{1220,15}}

Children of Cousin 894: {{483,1},{1212,1},{1215,1},{1217,1},{1219,1},{1221,1},{1223,1}}

Children of Cousin 895: {{1209,14},{1225,16},{1226,16},{1227,16}}

Children of Cousin 896: {{1210,14},{1225,15}}

Children of Cousin 897: {{1211,14},{1226,15}}

Children of Cousin 898: {{1227,15}}

Children of Cousin 899: {{484,1},{1212,14},{1228,1},{1230,1},{1231,1},{1233,1}}

Children of Cousin 900: {{1195,14},{1227,14}}

Children of Cousin 901: {{1196,14}}

Children of Cousin 902: {{1227,11}}

Children of Cousin 903: {{485,1},{1197,14},{1234,1},{1236,1},{1237,1}}

Children of Cousin 904: {{1154,11},{1199,14},{1214,14},{1225,14},{1226,14}}

Children of Cousin 905: {{486,1},{486,6},{1161,11},{1200,14},{1215,14},{1228,14},{1229,14},{1234,14},{1235,14},{1238,1},{1240,6}}

Children of Cousin 906: {{1151,11},{1201,14},{1216,14}}

Children of Cousin 907: {{1202,14}}

Children of Cousin 908: {{487,1},{1159,11},{1203,14},{1217,14},{1236,14},{1242,1},{1244,1}}

Children of Cousin 909: {{1218,14},{1226,11}}

Children of Cousin 910: {{488,1},{1160,11},{1204,14},{1219,14},{1230,14},{1238,14},{1245,1}}

Children of Cousin 911: {{1220,14},{1225,11}}

Children of Cousin 912: {{489,1},{1158,11},{1205,14},{1221,14},{1231,14},{1240,11},{1242,14},{1246,1}}

Children of Cousin 913: {{489,4},{1157,11},{1206,14},{1222,14},{1232,14},{1239,11},{1243,14},{1247,4}}

Children of Cousin 914: {{490,1},{1223,14},{1229,11},{1237,14},{1245,14},{1246,14}}

Children of Cousin 915: {{491,1},{1207,14},{1233,14},{1235,11},{1244,14}}

Children of Cousin 916: {{1202,12},{1249,16}}

Children of Cousin 917: {{1195,12}}

Children of Cousin 918: {{1249,15}}

Children of Cousin 919: {{493,1},{1208,12},{1250,1},{1251,1},{1252,1}}

Children of Cousin 920: {{1220,12},{1253,16},{1254,16}}

Children of Cousin 921: {{1218,12},{1257,16}}

Children of Cousin 922: {{1253,15}}

Children of Cousin 923: {{1209,12},{1254,15},{1257,15}}

Children of Cousin 924: {{494,1},{1224,12},{1255,1},{1258,1},{1259,1},{1260,1}}

Children of Cousin 925: {{1196,12},{1253,14}}

Children of Cousin 926: {{1210,12},{1254,14}}

Children of Cousin 927: {{1210,11},{1220,11}}

Children of Cousin 928: {{1196,11}}

Children of Cousin 929: {{495,1},{1255,14},{1261,1},{1262,1},{1263,1},{1264,1}}

Children of Cousin 930: {{1211,12},{1249,14},{1257,14}}

Children of Cousin 931: {{1211,11},{1218,11}}

Children of Cousin 932: {{1202,11}}

Children of Cousin 933: {{496,1},{1250,14},{1258,14},{1265,1},{1267,1},{1268,1}}

Children of Cousin 934: {{497,1},{1198,12},{1251,14},{1259,14},{1261,14}}

Children of Cousin 935: {{498,1},{1213,12},{1252,14},{1260,14},{1262,14},{1265,14}}

Children of Cousin 936: {{499,1},{1213,11},{1224,11},{1263,14},{1267,14}}

Children of Cousin 937: {{500,1},{1198,11},{1208,11},{1264,14},{1268,14}}

Children of Cousin 938: {{1269,16},{1270,16}}

Children of Cousin 939: {{1270,12}}

Children of Cousin 940: {{1269,15}}

Children of Cousin 941: {{1270,15}}

Children of Cousin 942: {{502,1},{1271,1},{1272,1},{1273,1},{1274,1}}

Children of Cousin 943: {{1170,10},{1170,11},{1275,16}}

Children of Cousin 944: {{1165,10},{1165,11},{1277,16}}

Children of Cousin 945: {{1277,15}}

Children of Cousin 946: {{1275,15}}

Children of Cousin 947: {{503,1},{1175,10},{1276,1},{1278,1},{1279,1},{1280,1}}

Children of Cousin 948:  $\{\{1281,16\},\{1282,16\}\}$

Children of Cousin 949:  $\{\{1281,15\}\}$

Children of Cousin 950:  $\{\{1282,15\}\}$

Children of Cousin 951:  $\{\{504,1\},\{1283,1\},\{1284,1\},\{1285,1\}\}$

Children of Cousin 952:  $\{\{1163,11\},\{1269,14\},\{1281,14\},\{1286,16\}\}$

Children of Cousin 953:  $\{\{1286,15\}\}$

Children of Cousin 954:  $\{\{1270,14\},\{1282,14\}\}$

Children of Cousin 955:  $\{\{505,1\},\{1174,11\},\{1271,14\},\{1283,14\},\{1287,1\},\{1289,1\},\{1290,1\}\}$

Children of Cousin 956:  $\{\{1270,11\},\{1275,14\}\}$

Children of Cousin 957:  $\{\{506,1\},\{1172,11\},\{1272,14\},\{1276,14\},\{1291,1\}\}$

Children of Cousin 958:  $\{\{1277,14\},\{1286,14\}\}$

Children of Cousin 959:  $\{\{507,1\},\{1167,11\},\{1273,14\},\{1278,14\},\{1284,14\},\{1287,14\},\{1292,1\}\}$

Children of Cousin 960:  $\{\{508,1\},\{1279,14\},\{1289,14\},\{1292,14\}\}$

Children of Cousin 961:  $\{\{509,1\},\{1274,14\},\{1280,14\},\{1285,14\},\{1290,14\},\{1291,14\}\}$

Children of Cousin 962:  $\{\{1195,13\}\}$

Children of Cousin 963:  $\{\{1196,13\}\}$

Children of Cousin 964:  $\{\{511,1\},\{1197,13\},\{1293,1\},\{1294,1\}\}$

Children of Cousin 965:  $\{\{1199,13\},\{1249,13\},\{1269,13\}\}$

Children of Cousin 966:  $\{\{1199,10\}\}$

Children of Cousin 967:  $\{\{1195,10\},\{1202,13\},\{1270,13\}\}$

Children of Cousin 968:  $\{\{512,1\},\{1200,13\},\{1250,13\},\{1271,13\},\{1293,14\},\{1295,1\},\{1297,1\},\{1298,1\}\}$

Children of Cousin 969:  $\{\{1201,13\}\}$

Children of Cousin 970:  $\{\{513,1\},\{1203,13\},\{1251,13\},\{1272,13\},\{1294,14\},\{1299,12\},\{1300,1\}\}$

Children of Cousin 971:  $\{\{514,1\},\{1204,13\},\{1252,13\},\{1273,13\},\{1295,14\}\}$

Children of Cousin 972:  $\{\{515,1\},\{1205,13\},\{1297,14\},\{1300,14\}\}$

Children of Cousin 973:  $\{\{516,1\},\{516,5\},\{1207,13\},\{1208,13\},\{1274,13\},\{1298,14\},\{1299,14\}\}$

Children of Cousin 974:  $\{\{1253,13\},\{1302,16\}\}$

Children of Cousin 975:  $\{\{1254,13\},\{1304,16\}\}$

Children of Cousin 976:  $\{\{1302,15\},\{1306,12\},\{1306,16\}\}$

Children of Cousin 977:  $\{\{1220,13\},\{1304,15\},\{1306,14\},\{1306,15\}\}$

Children of Cousin 978:  $\{\{518,1\},\{1255,13\},\{1303,1\},\{1305,1\},\{1307,1\},\{1308,1\}\}$

Children of Cousin 979:  $\{\{1209,13\},\{1310,16\},\{1311,16\}\}$

Children of Cousin 980:  $\{\{1210,13\},\{1310,15\}\}$

Children of Cousin 981:  $\{\{1211,13\},\{1311,15\}\}$

Children of Cousin 982:  $\{\{519,1\},\{1212,13\},\{1312,1\},\{1313,1\},\{1314,1\}\}$

Children of Cousin 983:  $\{\{1214,13\},\{1257,13\},\{1310,14\},\{1315,12\},\{1315,16\}\}$

Children of Cousin 984:  $\{\{1214,10\},\{1304,12\},\{1311,14\}\}$

Children of Cousin 985:  $\{\{1209,10\},\{1218,13\},\{1304,14\},\{1315,14\},\{1315,15\}\}$



Children of Cousin 986: {{520,1},{1215,13},{1258,13},{1312,14},{1316,1},{1318,1},{1319,1}}

Children of Cousin 987: {{1216,13},{1302,14}}

Children of Cousin 988: {{521,1},{1217,13},{1259,13},{1303,14},{1321,1}}

Children of Cousin 989: {{522,1},{1219,13},{1260,13},{1305,14},{1313,14},{1316,14},{1320,12}}

Children of Cousin 990: {{523,1},{1221,13},{1307,14},{1309,12},{1314,14},{1318,14},{1321,14}}

Children of Cousin 991: {{524,1},{524,5},{1223,13},{1224,13},{1308,14},{1309,14},{1319,14},{1320,14}}

Children of Cousin 992: {}

Children of Cousin 993: {}

Children of Cousin 994: {{526,1},{1323,1},{1324,1}}

Children of Cousin 995: {{1168,10},{1302,13}}

Children of Cousin 996: {{1196,10},{1275,13}}

Children of Cousin 997: {{527,1},{1171,10},{1261,13},{1276,13},{1303,13},{1323,14},{1325,1},{1326,1}}

Children of Cousin 998: {{1210,10},{1277,13},{1304,13}}

Children of Cousin 999: {{528,1},{1166,10},{1262,13},{1278,13},{1305,13},{1327,1}}

Children of Cousin 1000: {{1306,11},{1306,13}}

Children of Cousin 1001: {{529,1},{1173,10},{1307,13},{1325,14},{1328,1}}

Children of Cousin 1002: {{530,1},{1263,13},{1279,13},{1308,13},{1324,14},{1327,14},{1328,14}}

Children of Cousin 1003: {{531,1},{1264,13},{1280,13},{1326,14}}

Children of Cousin 1004: {{1225,13},{1281,13},{1310,13}}

Children of Cousin 1005: {{1226,13},{1311,13}}

Children of Cousin 1006: {{1227,13},{1282,13}}

Children of Cousin 1007: {{533,1},{1228,13},{1283,13},{1312,13},{1329,1},{1331,1},{1332,1}}

Children of Cousin 1008: {{534,1},{1230,13},{1284,13},{1313,13},{1329,14}}

Children of Cousin 1009: {{535,1},{1231,13},{1314,13},{1331,14}}

Children of Cousin 1010: {{536,1},{1233,13},{1285,13},{1332,14}}

Children of Cousin 1011: {{1227,10}}

Children of Cousin 1012: {{538,1},{1234,13},{1293,13},{1333,1}}

Children of Cousin 1013: {{539,1},{1236,13},{1294,13},{1323,13}}

Children of Cousin 1014: {{540,1},{1237,13},{1324,13},{1333,14}}

Children of Cousin 1015: {{1211,10},{1226,10},{1286,13},{1315,11},{1315,13}}

Children of Cousin 1016: {{542,1},{1179,10},{1238,13},{1265,13},{1287,13},{1295,13},{1316,13},{1329,13},{1334,1}}

Children of Cousin 1017: {{542,3},{1180,10},{1239,13},{1266,13},{1288,13},{1296,13},{1317,13},{1330,13},{1335,3}}

Children of Cousin 1018: {{1225,10},{1304,11}}

Children of Cousin 1019: {{543,1},{1183,10},{1240,10},{1297,13},{1318,13},{1331,13},{1337,1}}

Children of Cousin 1020: {{544,1},{1229,10},{1267,13},{1289,13},{1319,13},{1333,13},{1334,14},{1337,14}}

Children of Cousin 1021: {{545,1},{1235,10},{1268,13},{1290,13},{1298,13},{1332,13}}

Children of Cousin 1022: {{547,1},{1186,10},{1242,13},{1300,13},{1321,13},{1325,13}}

Children of Cousin 1023: {{548,1},{1198,10},{1244,13},{1291,13},{1299,11},{1326,13}}

Children of Cousin 1024:  $\{\{550,1\},\{1213,10\},\{1245,13\},\{1292,13\},\{1320,11\},\{1327,13\},\{1334,13\}\}$

Children of Cousin 1025:  $\{\{552,1\},\{1246,13\},\{1309,11\},\{1328,13\},\{1337,13\}\}$

Children of Cousin 1026:  $\{\{1199,12\}\}$

Children of Cousin 1027:  $\{\{1249,12\},\{1253,12\},\{1339,16\}\}$

Children of Cousin 1028:  $\{\{1339,15\}\}$

Children of Cousin 1029:  $\{\{1201,12\},\{1339,14\}\}$

Children of Cousin 1030:  $\{\{560,4\},\{1206,12\},\{1338,11\},\{1341,14\},\{1342,14\}\}$

Children of Cousin 1031:  $\{\{1214,12\},\{1254,12\},\{1257,12\}\}$

Children of Cousin 1032:  $\{\{1216,12\},\{1339,11\}\}$

Children of Cousin 1033:  $\{\{564,4\},\{1222,12\},\{1256,12\},\{1266,12\},\{1340,11\},\{1343,11\},\{1344,14\}\}$

Children of Cousin 1034:  $\{\{1225,12\},\{1254,11\}\}$

Children of Cousin 1035:  $\{\{1226,12\},\{1257,11\}\}$

Children of Cousin 1036:  $\{\{1227,12\}\}$

Children of Cousin 1037:  $\{\{1249,11\}\}$

Children of Cousin 1038:  $\{\}$

Children of Cousin 1039:  $\{\{568,4\},\{1232,12\},\{1266,11\},\{1346,14\},\{1347,14\}\}$

Children of Cousin 1040:  $\{\{1253,11\}\}$

Children of Cousin 1041:  $\{\}$

Children of Cousin 1042:  $\{\{574,3\},\{1155,11\},\{1239,12\},\{1338,13\},\{1343,13\},\{1345,13\},\{1346,13\}\}$

Children of Cousin 1043:  $\{\{1150,11\},\{1339,13\}\}$

Children of Cousin 1044:  $\{\{575,3\},\{1156,11\},\{1340,13\},\{1341,13\},\{1347,13\},\{1348,13\},\{1349,3\}\}$

Children of Cousin 1045:  $\{\{576,4\},\{1152,11\},\{1243,12\},\{1342,13\},\{1344,13\},\{1349,11\}\}$

Children of Cousin 1046:  $\{\{579,4\},\{1247,12\},\{1256,11\},\{1345,11\},\{1348,11\}\}$

Children of Cousin 1047:  $\{\{1216,11\}\}$

Children of Cousin 1048:  $\{\{1201,11\}\}$

Children of Cousin 1049:  $\{\{1269,12\}\}$

Children of Cousin 1050:  $\{\{1168,11\},\{1351,16\}\}$

Children of Cousin 1051:  $\{\}$

Children of Cousin 1052:  $\{\{1351,15\}\}$

Children of Cousin 1053:  $\{\{1275,12\},\{1351,14\}\}$

Children of Cousin 1054:  $\{\{1277,12\}\}$

Children of Cousin 1055:  $\{\{1281,12\}\}$

Children of Cousin 1056:  $\{\{1282,12\}\}$

Children of Cousin 1057:  $\{\}$

Children of Cousin 1058:  $\{\{1286,12\}\}$

Children of Cousin 1059:  $\{\{597,3\},\{1164,11\},\{1288,12\},\{1350,13\},\{1353,13\},\{1354,3\}\}$

Children of Cousin 1060:  $\{\{1269,11\},\{1351,13\}\}$

Children of Cousin 1061:  $\{\{600,3\},\{1169,11\},\{1350,11\},\{1352,13\},\{1355,3\}\}$

Children of Cousin 1062:  $\{\{1339,12\}\}$

Children of Cousin 1063:  $\{\}$

Children of Cousin 1064:  $\{\}$

Children of Cousin 1065:  $\{\{1253,10\}\}$

Children of Cousin 1066:  $\{\{613,3\},\{1296,12\},\{1338,12\},\{1340,12\},\{1350,12\},\{1356,13\},\{1357,13\}\}$

Children of Cousin 1067:  $\{\{1339,10\},\{1358,13\},\{1358,16\}\}$

Children of Cousin 1068:  $\{\{1302,12\},\{1358,14\},\{1358,15\}\}$

Children of Cousin 1069:  $\{\{1249,10\}\}$

Children of Cousin 1070:  $\{\{1257,10\},\{1311,12\}\}$

Children of Cousin 1071:  $\{\{1254,10\},\{1310,12\},\{1360,13\},\{1360,16\}\}$

Children of Cousin 1072:  $\{\{1360,14\},\{1360,15\}\}$

Children of Cousin 1073:  $\{\{623,3\},\{1317,12\},\{1343,12\},\{1361,13\}\}$

Children of Cousin 1074:  $\{\{624,3\},\{1341,10\},\{1359,13\}\}$

Children of Cousin 1075:  $\{\}$

Children of Cousin 1076:  $\{\}$

Children of Cousin 1077:  $\{\}$

Children of Cousin 1078:  $\{\}$

Children of Cousin 1079:  $\{\{1187,10\},\{1187,11\},\{1358,11\},\{1358,12\}\}$

Children of Cousin 1080:  $\{\{1201,10\},\{1351,12\}\}$

Children of Cousin 1081:  $\{\{629,3\},\{1190,10\},\{1342,10\},\{1352,12\},\{1359,12\},\{1362,13\},\{1363,3\},\{1364,3\}\}$

Children of Cousin 1082:  $\{\{1302,11\}\}$

Children of Cousin 1083:  $\{\{1202,10\}\}$

Children of Cousin 1084:  $\{\{1218,10\},\{1311,11\}\}$

Children of Cousin 1085:  $\{\}$

Children of Cousin 1086:  $\{\}$

Children of Cousin 1087:  $\{\}$

Children of Cousin 1088:  $\{\{1216,10\}\}$

Children of Cousin 1089:  $\{\{645,3\},\{1191,10\},\{1344,10\},\{1356,12\},\{1365,13\},\{1366,3\}\}$

Children of Cousin 1090:  $\{\}$

Children of Cousin 1091:  $\{\{1360,11\},\{1360,12\}\}$

Children of Cousin 1092:  $\{\{653,3\},\{1330,12\},\{1345,12\},\{1353,12\},\{1361,12\},\{1365,12\},\{1367,3\}\}$

Children of Cousin 1093:  $\{\}$

Children of Cousin 1094:  $\{\}$

Children of Cousin 1095:  $\{\{663,3\},\{1348,12\},\{1357,12\},\{1362,12\}\}$

Children of Cousin 1096:  $\{\{1220,10\},\{1310,11\}\}$

Children of Cousin 1097:  $\{\{667,3\},\{1192,11\},\{1256,10\},\{1357,11\},\{1361,11\},\{1367,12\},\{1368,3\}\}$

Children of Cousin 1098:  $\{\{668,3\},\{1222,10\},\{1317,11\},\{1335,12\},\{1346,10\},\{1354,12\},\{1366,12\},\{1368,14\}\}$

Children of Cousin 1099:  $\{\{673,3\},\{1188,11\},\{1349,12\},\{1356,11\},\{1359,11\},\{1363,12\}\}$

Children of Cousin 1100:  $\{\{674,3\},\{1206,10\},\{1296,11\},\{1347,10\},\{1355,12\},\{1364,12\}\}$

Children of Cousin 1101:  $\{\{1163,10\}\}$

Children of Cousin 1102:  $\{\{1277,11\}\}$

Children of Cousin 1103:  $\{\{1275,11\}\}$

Children of Cousin 1104:  $\{\}$

Children of Cousin 1105:  $\{\{1281,11\}\}$

Children of Cousin 1106:  $\{\{1282,11\}\}$

Children of Cousin 1107:  $\{\}$

Children of Cousin 1108:  $\{\}$

Children of Cousin 1109:  $\{\{1176,10\},\{1176,11\},\{1351,11\}\}$

Children of Cousin 1110:  $\{\{1286,11\}\}$

Children of Cousin 1111:  $\{\{694,3\},\{1181,10\},\{1288,11\},\{1355,11\},\{1369,13\},\{1370,3\},\{1371,3\}\}$

Children of Cousin 1112:  $\{\}$

Children of Cousin 1113:  $\{\{705,3\},\{1182,10\},\{1354,11\},\{1371,11\}\}$

Children of Cousin 1114:  $\{\{722,3\},\{1247,10\},\{1330,11\},\{1368,11\},\{1369,12\}\}$

Children of Cousin 1115:  $\{\{728,3\},\{1178,10\},\{1243,10\},\{1364,11\},\{1366,11\},\{1370,12\}\}$

Children of Cousin 1116:  $\{\{729,3\},\{1232,10\},\{1335,11\},\{1371,12\}\}$

Children of Cousin 1117:  $\{\{732,3\},\{1177,11\},\{1185,11\},\{1352,11\},\{1370,11\}\}$

Children of Cousin 1118:  $\{\{735,3\},\{1184,11\},\{1353,11\},\{1369,11\}\}$

Children of Cousin 1119:  $\{\{737,3\},\{1193,11\},\{1362,11\},\{1365,11\}\}$

Children of Cousin 1120:  $\{\{741,3\},\{1189,10\},\{1363,11\}\}$

Children of Cousin 1121:  $\{\{743,3\},\{1367,11\}\}$

Children of Cousin 1122:  $\{\}$

Children of Cousin 1123:  $\{\}$

Children of Cousin 1124:  $\{\}$

Children of Cousin 1125:  $\{\}$

Children of Cousin 1126:  $\{\{1281,10\}\}$

Children of Cousin 1127:  $\{\}$

Children of Cousin 1128:  $\{\{1269,10\}\}$

Children of Cousin 1129:  $\{\}$

Children of Cousin 1130:  $\{\{1286,10\}\}$

Children of Cousin 1131:  $\{\}$

Children of Cousin 1132:  $\{\}$

Children of Cousin 1133:  $\{\{1277,10\}\}$

Children of Cousin 1134:  $\{\{1304,10\},\{1310,10\}\}$

Children of Cousin 1135:  $\{\{1360,10\}\}$

Children of Cousin 1136:  $\{\{1302,10\}\}$

Children of Cousin 1137:  $\{\{1351,10\}\}$

Children of Cousin 1138:  $\{\{1275,10\}\}$

Children of Cousin 1139:  $\{\{1270,10\}\}$

Children of Cousin 1140:  $\{\}$

Children of Cousin 1141:  $\{\}$

Children of Cousin 1142:  $\{\{1306,10\}\}$

Children of Cousin 1143:  $\{\}$

Children of Cousin 1144:  $\{\{1282,10\}\}$

Children of Cousin 1145:  $\{\}$

Children of Cousin 1146:  $\{\}$

Children of Cousin 1147:  $\{\{1311,10\},\{1315,10\}\}$

Children of Cousin 1148:  $\{\}$

Children of Cousin 1149:  $\{\{1358,10\}\}$

Children of Cousin 1150:  $\{\}$

Children of Cousin 1151:  $\{\}$

Children of Cousin 1152:  $\{\{827,2\},\{1372,2\},\{1374,2\}\}$

Children of Cousin 1153:  $\{\{827,6\},\{1373,6\},\{1373,13\},\{1376,6\}\}$

Children of Cousin 1154:  $\{\}$

Children of Cousin 1155:  $\{\{828,2\},\{1378,2\}\}$

Children of Cousin 1156:  $\{\{829,2\},\{1372,15\}\}$

Children of Cousin 1157:  $\{\{830,2\},\{1374,15\},\{1378,15\}\}$

Children of Cousin 1158:  $\{\{830,5\},\{1375,15\},\{1379,15\}\}$

Children of Cousin 1159:  $\{\{832,5\},\{1375,14\}\}$

Children of Cousin 1160:  $\{\{833,5\},\{1380,13\}\}$

Children of Cousin 1161:  $\{\{834,5\},\{834,7\},\{1379,14\},\{1380,14\}\}$

Children of Cousin 1162:  $\{\{836,6\},\{1376,13\}\}$

Children of Cousin 1163:  $\{\}$

Children of Cousin 1164:  $\{\{838,3\},\{1383,3\}\}$

Children of Cousin 1165:  $\{\}$

Children of Cousin 1166:  $\{\{839,4\},\{1385,4\}\}$

Children of Cousin 1167:  $\{\{840,5\},\{1384,15\},\{1385,13\}\}$

Children of Cousin 1168:  $\{\}$

Children of Cousin 1169:  $\{\{841,3\},\{1386,3\}\}$

Children of Cousin 1170:  $\{\}$

Children of Cousin 1171:  $\{\{842,4\},\{1387,15\},\{1388,4\}\}$

Children of Cousin 1172:  $\{\{843,5\},\{1388,13\}\}$

Children of Cousin 1173:  $\{\{844,4\},\{1387,14\}\}$

Children of Cousin 1174:  $\{\{845,5\},\{1384,14\}\}$

Children of Cousin 1175:  $\{\{846,4\},\{846,5\},\{1385,14\},\{1388,14\}\}$

Children of Cousin 1176: {}

Children of Cousin 1177: {{849,3},{1376,10},{1390,3}}

Children of Cousin 1178: {{849,6},{1374,10},{1390,12}}

Children of Cousin 1179: {{850,4},{1380,10},{1384,12}}

Children of Cousin 1180: {{850,6},{1378,10},{1383,12}}

Children of Cousin 1181: {{851,6},{1383,13},{1390,13}}

Children of Cousin 1182: {{852,6}}

Children of Cousin 1183: {{854,4},{1379,12}}

Children of Cousin 1184: {{859,3}}

Children of Cousin 1185: {{863,3},{1376,12},{1386,13}}

Children of Cousin 1186: {{863,4},{1375,12},{1387,13}}

Children of Cousin 1187: {}

Children of Cousin 1188: {{867,3},{1372,10},{1394,3}}

Children of Cousin 1189: {{867,6},{1373,10},{1373,12},{1394,12}}

Children of Cousin 1190: {{868,6},{1386,12},{1394,13}}

Children of Cousin 1191: {{869,6}}

Children of Cousin 1192: {{874,3}}

Children of Cousin 1193: {{878,3},{878,6}}

Children of Cousin 1194: {{880,6},{1377,10},{1391,12},{1395,12},{1396,13}}

Children of Cousin 1195: {}

Children of Cousin 1196: {}

Children of Cousin 1197: {{881,1},{1397,1},{1400,1}}

Children of Cousin 1198: {{881,2},{1398,2},{1401,2}}

Children of Cousin 1199: {}

Children of Cousin 1200: {{882,1},{882,6},{1397,15},{1399,15},{1403,1},{1405,6}}

Children of Cousin 1201: {}

Children of Cousin 1202: {}

Children of Cousin 1203: {{883,1},{1400,15},{1407,1},{1409,1}}

Children of Cousin 1204: {{884,1},{1403,15}}

Children of Cousin 1205: {{885,1},{1405,11},{1407,15}}

Children of Cousin 1206: {{885,4},{1404,11},{1408,15}}

Children of Cousin 1207: {{886,1},{1399,11},{1409,15}}

Children of Cousin 1208: {{886,5},{1398,11},{1410,15}}

Children of Cousin 1209: {{1413,17},{1414,17}}

Children of Cousin 1210: {{1413,16}}

Children of Cousin 1211: {{1414,16}}

Children of Cousin 1212: {{888,1},{1415,1},{1418,1},{1420,1}}

Children of Cousin 1213: {{888,2},{1416,2},{1419,2},{1421,2}}

Children of Cousin 1214:  $\{\{1413,15\},\{1414,15\}\}$

Children of Cousin 1215:  $\{\{889,1\},\{889,6\},\{1415,15\},\{1417,15\},\{1424,1\},\{1426,6\}\}$

Children of Cousin 1216:  $\{\}$

Children of Cousin 1217:  $\{\{890,1\},\{1428,1\}\}$

Children of Cousin 1218:  $\{\{1414,11\}\}$

Children of Cousin 1219:  $\{\{891,1\},\{1418,15\},\{1424,15\},\{1430,1\}\}$

Children of Cousin 1220:  $\{\{1413,11\}\}$

Children of Cousin 1221:  $\{\{892,1\},\{1420,15\},\{1426,11\},\{1428,15\},\{1432,1\}\}$

Children of Cousin 1222:  $\{\{892,4\},\{1422,15\},\{1425,11\},\{1429,15\},\{1433,4\}\}$

Children of Cousin 1223:  $\{\{893,1\},\{1417,11\},\{1430,15\},\{1432,15\}\}$

Children of Cousin 1224:  $\{\{893,5\},\{1416,11\},\{1431,15\},\{1434,15\}\}$

Children of Cousin 1225:  $\{\{1413,14\}\}$

Children of Cousin 1226:  $\{\{1414,14\}\}$

Children of Cousin 1227:  $\{\}$

Children of Cousin 1228:  $\{\{895,1\},\{1415,14\},\{1437,1\},\{1440,1\},\{1443,1\}\}$

Children of Cousin 1229:  $\{\{895,6\},\{1417,14\},\{1439,6\},\{1442,6\},\{1444,6\}\}$

Children of Cousin 1230:  $\{\{896,1\},\{1418,14\},\{1437,15\}\}$

Children of Cousin 1231:  $\{\{897,1\},\{1420,14\},\{1440,15\}\}$

Children of Cousin 1232:  $\{\{897,4\},\{1422,14\},\{1441,15\}\}$

Children of Cousin 1233:  $\{\{898,1\},\{1443,15\}\}$

Children of Cousin 1234:  $\{\{900,1\},\{1397,14\},\{1444,14\}\}$

Children of Cousin 1235:  $\{\{900,6\},\{1399,14\},\{1443,14\}\}$

Children of Cousin 1236:  $\{\{901,1\},\{1400,14\}\}$

Children of Cousin 1237:  $\{\{902,1\},\{1444,11\}\}$

Children of Cousin 1238:  $\{\{904,1\},\{1380,11\},\{1403,14\},\{1424,14\},\{1437,14\},\{1442,14\}\}$

Children of Cousin 1239:  $\{\{904,3\},\{1378,11\},\{1404,14\},\{1425,14\},\{1438,14\},\{1441,14\}\}$

Children of Cousin 1240:  $\{\{904,6\},\{1379,11\},\{1405,14\},\{1426,14\},\{1439,14\},\{1440,14\}\}$

Children of Cousin 1241:  $\{\{905,6\},\{1382,11\},\{1406,6\},\{1427,6\},\{1445,6\},\{1447,6\},\{1449,1\}\}$

Children of Cousin 1242:  $\{\{906,1\},\{1375,11\},\{1407,14\},\{1428,14\}\}$

Children of Cousin 1243:  $\{\{906,4\},\{1374,11\},\{1408,14\},\{1429,14\}\}$

Children of Cousin 1244:  $\{\{907,1\},\{1409,14\}\}$

Children of Cousin 1245:  $\{\{909,1\},\{1430,14\},\{1442,11\}\}$

Children of Cousin 1246:  $\{\{911,1\},\{1432,14\},\{1439,11\}\}$

Children of Cousin 1247:  $\{\{911,4\},\{1433,14\},\{1438,11\}\}$

Children of Cousin 1248:  $\{\{912,4\},\{913,1\},\{1381,11\},\{1411,4\},\{1435,4\},\{1446,4\},\{1450,11\},\{1451,4\},\{1452,1\}\}$

Children of Cousin 1249:  $\{\}$

Children of Cousin 1250:  $\{\{916,1\},\{1410,12\},\{1453,1\}\}$

Children of Cousin 1251:  $\{\{917,1\},\{1398,12\}\}$

Children of Cousin 1252:  $\{\{918,1\},\{1453,15\}\}$

Children of Cousin 1253:  $\{\}$

Children of Cousin 1254:  $\{\{1413,12\}\}$

Children of Cousin 1255:  $\{\{920,1\},\{1434,12\},\{1455,1\},\{1457,1\}\}$

Children of Cousin 1256:  $\{\{920,2\},\{1433,12\},\{1456,2\},\{1458,2\}\}$

Children of Cousin 1257:  $\{\{1414,12\}\}$

Children of Cousin 1258:  $\{\{921,1\},\{1431,12\},\{1460,1\}\}$

Children of Cousin 1259:  $\{\{922,1\},\{1455,15\}\}$

Children of Cousin 1260:  $\{\{923,1\},\{1416,12\},\{1457,15\},\{1460,15\}\}$

Children of Cousin 1261:  $\{\{925,1\},\{1401,12\},\{1455,14\}\}$

Children of Cousin 1262:  $\{\{926,1\},\{1419,12\},\{1457,14\}\}$

Children of Cousin 1263:  $\{\{927,1\},\{1419,11\},\{1434,11\}\}$

Children of Cousin 1264:  $\{\{928,1\},\{1401,11\}\}$

Children of Cousin 1265:  $\{\{930,1\},\{1421,12\},\{1453,14\},\{1460,14\}\}$

Children of Cousin 1266:  $\{\{930,3\},\{1422,12\},\{1454,14\},\{1461,14\}\}$

Children of Cousin 1267:  $\{\{931,1\},\{1421,11\},\{1431,11\}\}$

Children of Cousin 1268:  $\{\{932,1\},\{1410,11\}\}$

Children of Cousin 1269:  $\{\}$

Children of Cousin 1270:  $\{\}$

Children of Cousin 1271:  $\{\{938,1\},\{1463,1\},\{1465,1\}\}$

Children of Cousin 1272:  $\{\{939,1\},\{1466,12\}\}$

Children of Cousin 1273:  $\{\{940,1\},\{1463,15\}\}$

Children of Cousin 1274:  $\{\{941,1\},\{941,5\},\{1465,15\},\{1466,15\}\}$

Children of Cousin 1275:  $\{\}$

Children of Cousin 1276:  $\{\{943,1\},\{1388,10\},\{1468,1\}\}$

Children of Cousin 1277:  $\{\}$

Children of Cousin 1278:  $\{\{944,1\},\{1385,10\},\{1469,1\}\}$

Children of Cousin 1279:  $\{\{945,1\},\{1469,15\}\}$

Children of Cousin 1280:  $\{\{946,1\},\{1468,15\}\}$

Children of Cousin 1281:  $\{\}$

Children of Cousin 1282:  $\{\}$

Children of Cousin 1283:  $\{\{948,1\},\{1470,1\},\{1472,1\}\}$

Children of Cousin 1284:  $\{\{949,1\},\{1470,15\}\}$

Children of Cousin 1285:  $\{\{950,1\},\{1472,15\}\}$

Children of Cousin 1286:  $\{\}$

Children of Cousin 1287:  $\{\{952,1\},\{1384,11\},\{1463,14\},\{1470,14\},\{1473,1\}\}$

Children of Cousin 1288:  $\{\{952,3\},\{1383,11\},\{1464,14\},\{1471,14\},\{1474,3\}\}$

Children of Cousin 1289:  $\{\{953,1\},\{1473,15\}\}$



Children of Cousin 1290: {{954,1},{1465,14},{1472,14}}

Children of Cousin 1291: {{956,1},{1466,11},{1468,14}}

Children of Cousin 1292: {{958,1},{1469,14},{1473,14}}

Children of Cousin 1293: {{962,1},{1397,13}}

Children of Cousin 1294: {{963,1},{1400,13}}

Children of Cousin 1295: {{965,1},{1403,13},{1453,13},{1463,13}}

Children of Cousin 1296: {{965,3},{1404,13},{1454,13},{1464,13}}

Children of Cousin 1297: {{966,1},{1405,10}}

Children of Cousin 1298: {{967,1},{1399,10},{1410,13},{1465,13}}

Children of Cousin 1299: {{967,5},{1398,10},{1409,13},{1466,13}}

Children of Cousin 1300: {{969,1},{1407,13}}

Children of Cousin 1301: {{973,5},{1412,13},{1467,13},{1477,5}}

Children of Cousin 1302: {}

Children of Cousin 1303: {{974,1},{1455,13},{1478,1}}

Children of Cousin 1304: {{1413,10}}

Children of Cousin 1305: {{975,1},{1457,13},{1479,1}}

Children of Cousin 1306: {}

Children of Cousin 1307: {{976,1},{1478,15},{1481,1}}

Children of Cousin 1308: {{977,1},{1434,13},{1479,15},{1481,15}}

Children of Cousin 1309: {{977,5},{1432,13},{1480,15},{1481,14}}

Children of Cousin 1310: {{1413,13}}

Children of Cousin 1311: {{1414,13}}

Children of Cousin 1312: {{979,1},{1415,13},{1483,1},{1485,1}}

Children of Cousin 1313: {{980,1},{1418,13},{1483,15}}

Children of Cousin 1314: {{981,1},{1420,13},{1485,15}}

Children of Cousin 1315: {{1414,10}}

Children of Cousin 1316: {{983,1},{1424,13},{1460,13},{1483,14},{1486,1}}

Children of Cousin 1317: {{983,3},{1425,13},{1461,13},{1484,14},{1487,3},{1487,12}}

Children of Cousin 1318: {{984,1},{1426,10},{1480,12},{1485,14}}

Children of Cousin 1319: {{985,1},{1417,10},{1431,13},{1480,14},{1486,15}}

Children of Cousin 1320: {{985,5},{1416,10},{1430,13},{1479,14},{1486,14}}

Children of Cousin 1321: {{987,1},{1428,13},{1478,14}}

Children of Cousin 1322: {{991,5},{1436,13},{1482,5},{1489,5}}

Children of Cousin 1323: {{992,1}}

Children of Cousin 1324: {{993,1}}

Children of Cousin 1325: {{995,1},{1387,10},{1478,13}}

Children of Cousin 1326: {{996,1},{1401,10},{1468,13}}

Children of Cousin 1327: {{998,1},{1419,10},{1469,13},{1479,13}}

Children of Cousin 1328:  $\{\{1000,1\},\{1481,13\}\}$

Children of Cousin 1329:  $\{\{1004,1\},\{1437,13\},\{1470,13\},\{1483,13\}\}$

Children of Cousin 1330:  $\{\{1004,3\},\{1438,13\},\{1471,13\},\{1484,13\}\}$

Children of Cousin 1331:  $\{\{1005,1\},\{1440,13\},\{1485,13\}\}$

Children of Cousin 1332:  $\{\{1006,1\},\{1443,13\},\{1472,13\}\}$

Children of Cousin 1333:  $\{\{1011,1\},\{1444,10\}\}$

Children of Cousin 1334:  $\{\{1015,1\},\{1421,10\},\{1442,10\},\{1473,13\},\{1486,13\}\}$

Children of Cousin 1335:  $\{\{1015,3\},\{1422,10\},\{1441,10\},\{1474,13\},\{1487,11\},\{1487,13\}\}$

Children of Cousin 1336:  $\{\{1016,3\},\{1017,1\},\{1392,10\},\{1448,13\},\{1462,13\},\{1475,13\},\{1476,13\},\{1488,13\},\{1490,13\},\{1491,1\}\}$

Children of Cousin 1337:  $\{\{1018,1\},\{1439,10\},\{1480,11\}\}$

Children of Cousin 1338:  $\{\{1026,3\},\{1404,12\}\}$

Children of Cousin 1339:  $\{\}$

Children of Cousin 1340:  $\{\{1027,3\},\{1454,12\},\{1456,12\},\{1492,3\}\}$

Children of Cousin 1341:  $\{\{1028,4\},\{1493,15\}\}$

Children of Cousin 1342:  $\{\{1029,4\},\{1408,12\},\{1493,14\}\}$

Children of Cousin 1343:  $\{\{1031,3\},\{1425,12\},\{1458,12\},\{1461,12\}\}$

Children of Cousin 1344:  $\{\{1032,4\},\{1429,12\},\{1492,11\}\}$

Children of Cousin 1345:  $\{\{1034,3\},\{1438,12\},\{1458,11\}\}$

Children of Cousin 1346:  $\{\{1035,4\},\{1441,12\},\{1461,11\}\}$

Children of Cousin 1347:  $\{\{1037,4\},\{1454,11\}\}$

Children of Cousin 1348:  $\{\{1040,3\},\{1456,11\}\}$

Children of Cousin 1349:  $\{\{1043,3\},\{1043,4\},\{1372,11\},\{1492,13\},\{1493,13\}\}$

Children of Cousin 1350:  $\{\{1049,3\},\{1464,12\}\}$

Children of Cousin 1351:  $\{\}$

Children of Cousin 1352:  $\{\{1050,3\},\{1386,11\},\{1495,3\}\}$

Children of Cousin 1353:  $\{\{1055,3\},\{1471,12\}\}$

Children of Cousin 1354:  $\{\{1058,3\},\{1474,12\}\}$

Children of Cousin 1355:  $\{\{1060,3\},\{1464,11\},\{1495,13\}\}$

Children of Cousin 1356:  $\{\{1062,3\},\{1492,12\}\}$

Children of Cousin 1357:  $\{\{1065,3\},\{1456,10\}\}$

Children of Cousin 1358:  $\{\}$

Children of Cousin 1359:  $\{\{1067,3\},\{1493,10\},\{1496,3\},\{1496,13\}\}$

Children of Cousin 1360:  $\{\}$

Children of Cousin 1361:  $\{\{1071,3\},\{1458,10\},\{1484,12\},\{1497,3\},\{1497,13\}\}$

Children of Cousin 1362:  $\{\{1075,3\}\}$

Children of Cousin 1363:  $\{\{1079,3\},\{1394,11\},\{1496,11\},\{1496,12\}\}$

Children of Cousin 1364:  $\{\{1080,3\},\{1408,10\},\{1495,12\}\}$

Children of Cousin 1365:  $\{\{1085,3\}\}$

Children of Cousin 1366: {{1088,3},{1429,10}}

Children of Cousin 1367: {{1091,3},{1497,11},{1497,12}}

Children of Cousin 1368: {{1096,3},{1433,10},{1484,11}}

Children of Cousin 1369: {{1105,3},{1471,11}}

Children of Cousin 1370: {{1109,3},{1390,11},{1495,11}}

Children of Cousin 1371: {{1110,3},{1474,11}}

Children of Cousin 1372: {{1150,2},{1150,3}}

Children of Cousin 1373: {{1150,6}}

Children of Cousin 1374: {{1151,2}}

Children of Cousin 1375: {{1151,5}}

Children of Cousin 1376: {{1151,6}}

Children of Cousin 1377: {{1152,6},{1153,2},{1499,2},{1501,2}}

Children of Cousin 1378: {{1154,2}}

Children of Cousin 1379: {{1154,5}}

Children of Cousin 1380: {{1154,7}}

Children of Cousin 1381: {{1157,5},{1158,2},{1500,5},{1503,5}}

Children of Cousin 1382: {{1161,7},{1505,14}}

Children of Cousin 1383: {{1163,3}}

Children of Cousin 1384: {{1163,5}}

Children of Cousin 1385: {{1165,4},{1165,5}}

Children of Cousin 1386: {{1168,3}}

Children of Cousin 1387: {{1168,4}}

Children of Cousin 1388: {{1170,4},{1170,5}}

Children of Cousin 1389: {{1175,5},{1507,14},{1509,14}}

Children of Cousin 1390: {{1176,3},{1176,6}}

Children of Cousin 1391: {{1177,6},{1178,3},{1501,10},{1510,3},{1510,12}}

Children of Cousin 1392: {{1179,6},{1180,4},{1504,10},{1506,12}}

Children of Cousin 1393: {{1185,4},{1186,3},{1502,12},{1508,13}}

Children of Cousin 1394: {{1187,3},{1187,6}}

Children of Cousin 1395: {{1188,6},{1189,3},{1499,10},{1511,3},{1511,12}}

Children of Cousin 1396: {{1193,6}}

Children of Cousin 1397: {{1195,1}}

Children of Cousin 1398: {{1195,2}}

Children of Cousin 1399: {{1195,6}}

Children of Cousin 1400: {{1196,1}}

Children of Cousin 1401: {{1196,2}}

Children of Cousin 1402: {{1197,2},{1198,1},{1512,1},{1515,1}}

Children of Cousin 1403: {{1199,1}}

Children of Cousin 1404: {{1199,3}}

Children of Cousin 1405: {{1199,6}}

Children of Cousin 1406: {{1200,6},{1513,6},{1517,1}}

Children of Cousin 1407: {{1201,1}}

Children of Cousin 1408: {{1201,4}}

Children of Cousin 1409: {{1202,1}}

Children of Cousin 1410: {{1202,5}}

Children of Cousin 1411: {{1205,4},{1206,1},{1518,11},{1519,4}}

Children of Cousin 1412: {{1207,5},{1208,1},{1514,11},{1520,5}}

Children of Cousin 1413: {}

Children of Cousin 1414: {}

Children of Cousin 1415: {{1209,1},{1521,1},{1525,1}}

Children of Cousin 1416: {{1209,2},{1522,2},{1526,2}}

Children of Cousin 1417: {{1209,6},{1524,6},{1528,6}}

Children of Cousin 1418: {{1210,1},{1521,16}}

Children of Cousin 1419: {{1210,2},{1522,16}}

Children of Cousin 1420: {{1211,1},{1525,16}}

Children of Cousin 1421: {{1211,2},{1526,16}}

Children of Cousin 1422: {{1211,4},{1527,16}}

Children of Cousin 1423: {{1212,2},{1213,1},{1529,1},{1532,1},{1533,1}}

Children of Cousin 1424: {{1214,1},{1521,15},{1528,15}}

Children of Cousin 1425: {{1214,3},{1523,15},{1527,15}}

Children of Cousin 1426: {{1214,6},{1524,15},{1525,15}}

Children of Cousin 1427: {{1215,6},{1530,6},{1537,1}}

Children of Cousin 1428: {{1216,1}}

Children of Cousin 1429: {{1216,4}}

Children of Cousin 1430: {{1218,1},{1528,11}}

Children of Cousin 1431: {{1218,5},{1526,11}}

Children of Cousin 1432: {{1220,1},{1524,11}}

Children of Cousin 1433: {{1220,4},{1523,11}}

Children of Cousin 1434: {{1220,5},{1522,11}}

Children of Cousin 1435: {{1221,4},{1222,1},{1534,4},{1538,11},{1539,4},{1541,1}}

Children of Cousin 1436: {{1223,5},{1224,1},{1531,11},{1540,5},{1542,5}}

Children of Cousin 1437: {{1225,1},{1521,14}}

Children of Cousin 1438: {{1225,3},{1523,14}}

Children of Cousin 1439: {{1225,6},{1524,14}}

Children of Cousin 1440: {{1226,1},{1525,14}}

Children of Cousin 1441: {{1226,4},{1527,14}}

Children of Cousin 1442: {{1226,6},{1528,14}}

Children of Cousin 1443: {{1227,1}}

Children of Cousin 1444: {{1227,6}}

Children of Cousin 1445: {{1228,6},{1229,1},{1530,14},{1545,1},{1548,1},{1550,1}}

Children of Cousin 1446: {{1231,4},{1232,1},{1534,14},{1547,4}}

Children of Cousin 1447: {{1234,6},{1235,1},{1513,14},{1550,14}}

Children of Cousin 1448: {{1238,3},{1239,1},{1504,11},{1516,14},{1536,14},{1544,14},{1549,14}}

Children of Cousin 1449: {{1238,6},{1240,1},{1505,11},{1517,14},{1537,14},{1545,14},{1548,14}}

Children of Cousin 1450: {{1239,6},{1240,3},{1503,11},{1518,14},{1538,14},{1546,14},{1547,14}}

Children of Cousin 1451: {{1242,4},{1243,1},{1500,11},{1519,14},{1539,14}}

Children of Cousin 1452: {{1246,4},{1247,1},{1541,14},{1546,11}}

Children of Cousin 1453: {{1249,1}}

Children of Cousin 1454: {{1249,3}}

Children of Cousin 1455: {{1253,1}}

Children of Cousin 1456: {{1253,2}}

Children of Cousin 1457: {{1254,1},{1522,12}}

Children of Cousin 1458: {{1254,2},{1523,12}}

Children of Cousin 1459: {{1255,2},{1256,1},{1543,12},{1553,1},{1554,1}}

Children of Cousin 1460: {{1257,1},{1526,12}}

Children of Cousin 1461: {{1257,3},{1527,12}}

Children of Cousin 1462: {{1265,3},{1266,1},{1535,12},{1552,14},{1555,14}}

Children of Cousin 1463: {{1269,1}}

Children of Cousin 1464: {{1269,3}}

Children of Cousin 1465: {{1270,1}}

Children of Cousin 1466: {{1270,5}}

Children of Cousin 1467: {{1274,5},{1557,5}}

Children of Cousin 1468: {{1275,1}}

Children of Cousin 1469: {{1277,1}}

Children of Cousin 1470: {{1281,1}}

Children of Cousin 1471: {{1281,3}}

Children of Cousin 1472: {{1282,1}}

Children of Cousin 1473: {{1286,1}}

Children of Cousin 1474: {{1286,3}}

Children of Cousin 1475: {{1287,3},{1288,1},{1506,11},{1556,14},{1558,14},{1559,1}}

Children of Cousin 1476: {{1295,3},{1296,1},{1516,13},{1552,13},{1556,13}}

Children of Cousin 1477: {{1298,5},{1299,1},{1514,10},{1520,13},{1557,13}}

Children of Cousin 1478: {{1302,1}}

Children of Cousin 1479: {{1304,1},{1522,10}}

Children of Cousin 1480: {{1304,5},{1524,10}}

Children of Cousin 1481: {{1306,1},{1306,5}}

Children of Cousin 1482: {{1308,5},{1309,1},{1542,13},{1560,5},{1561,5},{1561,14}}

Children of Cousin 1483: {{1310,1},{1521,13}}

Children of Cousin 1484: {{1310,3},{1523,13}}

Children of Cousin 1485: {{1311,1},{1525,13}}

Children of Cousin 1486: {{1315,1},{1315,5},{1526,10},{1528,10}}

Children of Cousin 1487: {{1315,3},{1527,10}}

Children of Cousin 1488: {{1316,3},{1317,1},{1536,13},{1555,13},{1562,14},{1563,1}}

Children of Cousin 1489: {{1319,5},{1320,1},{1531,10},{1540,13},{1560,14},{1564,5},{1564,14}}

Children of Cousin 1490: {{1329,3},{1330,1},{1544,13},{1558,13},{1562,13}}

Children of Cousin 1491: {{1334,3},{1335,1},{1535,10},{1549,10},{1559,13},{1563,13}}

Children of Cousin 1492: {{1339,3}}

Children of Cousin 1493: {{1339,4}}

Children of Cousin 1494: {{1349,4},{1498,11},{1565,13}}

Children of Cousin 1495: {{1351,3}}

Children of Cousin 1496: {{1358,3}}

Children of Cousin 1497: {{1360,3}}

Children of Cousin 1498: {{1372,3}}

Children of Cousin 1499: {{1372,6},{1373,2},{1373,3}}

Children of Cousin 1500: {{1374,5},{1375,2}}

Children of Cousin 1501: {{1374,6},{1376,2}}

Children of Cousin 1502: {{1375,6},{1376,5}}

Children of Cousin 1503: {{1378,5},{1379,2}}

Children of Cousin 1504: {{1378,7},{1380,2}}

Children of Cousin 1505: {{1379,7},{1380,5}}

Children of Cousin 1506: {{1383,5},{1384,3}}

Children of Cousin 1507: {{1385,5}}

Children of Cousin 1508: {{1386,4},{1387,3}}

Children of Cousin 1509: {{1388,5}}

Children of Cousin 1510: {{1390,6}}

Children of Cousin 1511: {{1394,6}}

Children of Cousin 1512: {{1397,2},{1398,1}}

Children of Cousin 1513: {{1397,6},{1399,1}}

Children of Cousin 1514: {{1398,6},{1399,2}}

Children of Cousin 1515: {{1400,2},{1401,1}}

Children of Cousin 1516: {{1403,3},{1404,1}}

Children of Cousin 1517: {{1403,6},{1405,1}}

Children of Cousin 1518:  $\{\{1404,6\},\{1405,3\}\}$

Children of Cousin 1519:  $\{\{1407,4\},\{1408,1\}\}$

Children of Cousin 1520:  $\{\{1409,5\},\{1410,1\}\}$

Children of Cousin 1521:  $\{\{1413,1\}\}$

Children of Cousin 1522:  $\{\{1413,2\}\}$

Children of Cousin 1523:  $\{\{1413,3\}\}$

Children of Cousin 1524:  $\{\{1413,6\}\}$

Children of Cousin 1525:  $\{\{1414,1\}\}$

Children of Cousin 1526:  $\{\{1414,2\}\}$

Children of Cousin 1527:  $\{\{1414,4\}\}$

Children of Cousin 1528:  $\{\{1414,6\}\}$

Children of Cousin 1529:  $\{\{1415,2\},\{1416,1\},\{1571,1\},\{1577,1\}\}$

Children of Cousin 1530:  $\{\{1415,6\},\{1417,1\},\{1573,1\},\{1579,1\}\}$

Children of Cousin 1531:  $\{\{1416,6\},\{1417,2\},\{1575,2\},\{1581,2\}\}$

Children of Cousin 1532:  $\{\{1418,2\},\{1419,1\},\{1571,2\}\}$

Children of Cousin 1533:  $\{\{1420,2\},\{1421,1\},\{1577,2\}\}$

Children of Cousin 1534:  $\{\{1420,4\},\{1422,1\},\{1578,4\}\}$

Children of Cousin 1535:  $\{\{1421,4\},\{1422,2\},\{1580,4\}\}$

Children of Cousin 1536:  $\{\{1424,3\},\{1425,1\},\{1572,15\},\{1582,15\}\}$

Children of Cousin 1537:  $\{\{1424,6\},\{1426,1\},\{1573,15\},\{1579,15\}\}$

Children of Cousin 1538:  $\{\{1425,6\},\{1426,3\},\{1576,15\},\{1578,15\}\}$

Children of Cousin 1539:  $\{\{1428,4\},\{1429,1\}\}$

Children of Cousin 1540:  $\{\{1430,5\},\{1431,1\},\{1581,11\}\}$

Children of Cousin 1541:  $\{\{1432,4\},\{1433,1\},\{1576,11\}\}$

Children of Cousin 1542:  $\{\{1432,5\},\{1434,1\},\{1575,11\}\}$

Children of Cousin 1543:  $\{\{1433,5\},\{1434,4\},\{1574,11\}\}$

Children of Cousin 1544:  $\{\{1437,3\},\{1438,1\},\{1572,14\}\}$

Children of Cousin 1545:  $\{\{1437,6\},\{1439,1\},\{1573,14\}\}$

Children of Cousin 1546:  $\{\{1438,6\},\{1439,3\},\{1576,14\}\}$

Children of Cousin 1547:  $\{\{1440,4\},\{1441,1\},\{1578,14\}\}$

Children of Cousin 1548:  $\{\{1440,6\},\{1442,1\},\{1579,14\}\}$

Children of Cousin 1549:  $\{\{1441,6\},\{1442,4\},\{1582,14\}\}$

Children of Cousin 1550:  $\{\{1443,6\},\{1444,1\}\}$

Children of Cousin 1551:  $\{\{1448,6\},\{1449,3\},\{1450,1\},\{1568,11\},\{1570,6\},\{1585,6\},\{1587,6\},\{1588,6\},\{1589,13\}\}$

Children of Cousin 1552:  $\{\{1453,3\},\{1454,1\}\}$

Children of Cousin 1553:  $\{\{1455,2\},\{1456,1\}\}$

Children of Cousin 1554:  $\{\{1457,2\},\{1458,1\},\{1574,12\}\}$

Children of Cousin 1555:  $\{\{1460,3\},\{1461,1\},\{1580,12\}\}$

Children of Cousin 1556:  $\{\{1463,3\},\{1464,1\}\}$

Children of Cousin 1557:  $\{\{1465,5\},\{1466,1\}\}$

Children of Cousin 1558:  $\{\{1470,3\},\{1471,1\}\}$

Children of Cousin 1559:  $\{\{1473,3\},\{1474,1\}\}$

Children of Cousin 1560:  $\{\{1479,5\},\{1480,1\},\{1575,10\}\}$

Children of Cousin 1561:  $\{\{1481,5\}\}$

Children of Cousin 1562:  $\{\{1483,3\},\{1484,1\},\{1572,13\}\}$

Children of Cousin 1563:  $\{\{1486,3\},\{1487,1\},\{1487,5\},\{1580,10\},\{1582,10\}\}$

Children of Cousin 1564:  $\{\{1486,5\},\{1581,10\}\}$

Children of Cousin 1565:  $\{\{1492,4\},\{1493,3\}\}$

Children of Cousin 1566:  $\{\{1498,6\},\{1499,3\}\}$

Children of Cousin 1567:  $\{\{1500,6\},\{1501,5\},\{1502,2\}\}$

Children of Cousin 1568:  $\{\{1503,7\},\{1504,5\},\{1505,2\},\{1591,14\}\}$

Children of Cousin 1569:  $\{\{1512,6\},\{1513,2\},\{1514,1\}\}$

Children of Cousin 1570:  $\{\{1516,6\},\{1517,3\},\{1518,1\},\{1592,14\}\}$

Children of Cousin 1571:  $\{\{1521,2\},\{1522,1\}\}$

Children of Cousin 1572:  $\{\{1521,3\},\{1523,1\}\}$

Children of Cousin 1573:  $\{\{1521,6\},\{1524,1\}\}$

Children of Cousin 1574:  $\{\{1522,3\},\{1523,2\}\}$

Children of Cousin 1575:  $\{\{1522,6\},\{1524,2\}\}$

Children of Cousin 1576:  $\{\{1523,6\},\{1524,3\}\}$

Children of Cousin 1577:  $\{\{1525,2\},\{1526,1\}\}$

Children of Cousin 1578:  $\{\{1525,4\},\{1527,1\}\}$

Children of Cousin 1579:  $\{\{1525,6\},\{1528,1\}\}$

Children of Cousin 1580:  $\{\{1526,4\},\{1527,2\}\}$

Children of Cousin 1581:  $\{\{1526,6\},\{1528,2\}\}$

Children of Cousin 1582:  $\{\{1527,6\},\{1528,4\}\}$

Children of Cousin 1583:  $\{\{1529,6\},\{1530,2\},\{1531,1\},\{1594,1\},\{1598,1\}\}$

Children of Cousin 1584:  $\{\{1533,4\},\{1534,2\},\{1535,1\},\{1597,2\}\}$

Children of Cousin 1585:  $\{\{1536,6\},\{1537,3\},\{1538,1\},\{1595,6\},\{1599,6\},\{1601,14\}\}$

Children of Cousin 1586:  $\{\{1541,5\},\{1542,4\},\{1543,1\},\{1596,11\}\}$

Children of Cousin 1587:  $\{\{1544,6\},\{1545,3\},\{1546,1\},\{1595,14\},\{1602,14\}\}$

Children of Cousin 1588:  $\{\{1547,6\},\{1548,4\},\{1549,1\},\{1599,14\},\{1603,14\}\}$

Children of Cousin 1589:  $\{\{1591,11\},\{1592,6\},\{1601,6\},\{1602,6\},\{1603,6\}\}$

Children of Cousin 1590:  $\{\{1563,5\},\{1564,3\},\{1600,10\}\}$

Children of Cousin 1591:  $\{\}$

Children of Cousin 1592:  $\{\}$

Children of Cousin 1593:  $\{\{1571,3\},\{1572,2\},\{1574,1\}\}$



Children of Cousin 1594:  $\{\{1571,6\},\{1573,2\},\{1575,1\}\}$

Children of Cousin 1595:  $\{\{1572,6\},\{1573,3\},\{1576,1\},\{1605,15\}\}$

Children of Cousin 1596:  $\{\{1574,6\},\{1575,3\},\{1576,2\}\}$

Children of Cousin 1597:  $\{\{1577,4\},\{1578,2\},\{1580,1\}\}$

Children of Cousin 1598:  $\{\{1577,6\},\{1579,2\},\{1581,1\}\}$

Children of Cousin 1599:  $\{\{1578,6\},\{1579,4\},\{1582,1\},\{1607,15\}\}$

Children of Cousin 1600:  $\{\{1580,6\},\{1581,4\},\{1582,2\}\}$

Children of Cousin 1601:  $\{\{1605,6\},\{1607,6\}\}$

Children of Cousin 1602:  $\{\{1605,14\}\}$

Children of Cousin 1603:  $\{\{1607,14\}\}$

Children of Cousin 1604:  $\{\{1593,6\},\{1594,3\},\{1595,2\},\{1596,1\},\{1608,14\}\}$

Children of Cousin 1605:  $\{\}$

Children of Cousin 1606:  $\{\{1597,6\},\{1598,4\},\{1599,2\},\{1600,1\},\{1609,14\}\}$

Children of Cousin 1607:  $\{\}$

Children of Cousin 1608:  $\{\{1605,2\}\}$

Children of Cousin 1609:  $\{\{1607,2\}\}$
